# Supplementary material for: When Single Answer Is Not Enough: Rethinking Single-Step Retrosynthesis Benchmarks for LLMs
Source: arXiv:2602.03554 source file (2026-05-29)
Supplement: Supplementary file 1 [file ether0_study.tex]

\section{Influence of prompt formulation on model performance: ether0 case study}
\label{app:ether0_study}

It is now well established that the quality of prompt instructions substantially affects the quality, coherence, and consistency of outputs produced by LLMs. In specialist, domain-specific tasks, prompt quality often becomes a dominant factor because the prompt specifies the scientific assumptions, constraints, and evaluation target. Small changes in wording can therefore shift the task definition and the model’s search space. 

To illustrate the importance of the formulation of LLM inputs in the context of a single-step retrosynthesis task, we launched ether0 on URSA-expert-2026 and USPTO-50K-test with two different templates: original ones and ones we used for benchmarking (see \autoref{app:templates}). The main difference between these template sets is an additional constraint of commercial availability in case of the original ehter0's prompt. Generally, it looks like this: "Propose 1-step retrosynthesis from likely commercially available reagents". This instruction is actually irrelevant for the classical 1-step retrosynthesis task formulation devoid of the purchasability status of reactants. As can be seen from \autoref{tab:ethe0_table}, ether0 showed better CC-based metrics for both sets on the simplified templates. This comparison underpins the importance of prompt design which should be clear and specific to the domain of knowledge.

\begin{table*}[th!]
\centering
\begin{tabular}{@{}l|c|cccc|c|cccc@{}}
\toprule
\multirow{2}{*}{\textbf{Model}} &
\multicolumn{5}{c|}{\textbf{URSA-expert-2026}} &
\multicolumn{5}{c}{\textbf{USPTO-50K-test}} \\
\cline{2-6}\cline{7-11}
& \multirow{2}{*}{\textbf{Unique}} & \multirow{2}{*}{\textbf{Max}} & \multicolumn{3}{c|}{\textbf{Av. PT-Top-K CC}}
& \multirow{2}{*}{\textbf{Unique}} & \multirow{2}{*}{\textbf{Max}} & \multicolumn{3}{c}{\textbf{Av. PT-Top-K CC}} \\
&  &  & \textbf{@3} & \textbf{@5} & \textbf{@10}
&  &  & \textbf{@3} & \textbf{@5} & \textbf{@10} \\
\midrule
ether0, original prompts                     & 20\% & 1.01 & 0.55 & 0.35 & 0.17 & 19\% & 2.08 & 1.07 & 0.67 & 0.34 \\
ether0, revised prompts                   & 24\% & 1.25 & 0.73 & 0.47 & 0.24 & 25\% & 2.17 & 1.24 & 0.79 & 0.40 \\
\bottomrule
\end{tabular}

\caption{The case study on the influence of prompt formulation for SSRS task performance}
\label{tab:ethe0_table}
\end{table*}
