# Supplementary material for: When Single Answer Is Not Enough: Rethinking Single-Step Retrosynthesis Benchmarks for LLMs
Source: arXiv:2602.03554 source file (2026-05-29)
Supplement: Supplementary file 2 [file Expert_Data_Set.pdf]

|                                                                                     |                                                                                     |                                                                                      |                                                                                       |
|-------------------------------------------------------------------------------------|-------------------------------------------------------------------------------------|--------------------------------------------------------------------------------------|---------------------------------------------------------------------------------------|
| 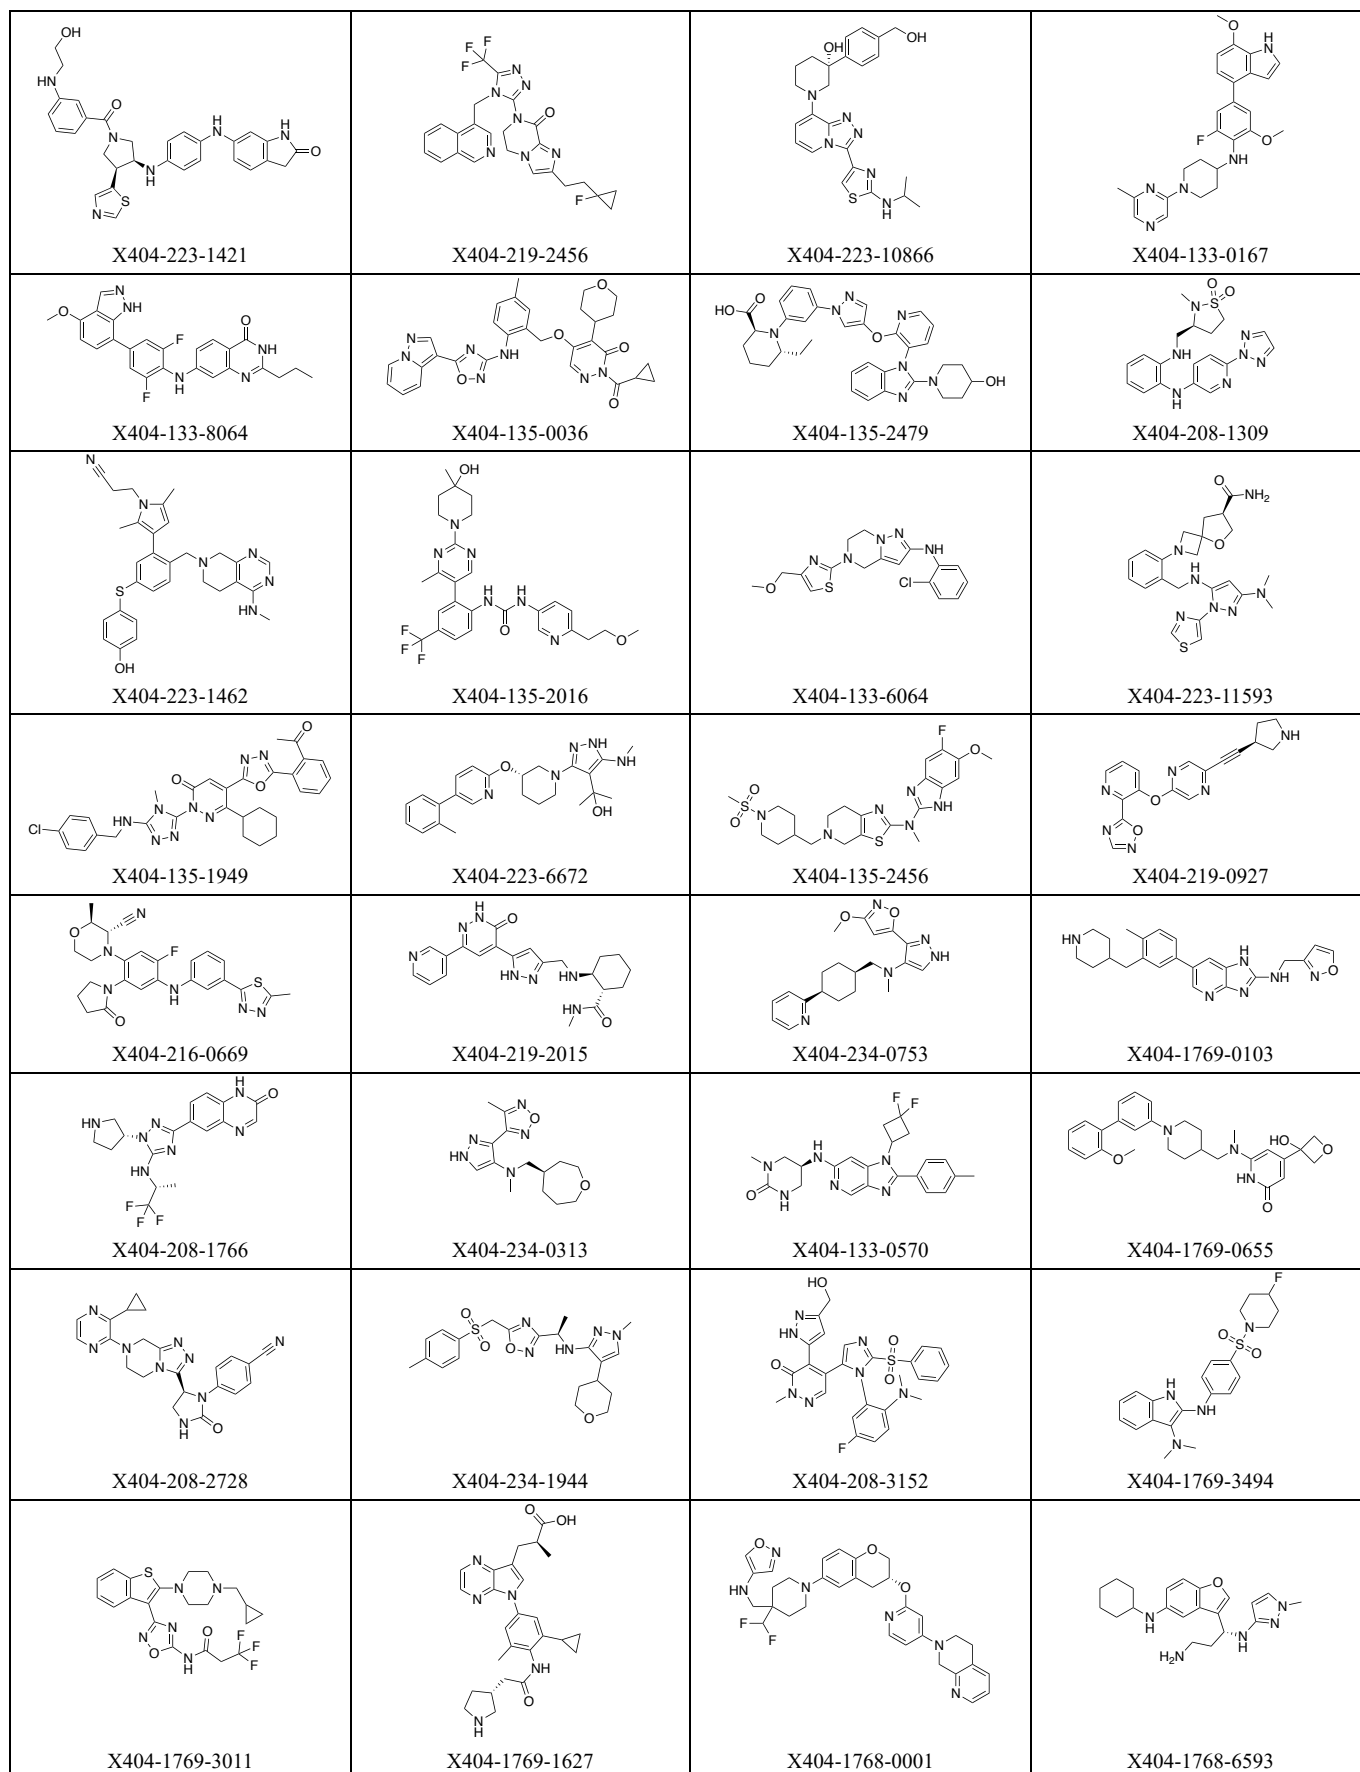   | 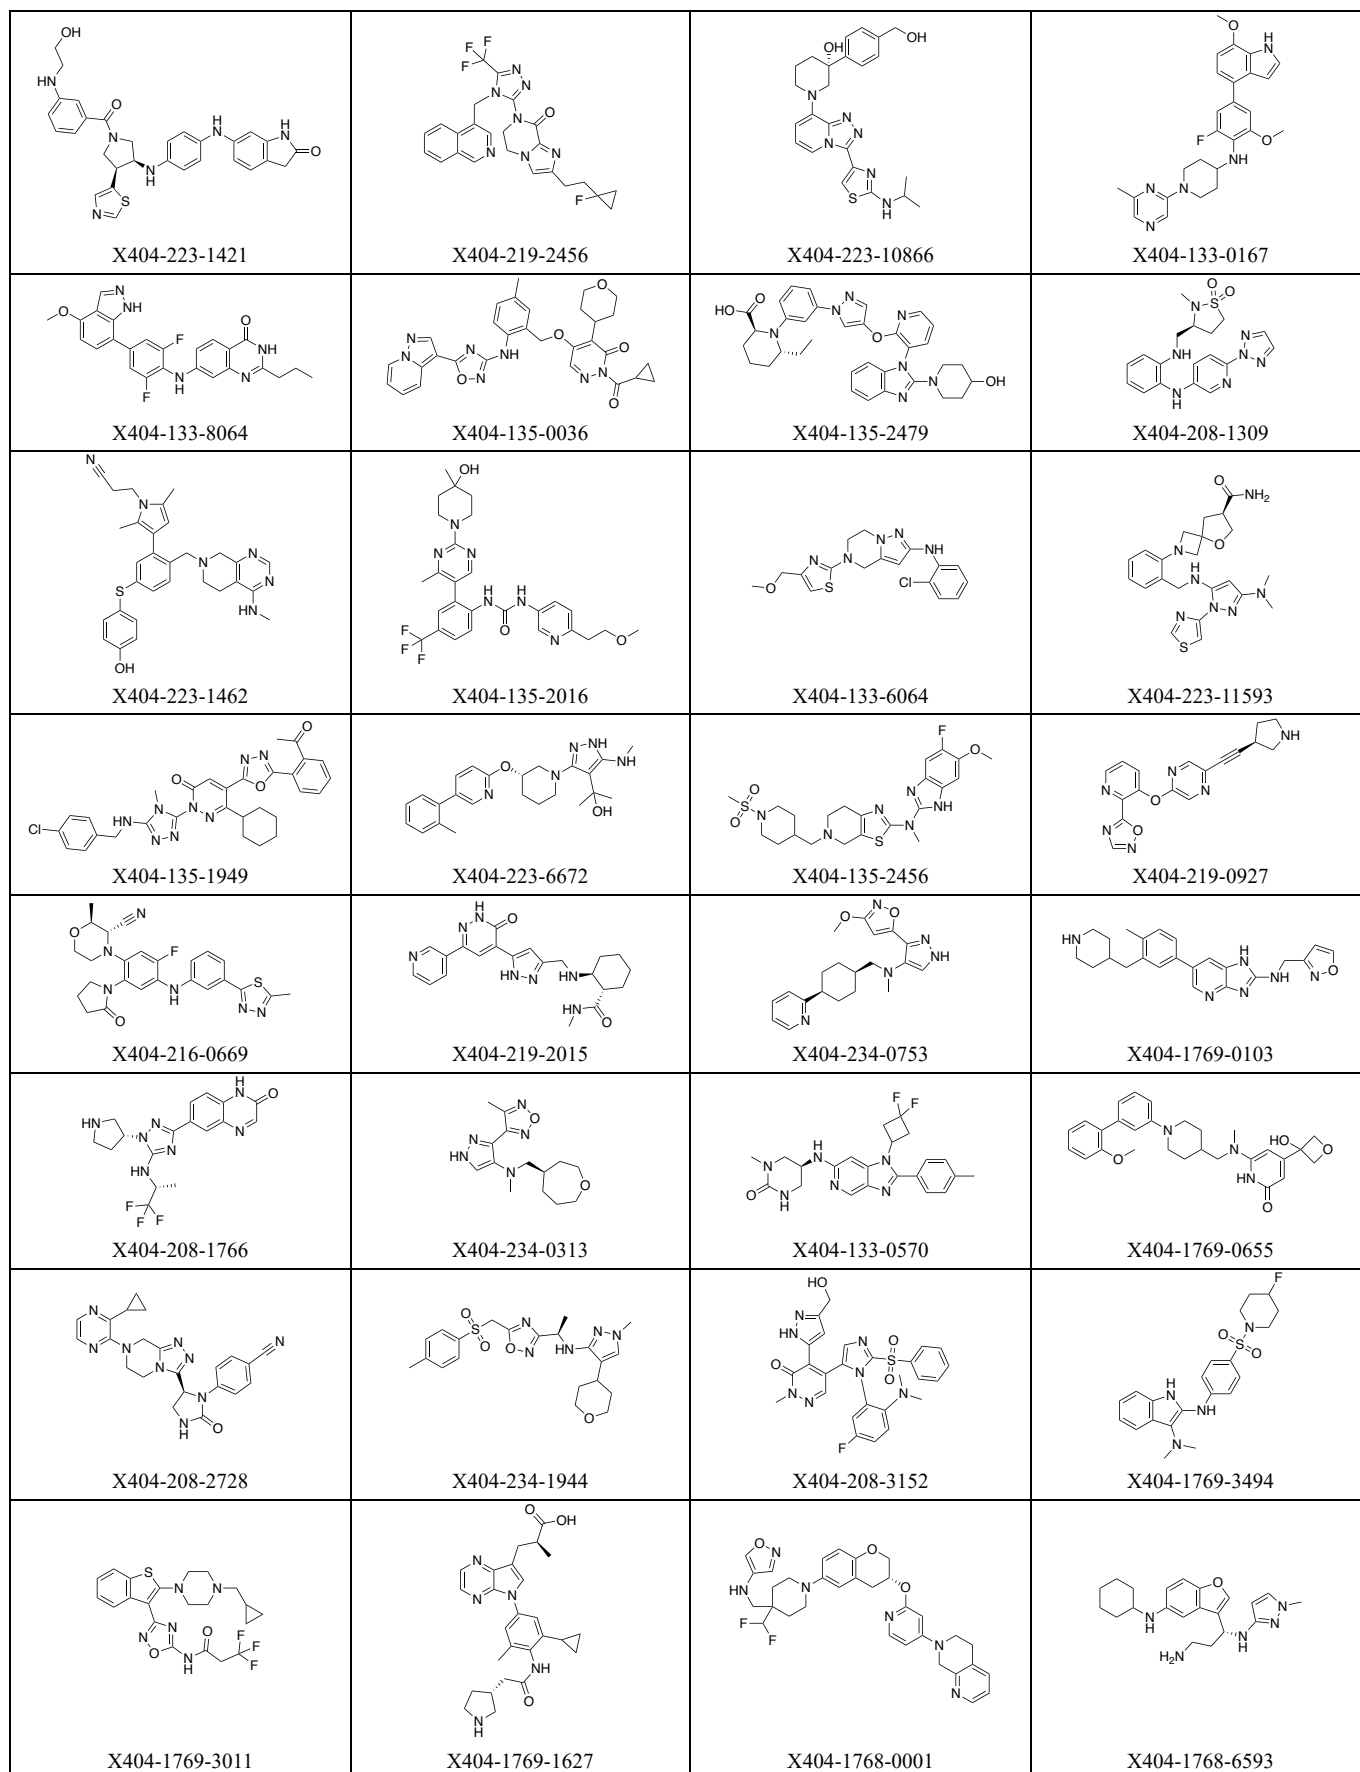   | 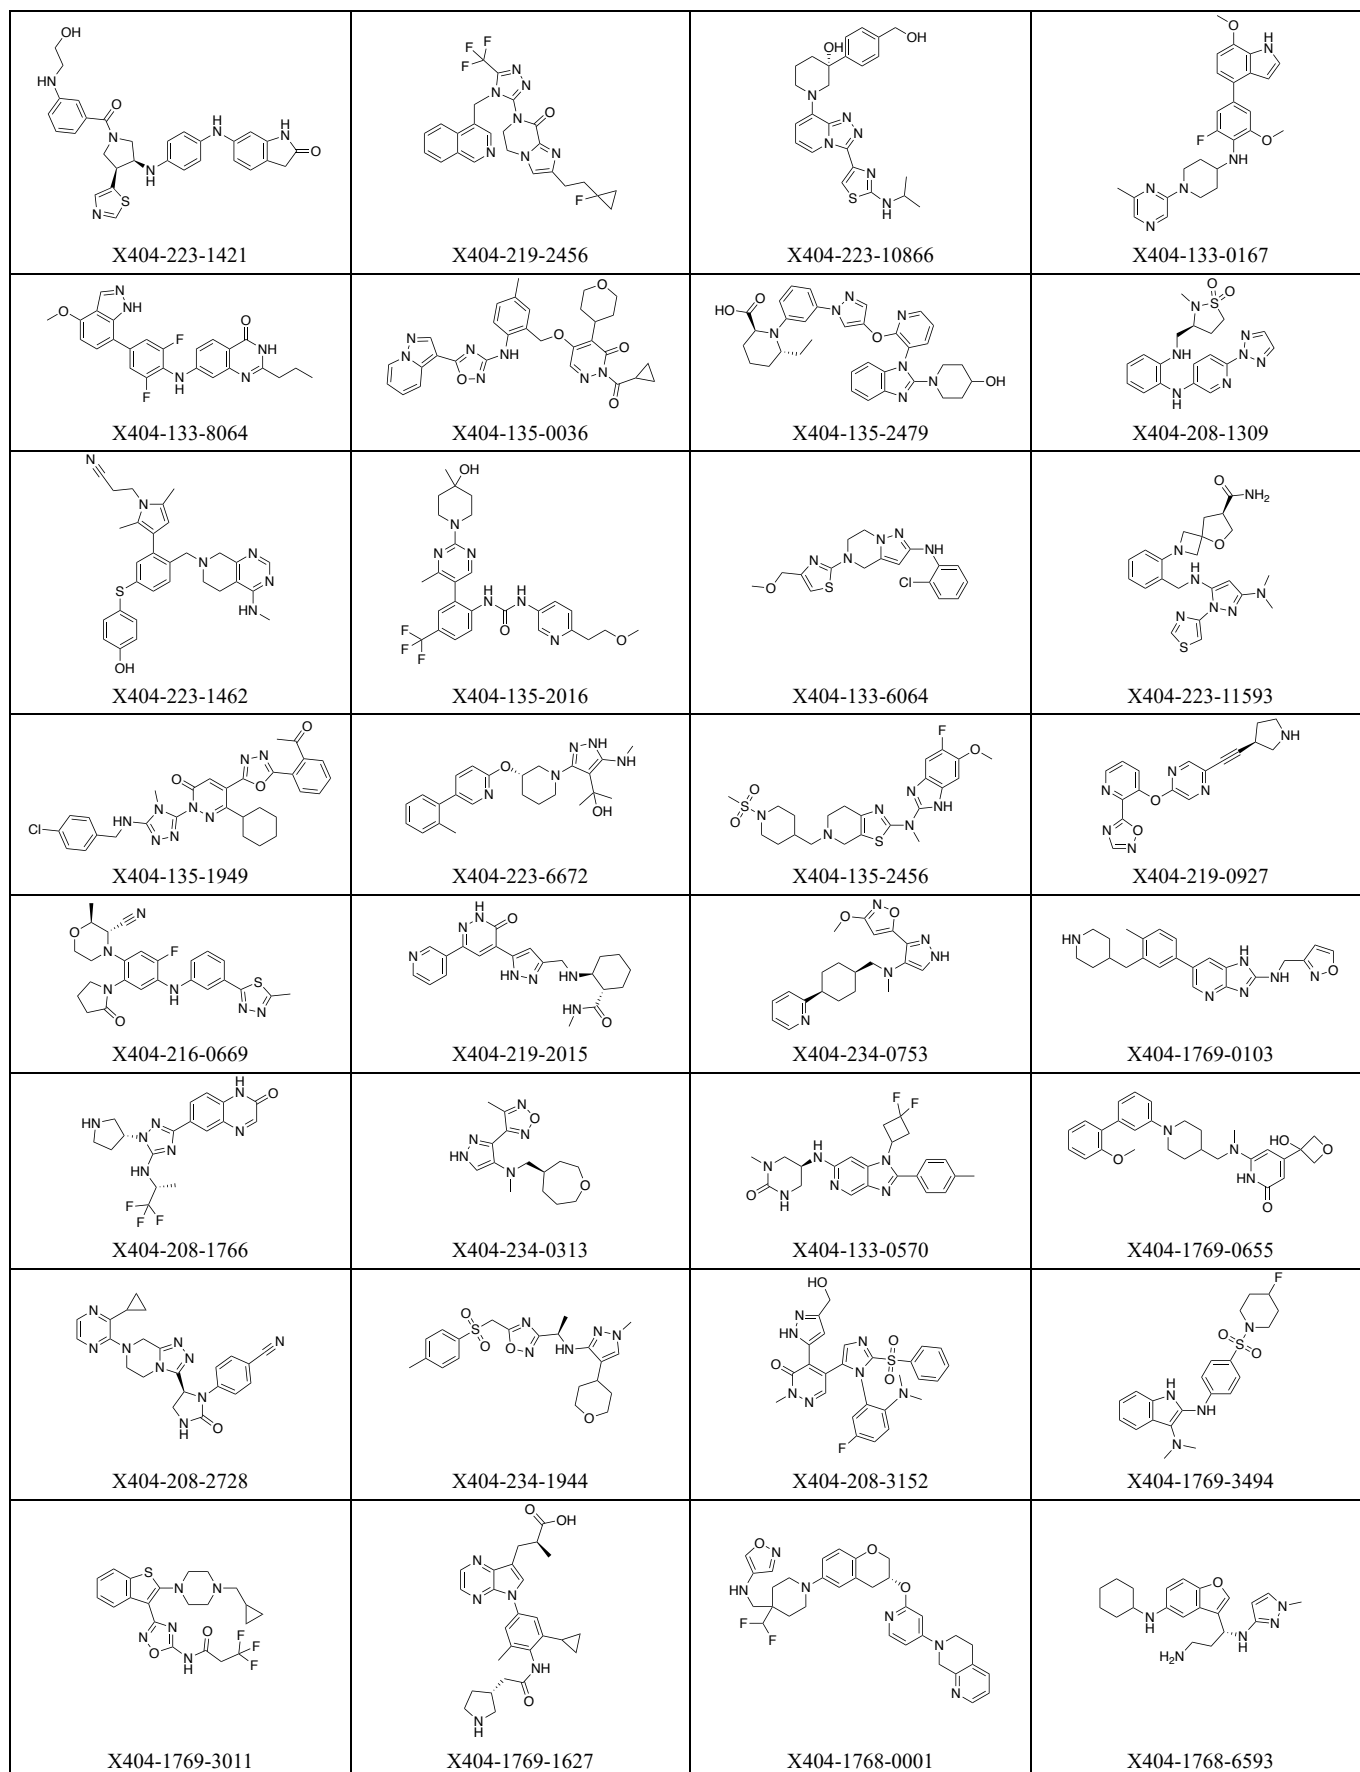   | 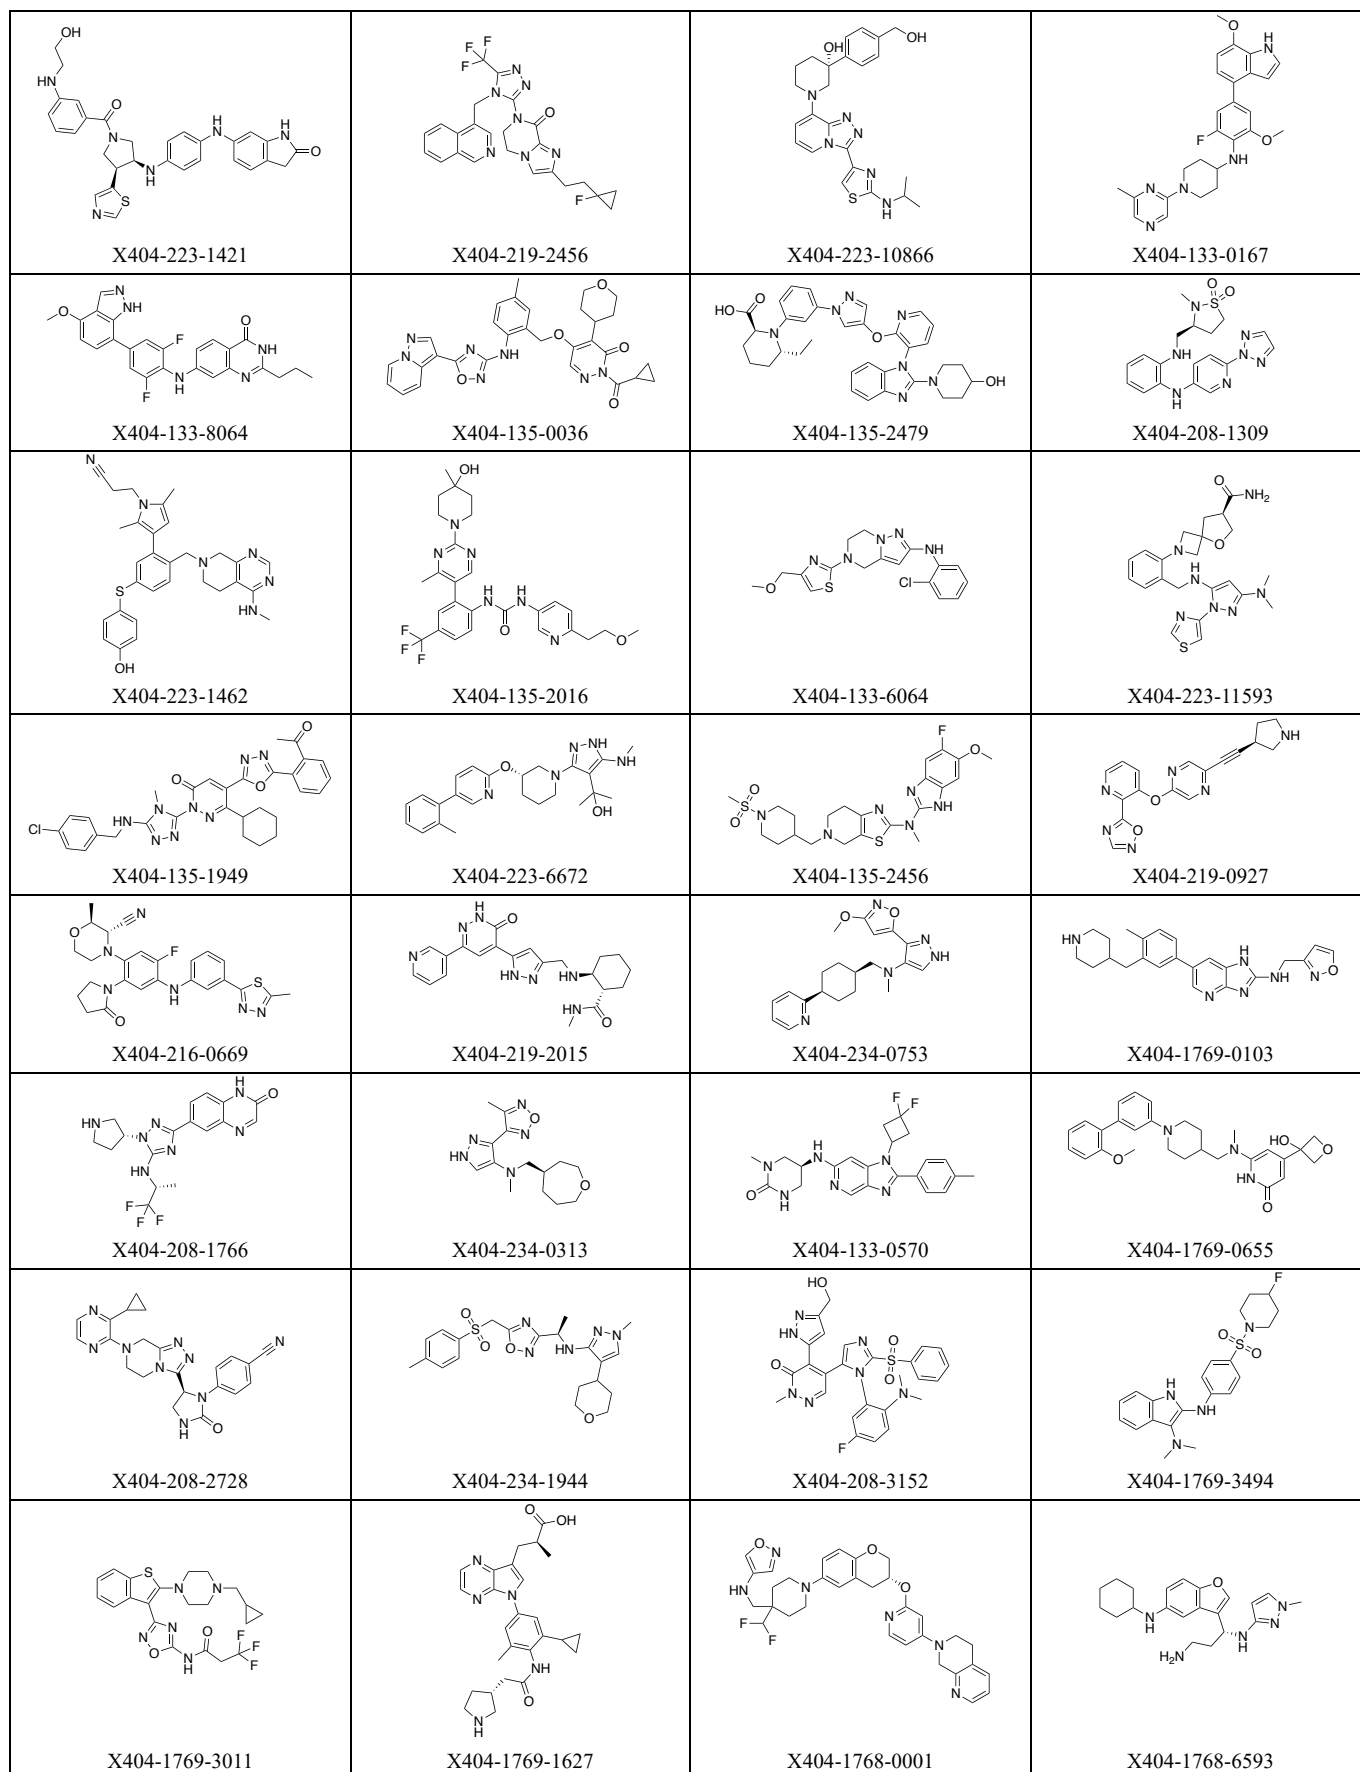   |
| X404-223-1421                                                                       | X404-219-2456                                                                       | X404-223-10866                                                                       | X404-133-0167                                                                         |
| 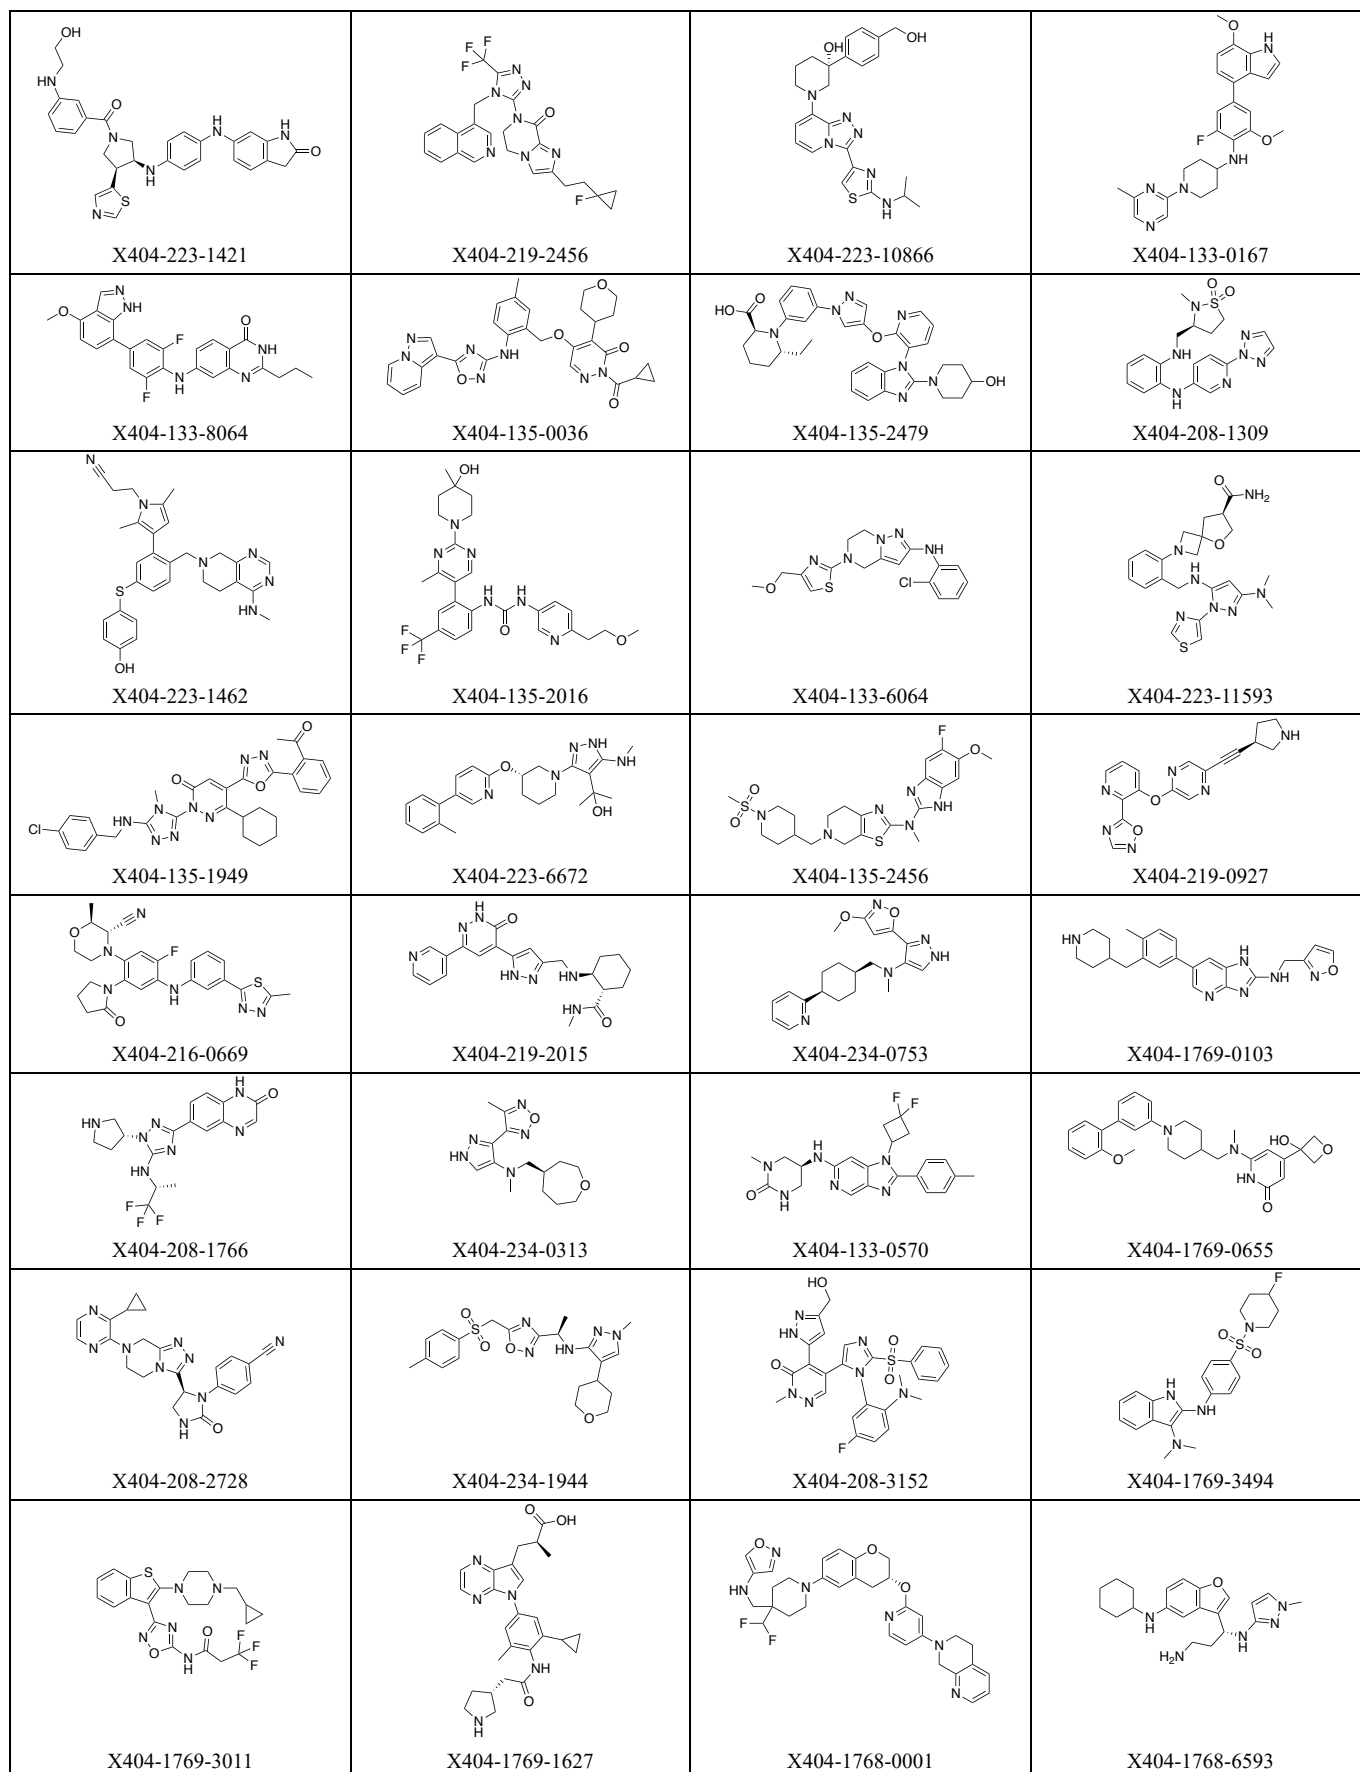   | 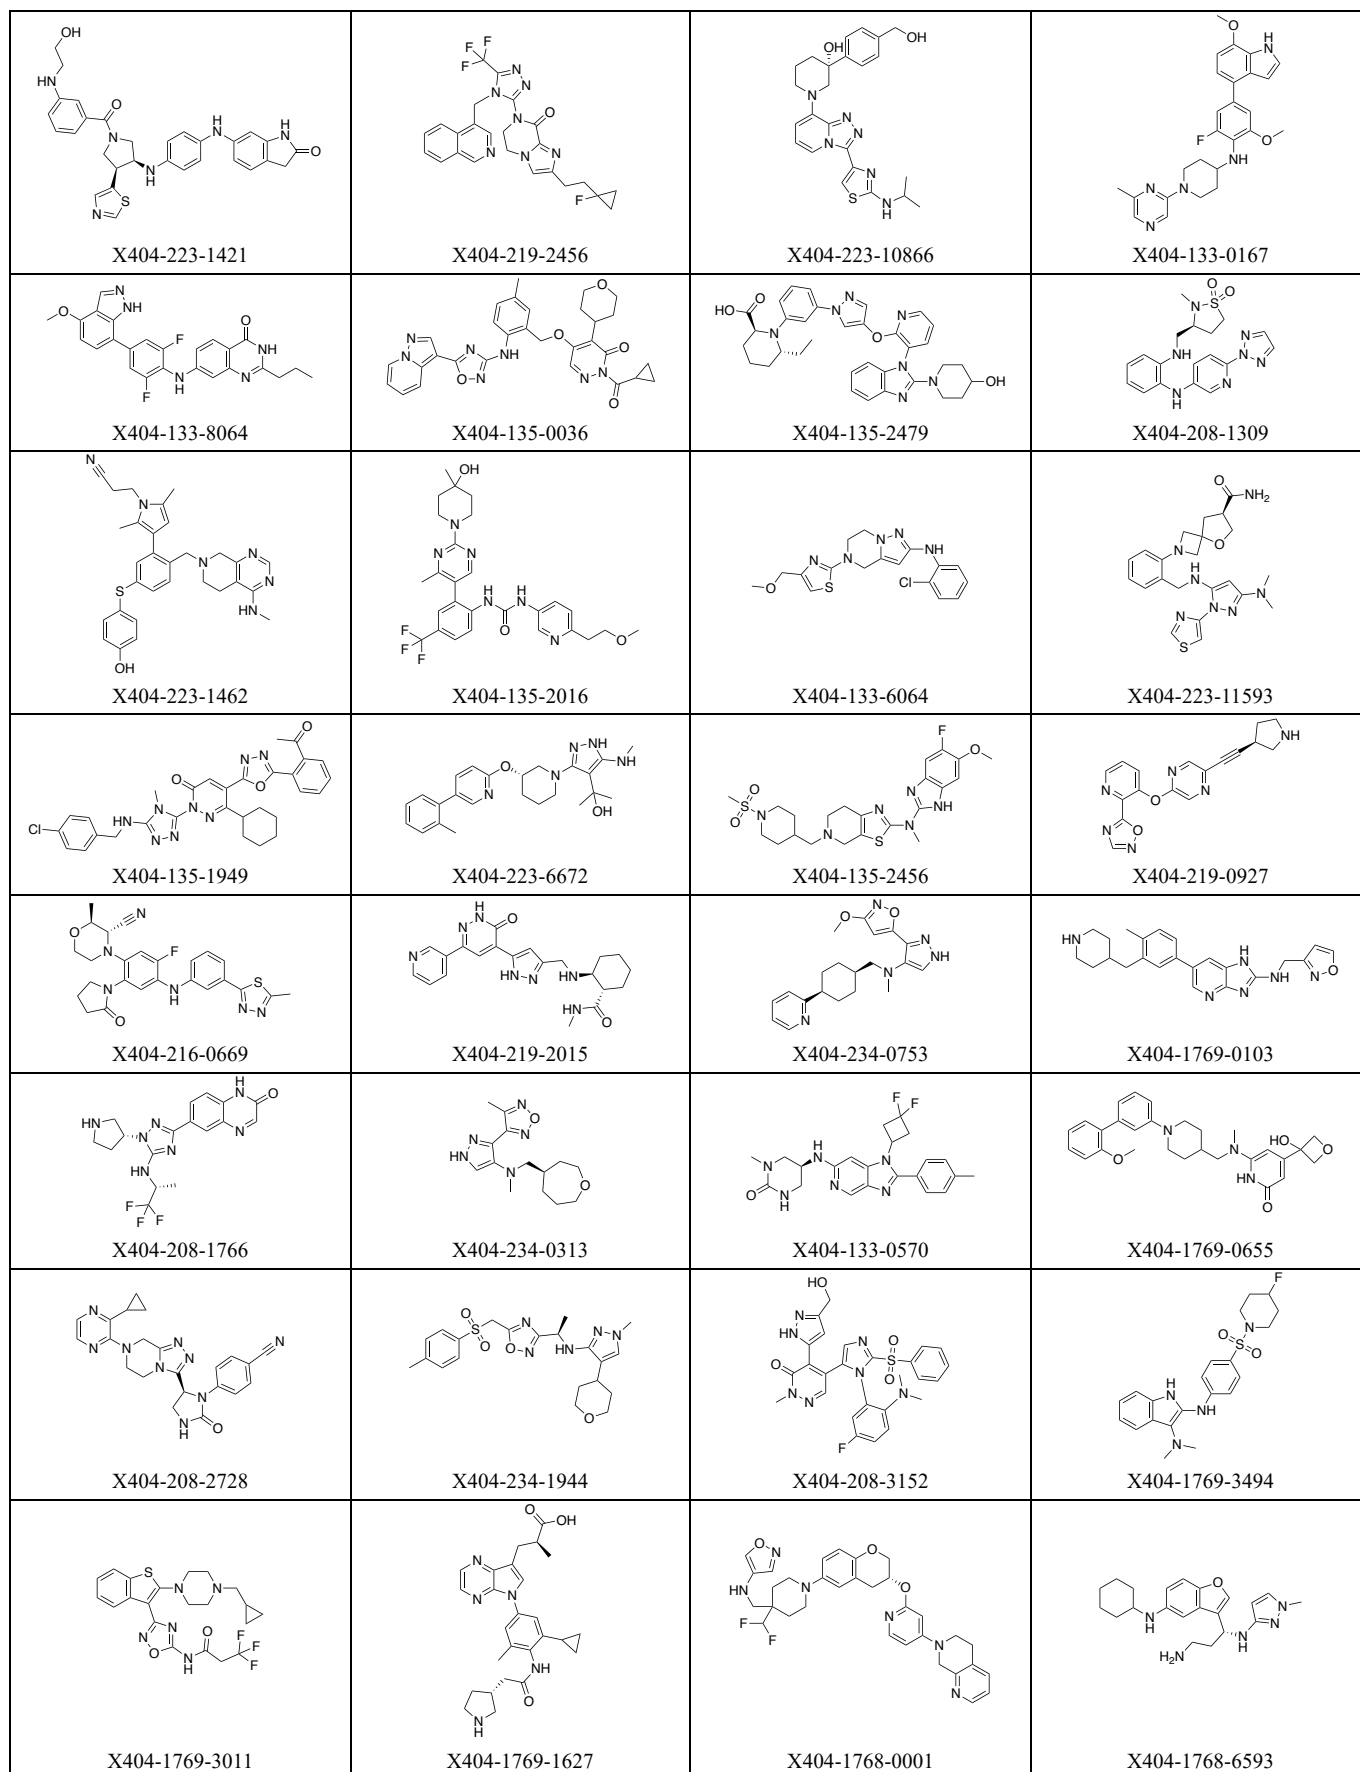   | 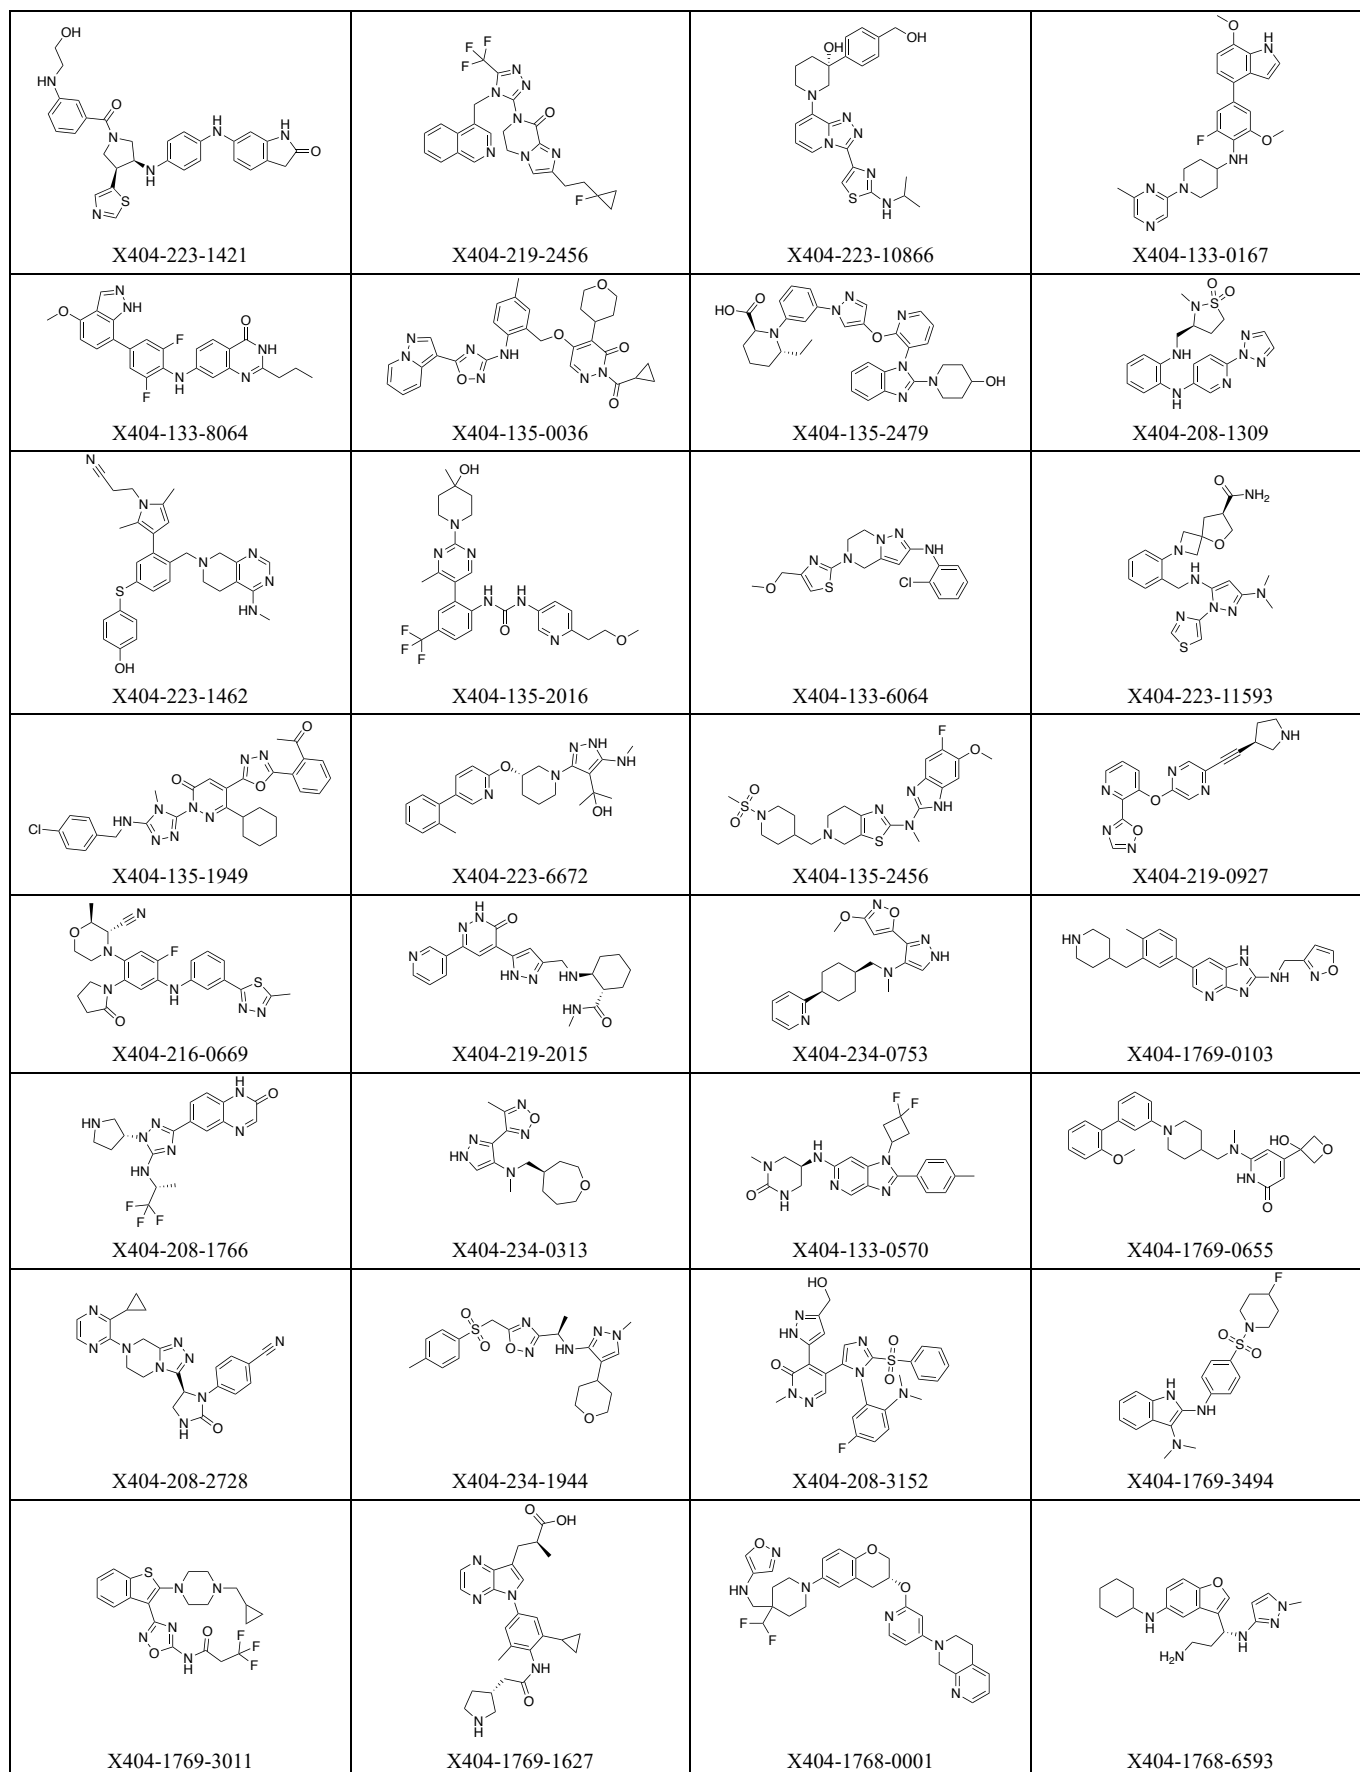   | 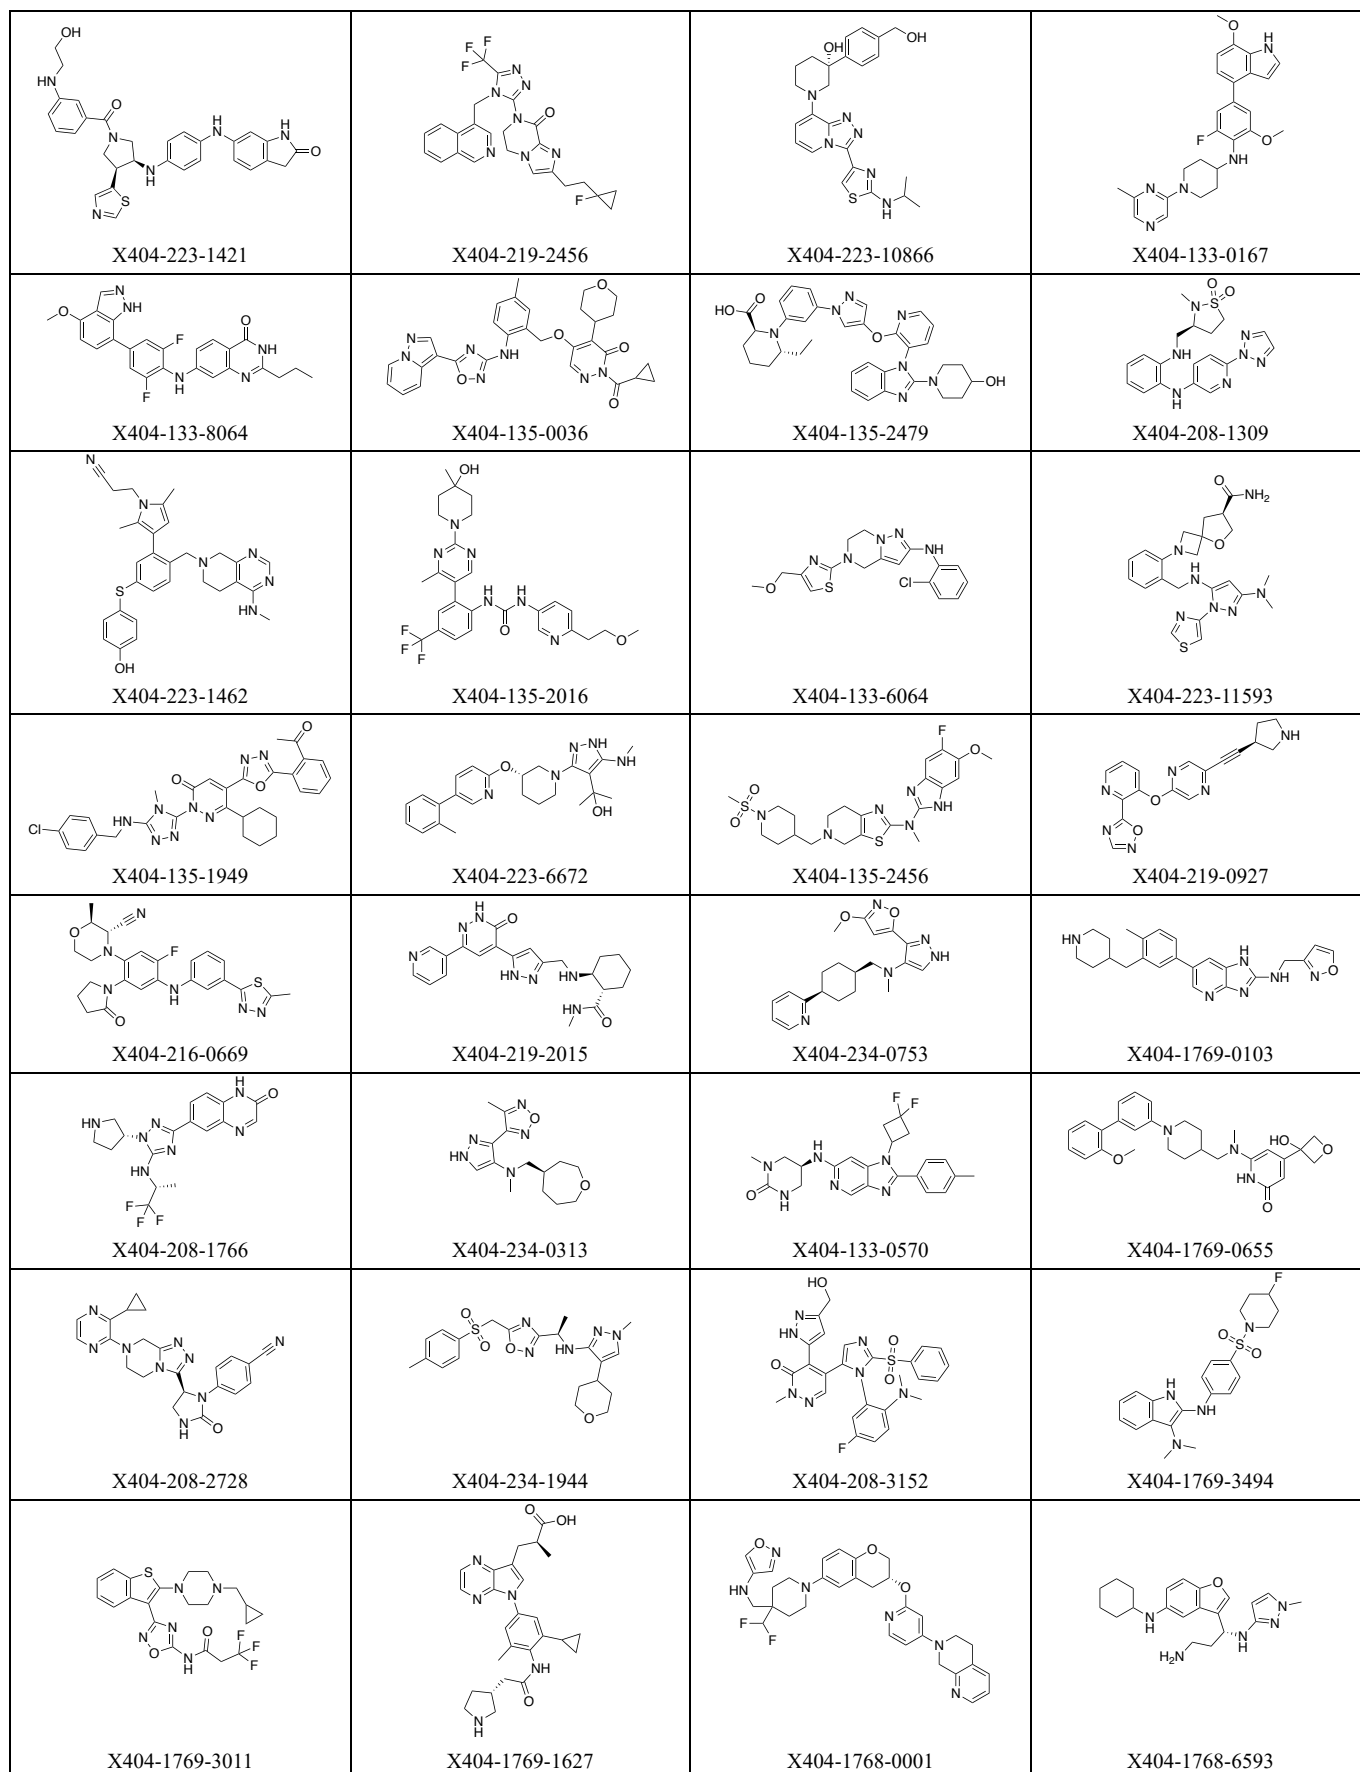   |
| X404-133-8064                                                                       | X404-135-0036                                                                       | X404-135-2479                                                                        | X404-208-1309                                                                         |
| 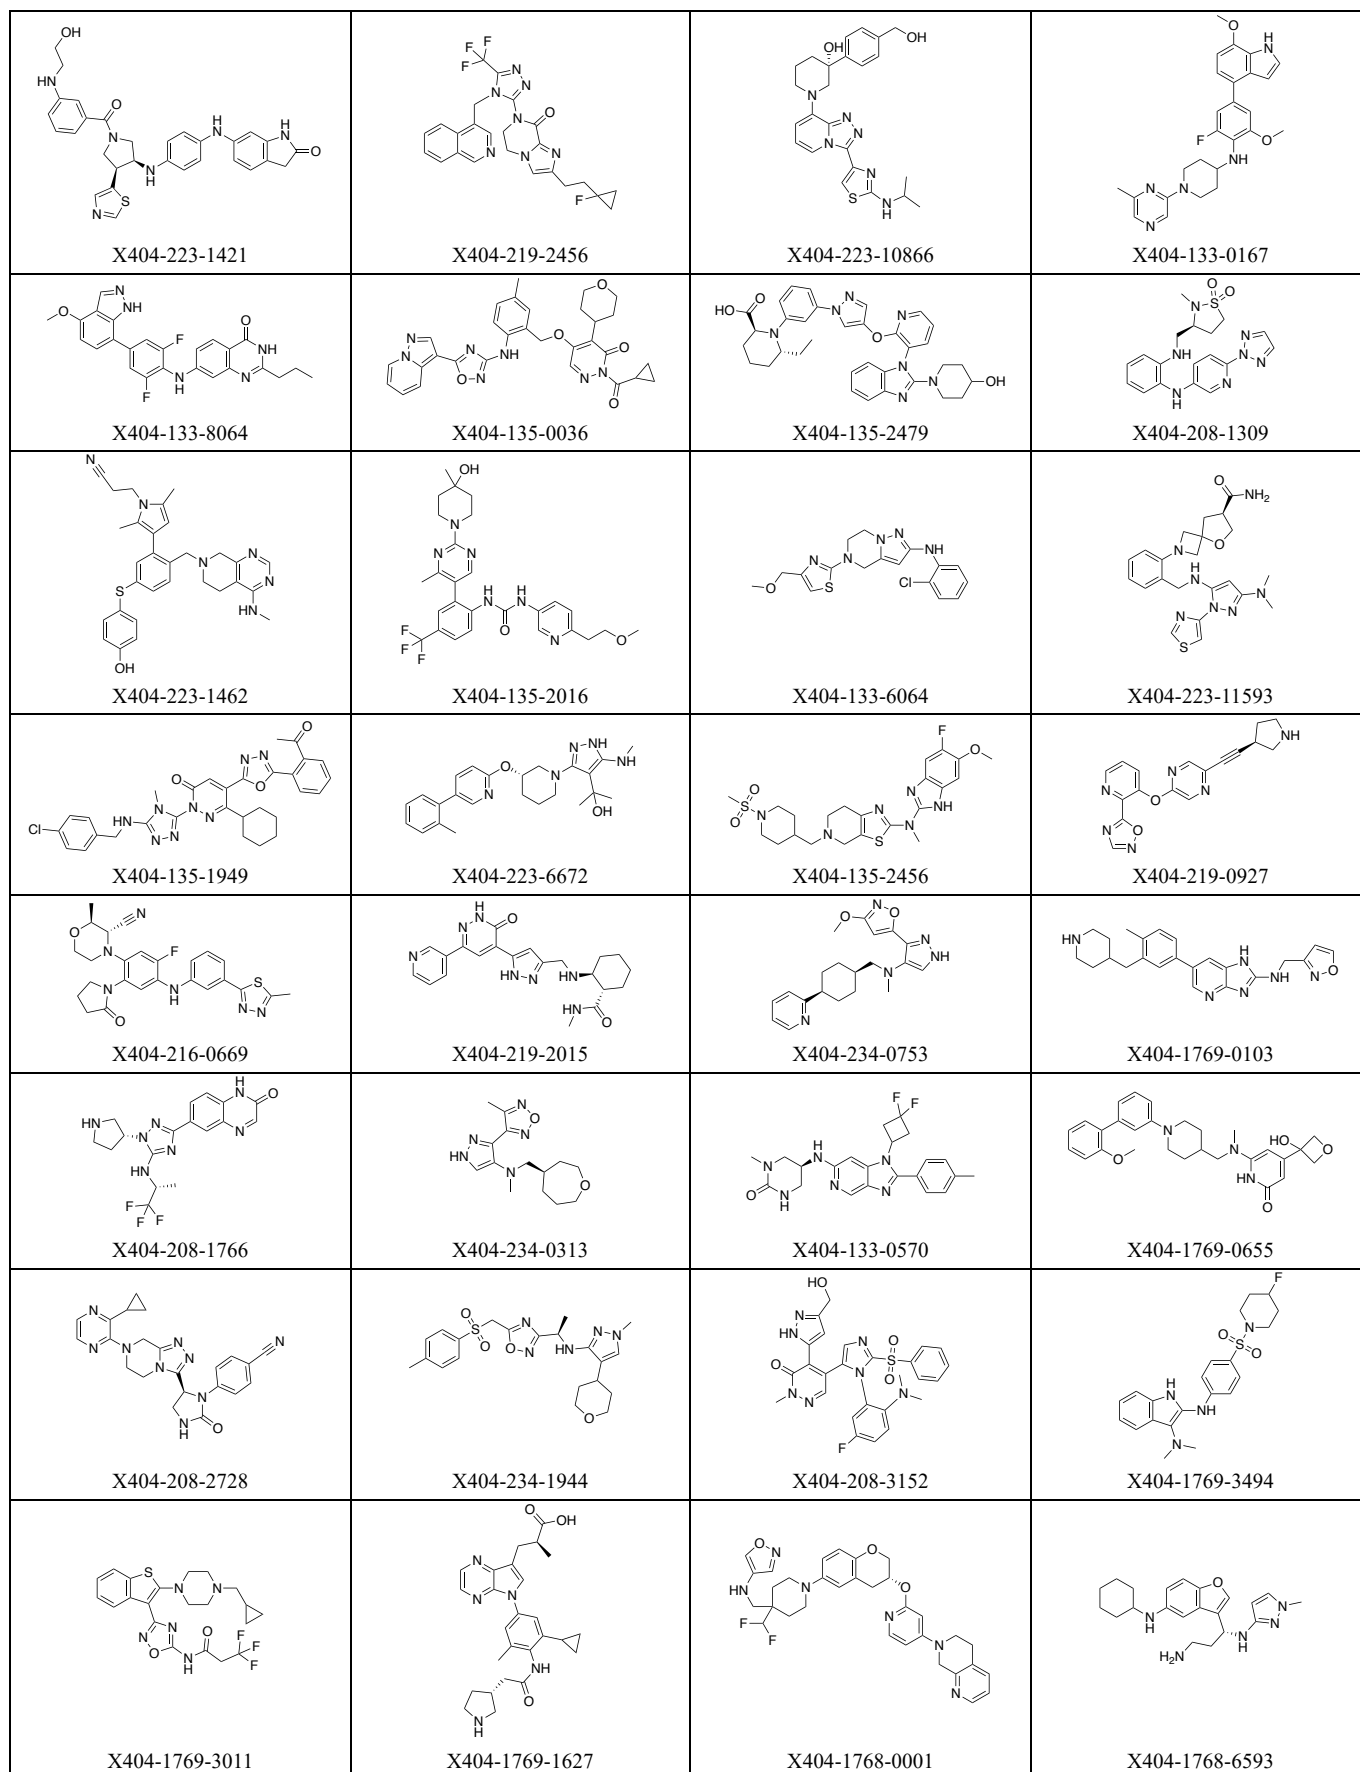   | 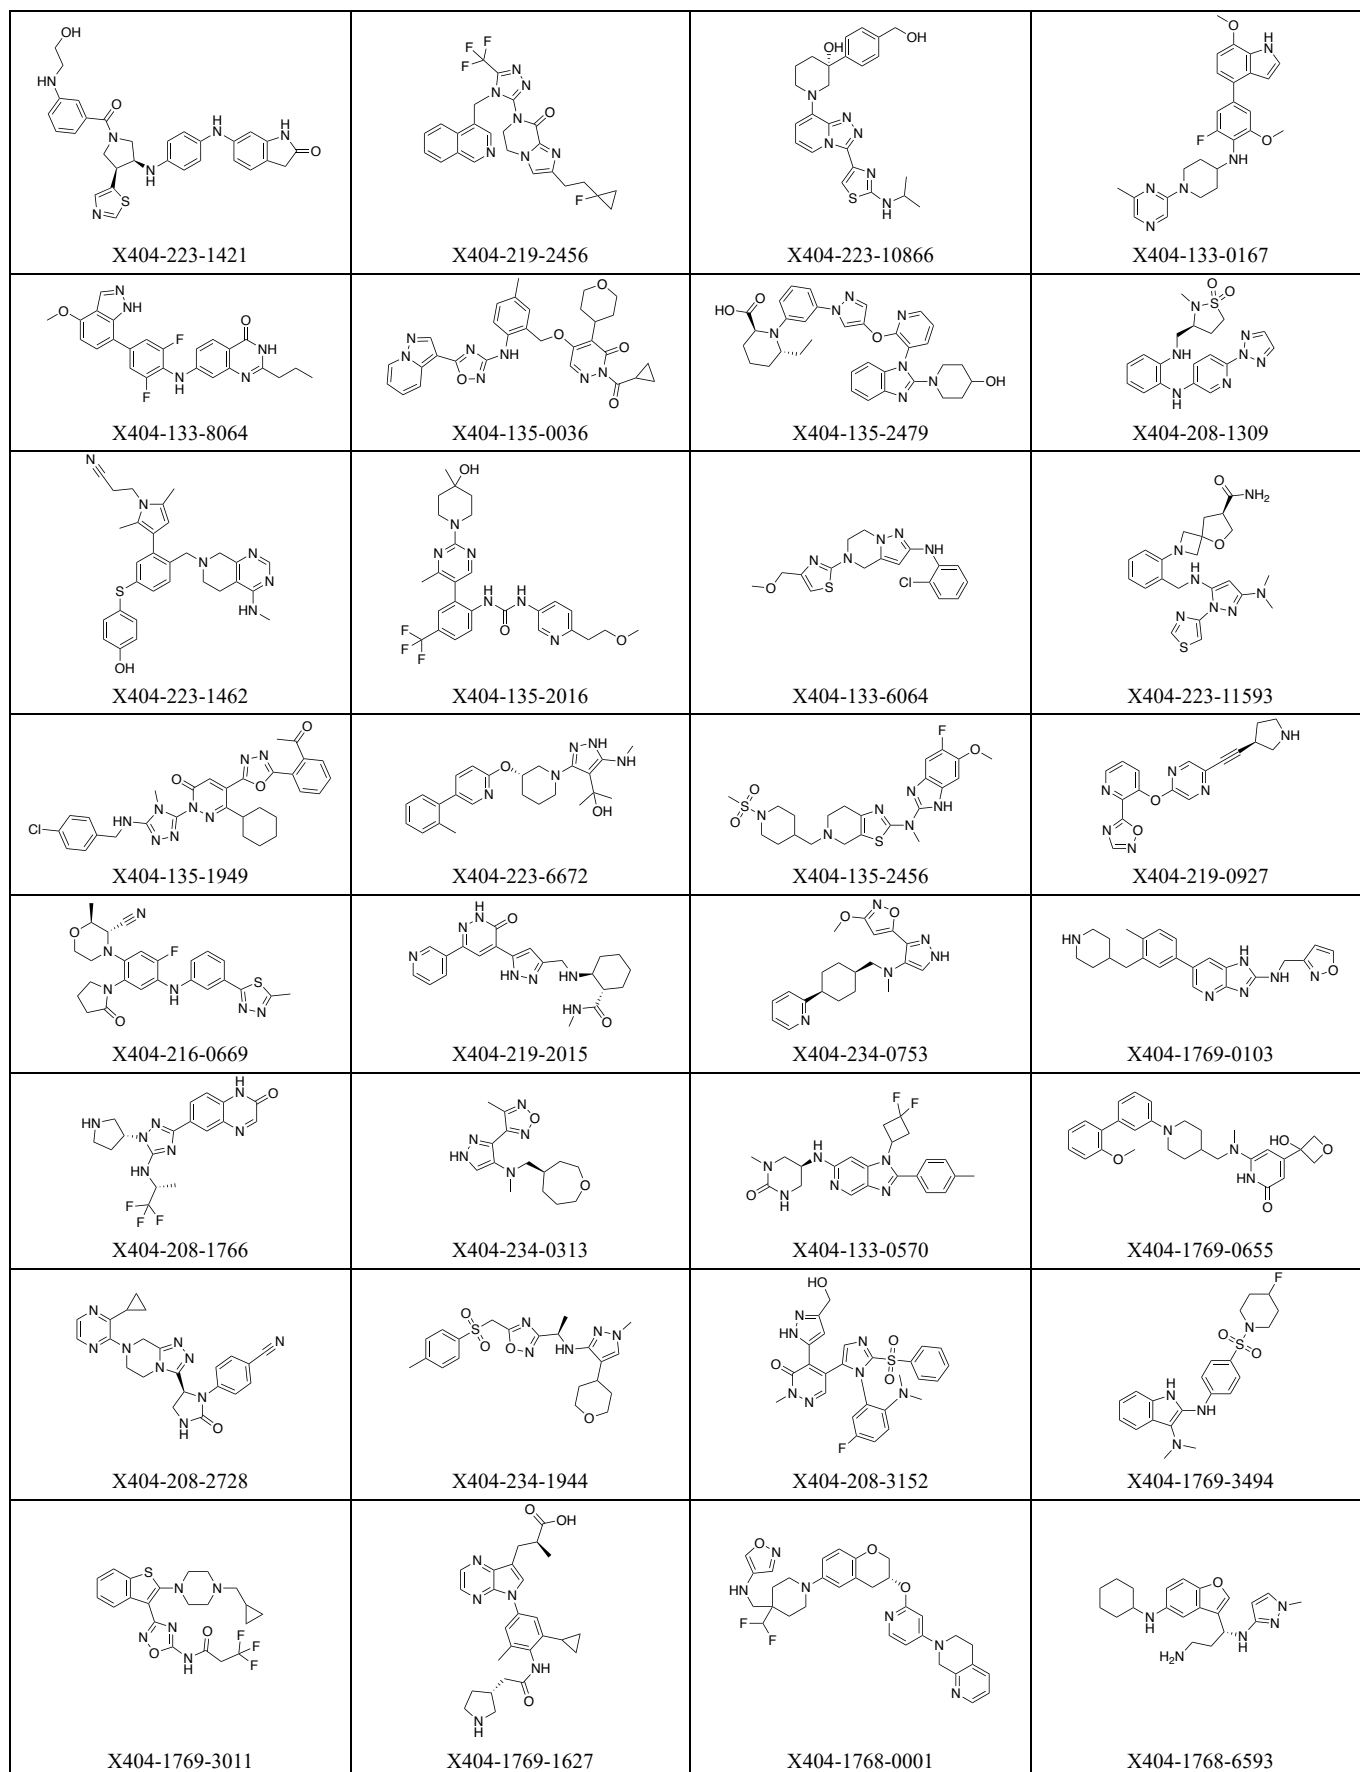   | 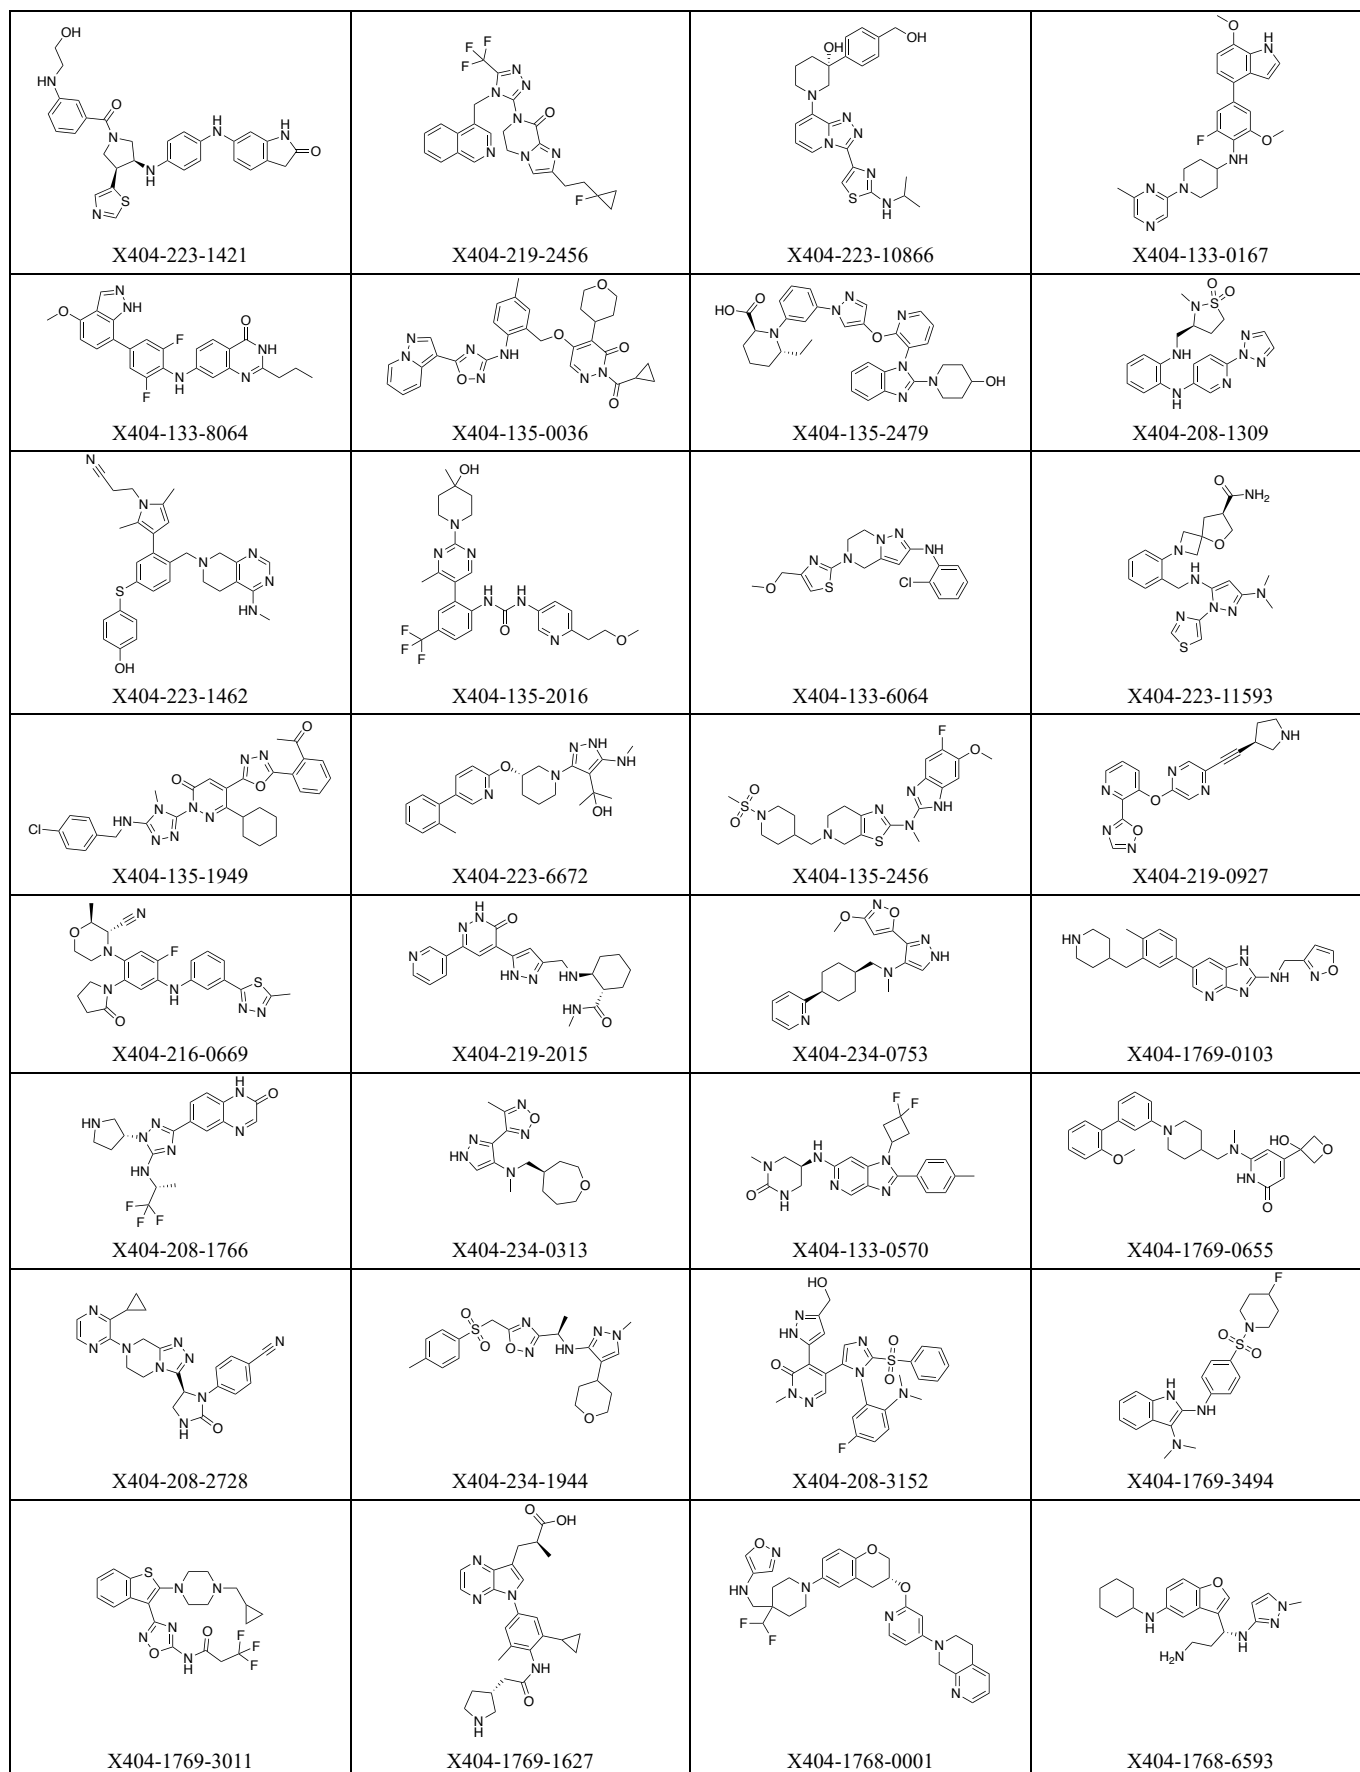   | 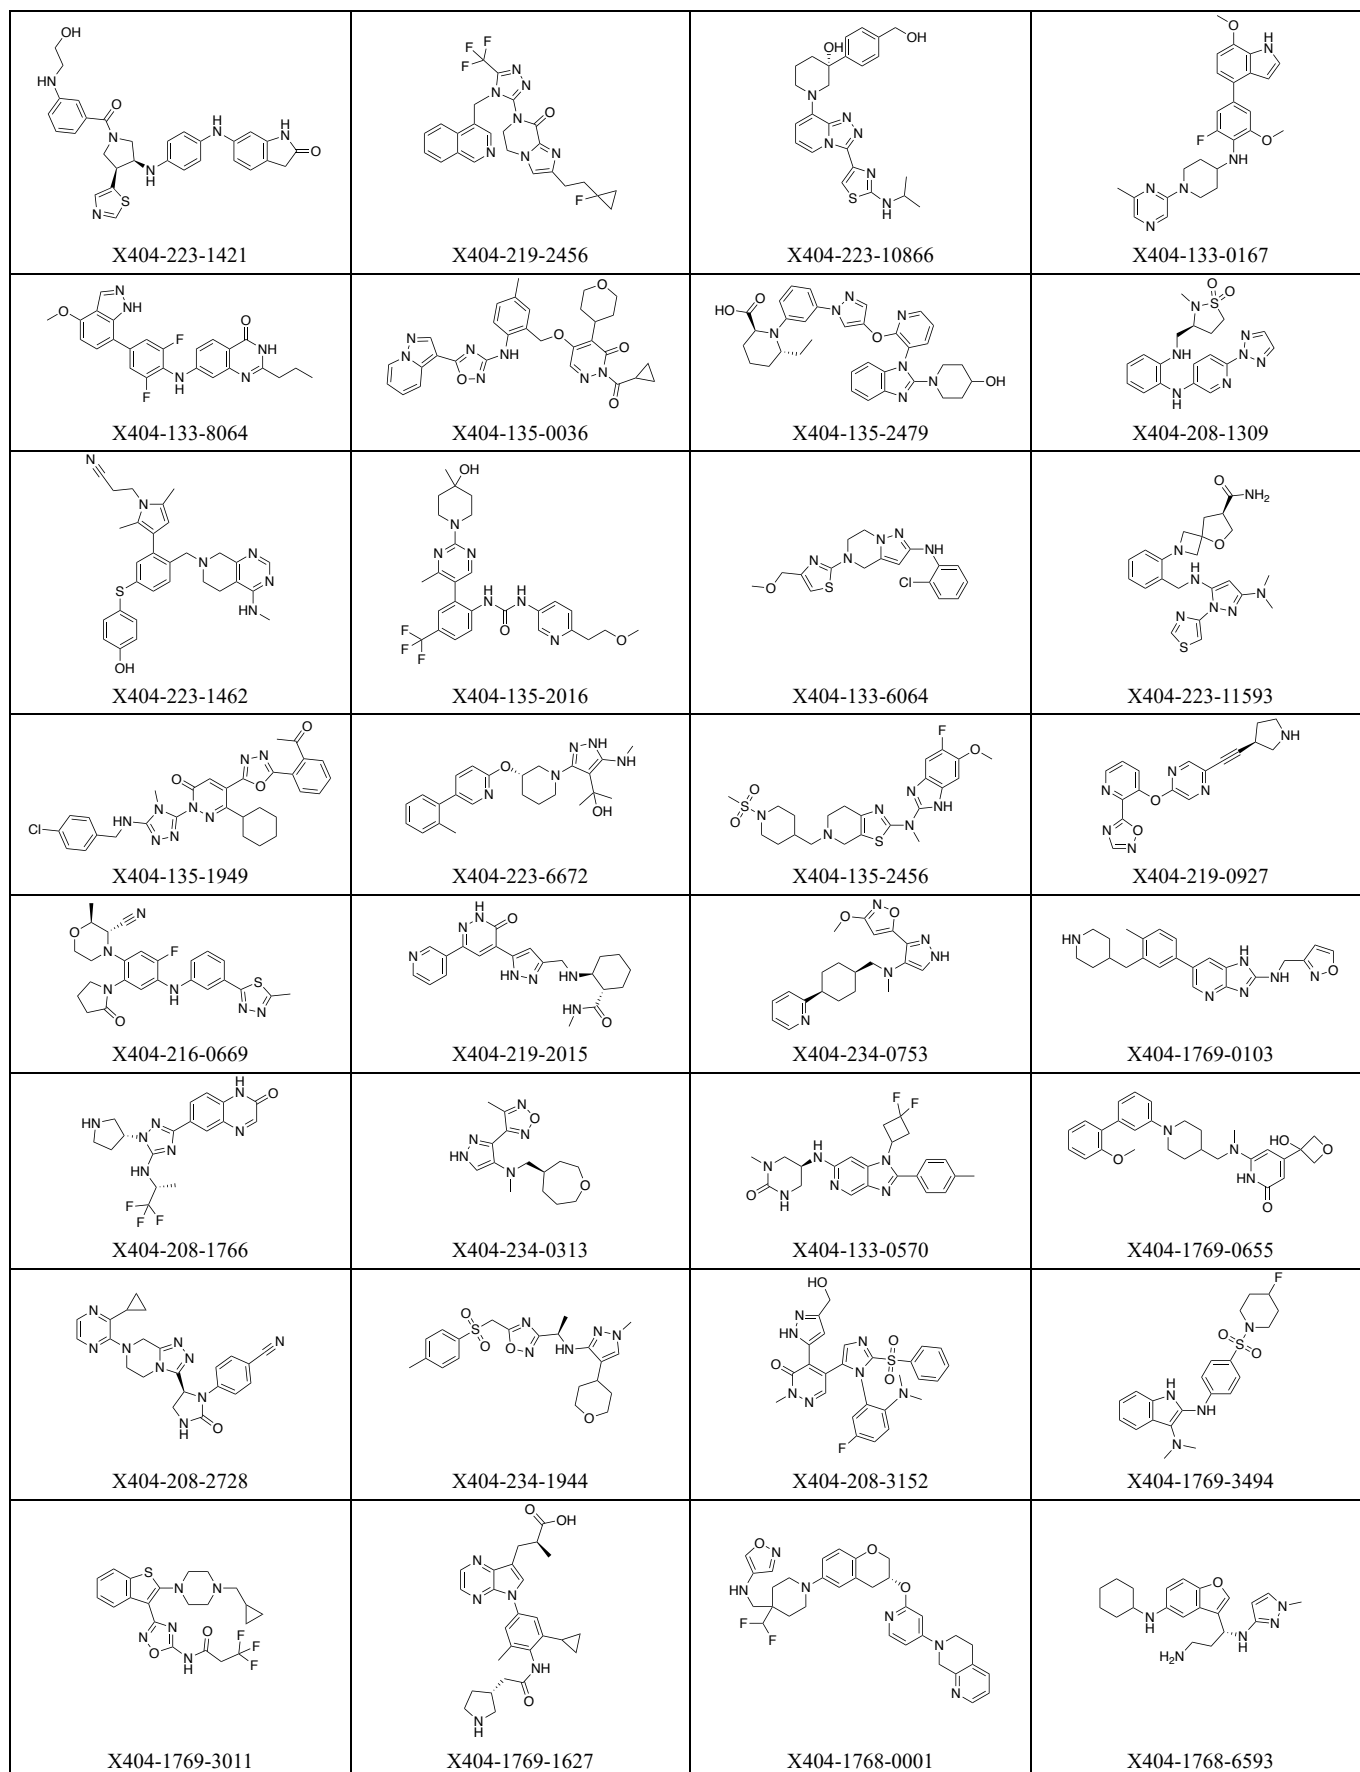   |
| X404-223-1462                                                                       | X404-135-2016                                                                       | X404-133-6064                                                                        | X404-223-11593                                                                        |
| 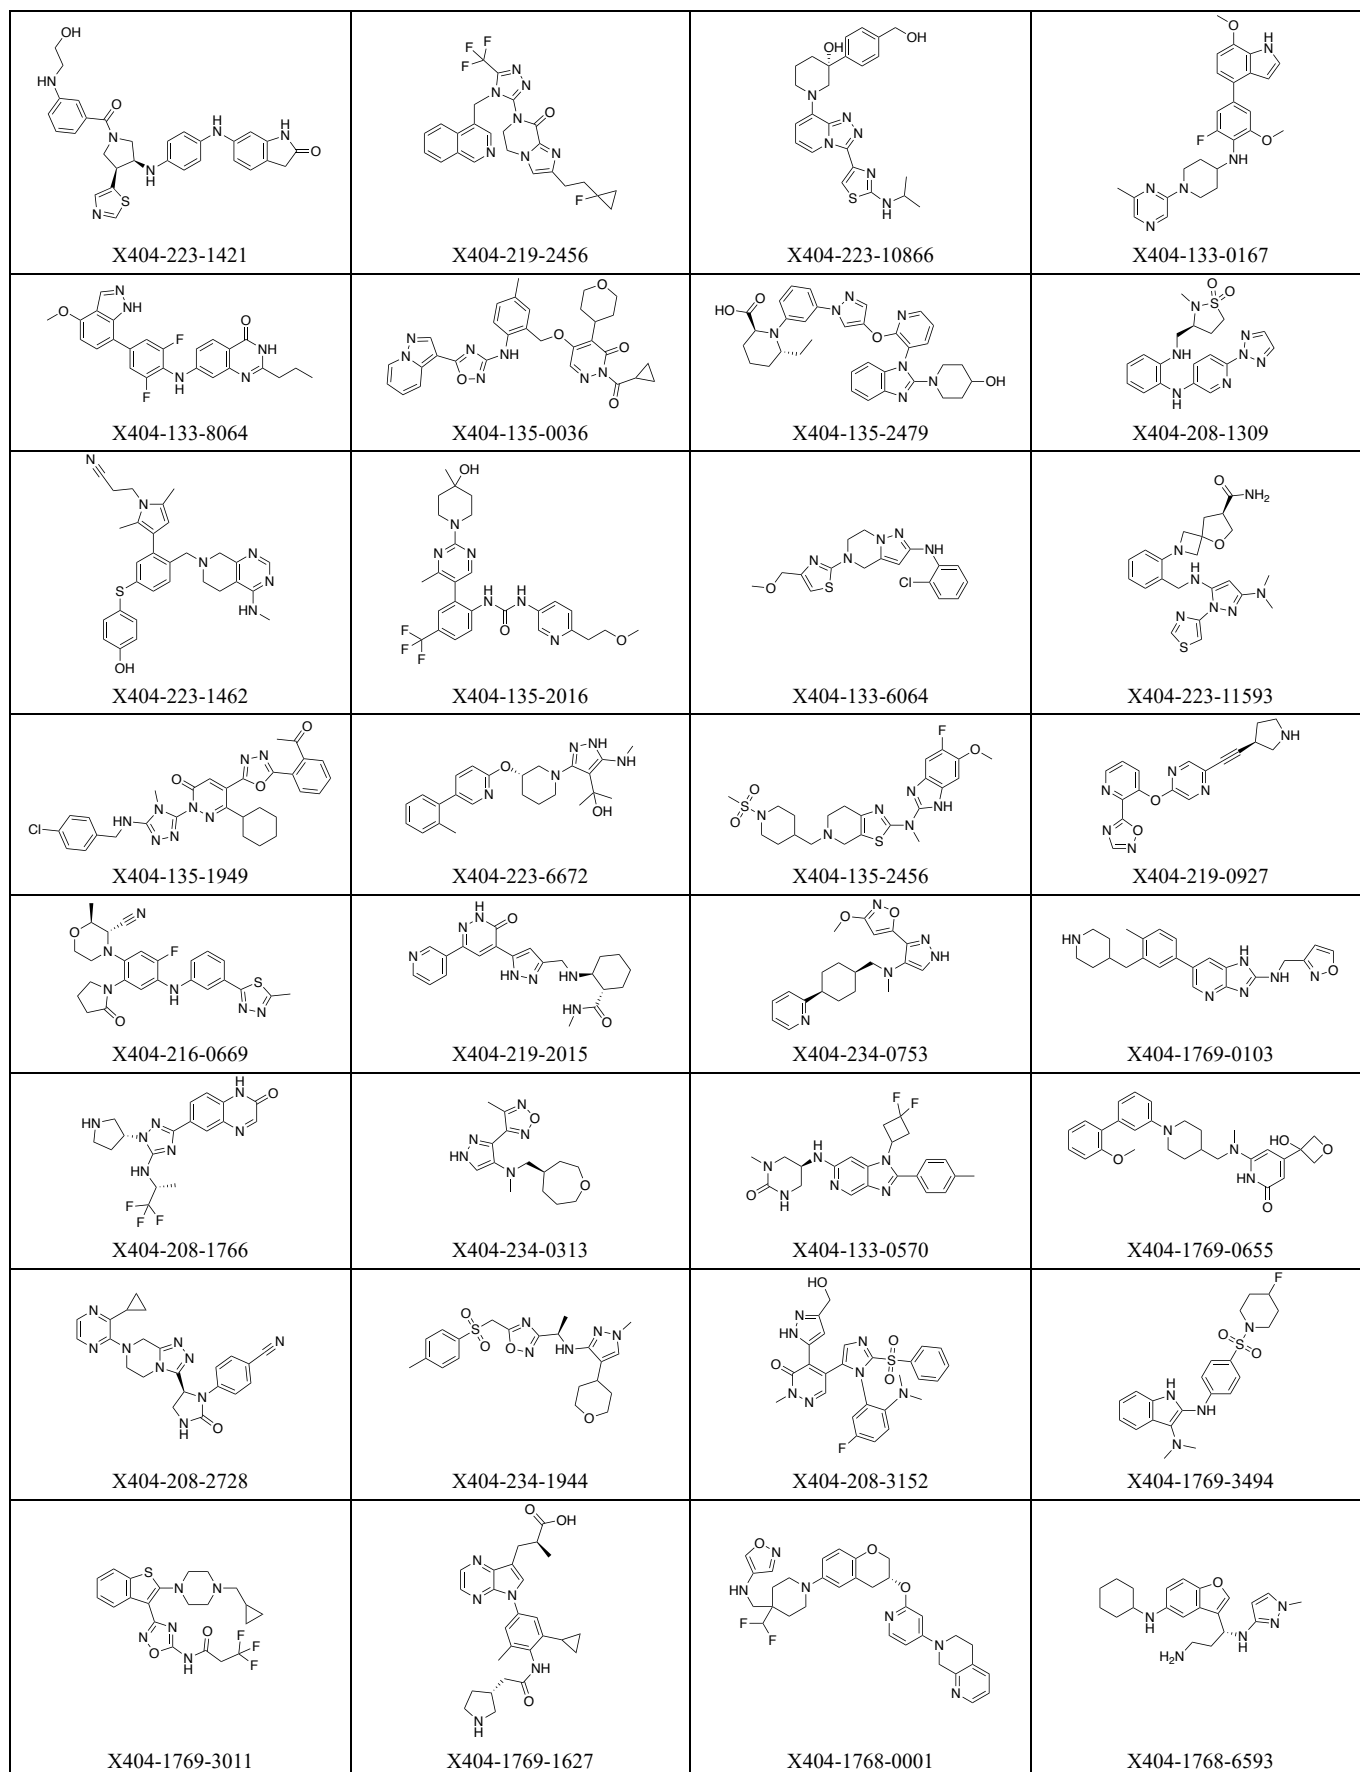   | 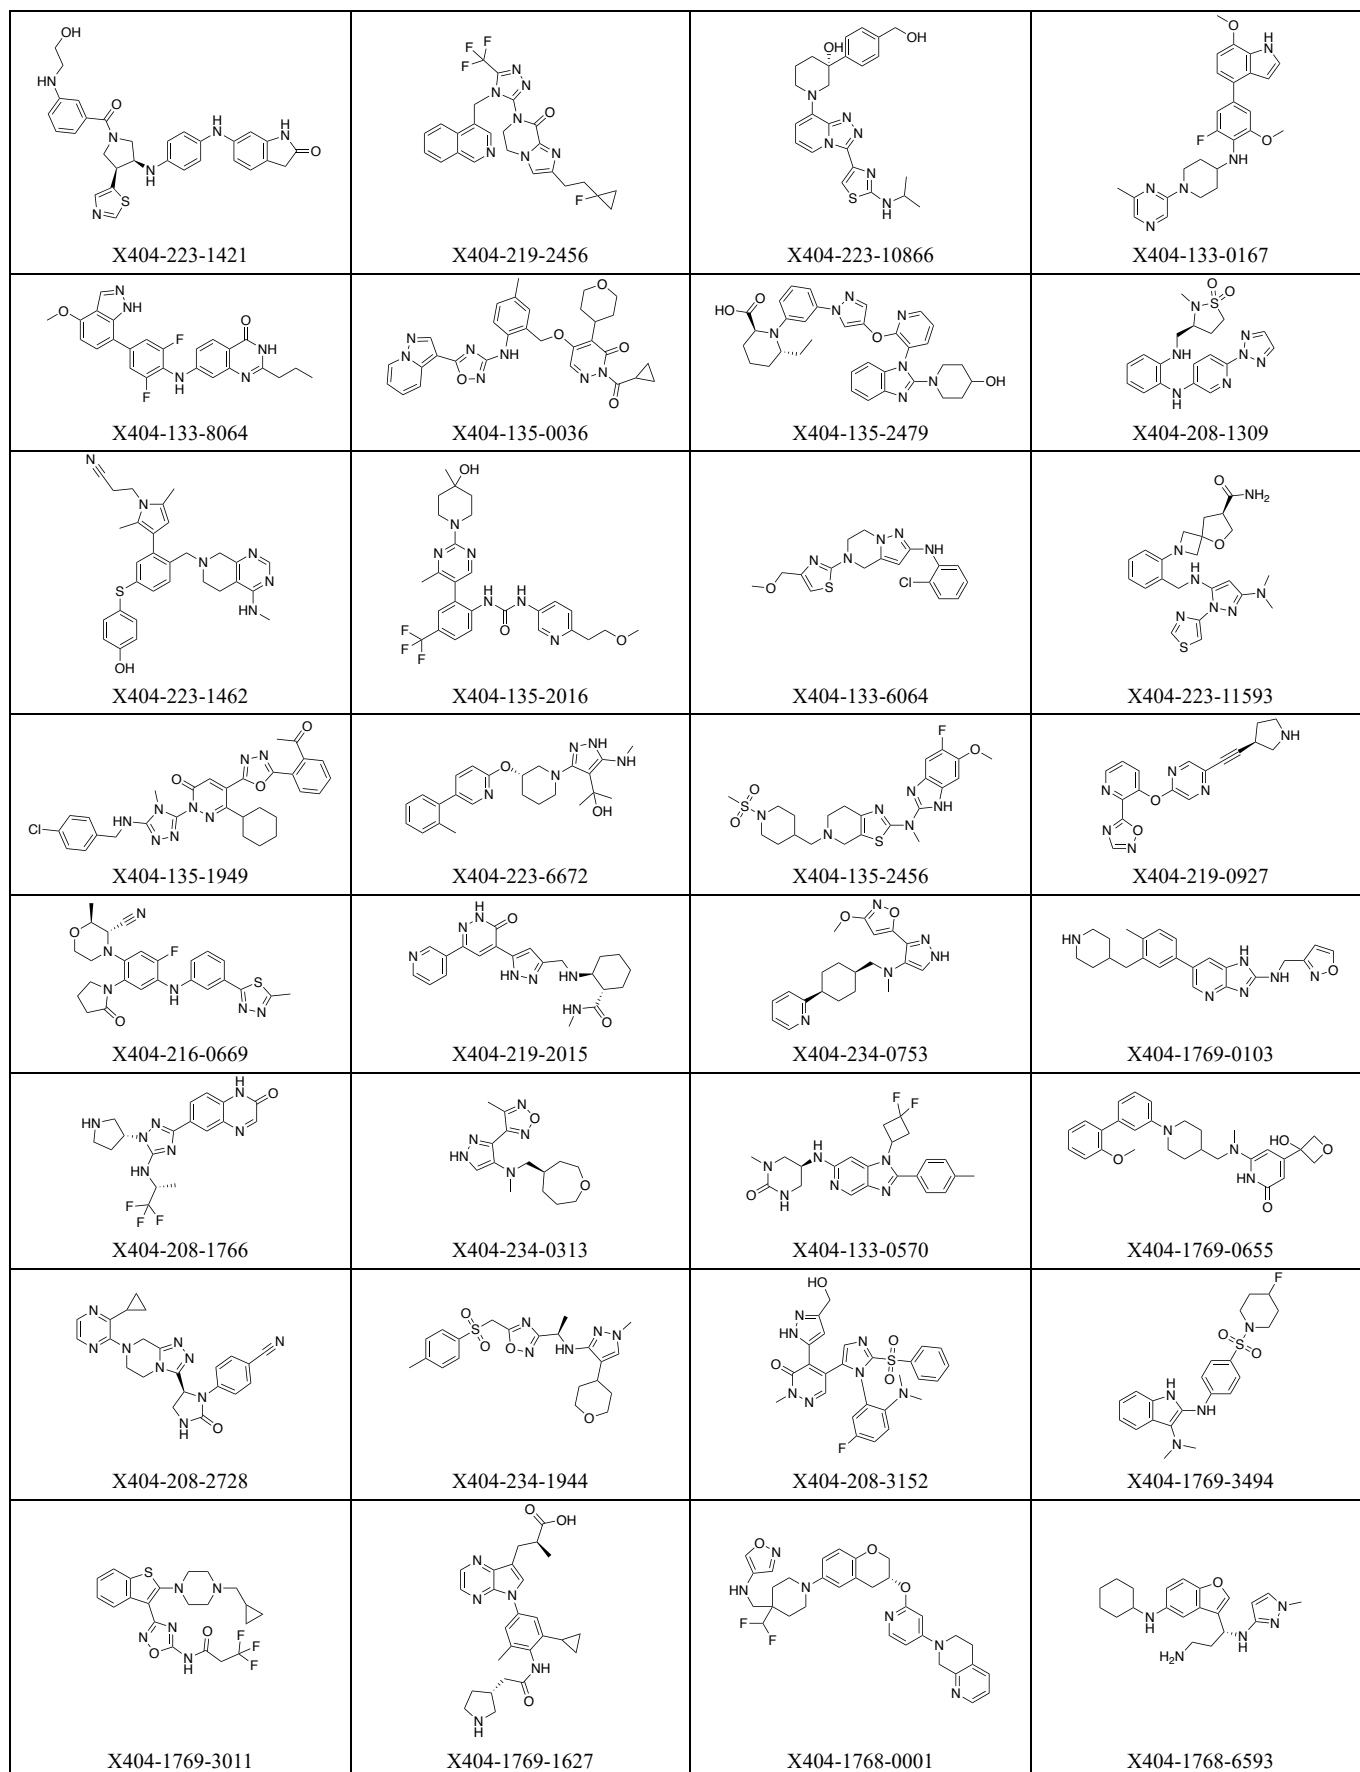   | 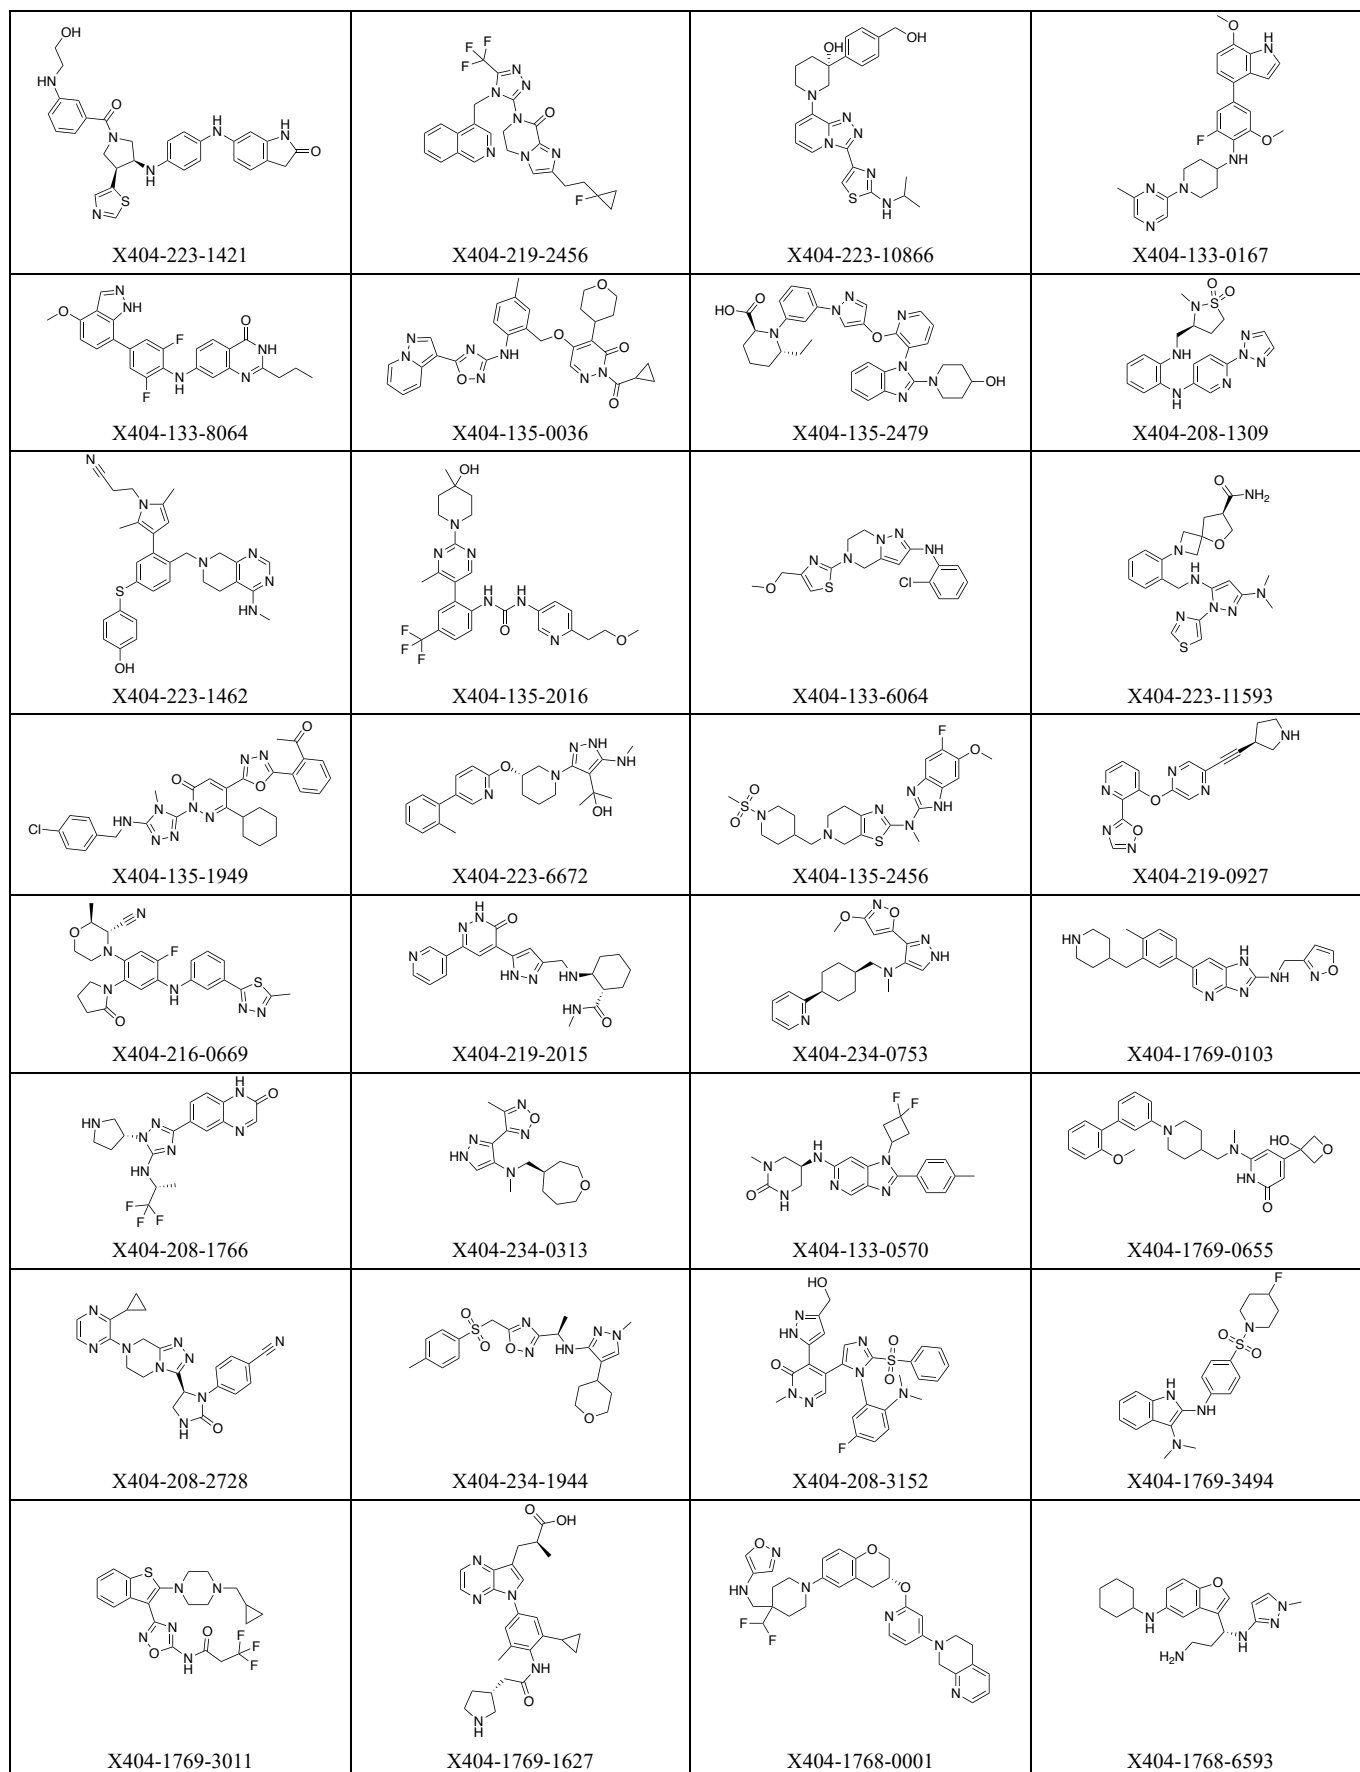   | 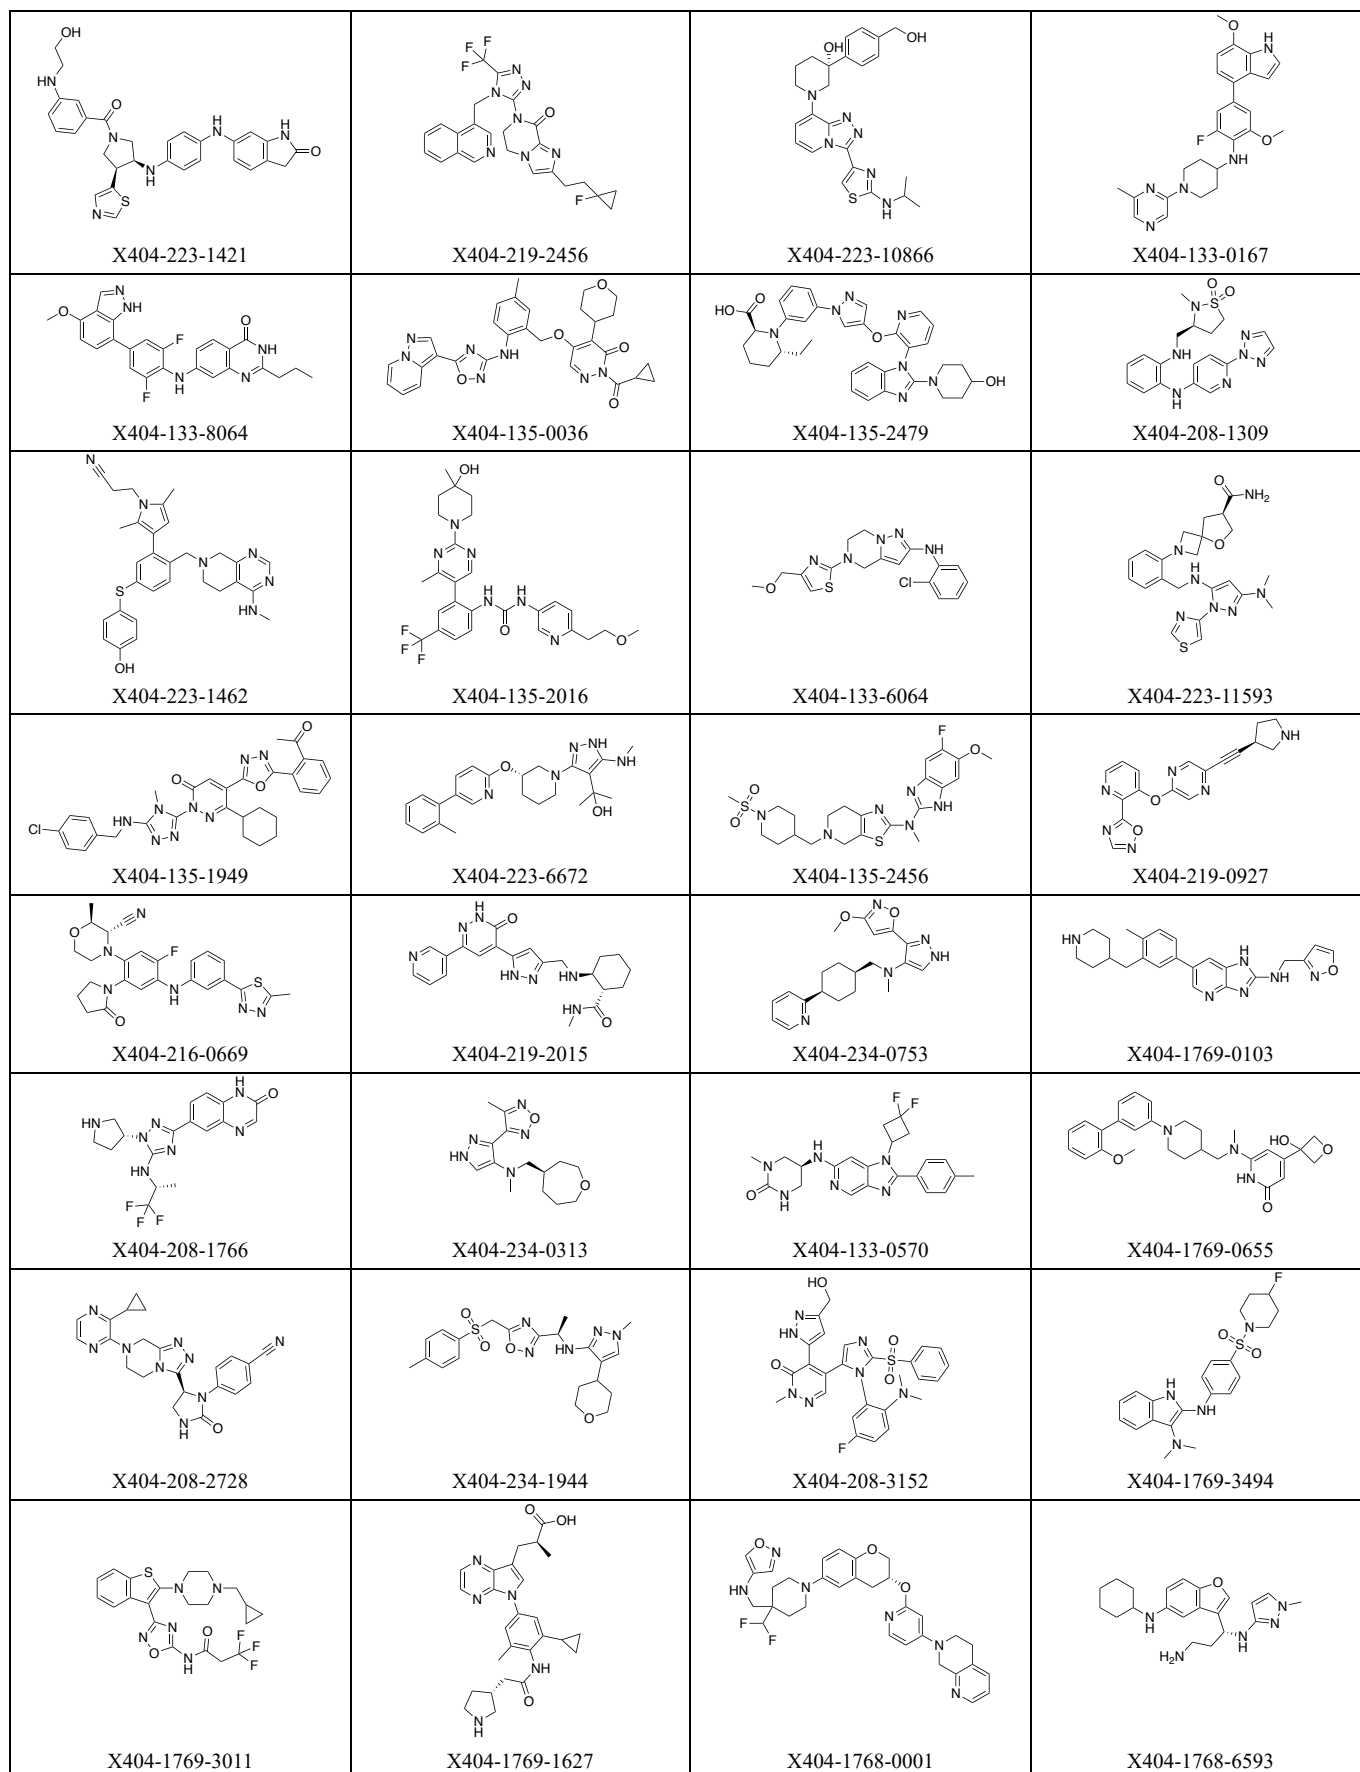   |
| X404-135-1949                                                                       | X404-223-6672                                                                       | X404-135-2456                                                                        | X404-219-0927                                                                         |
| 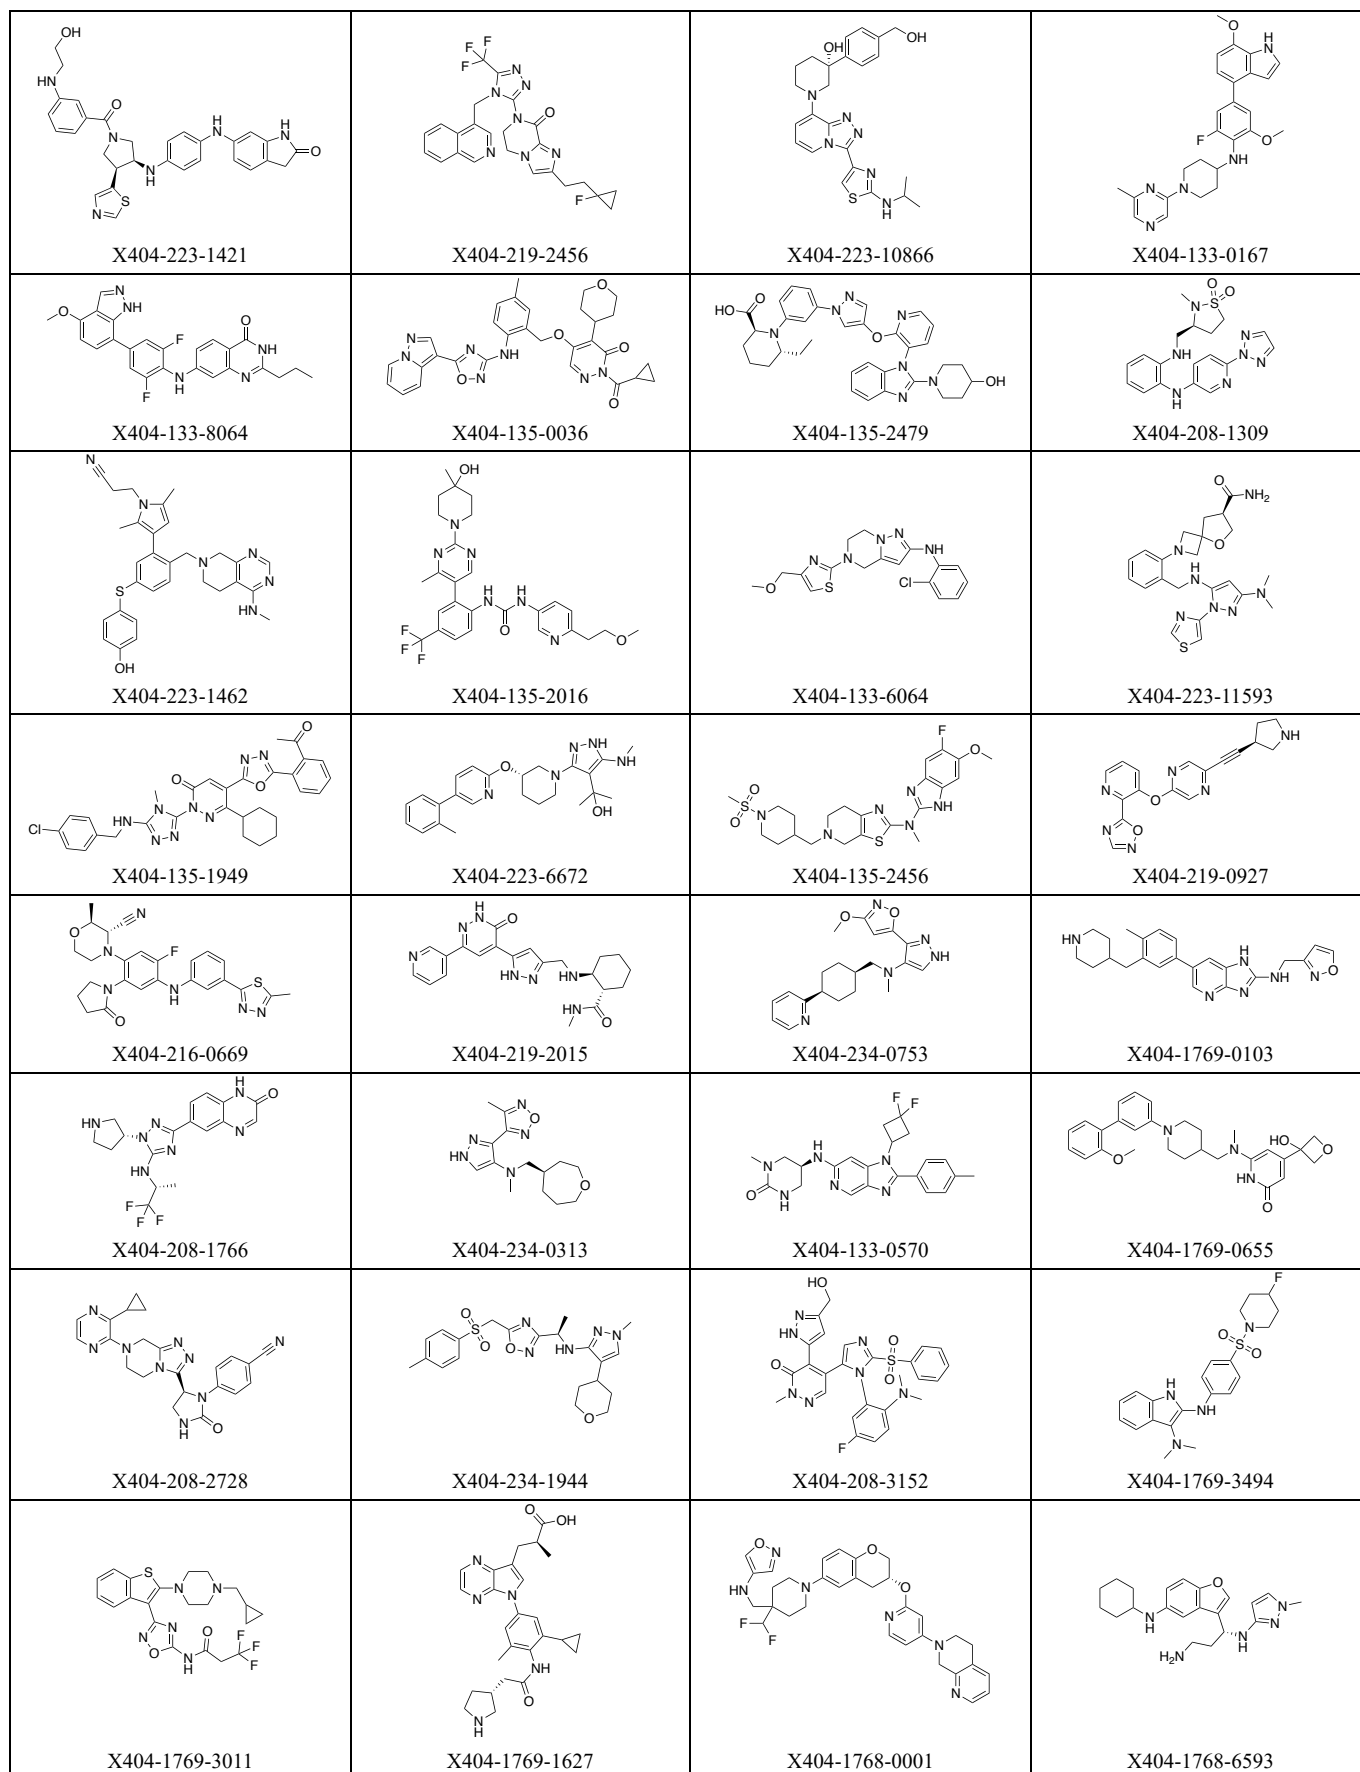 | 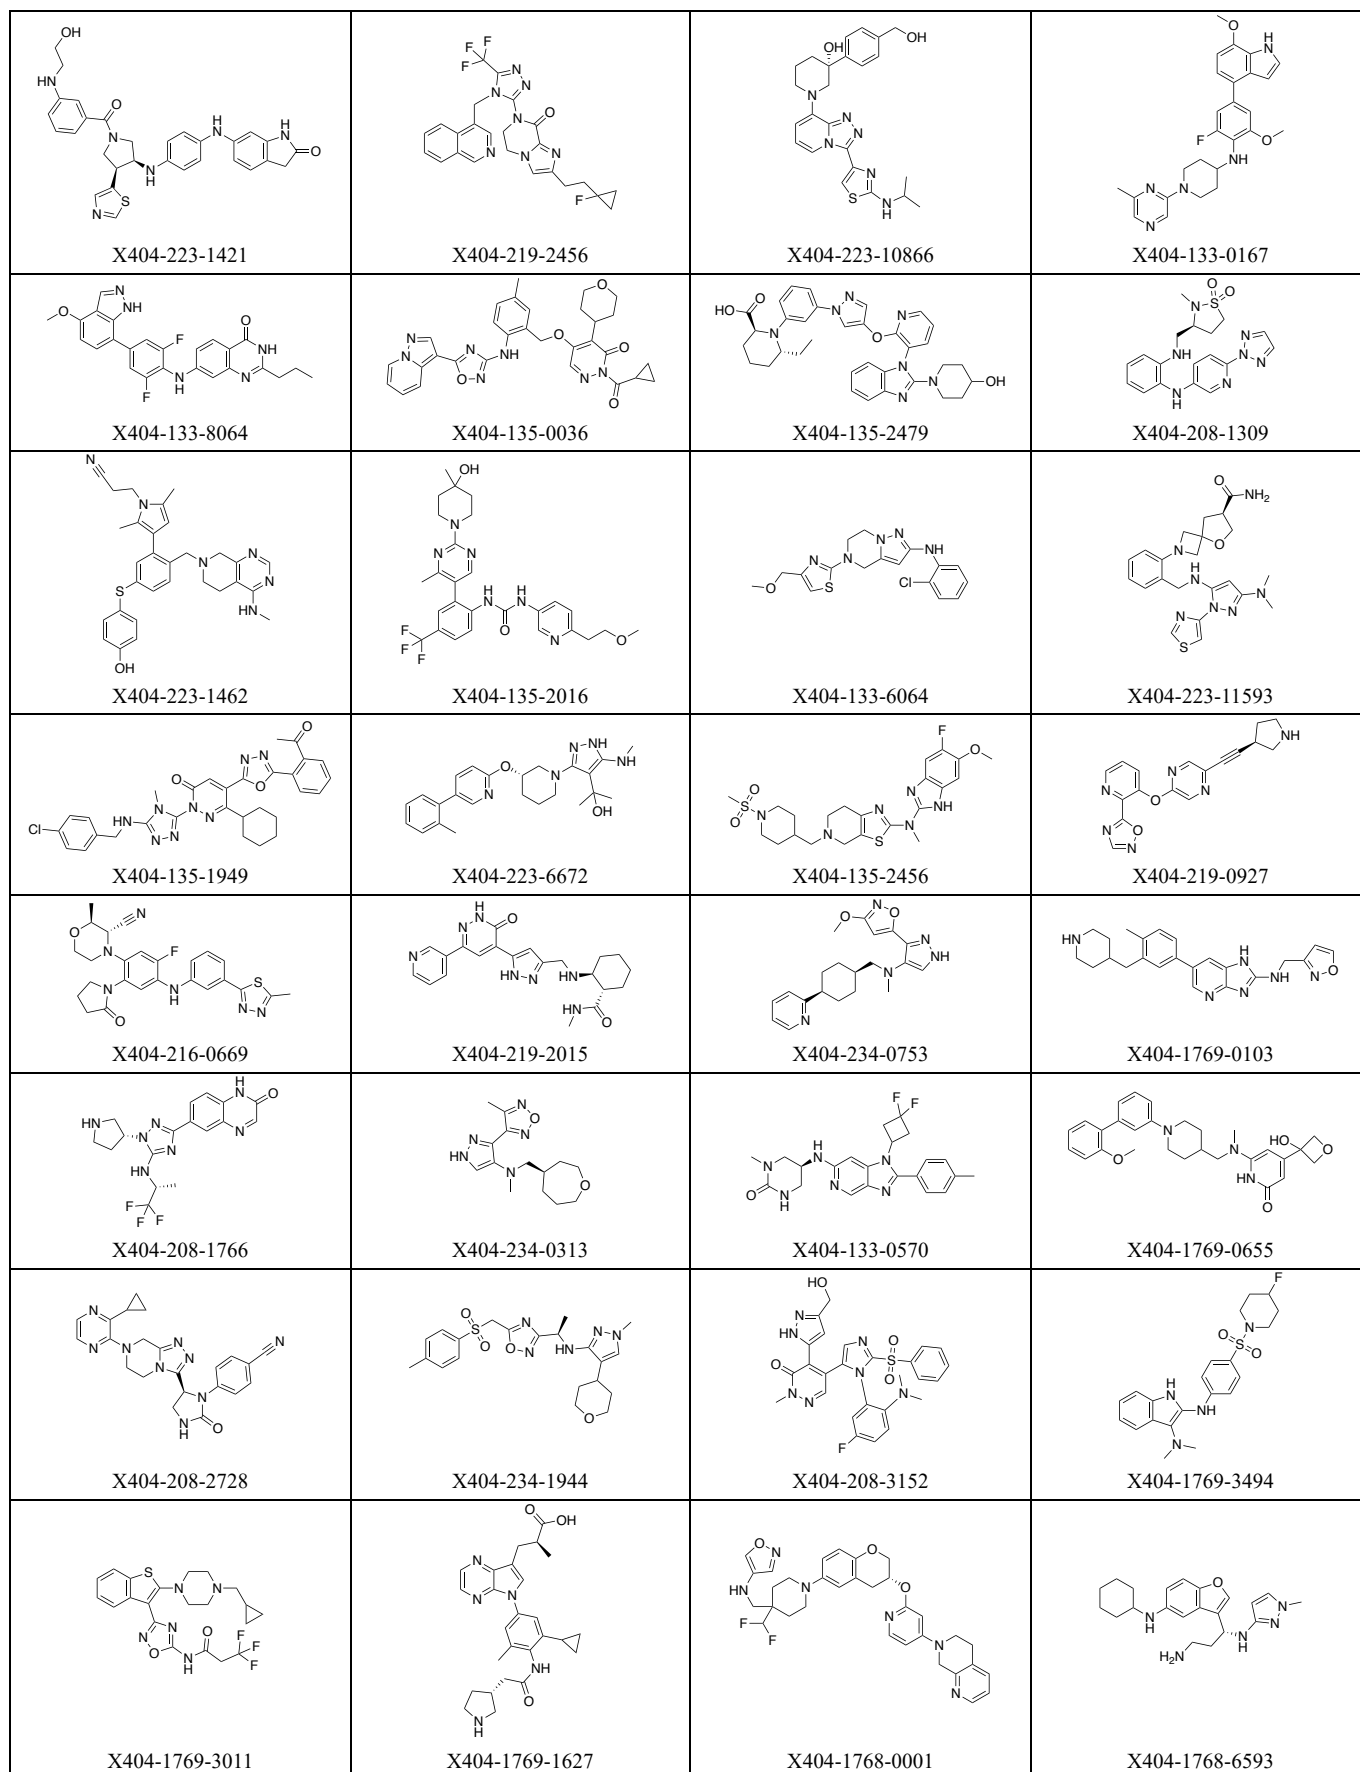 | 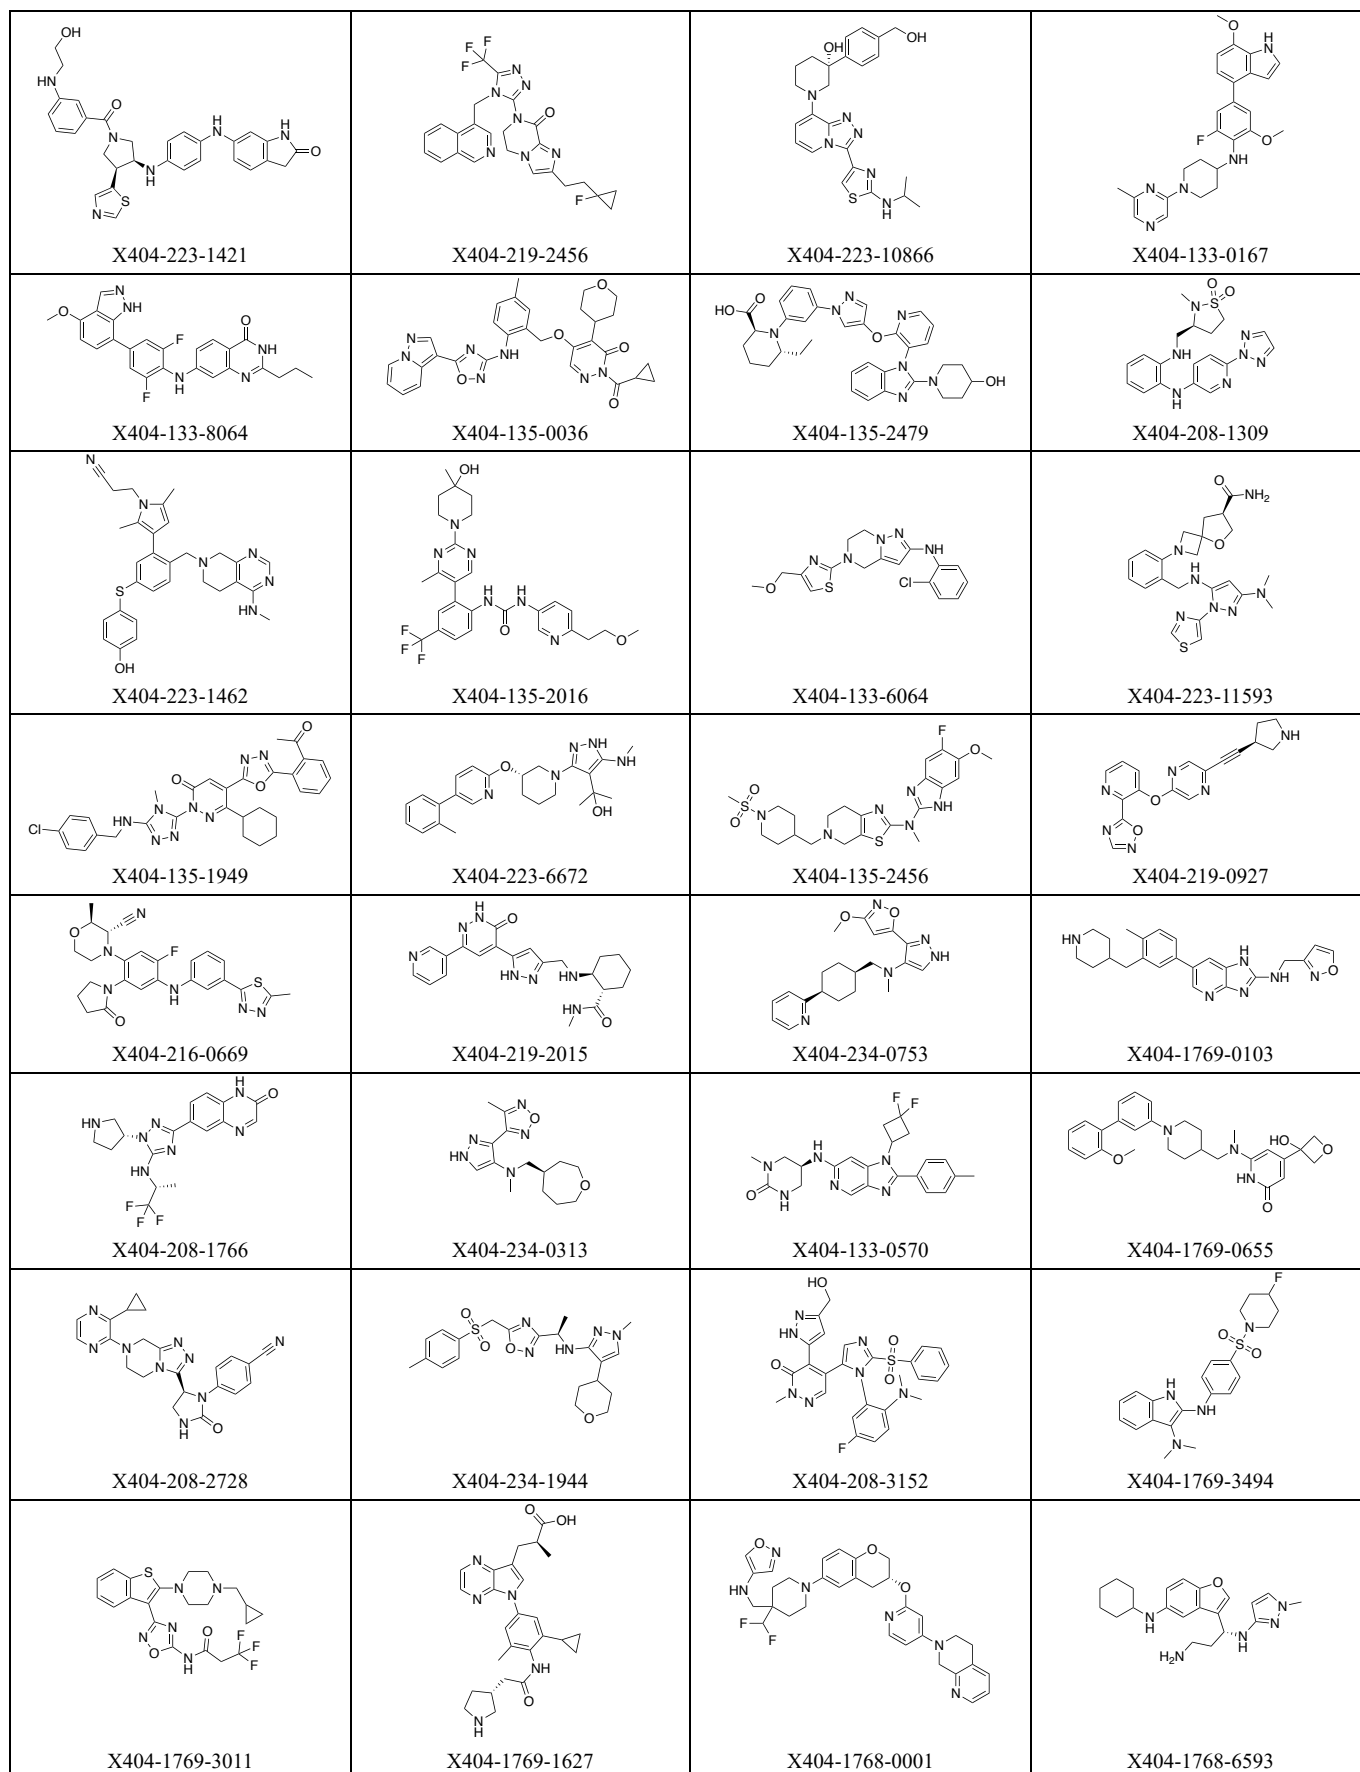 | 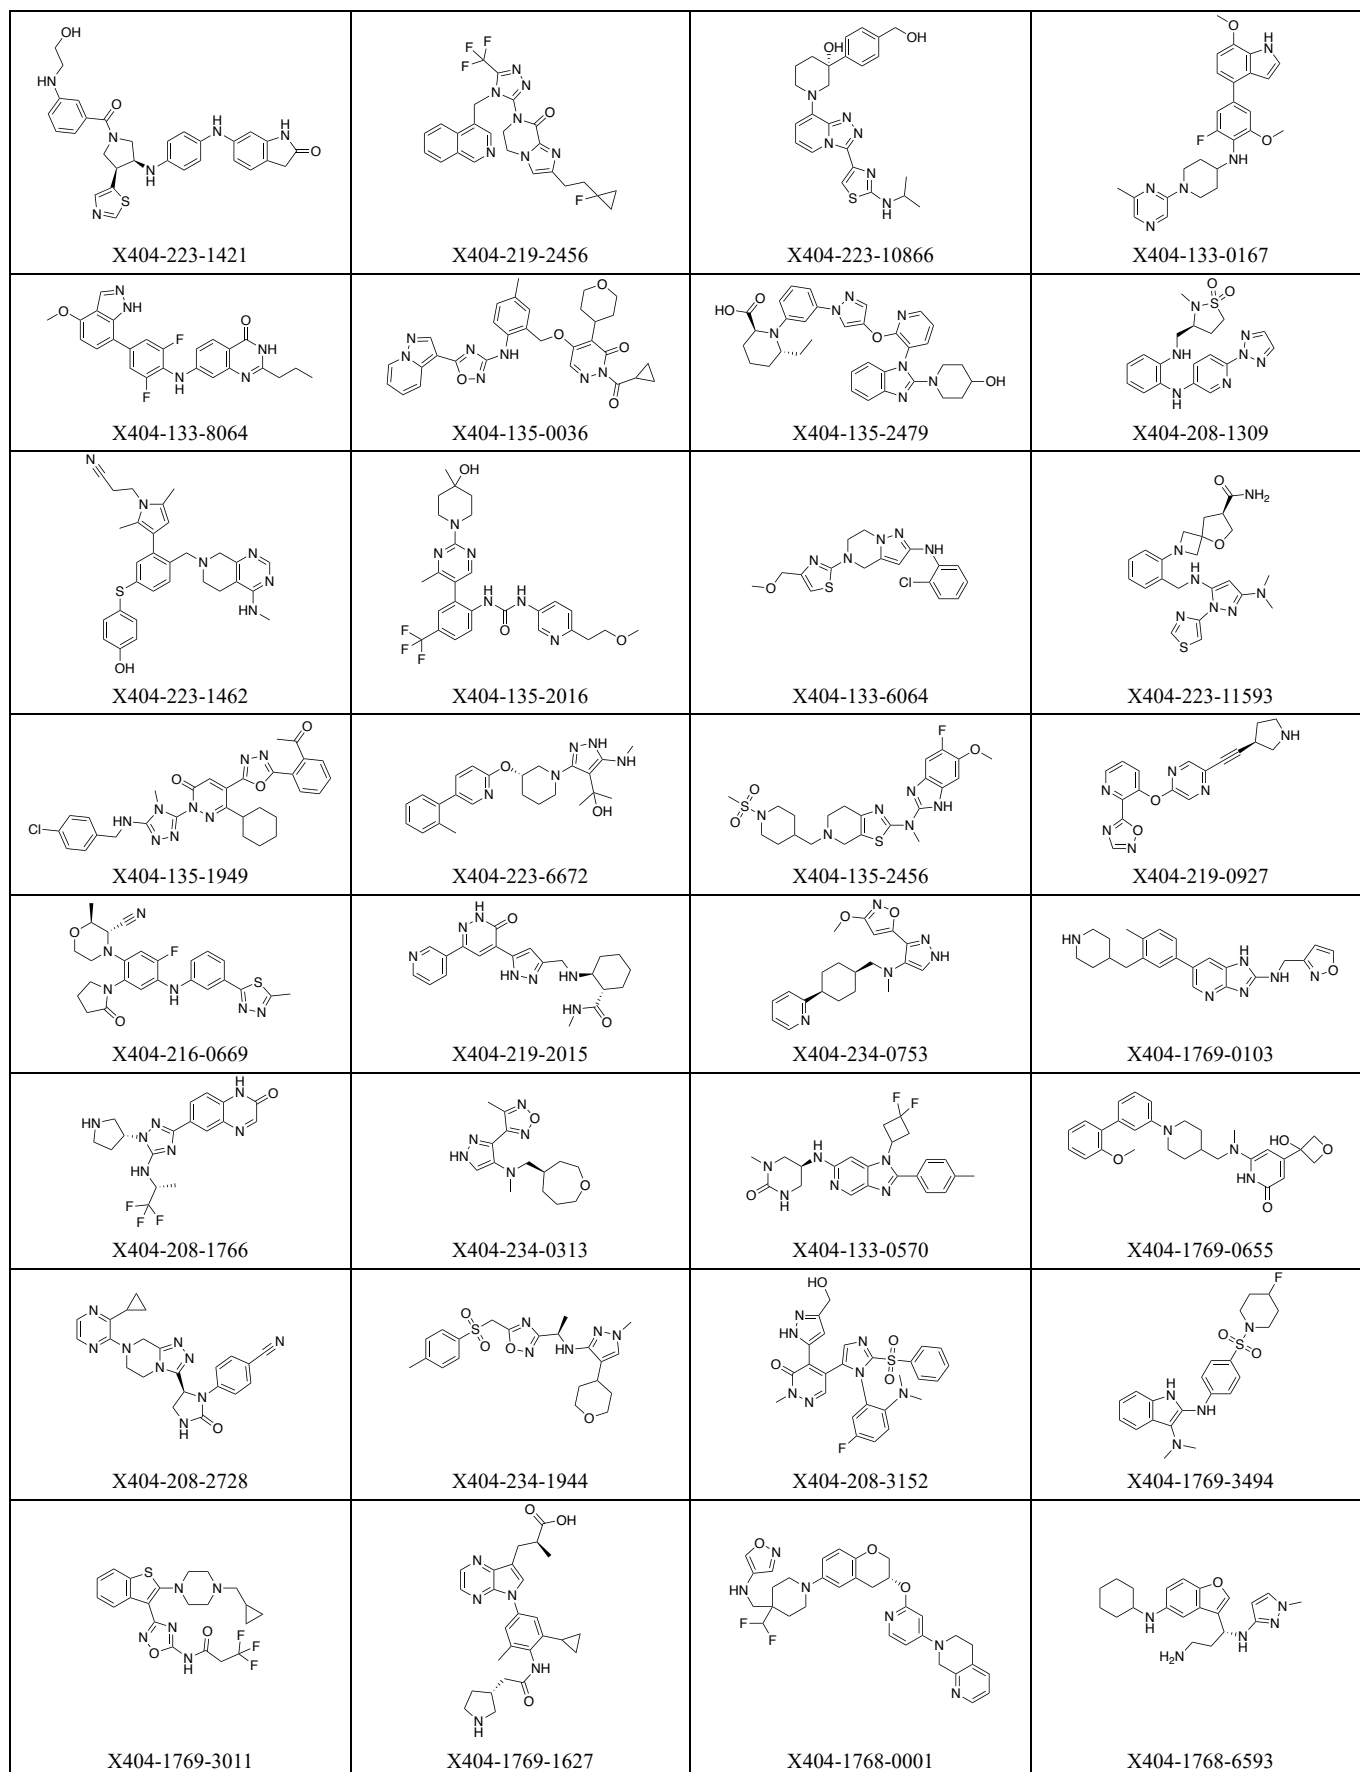 |
| X404-216-0669                                                                       | X404-219-2015                                                                       | X404-234-0753                                                                        | X404-1769-0103                                                                        |
| 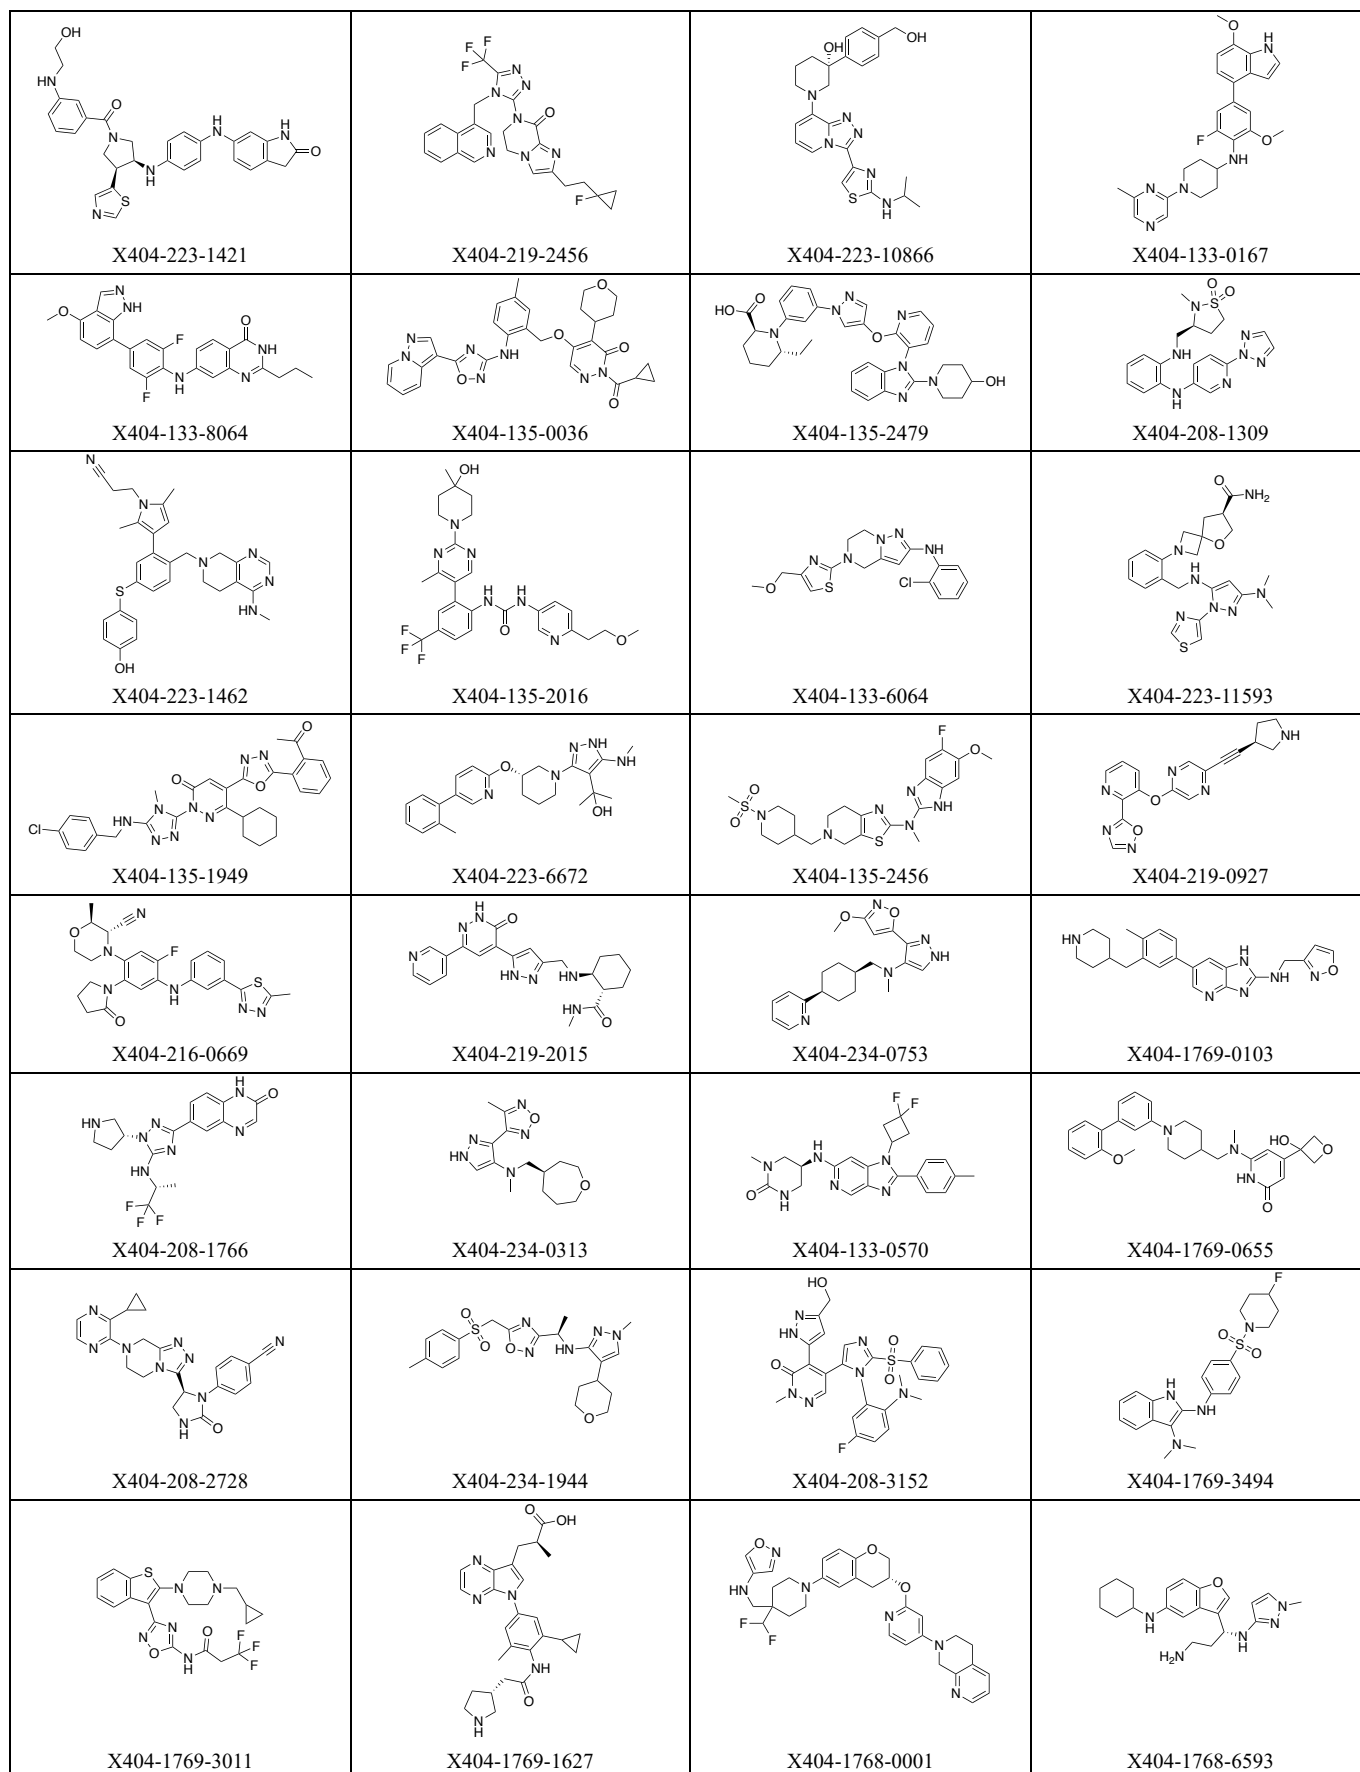 | 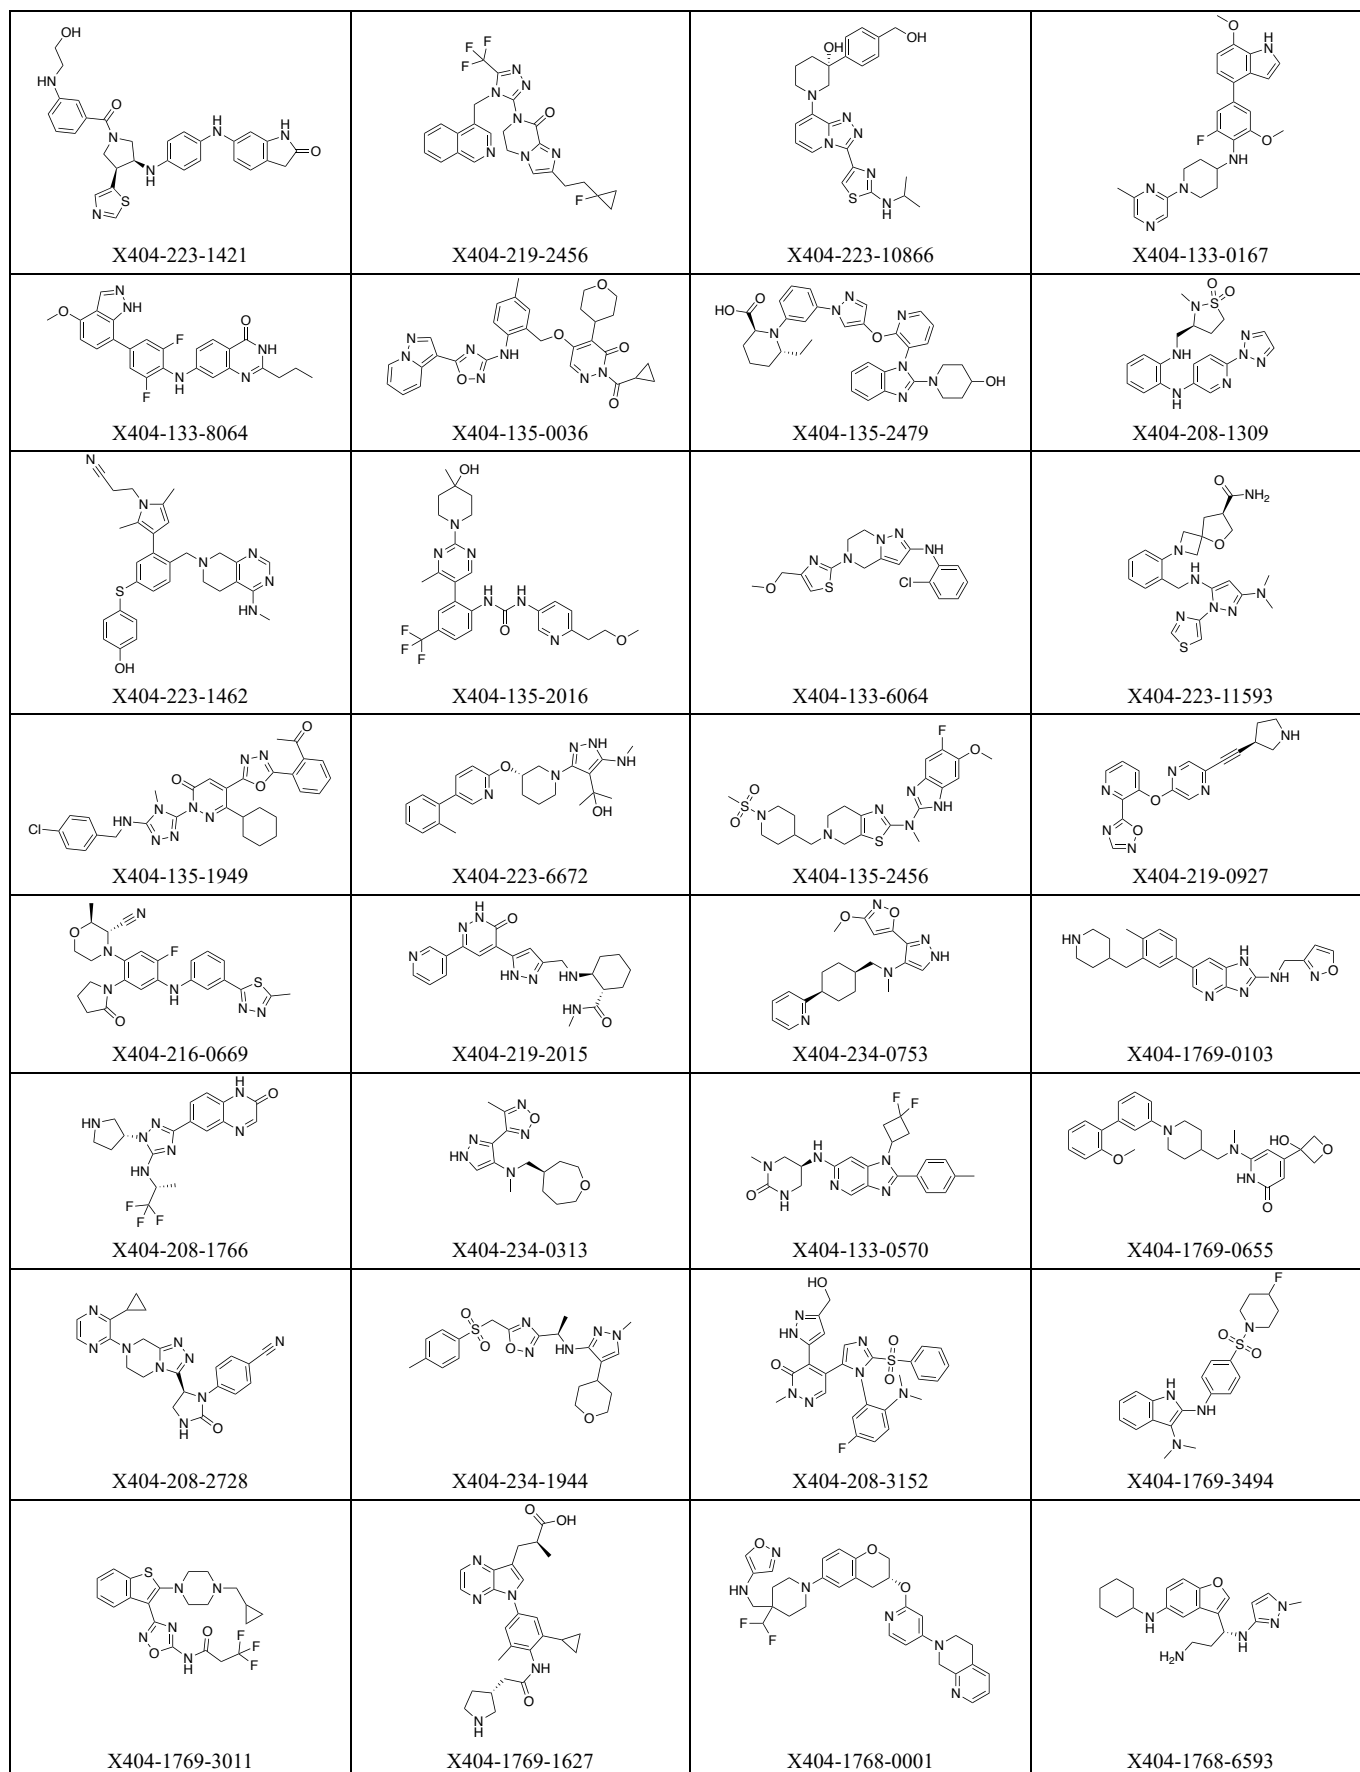 | 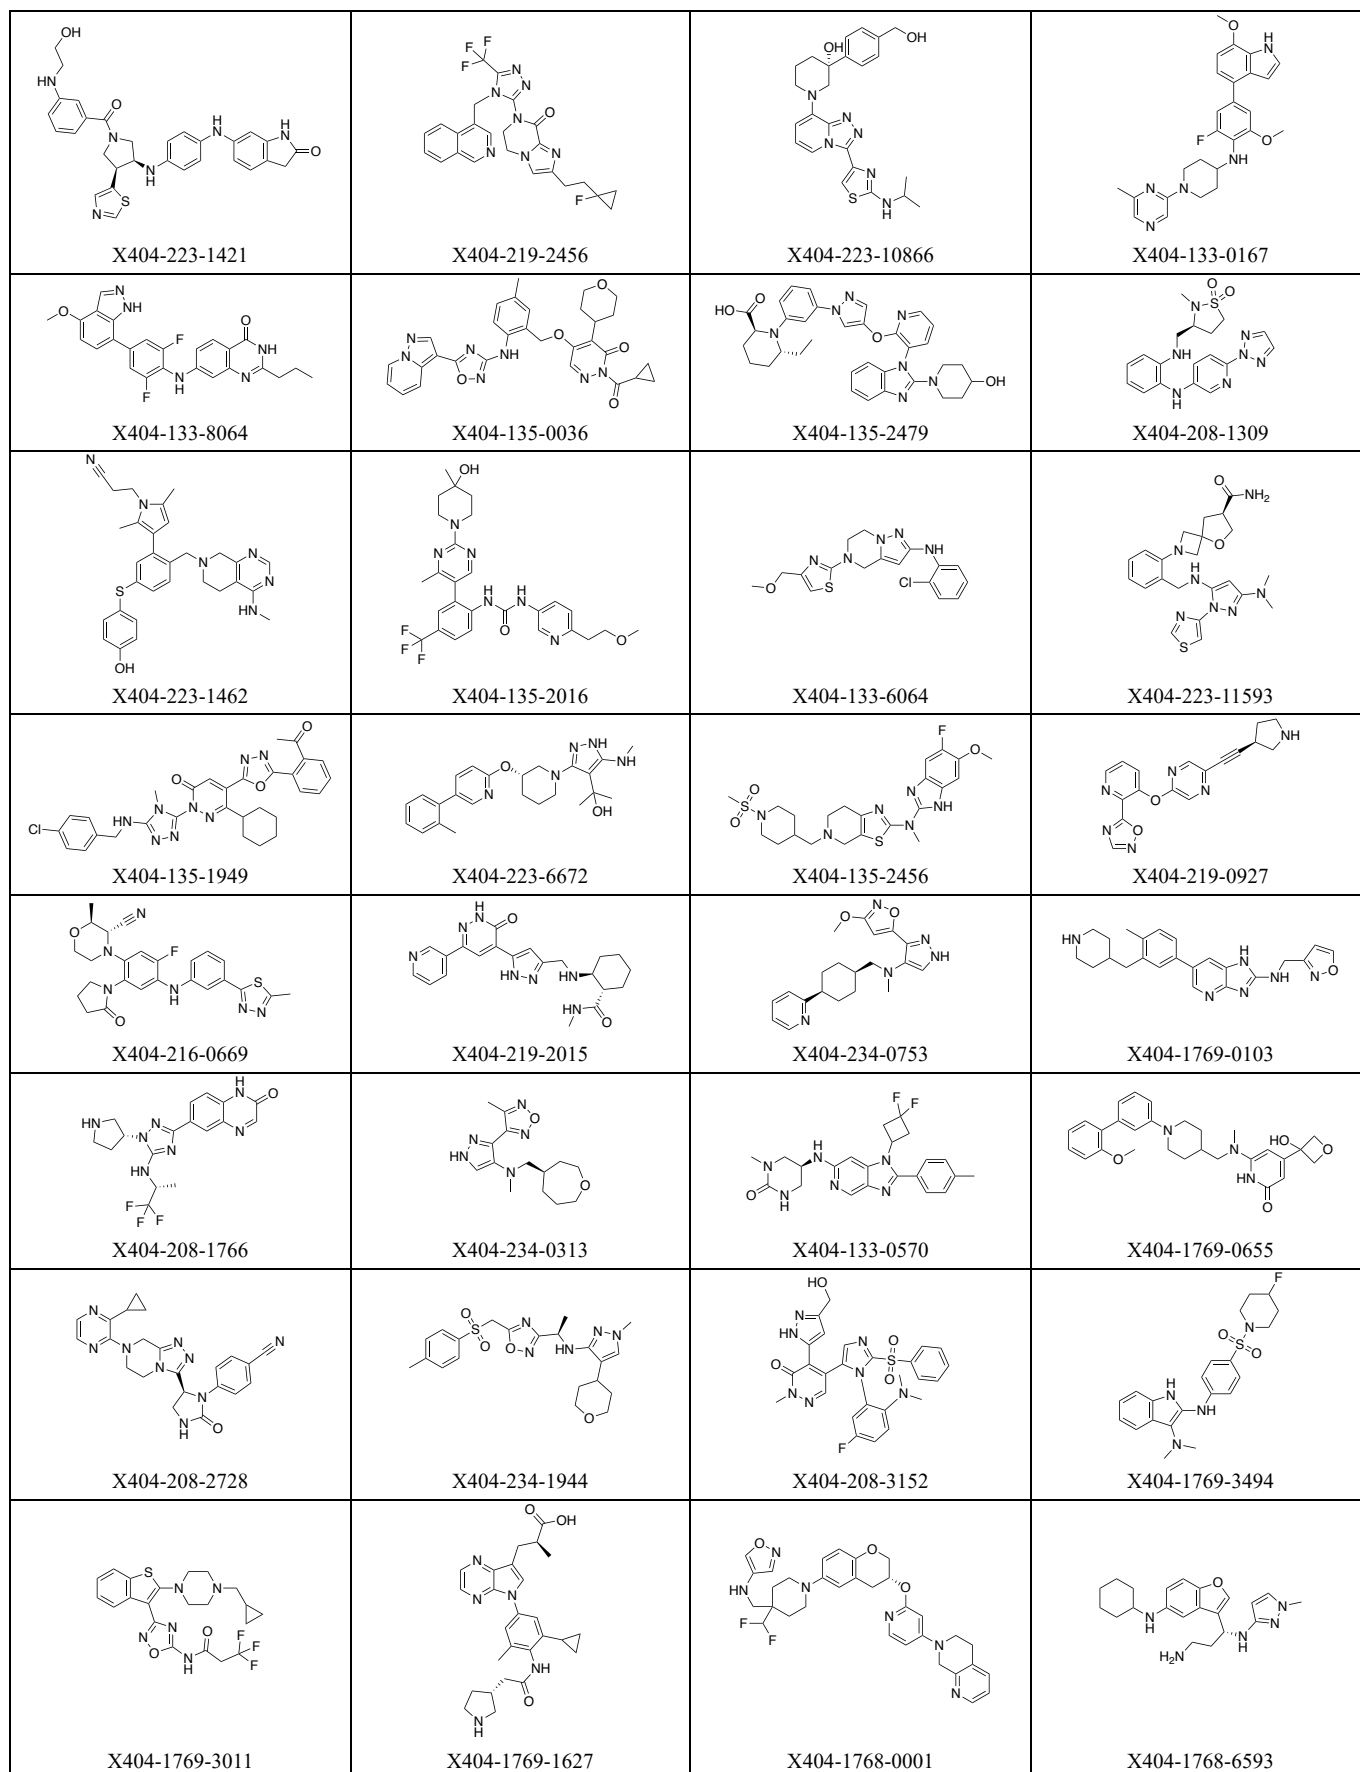 | 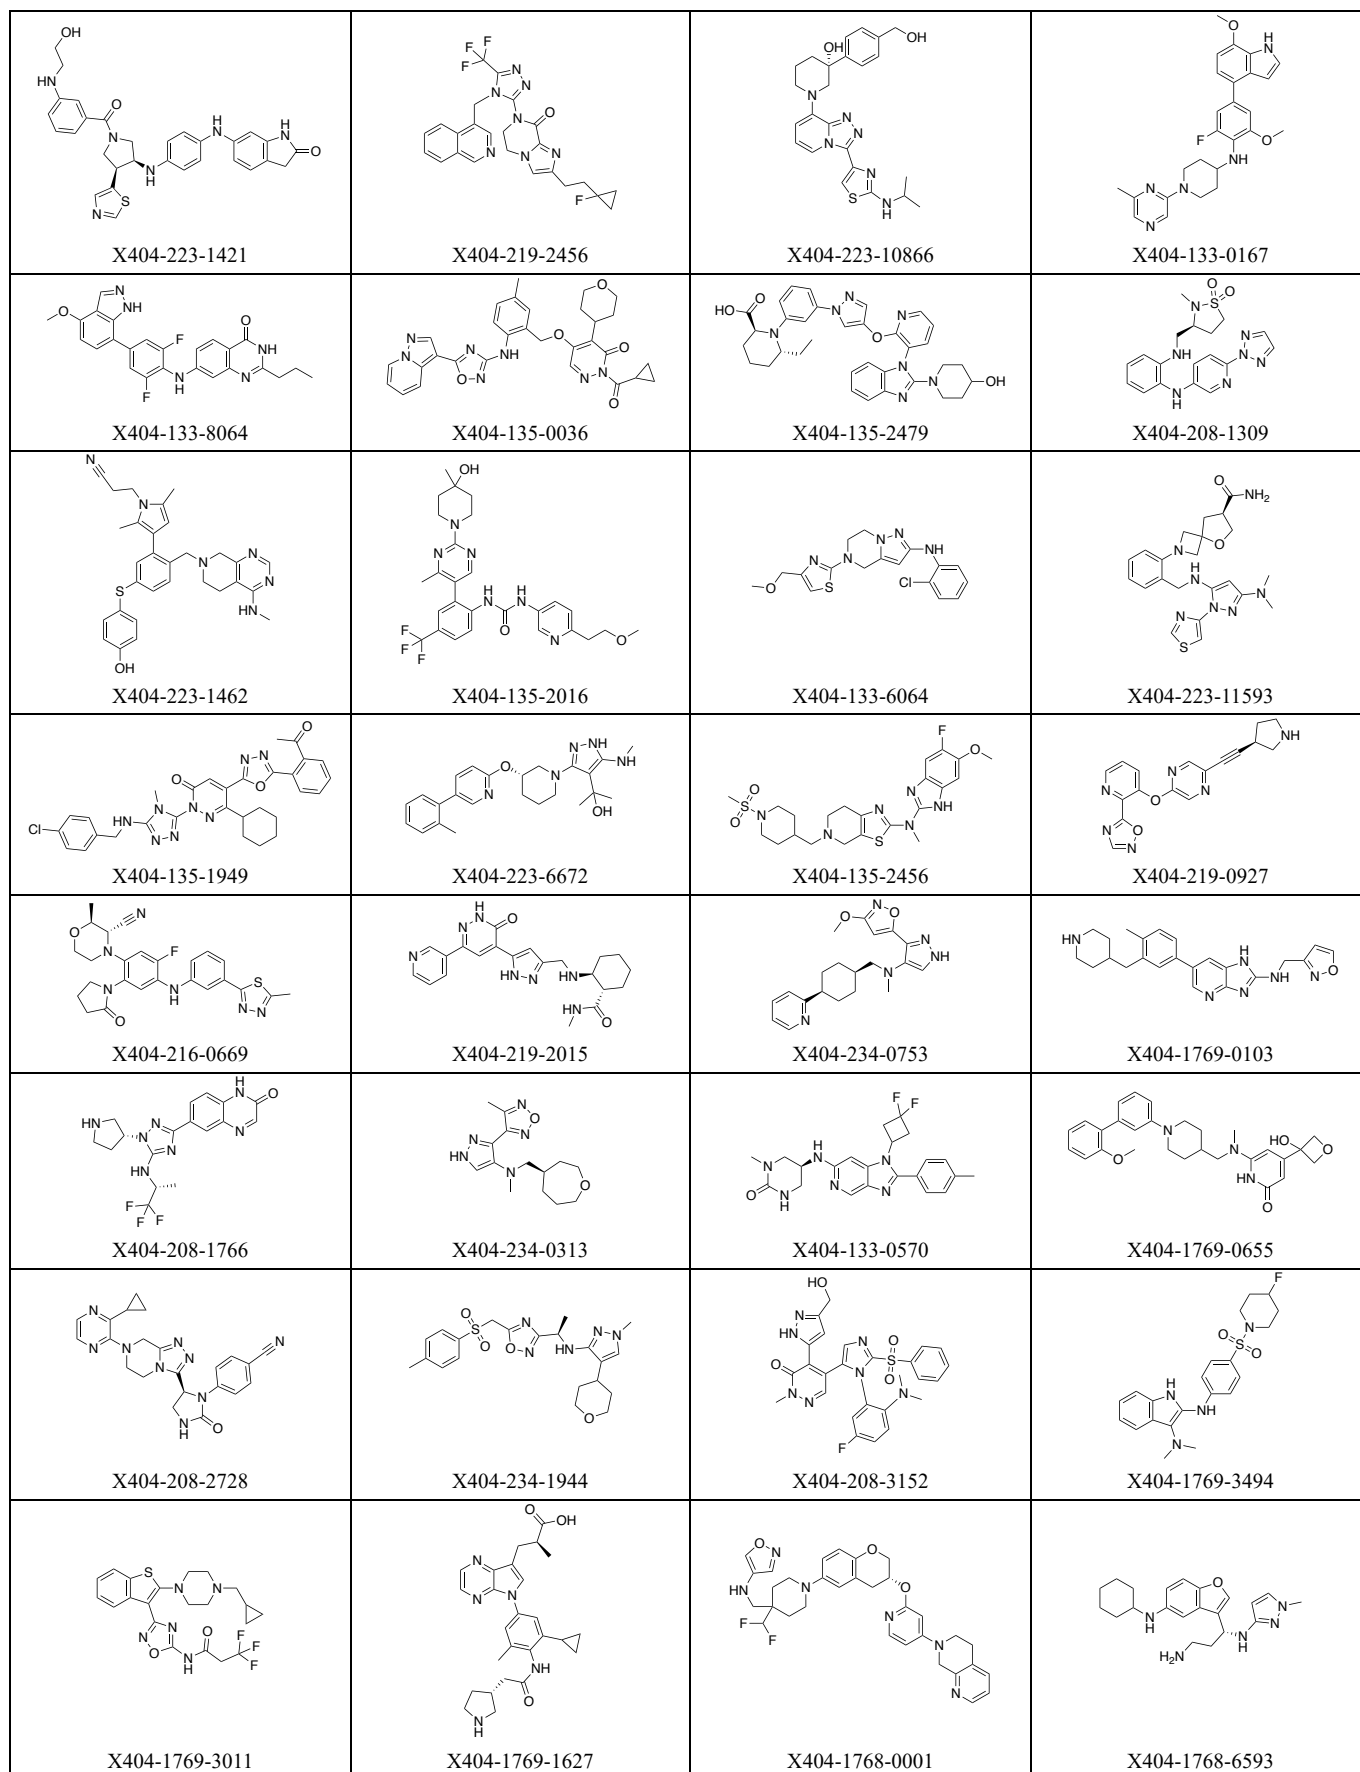 |
| X404-208-1766                                                                       | X404-234-0313                                                                       | X404-133-0570                                                                        | X404-1769-0655                                                                        |
| 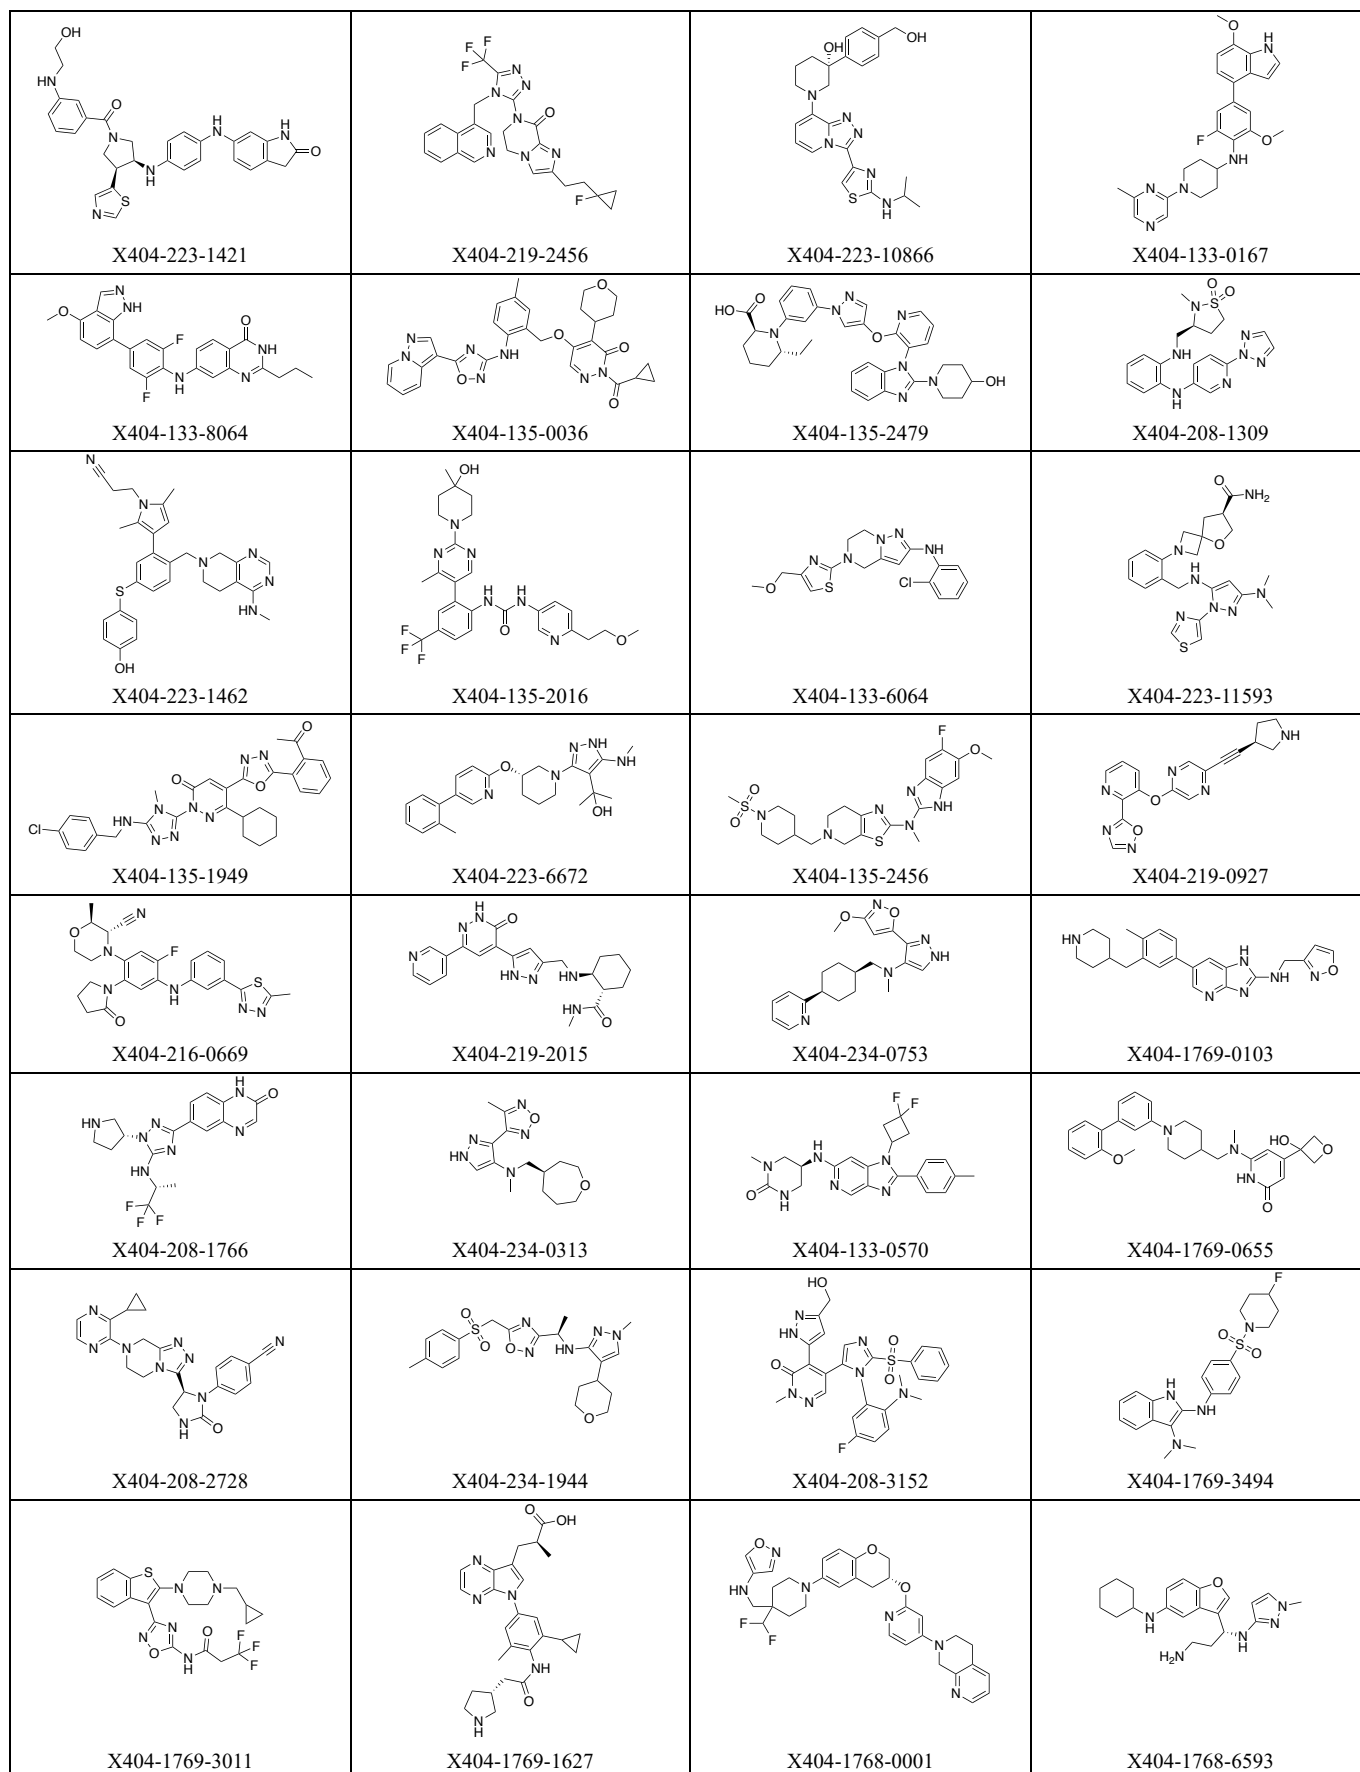 | 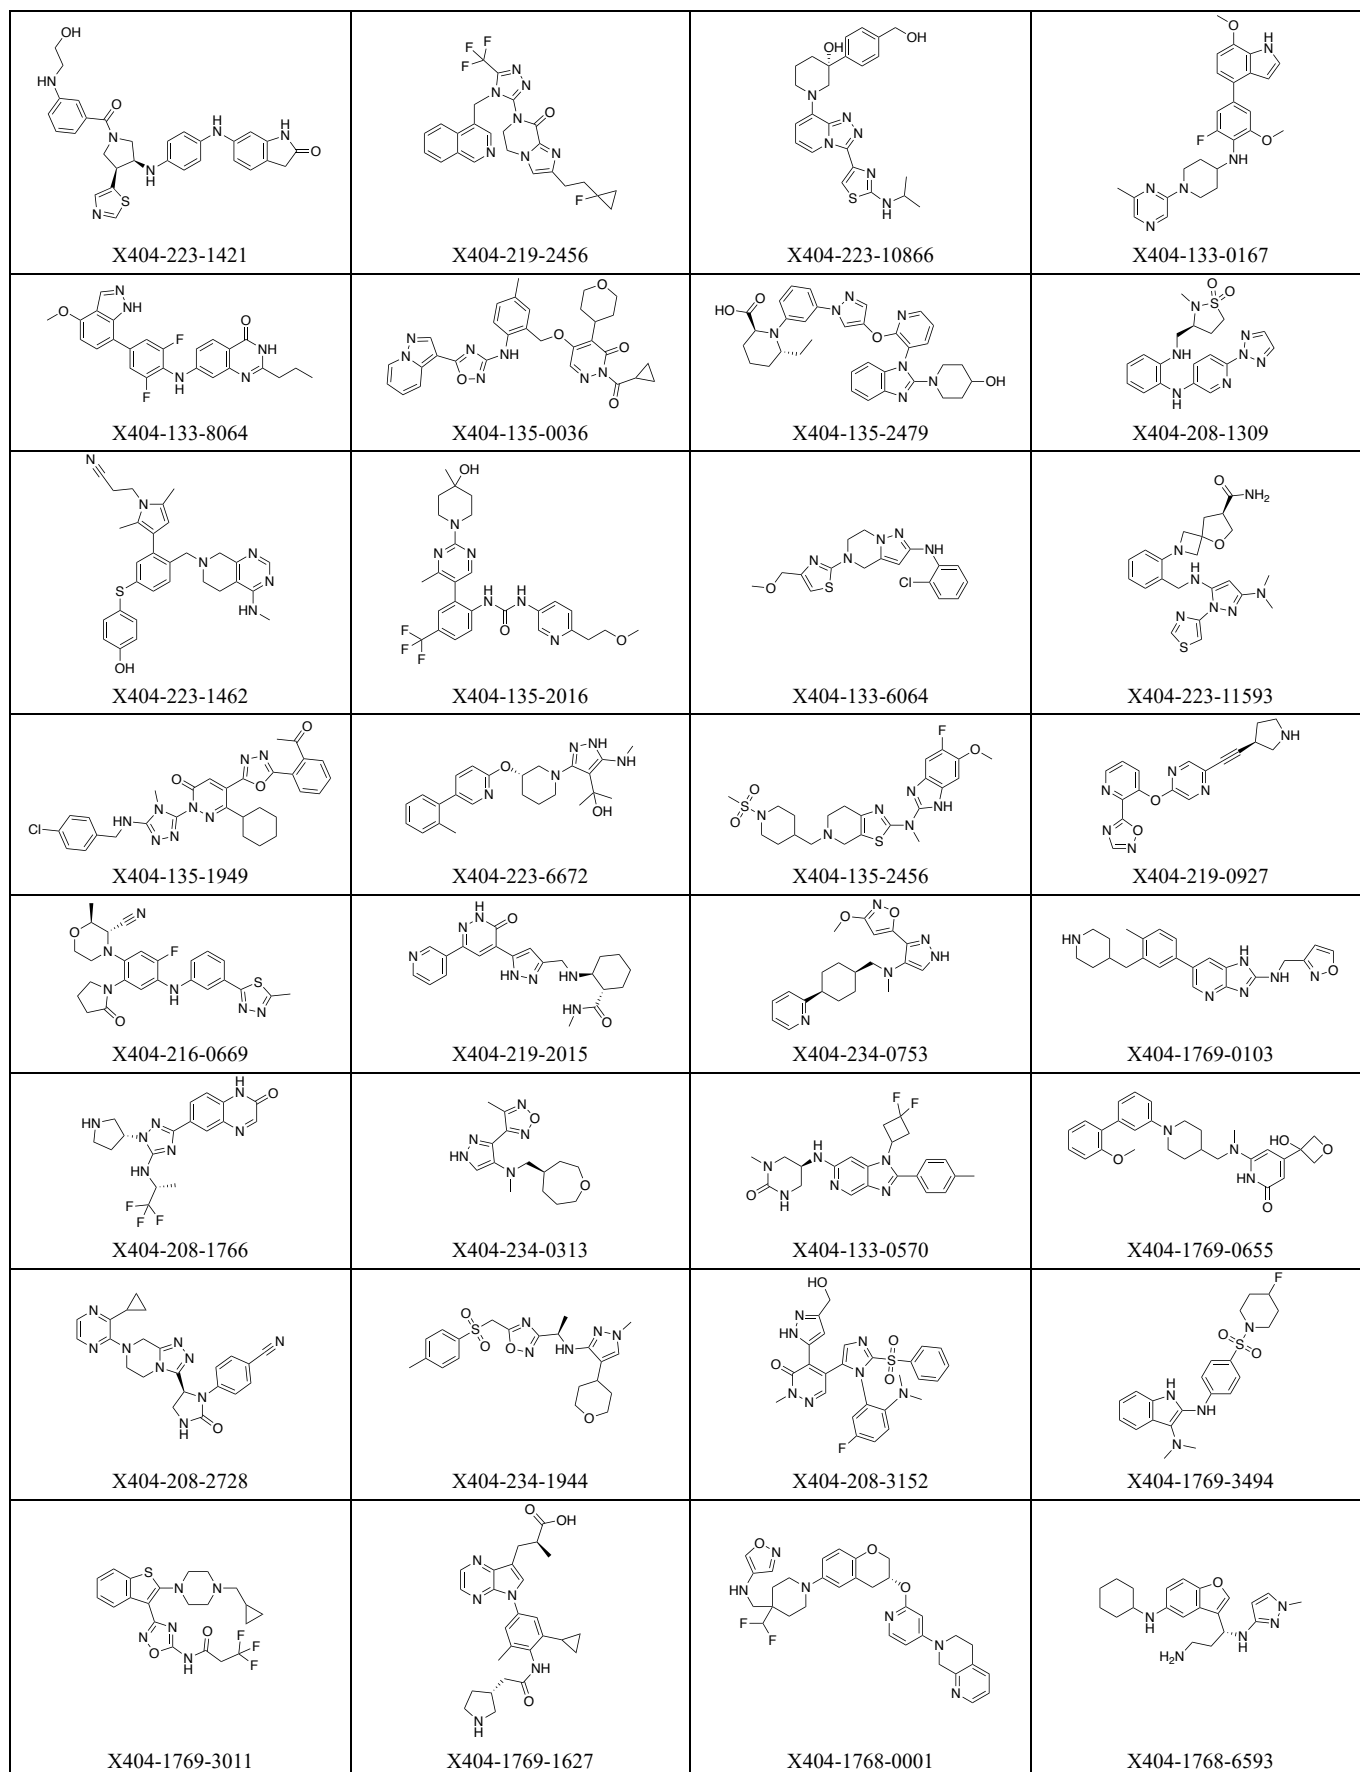 | 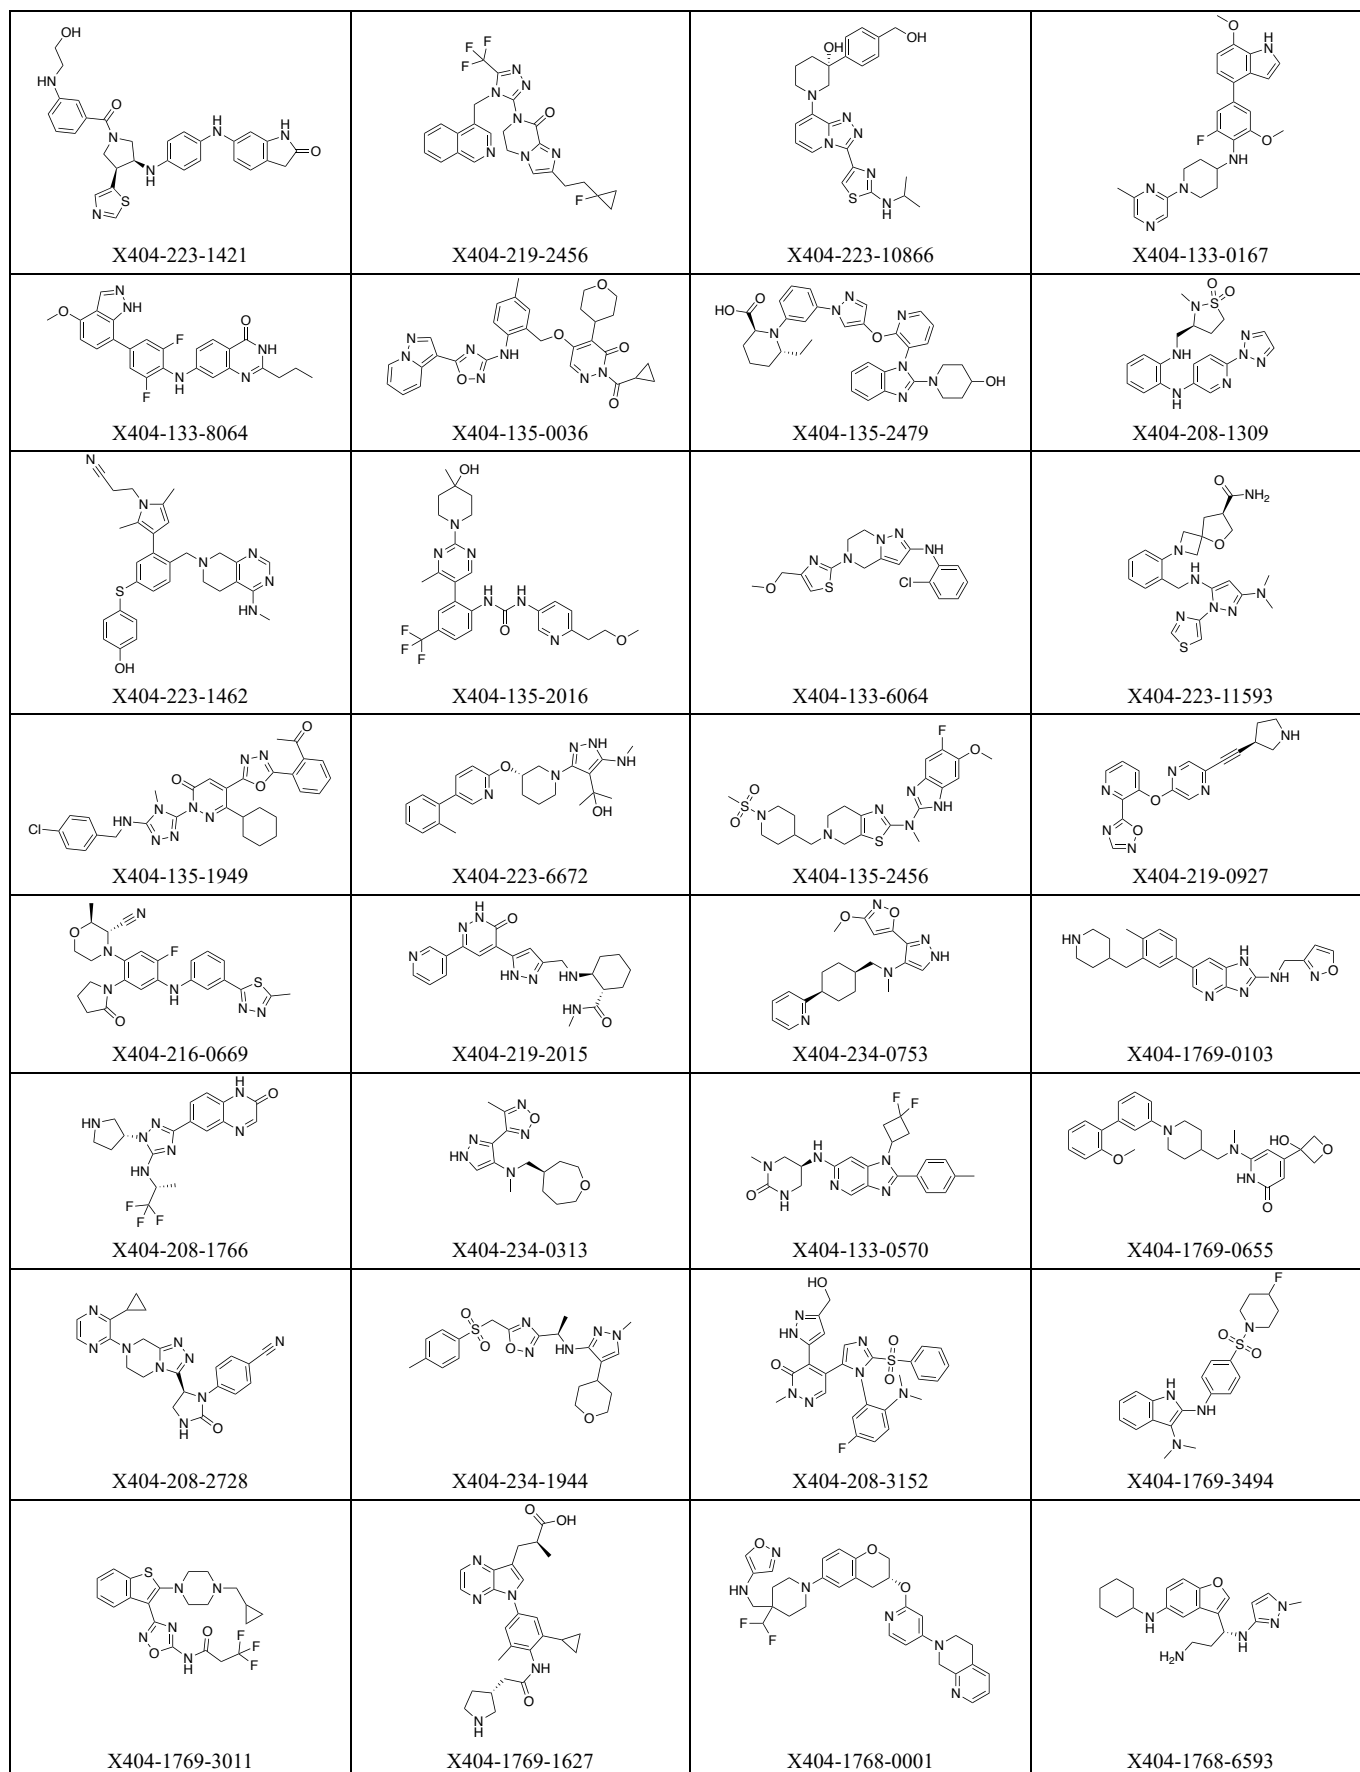 | 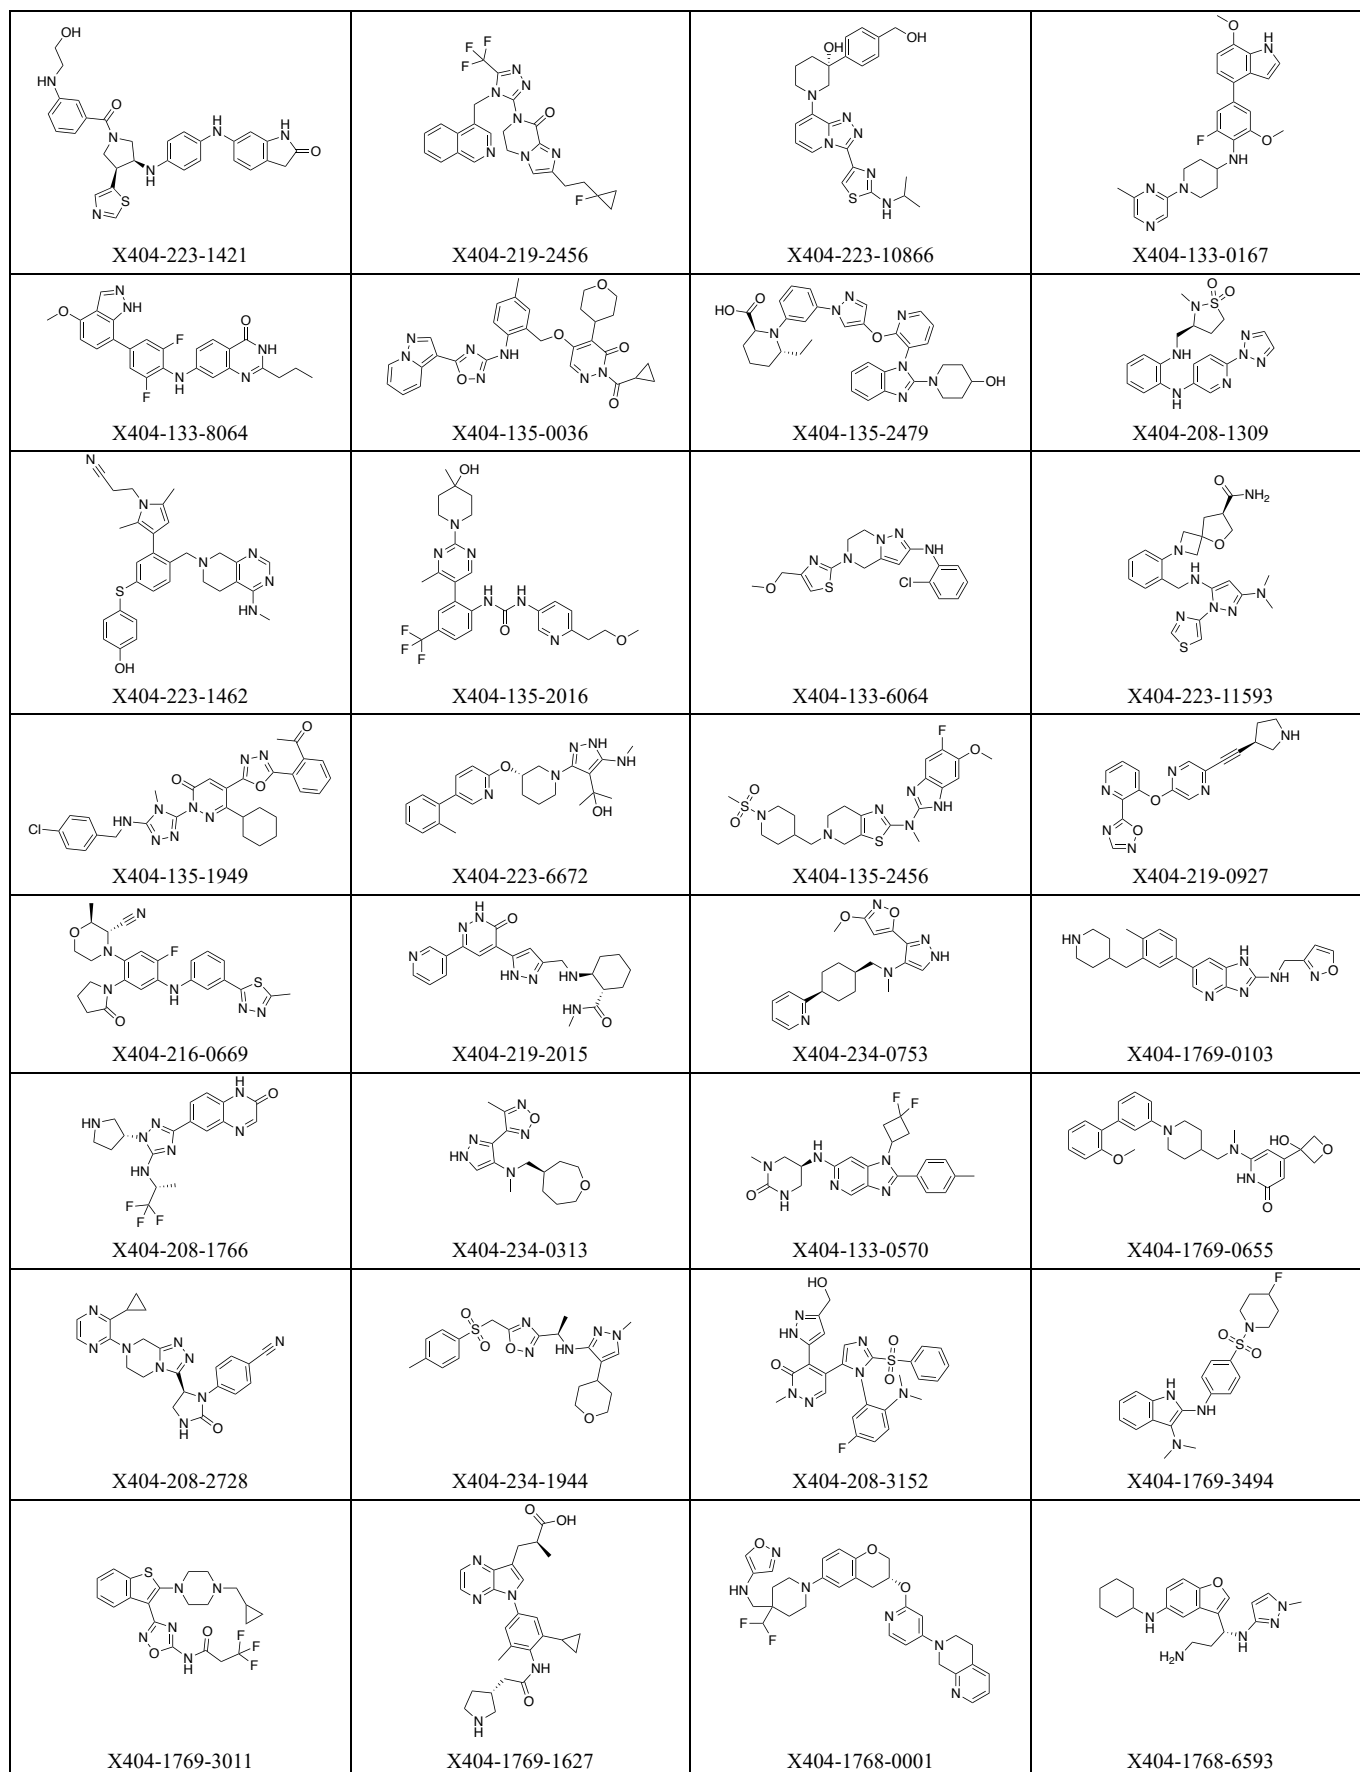 |
| X404-208-2728                                                                       | X404-234-1944                                                                       | X404-208-3152                                                                        | X404-1769-3494                                                                        |
| 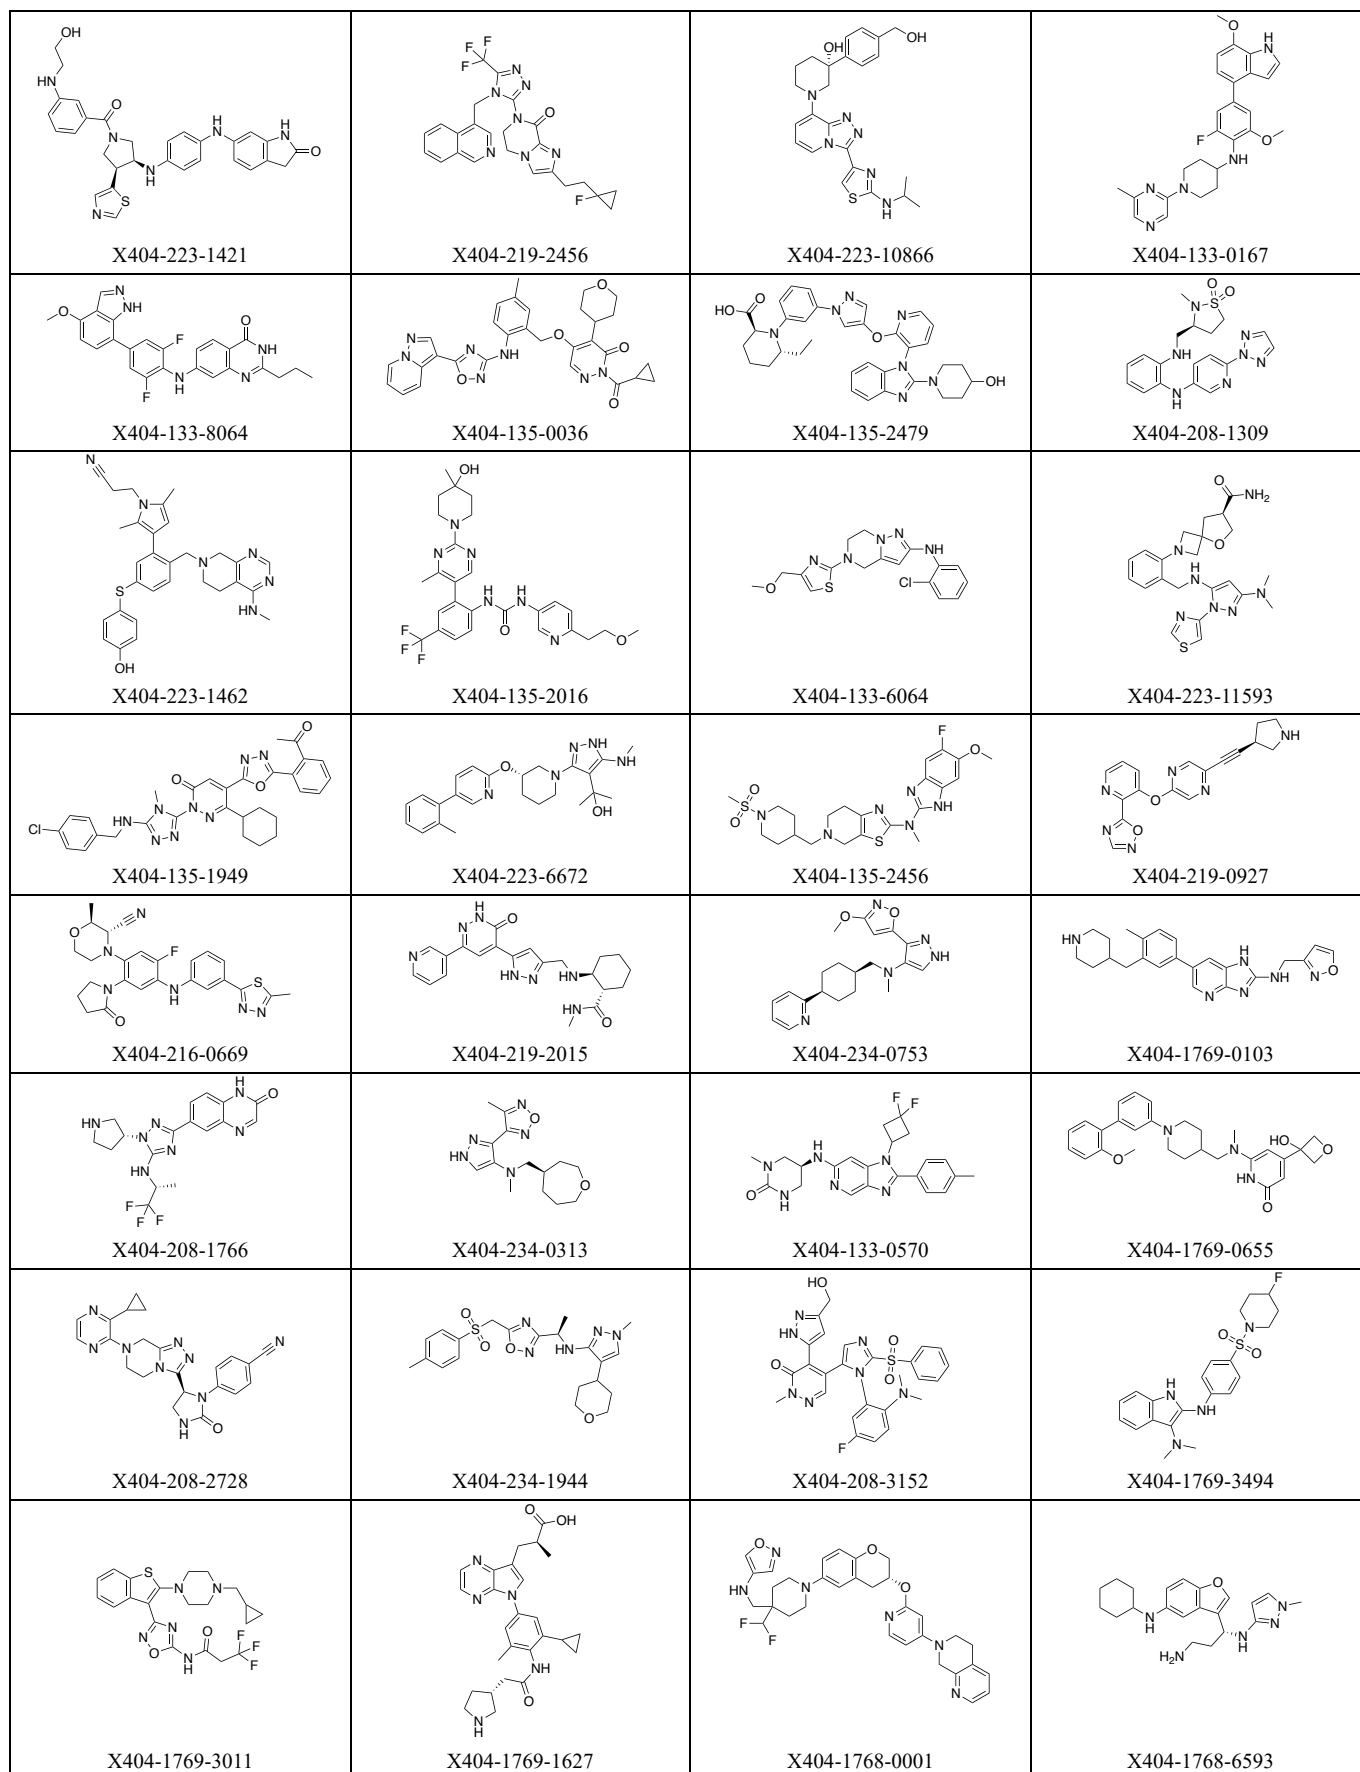 | 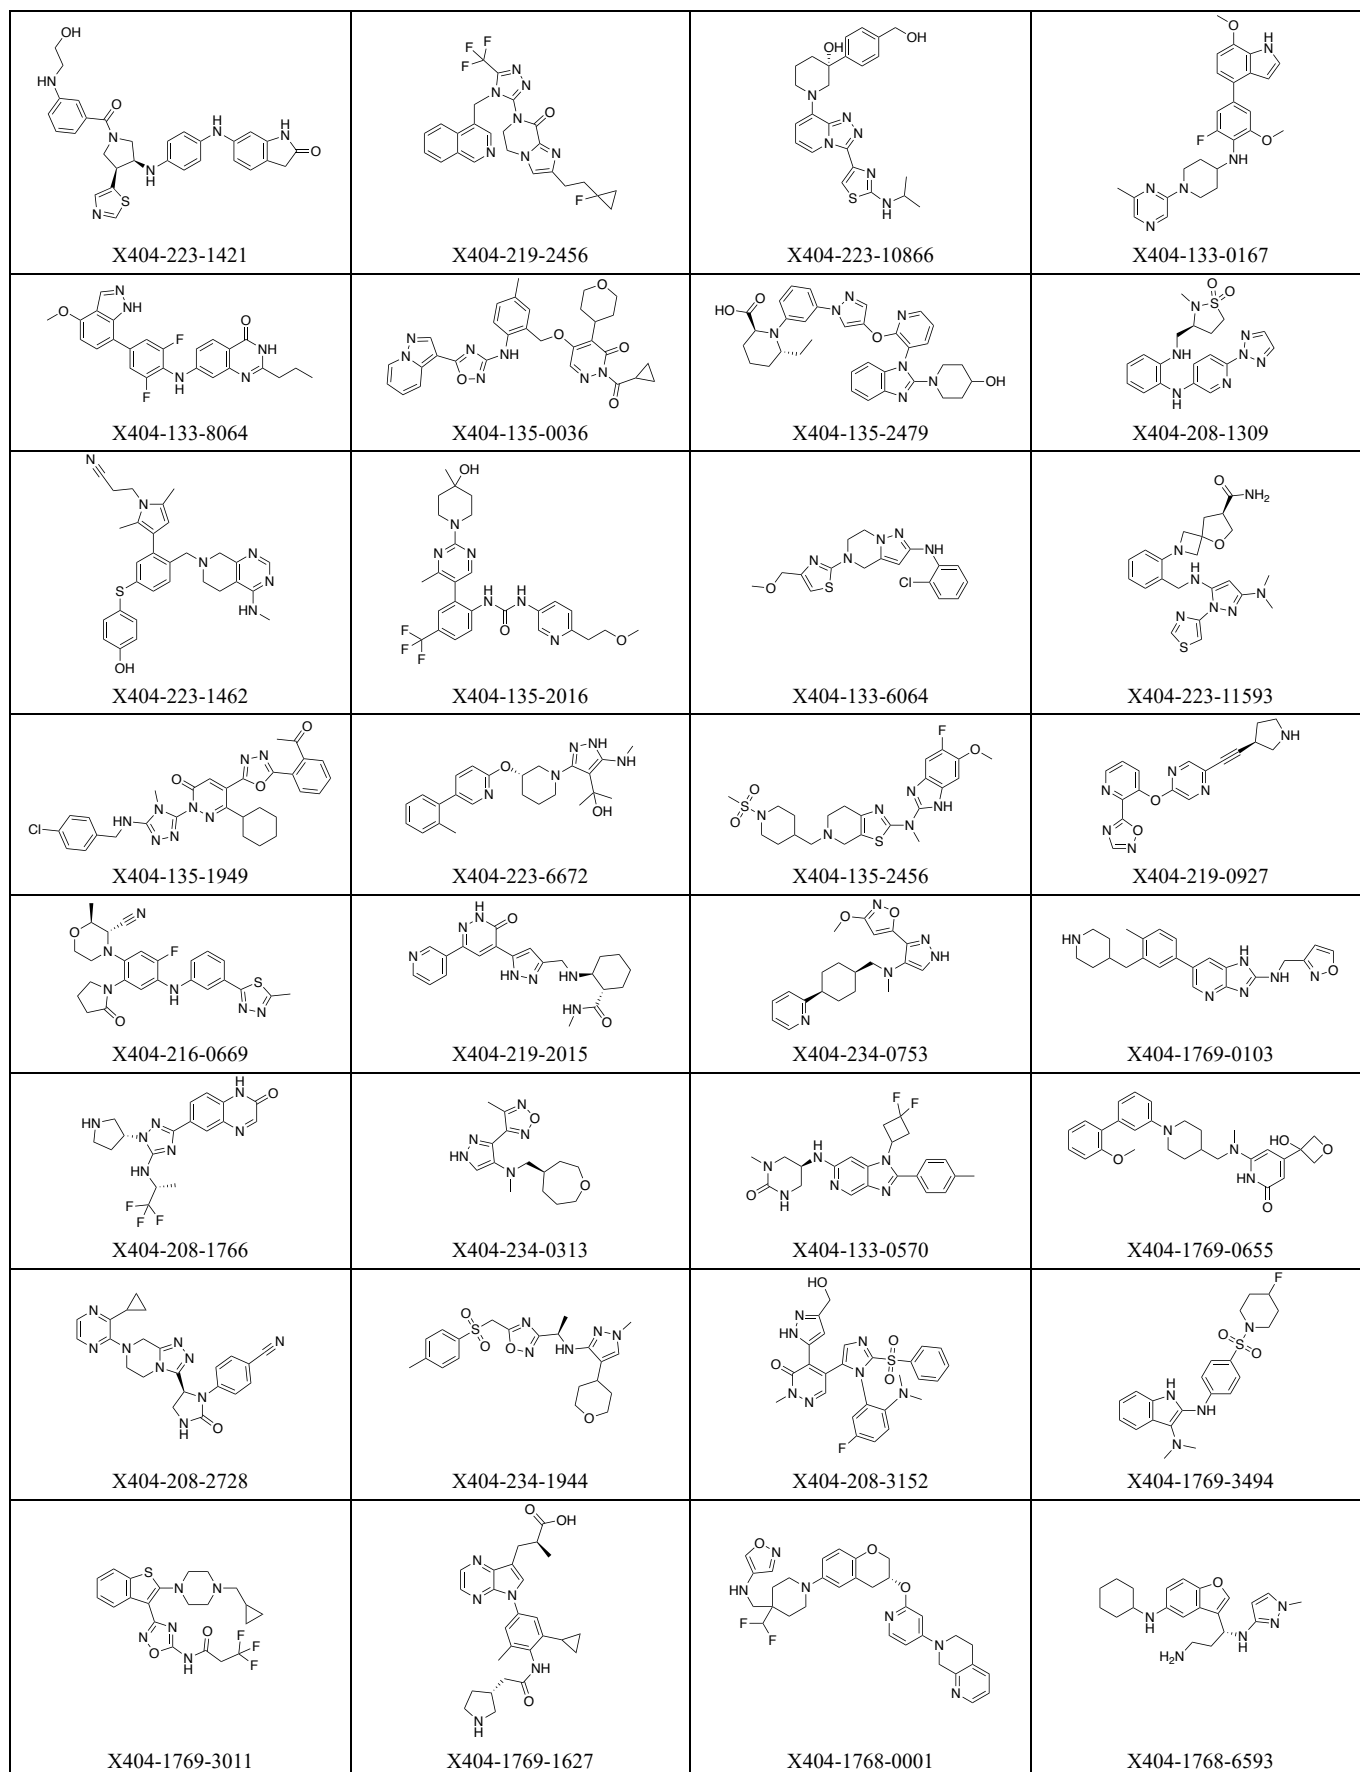 | 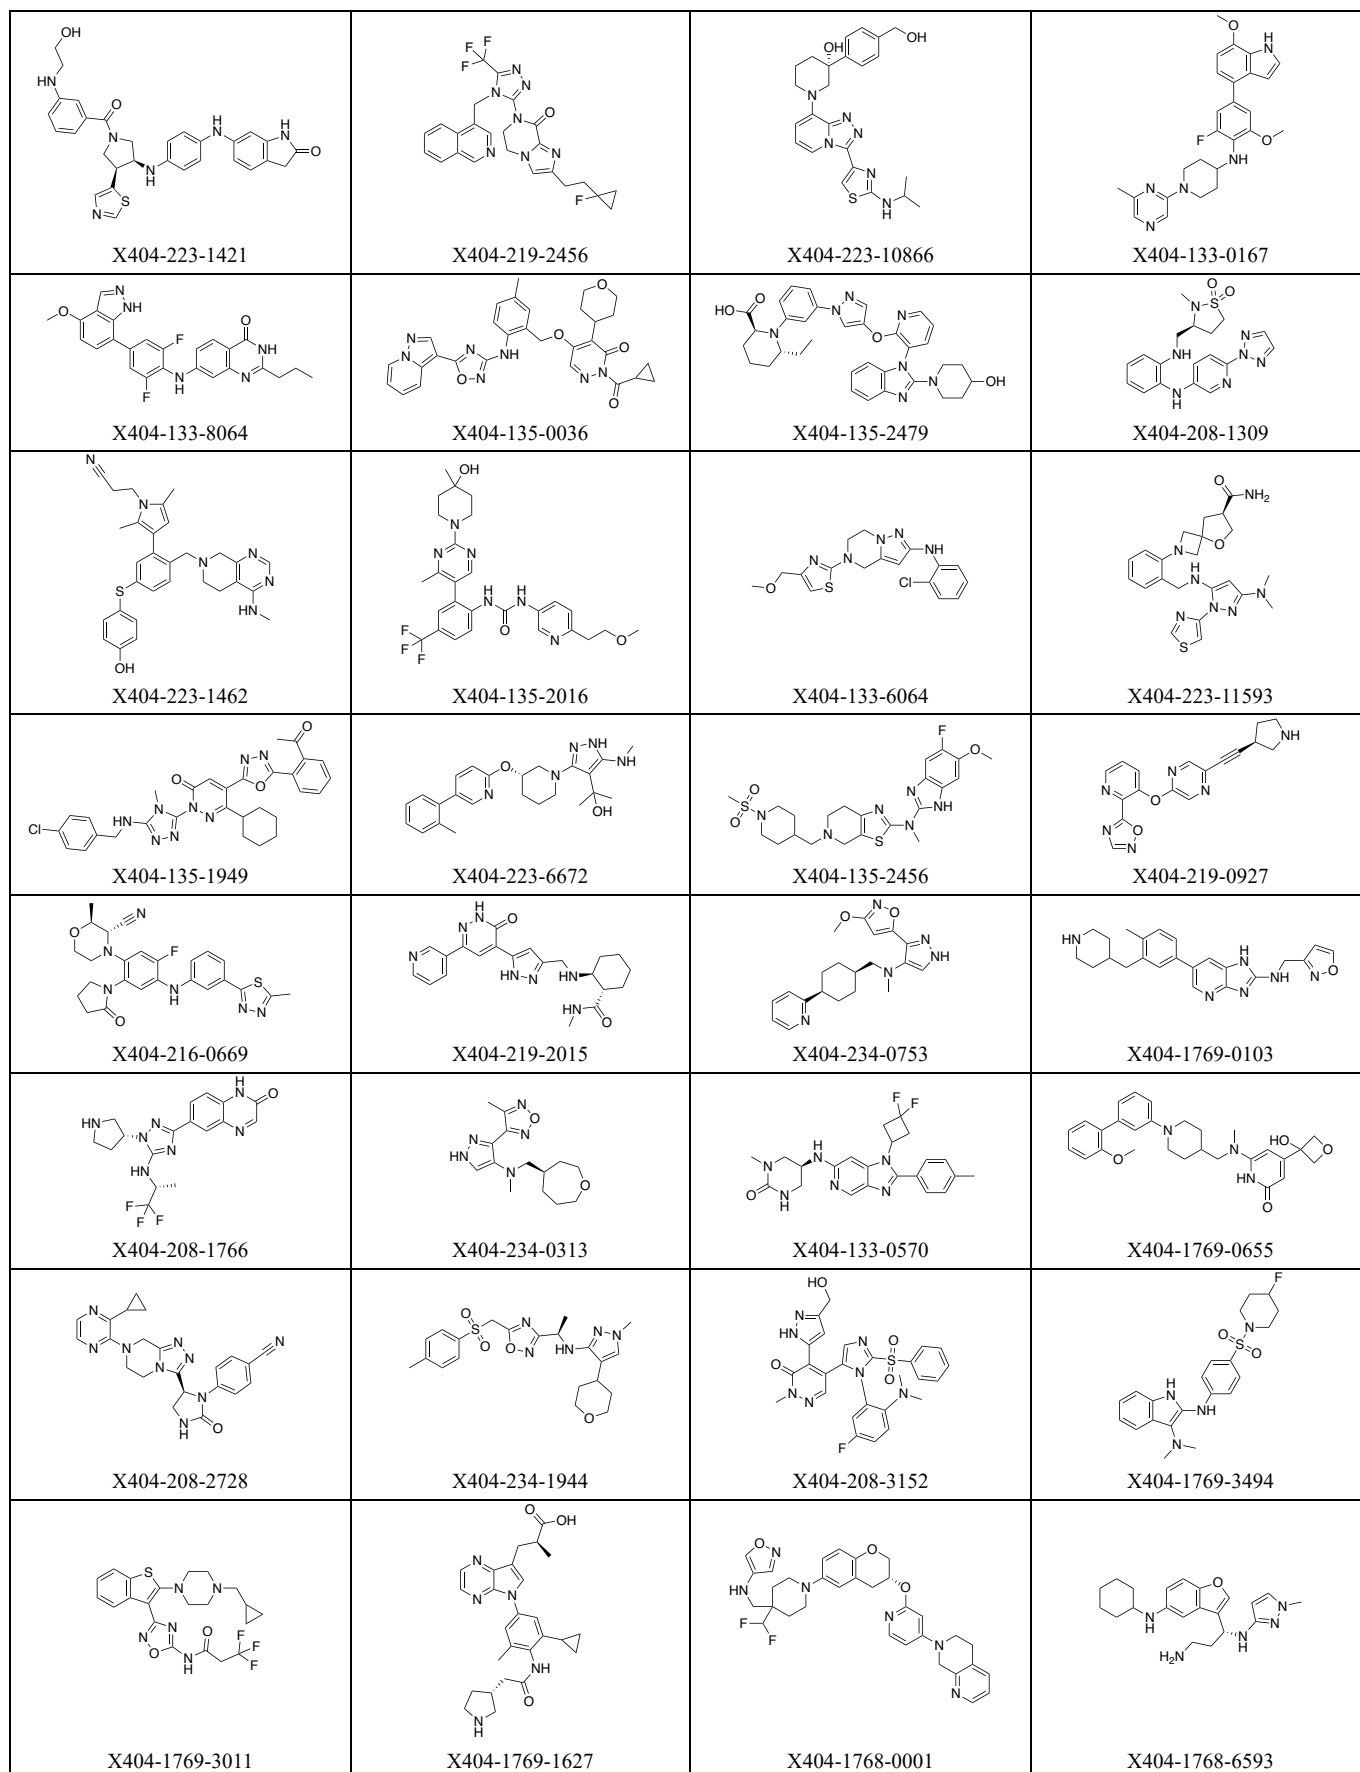 | 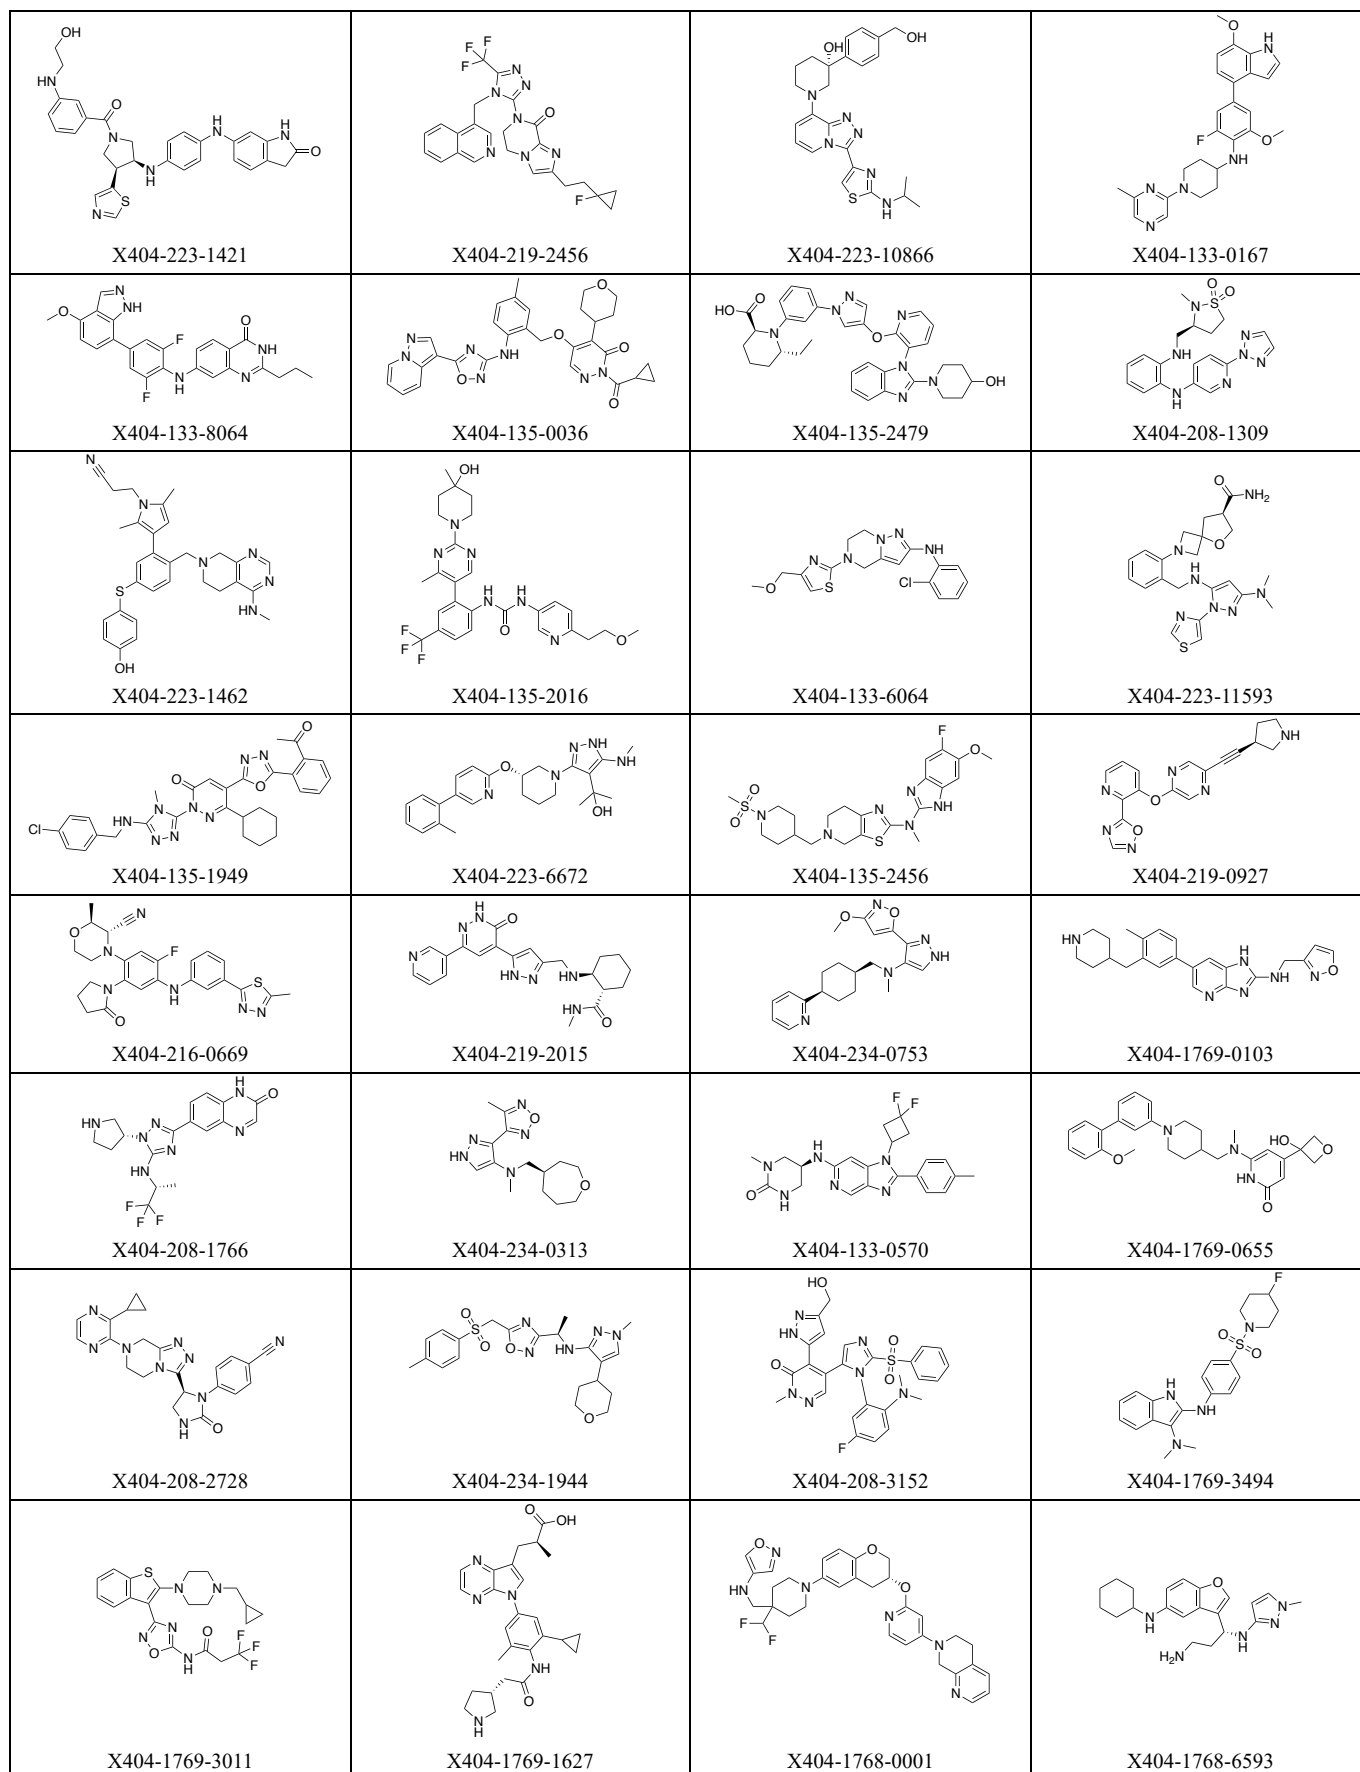 |
| X404-1769-3011                                                                      | X404-1769-1627                                                                      | X404-1768-0001                                                                       | X404-1768-6593                                                                        |

|                                                                                     |                                                                                     |                                                                                      |                                                                                       |
|-------------------------------------------------------------------------------------|-------------------------------------------------------------------------------------|--------------------------------------------------------------------------------------|---------------------------------------------------------------------------------------|
| 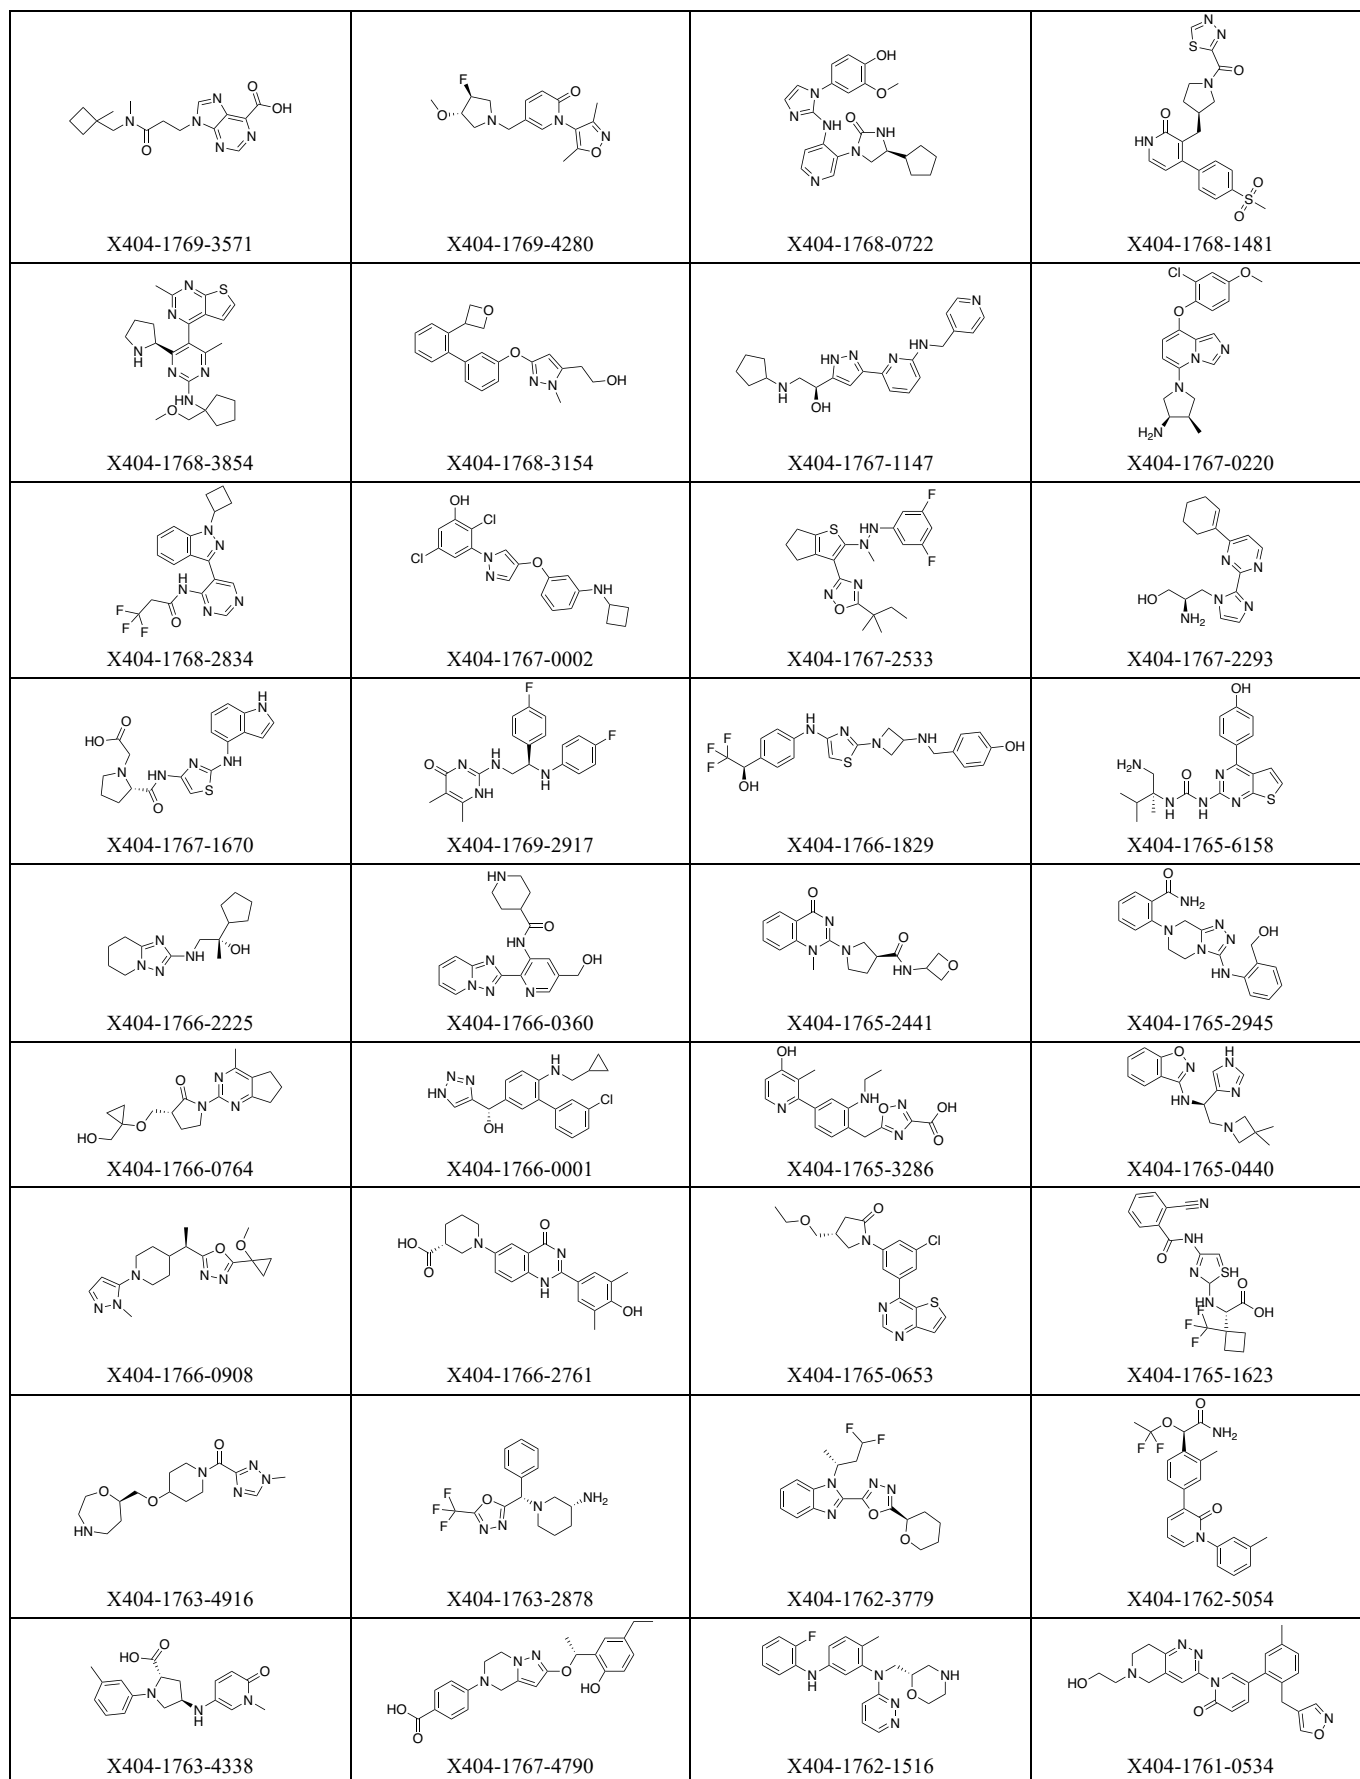   | 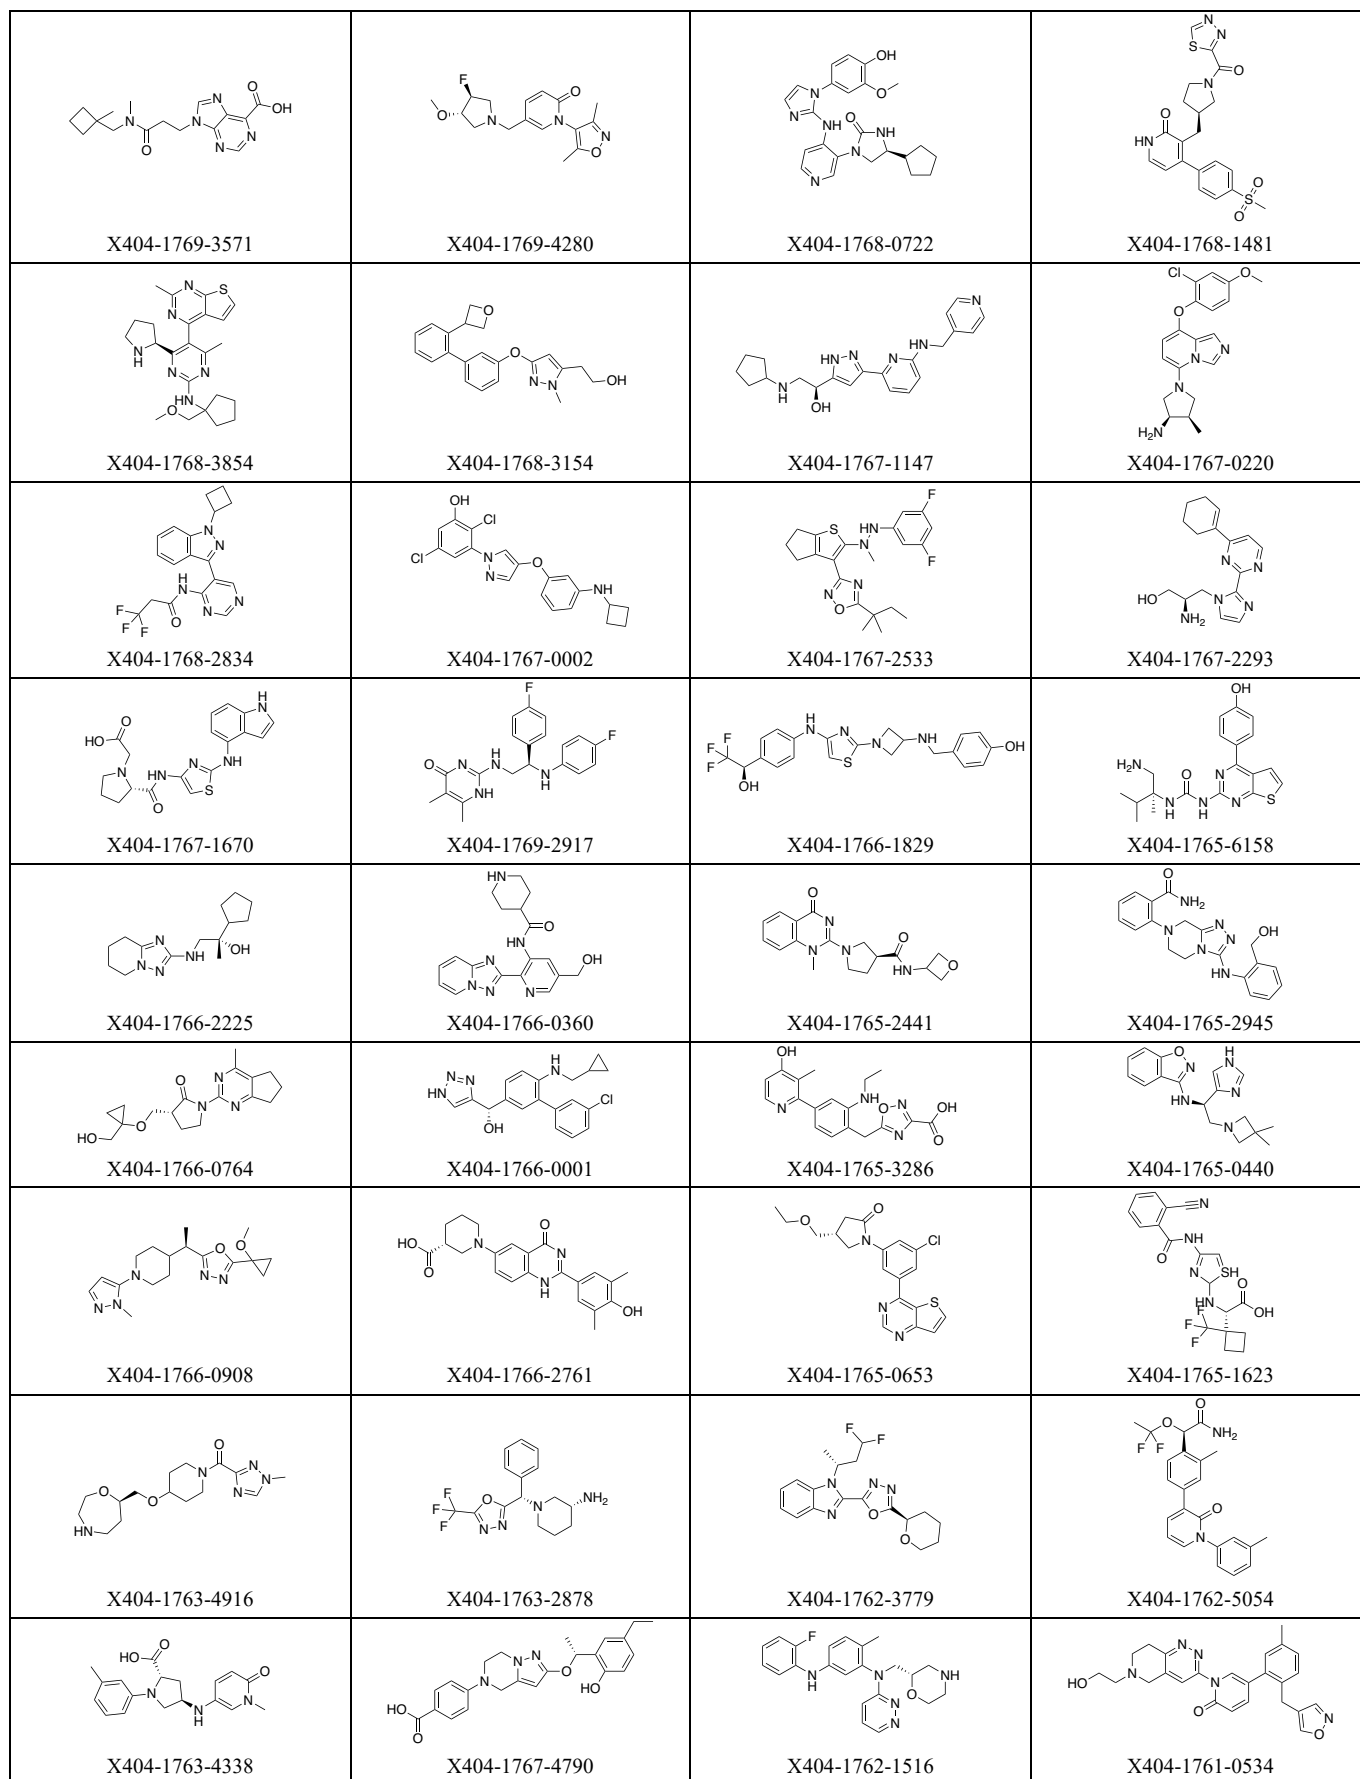   | 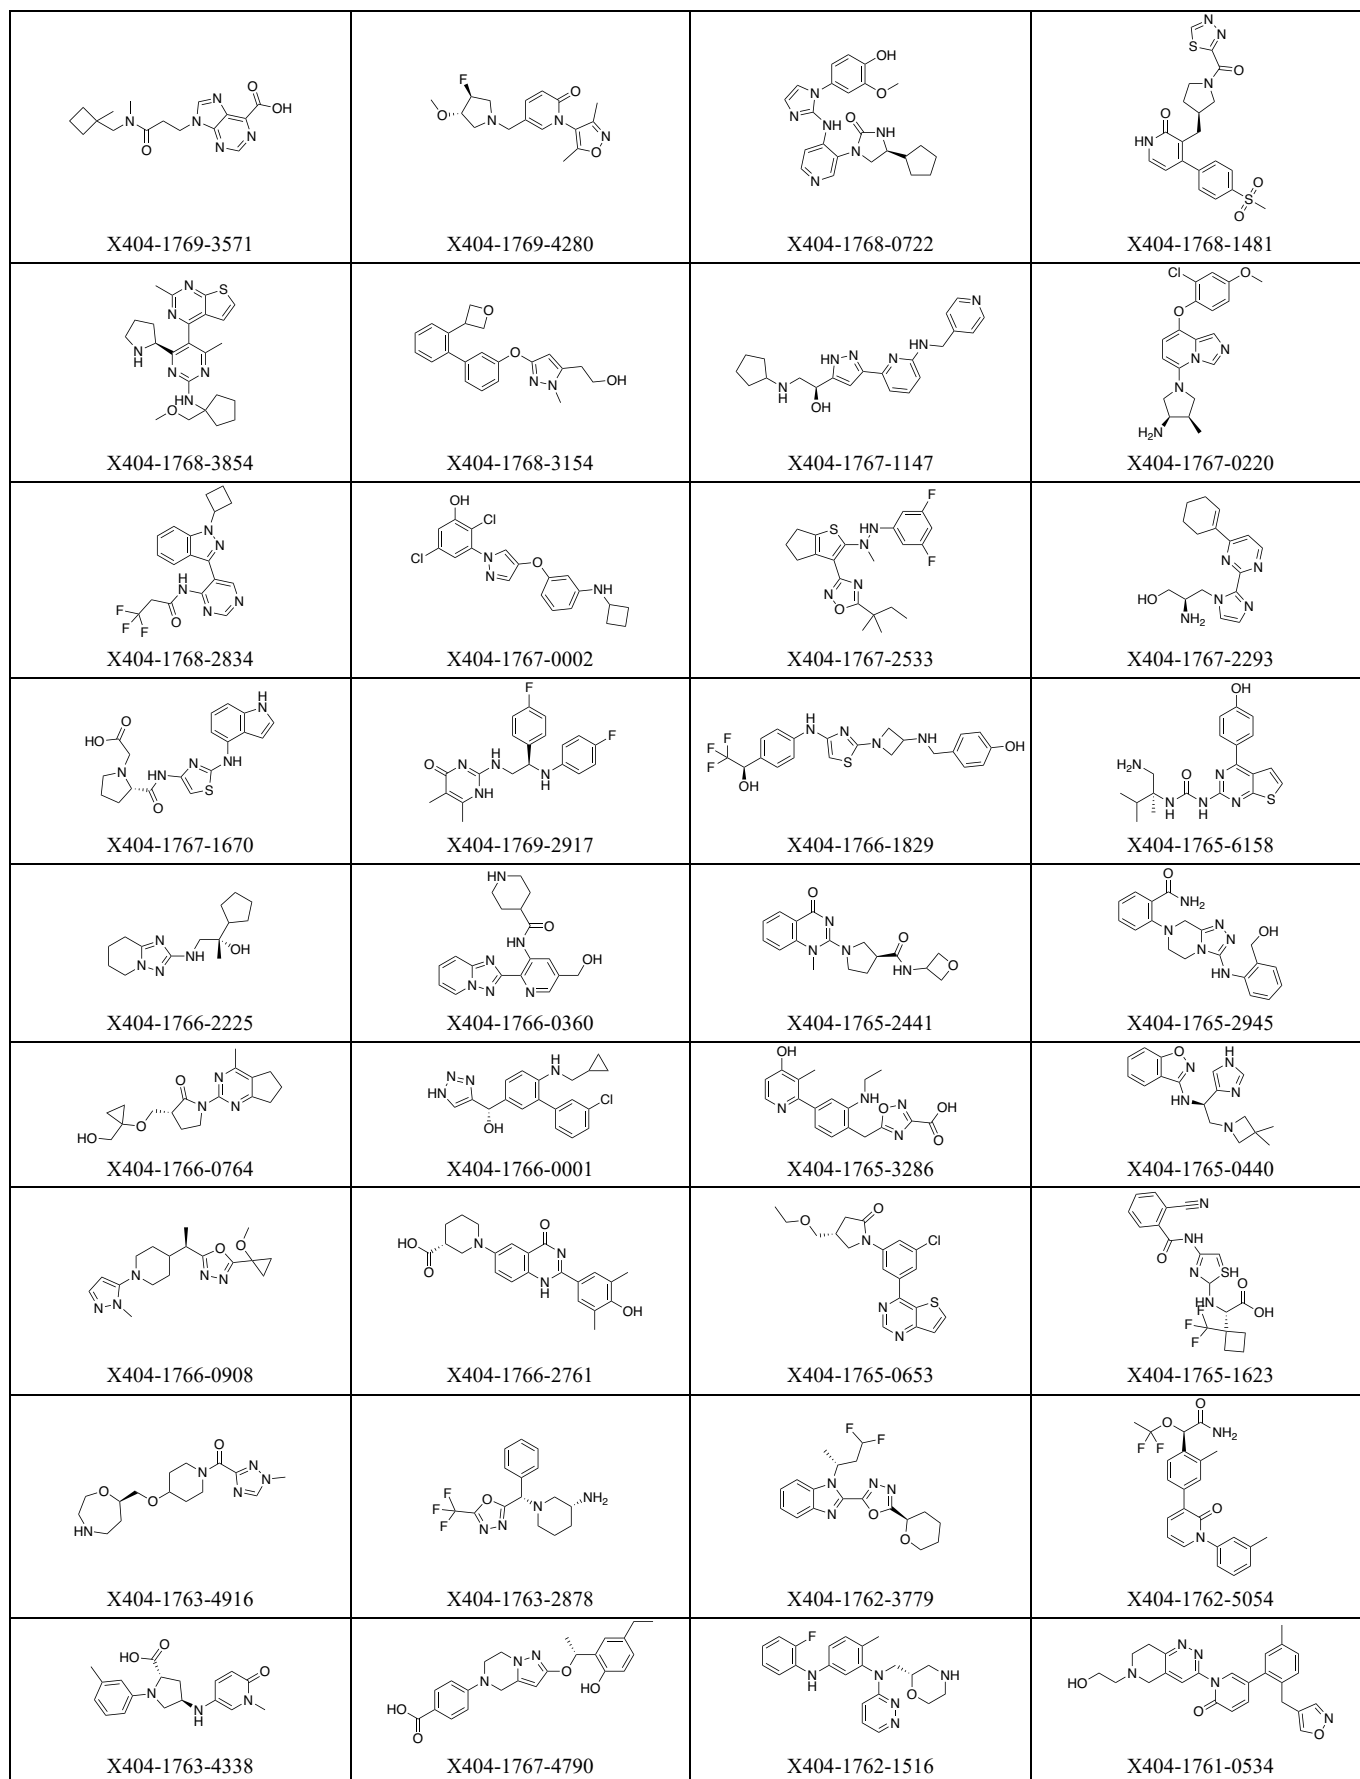   | 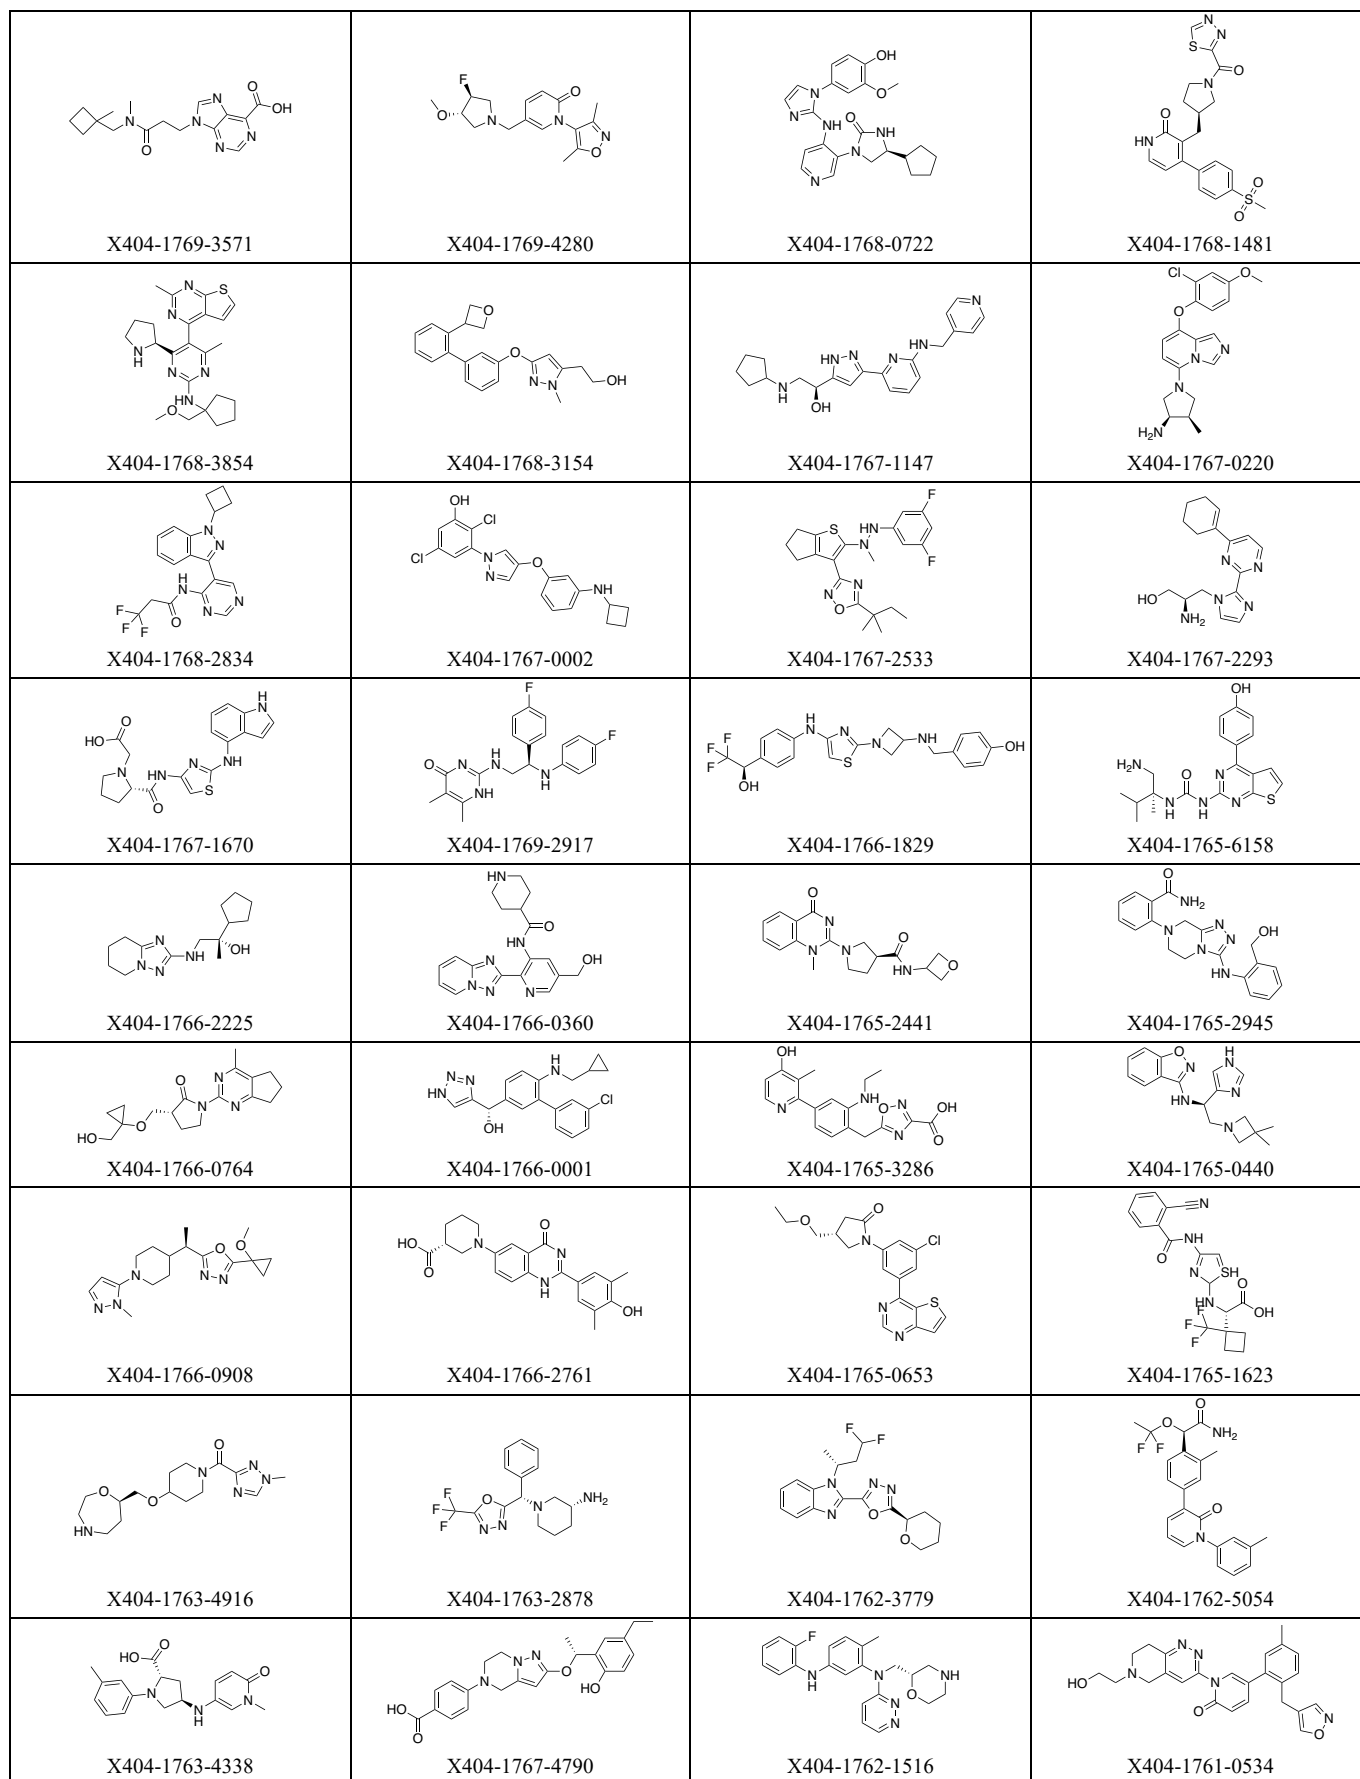   |
| 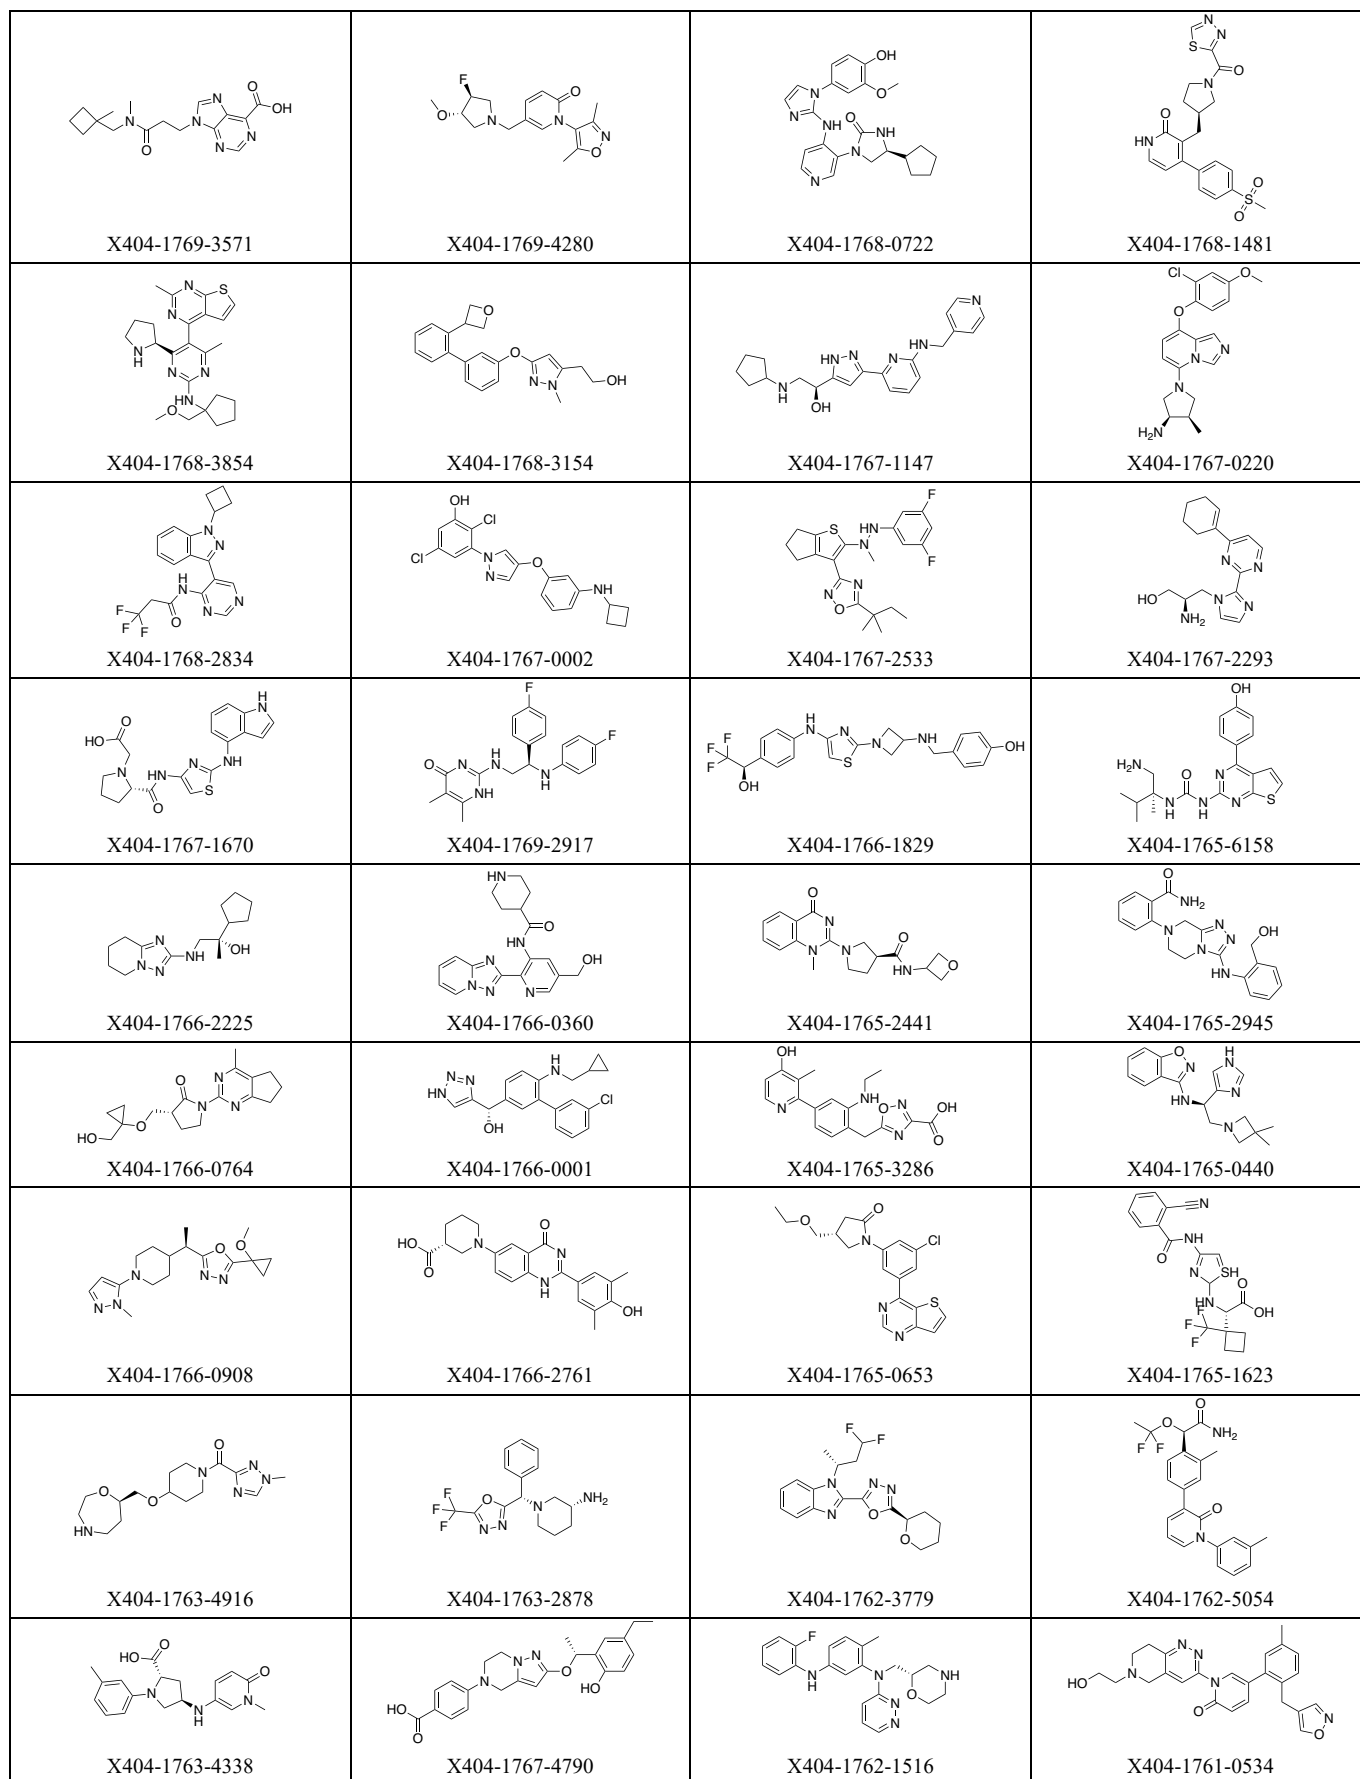   | 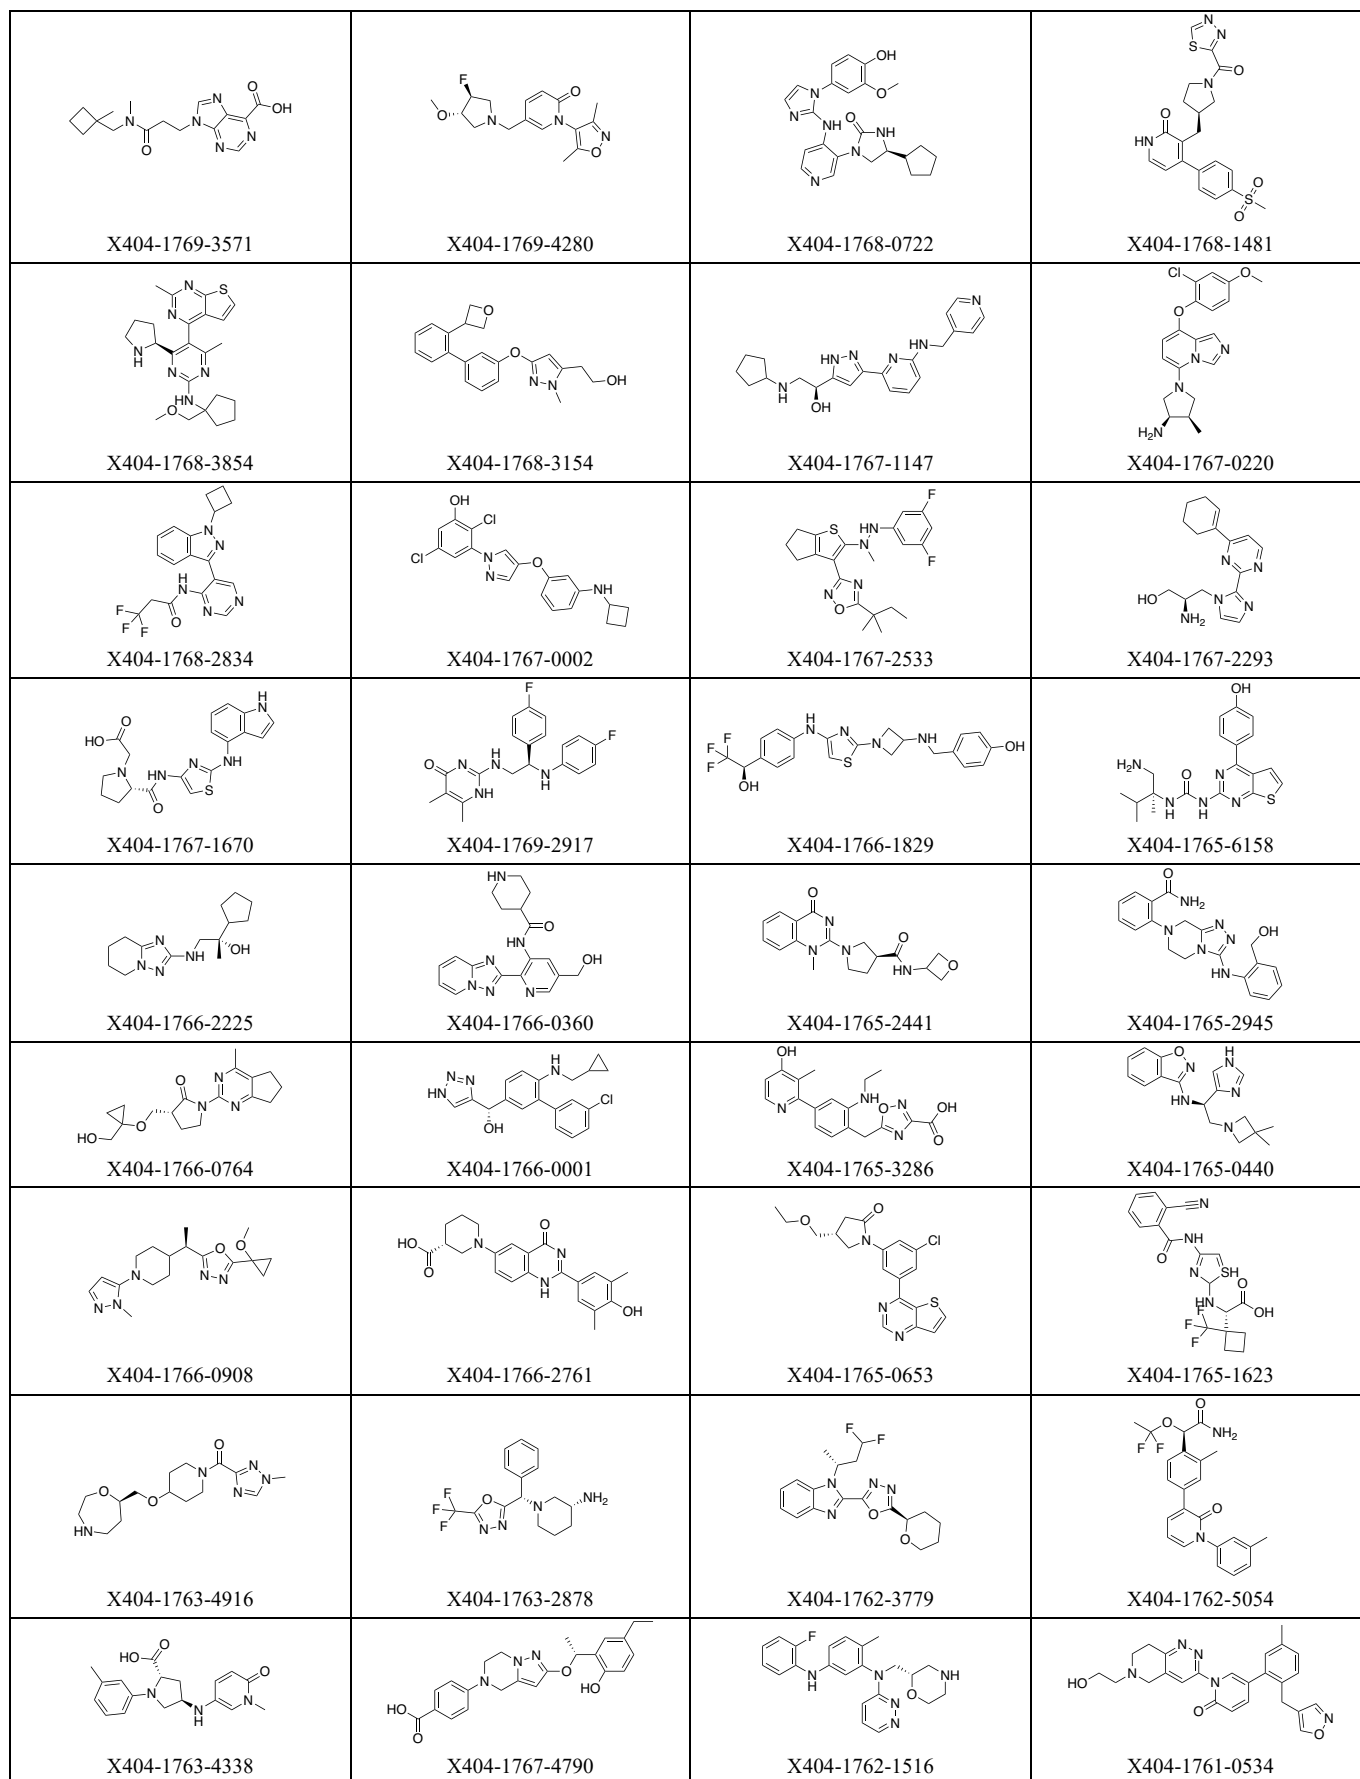   | 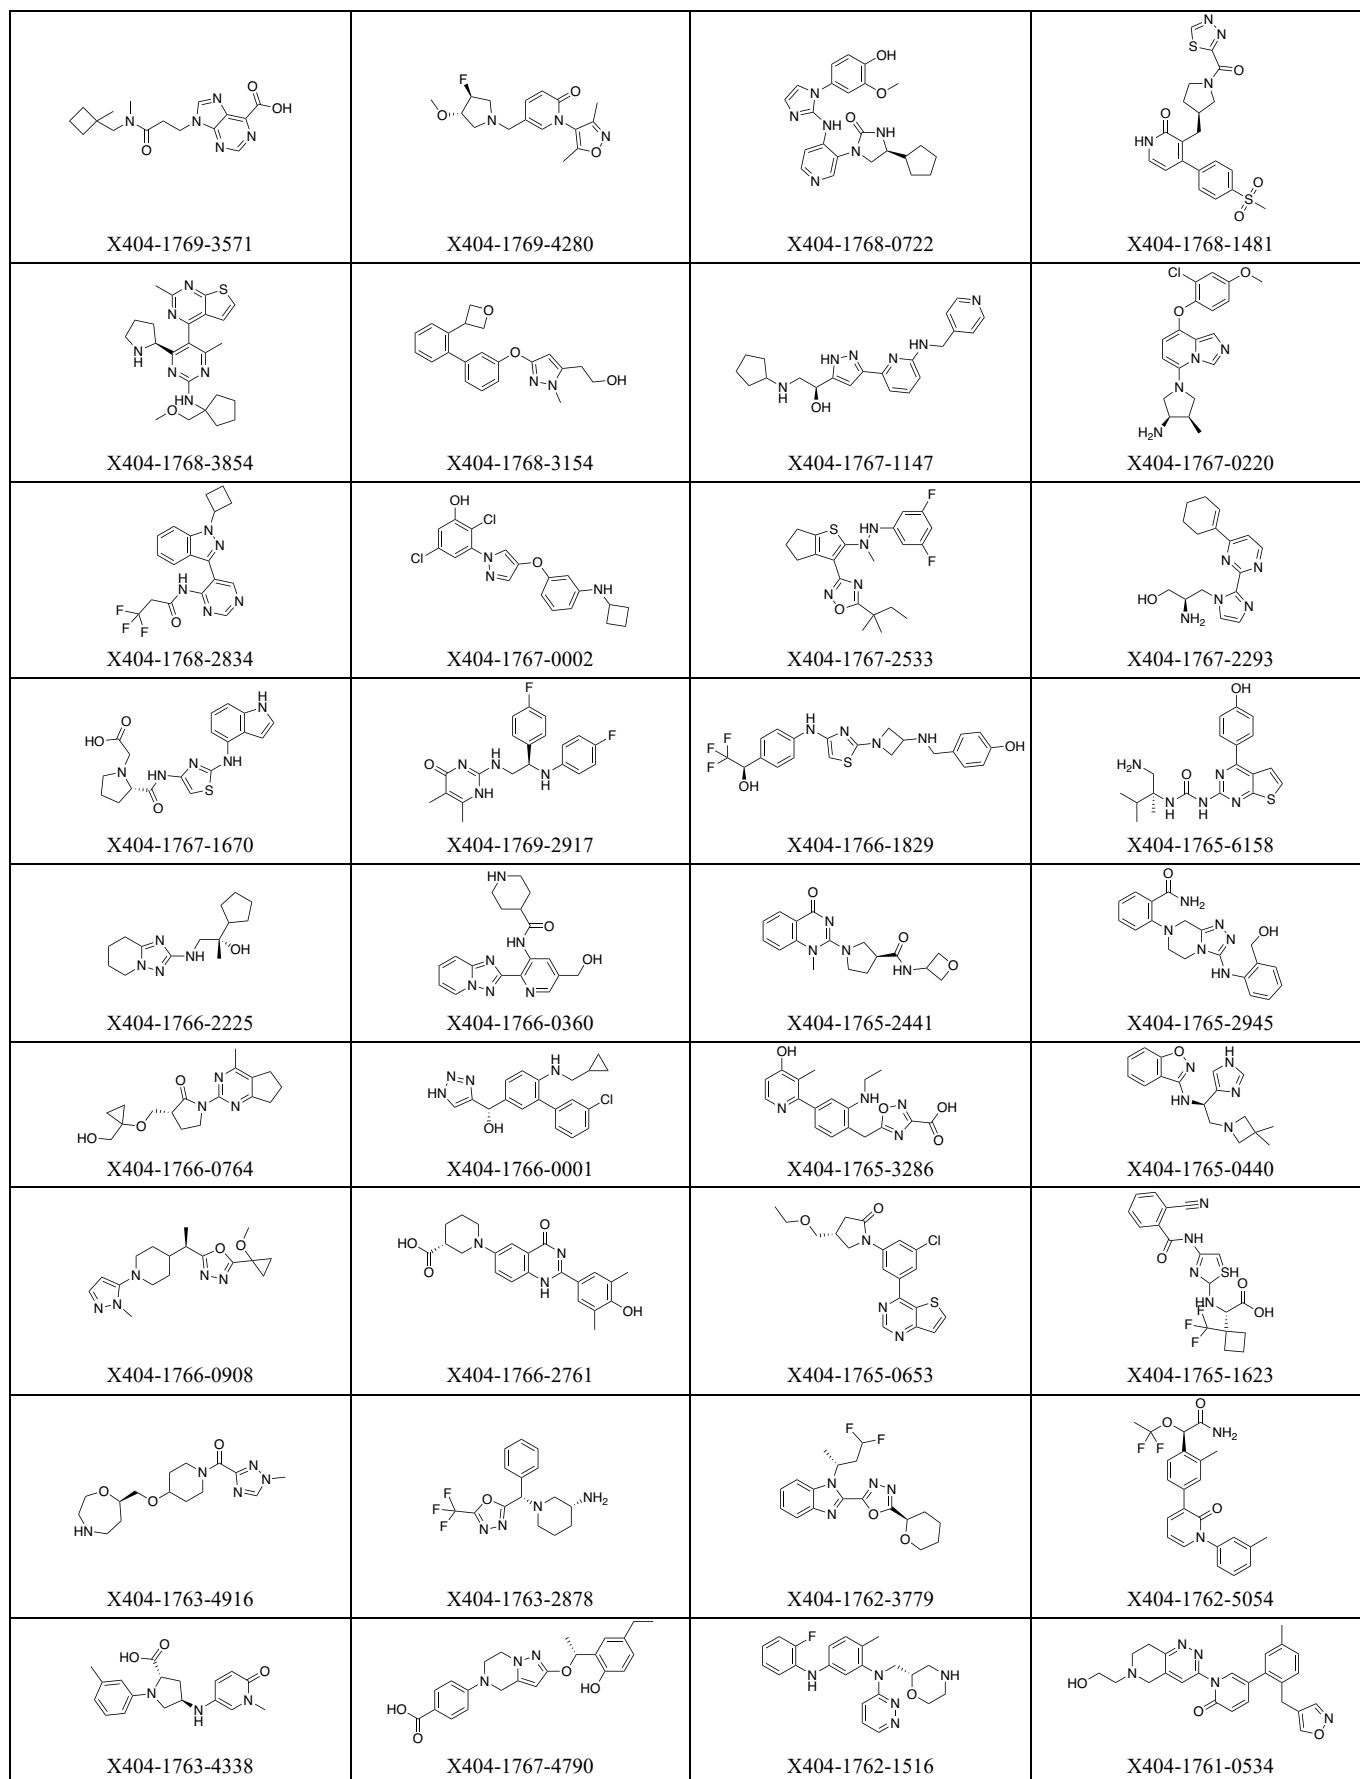   | 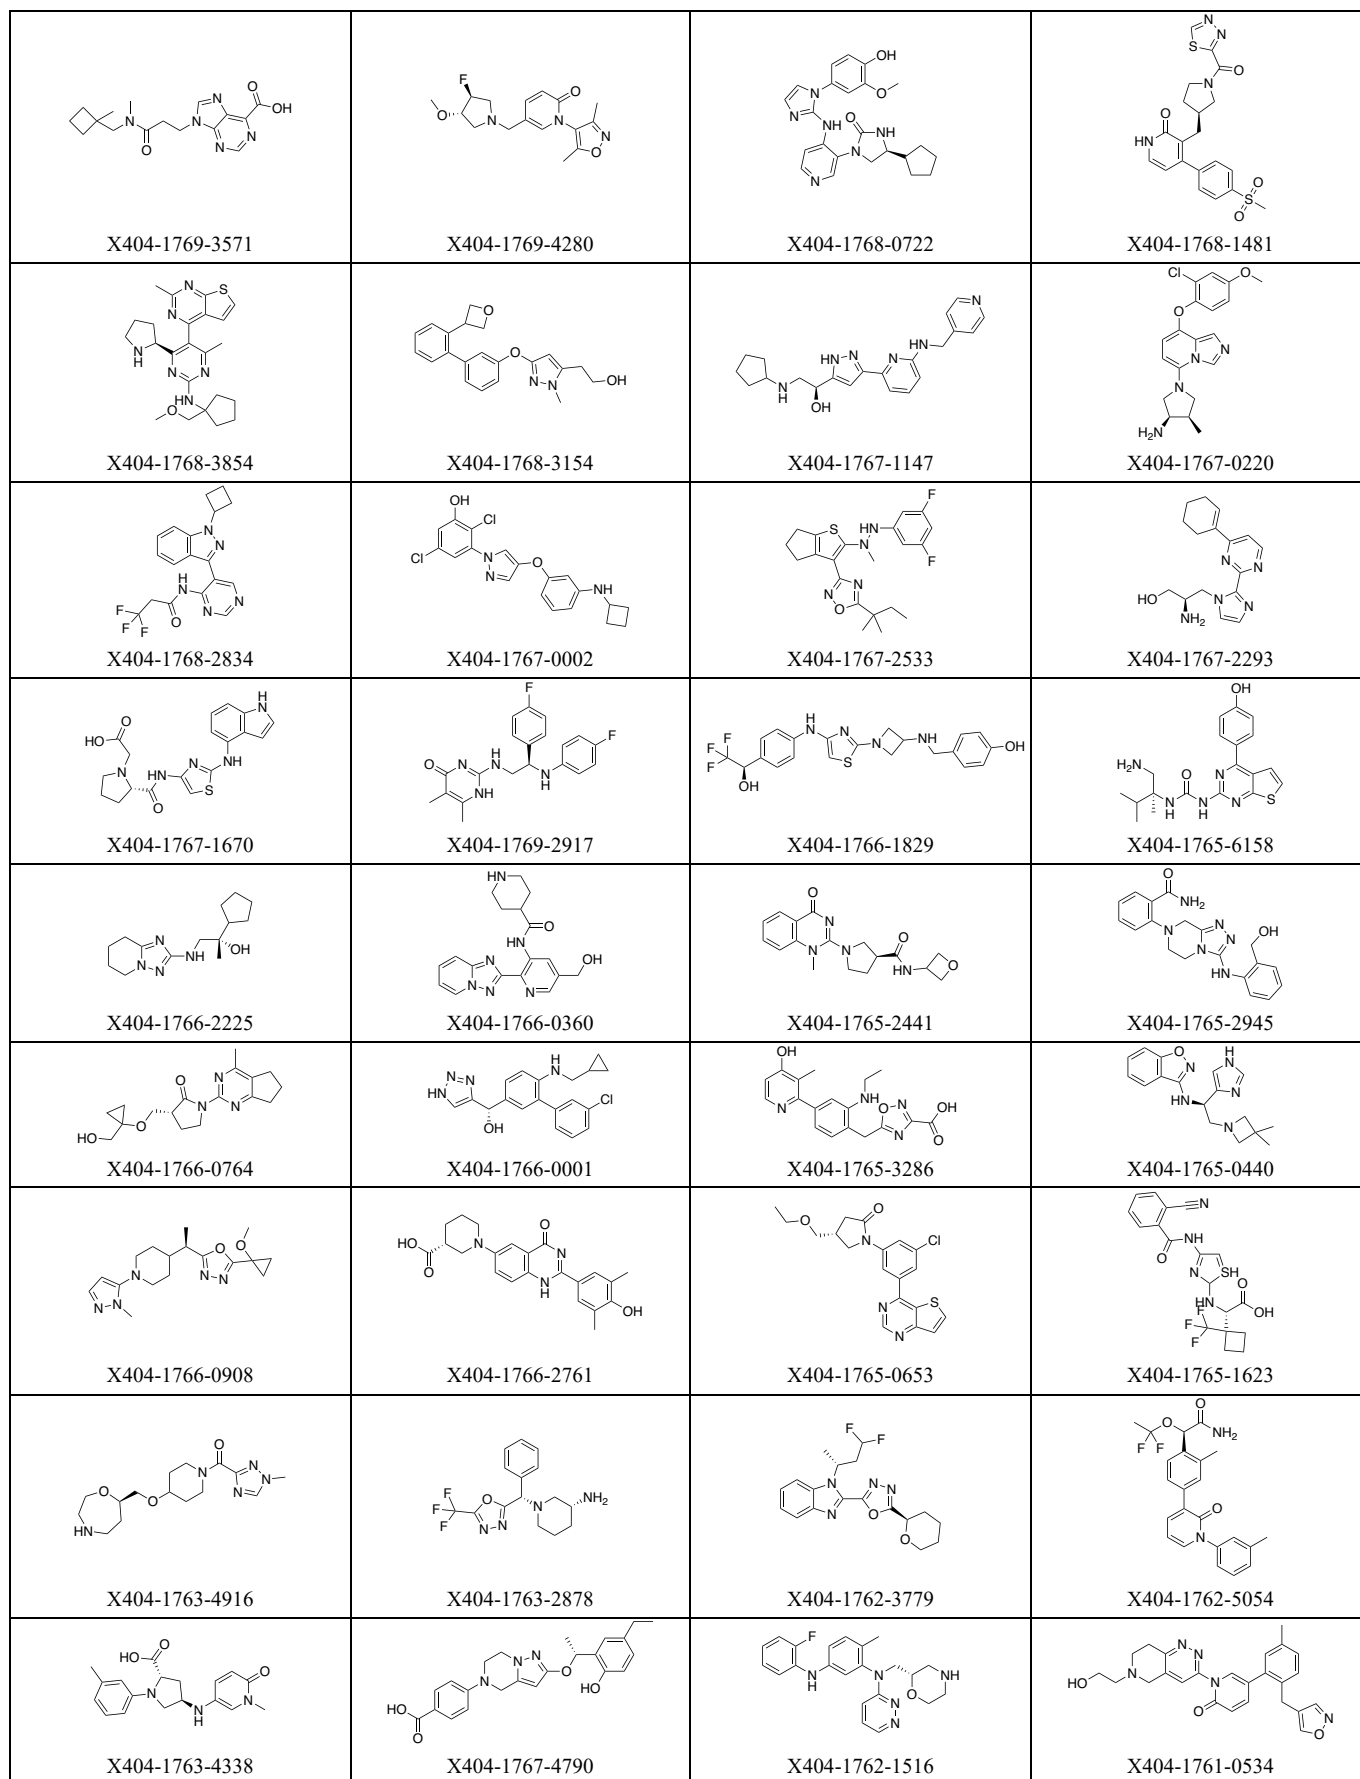   |
| 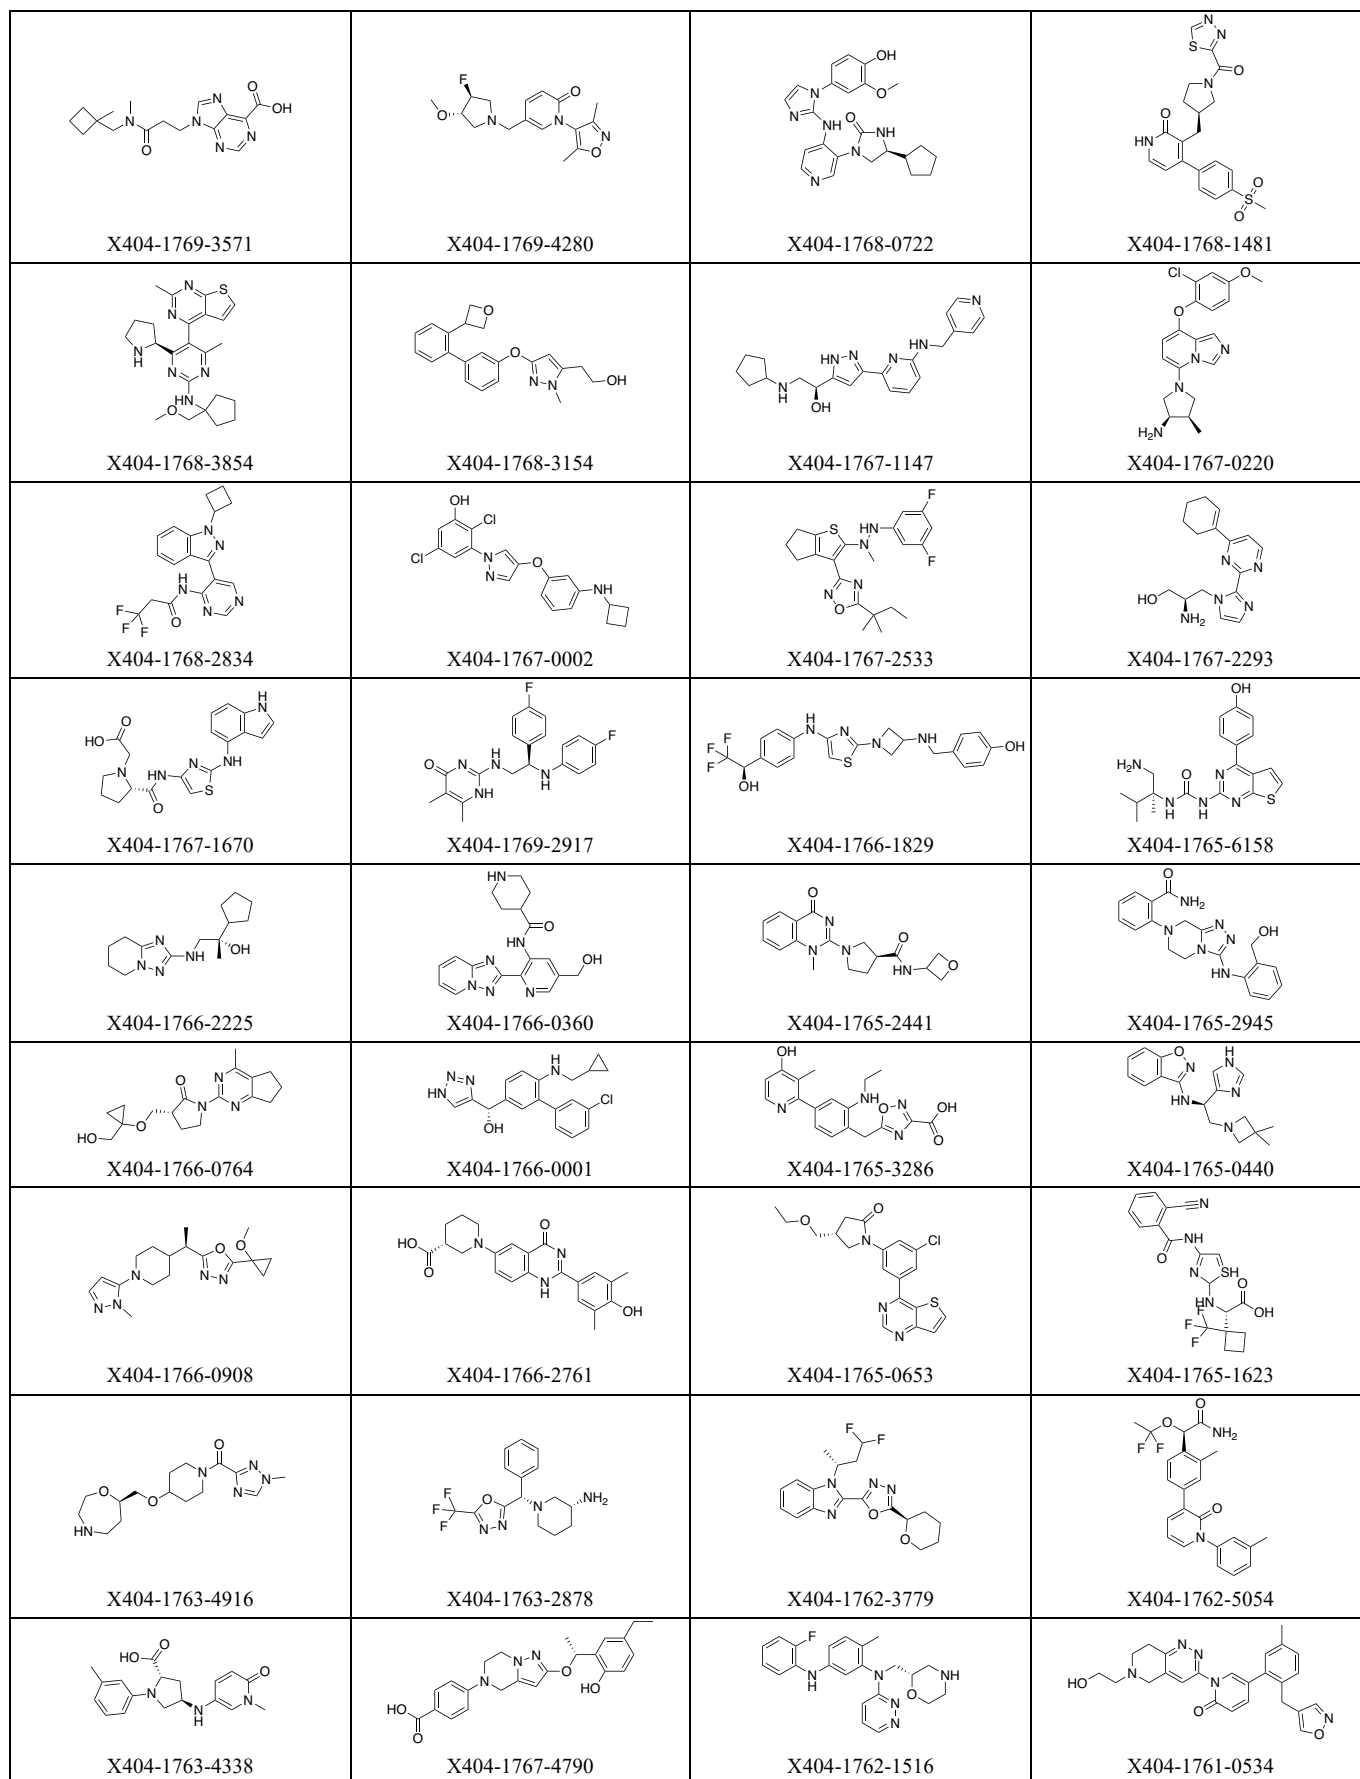   | 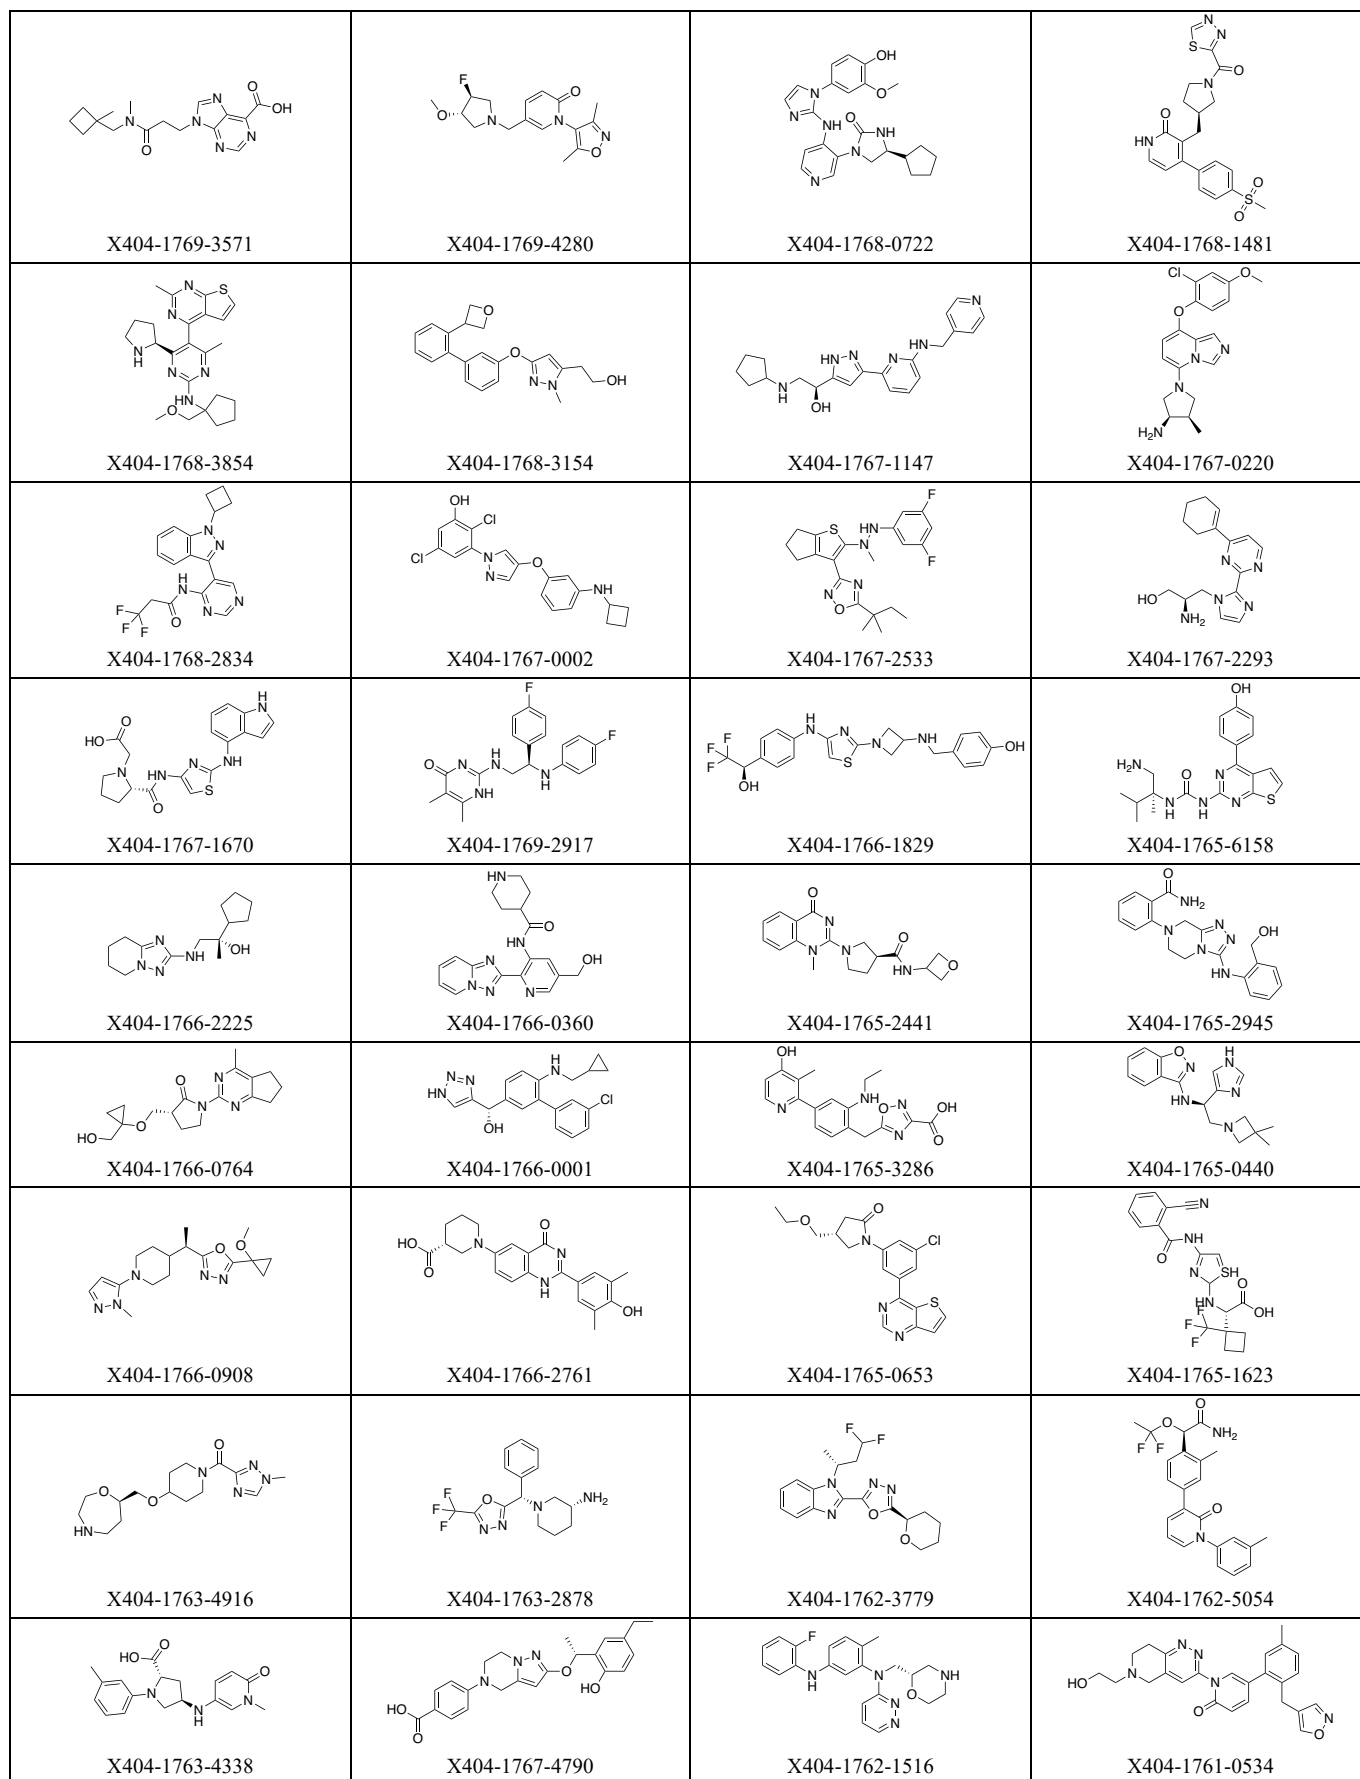   | 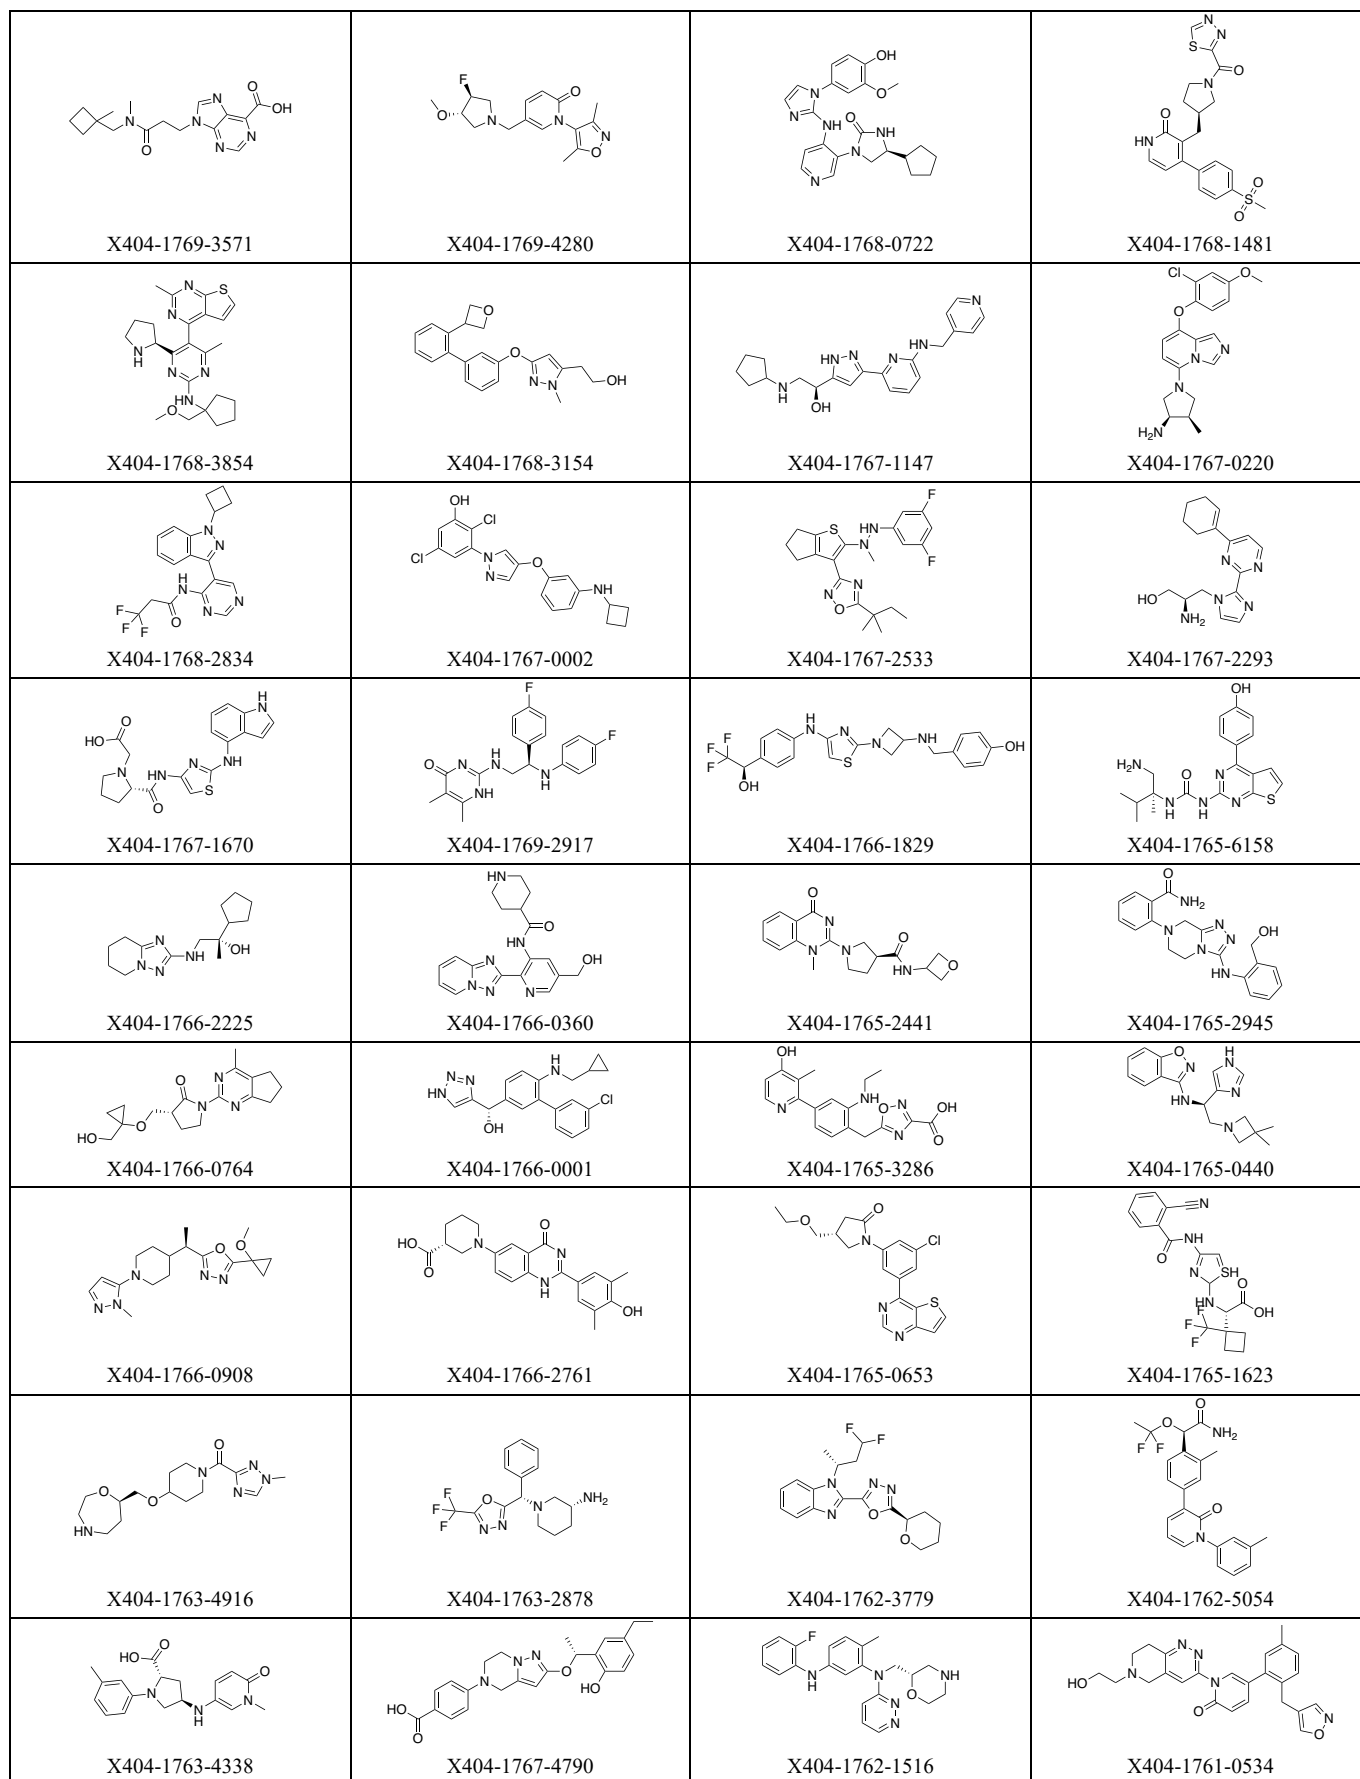   | 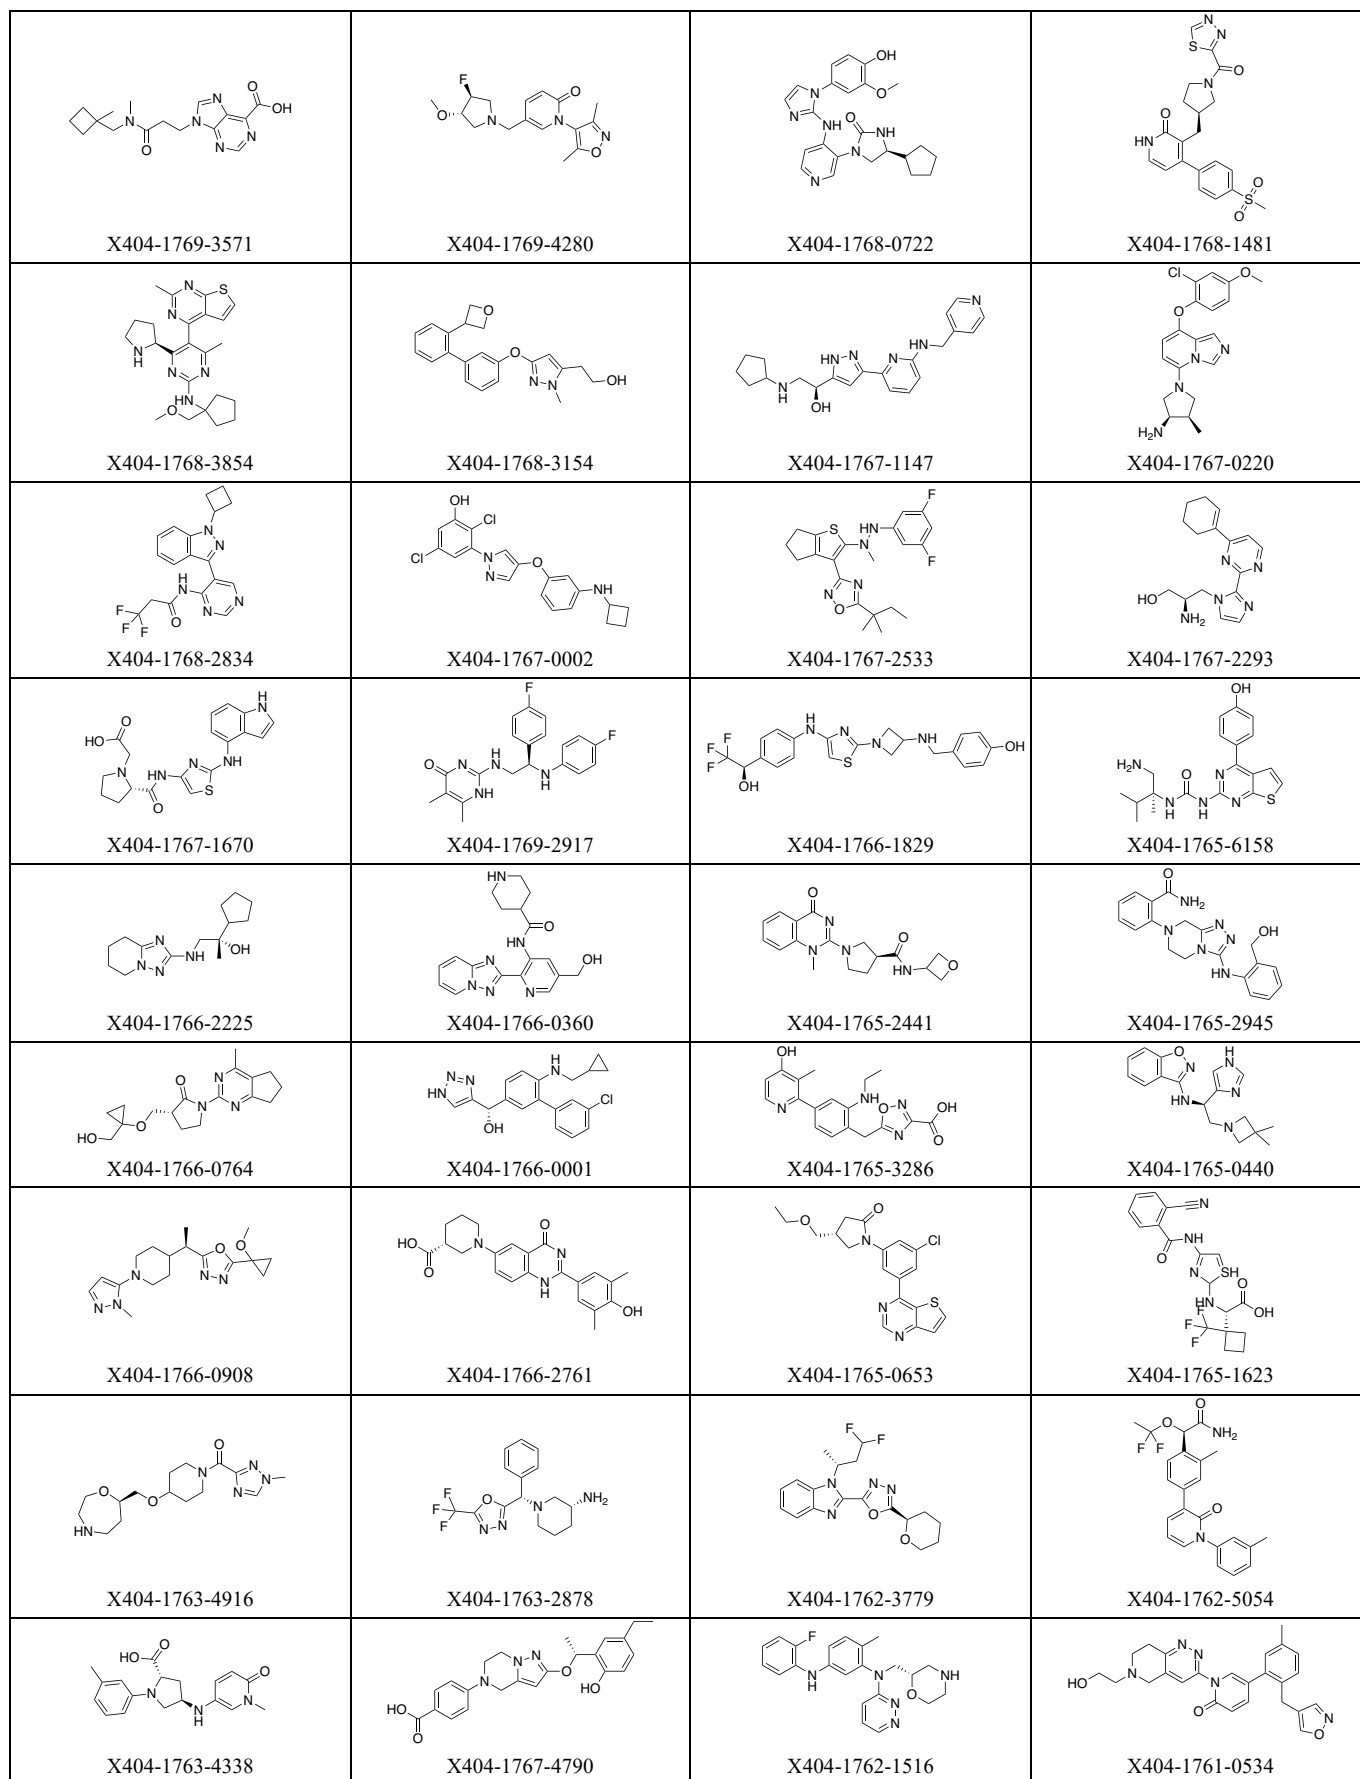   |
| 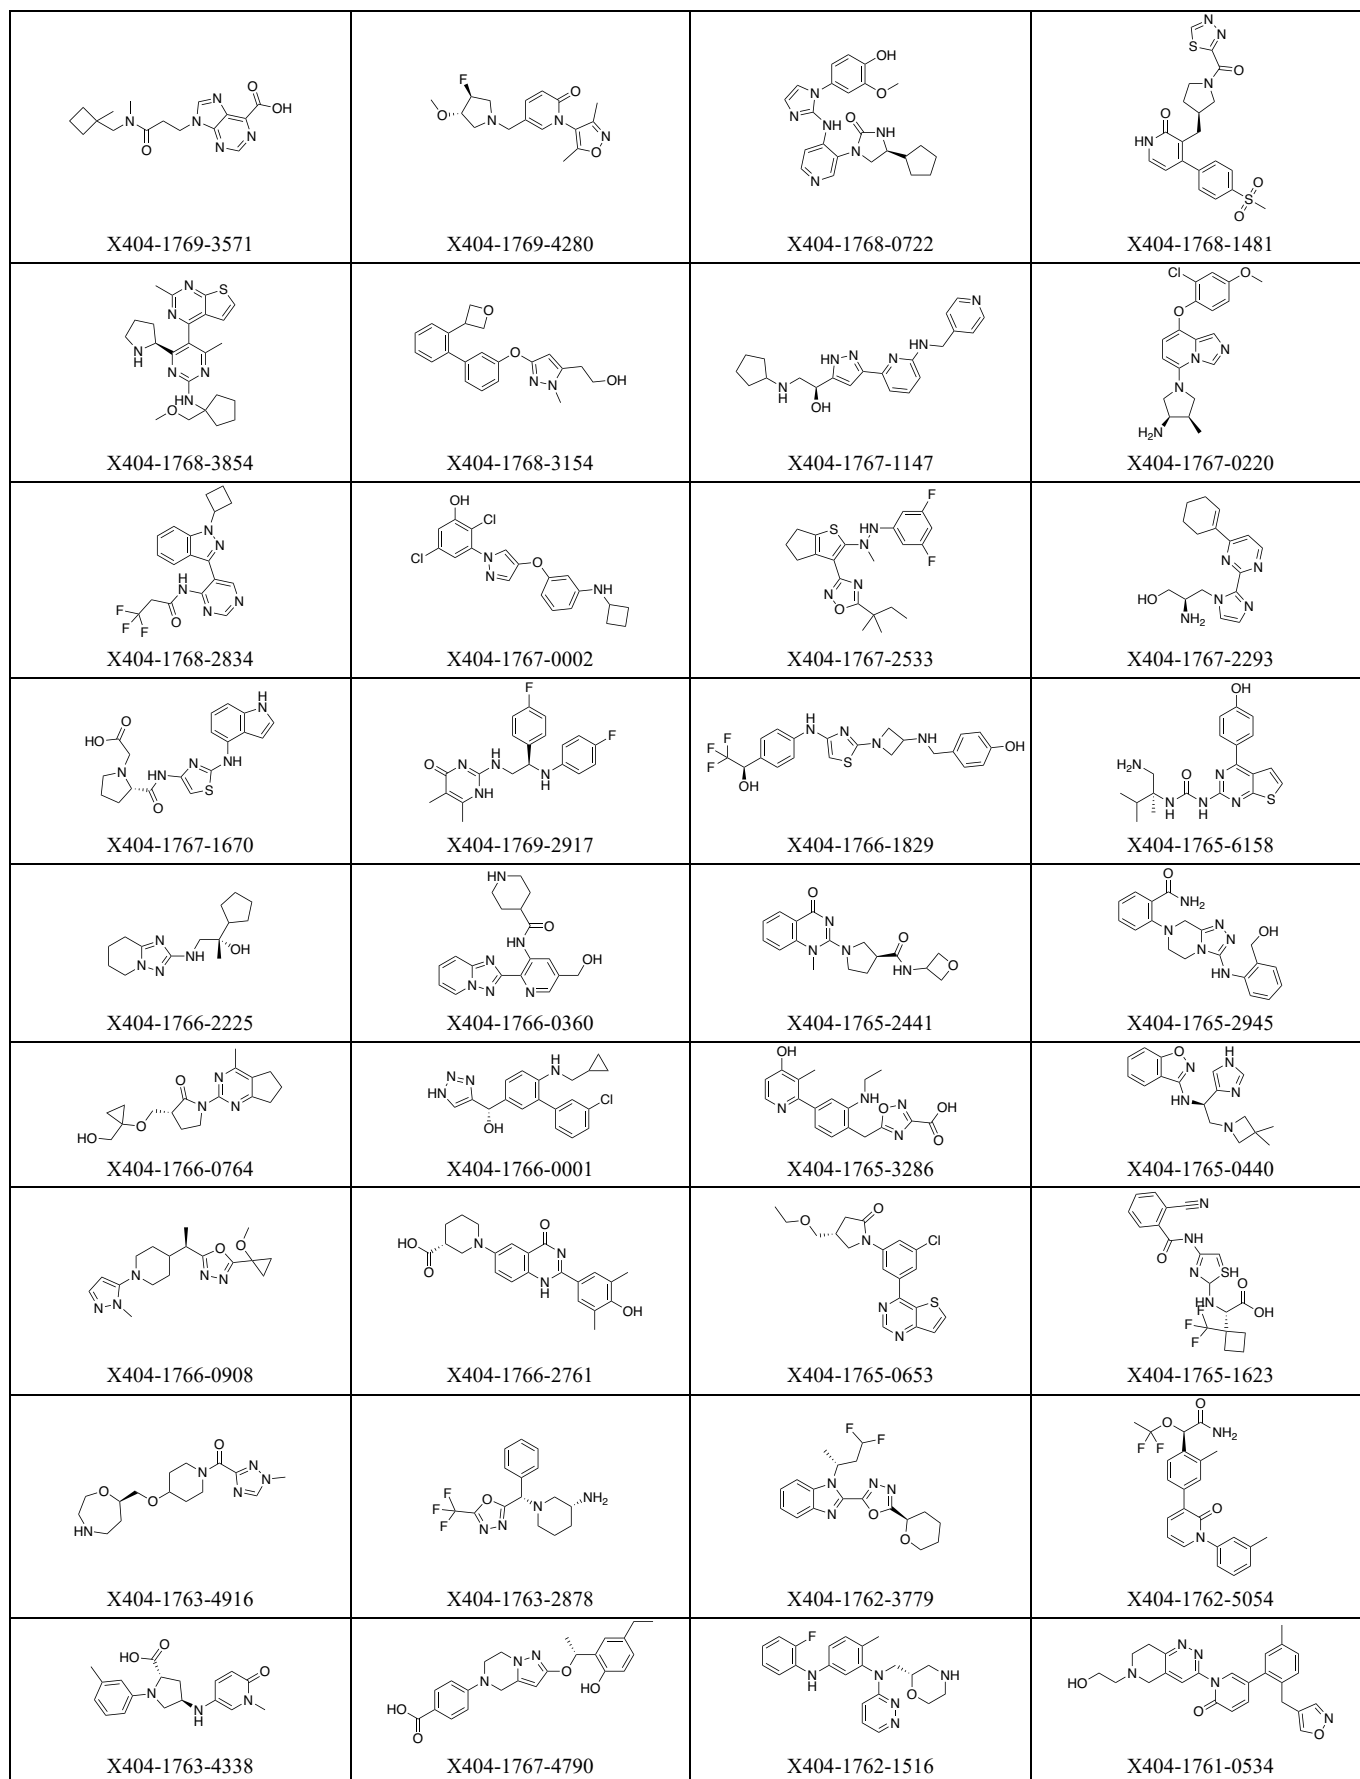   | 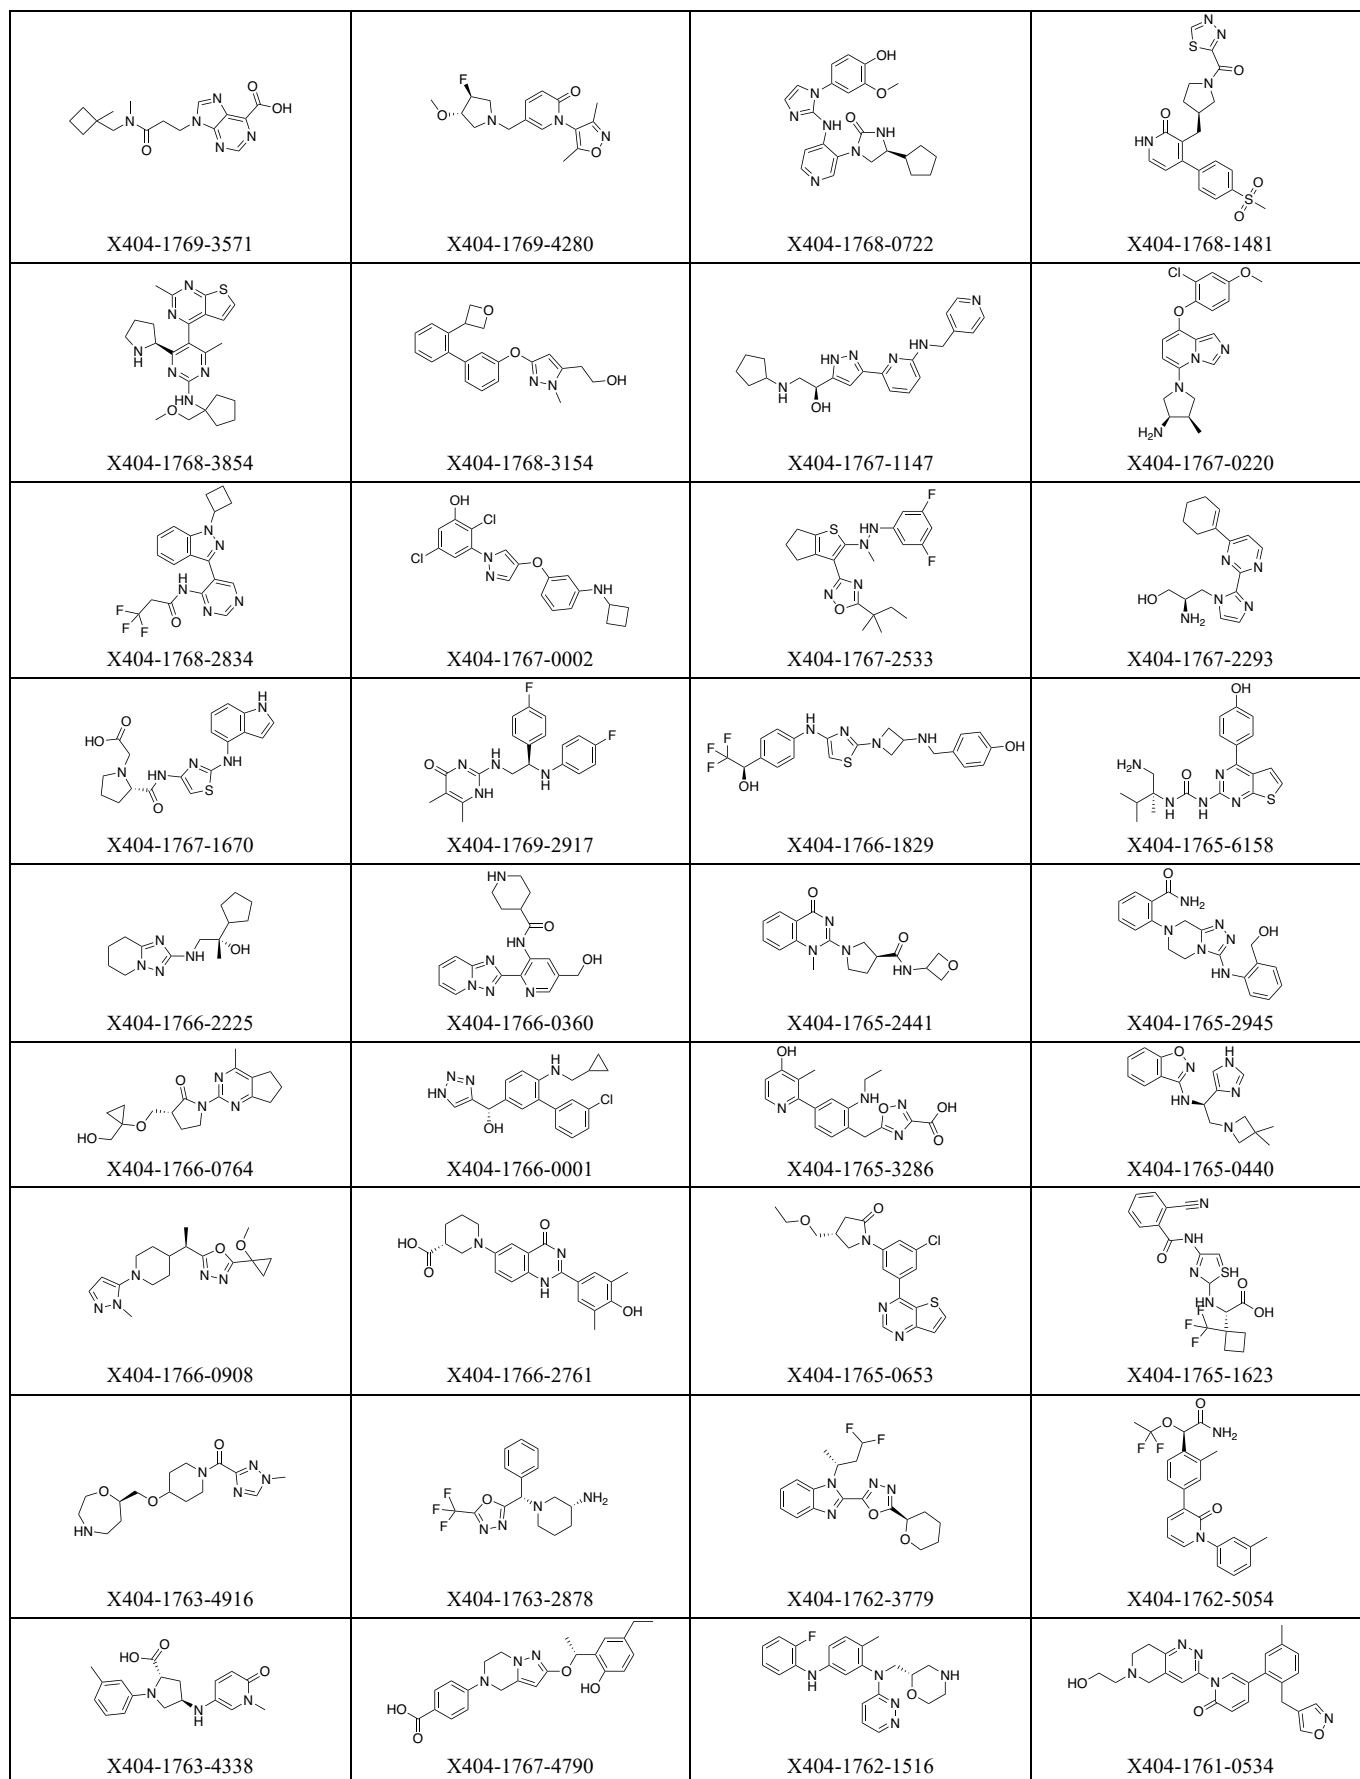   | 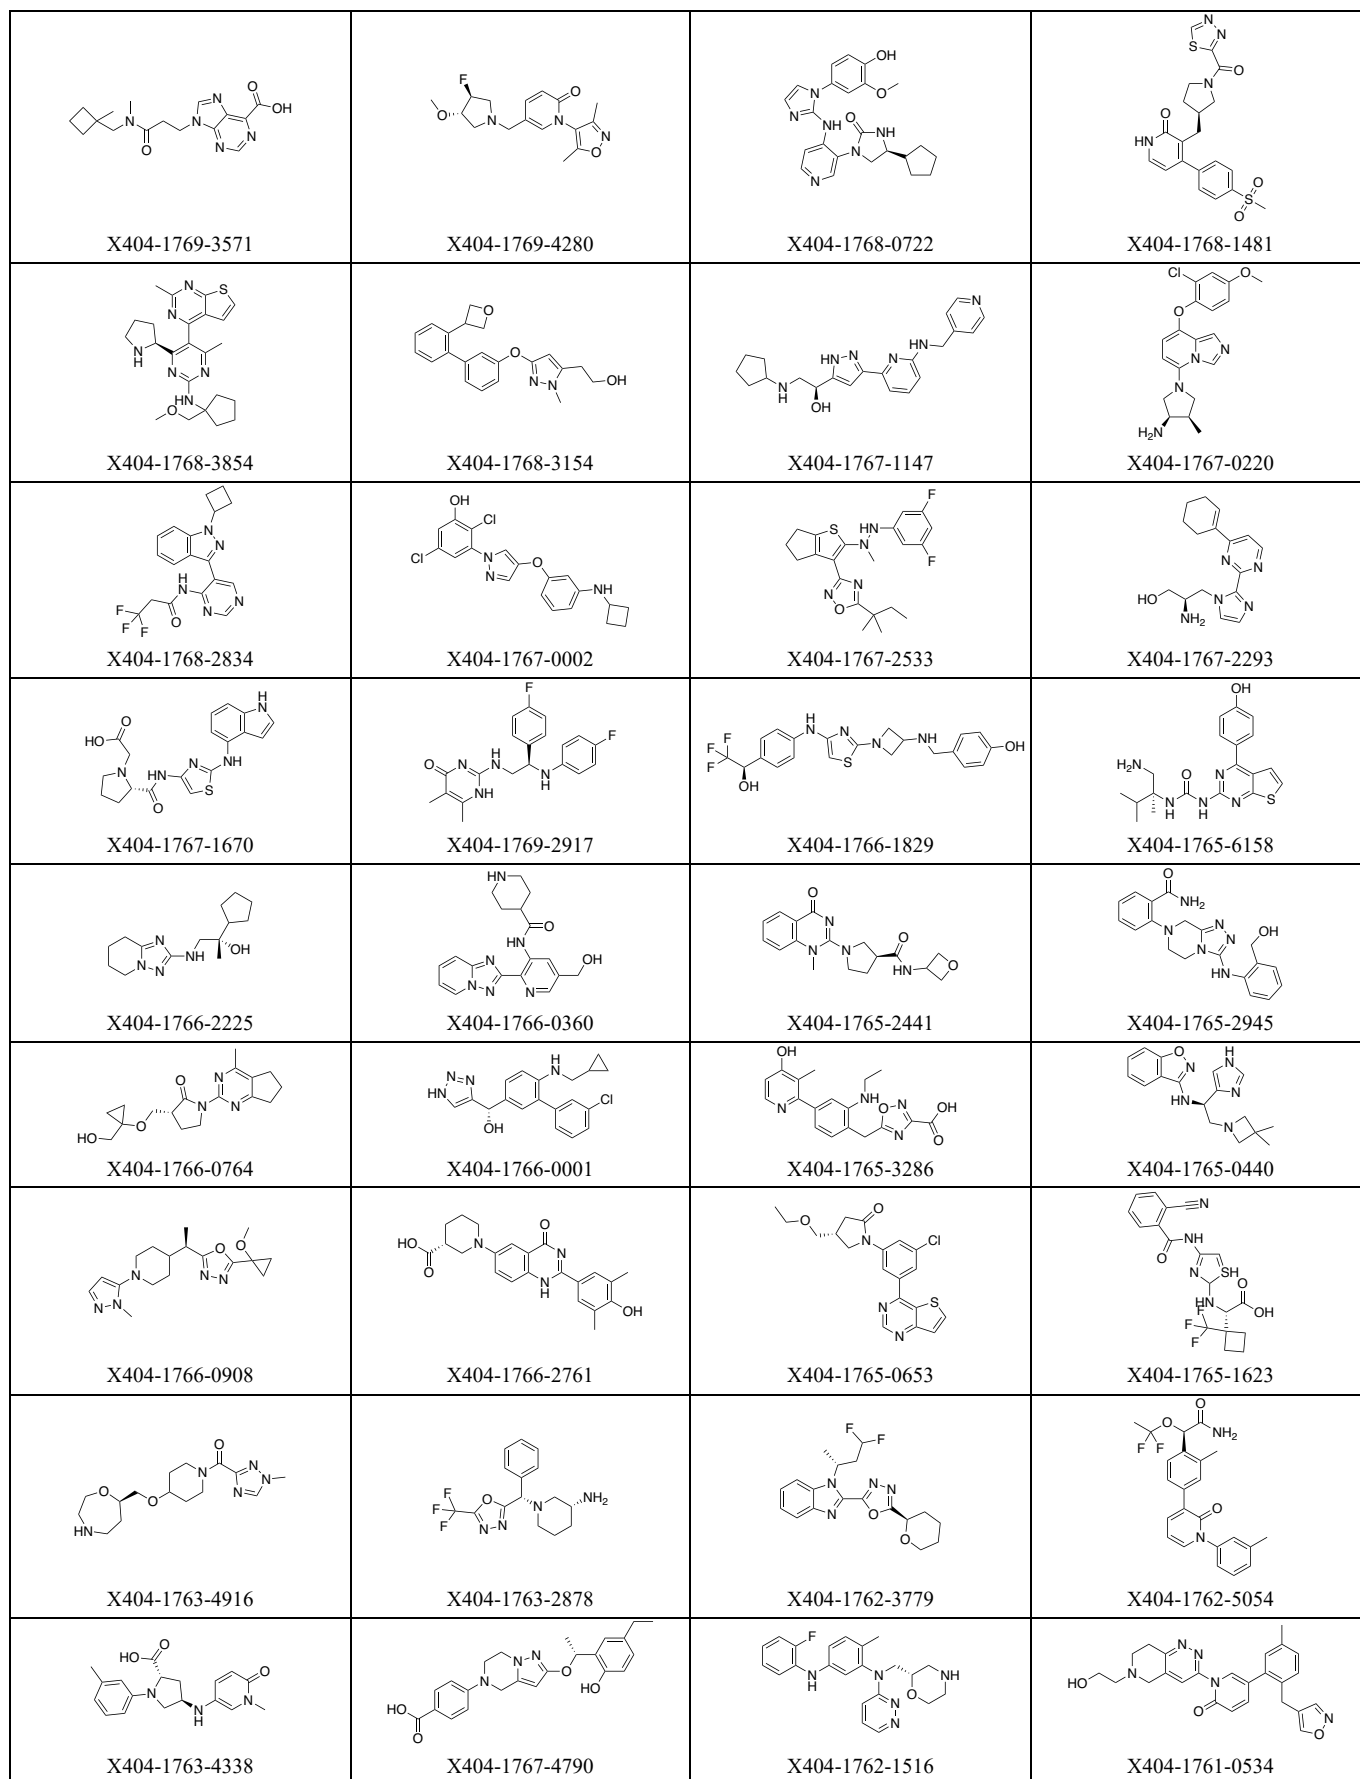   | 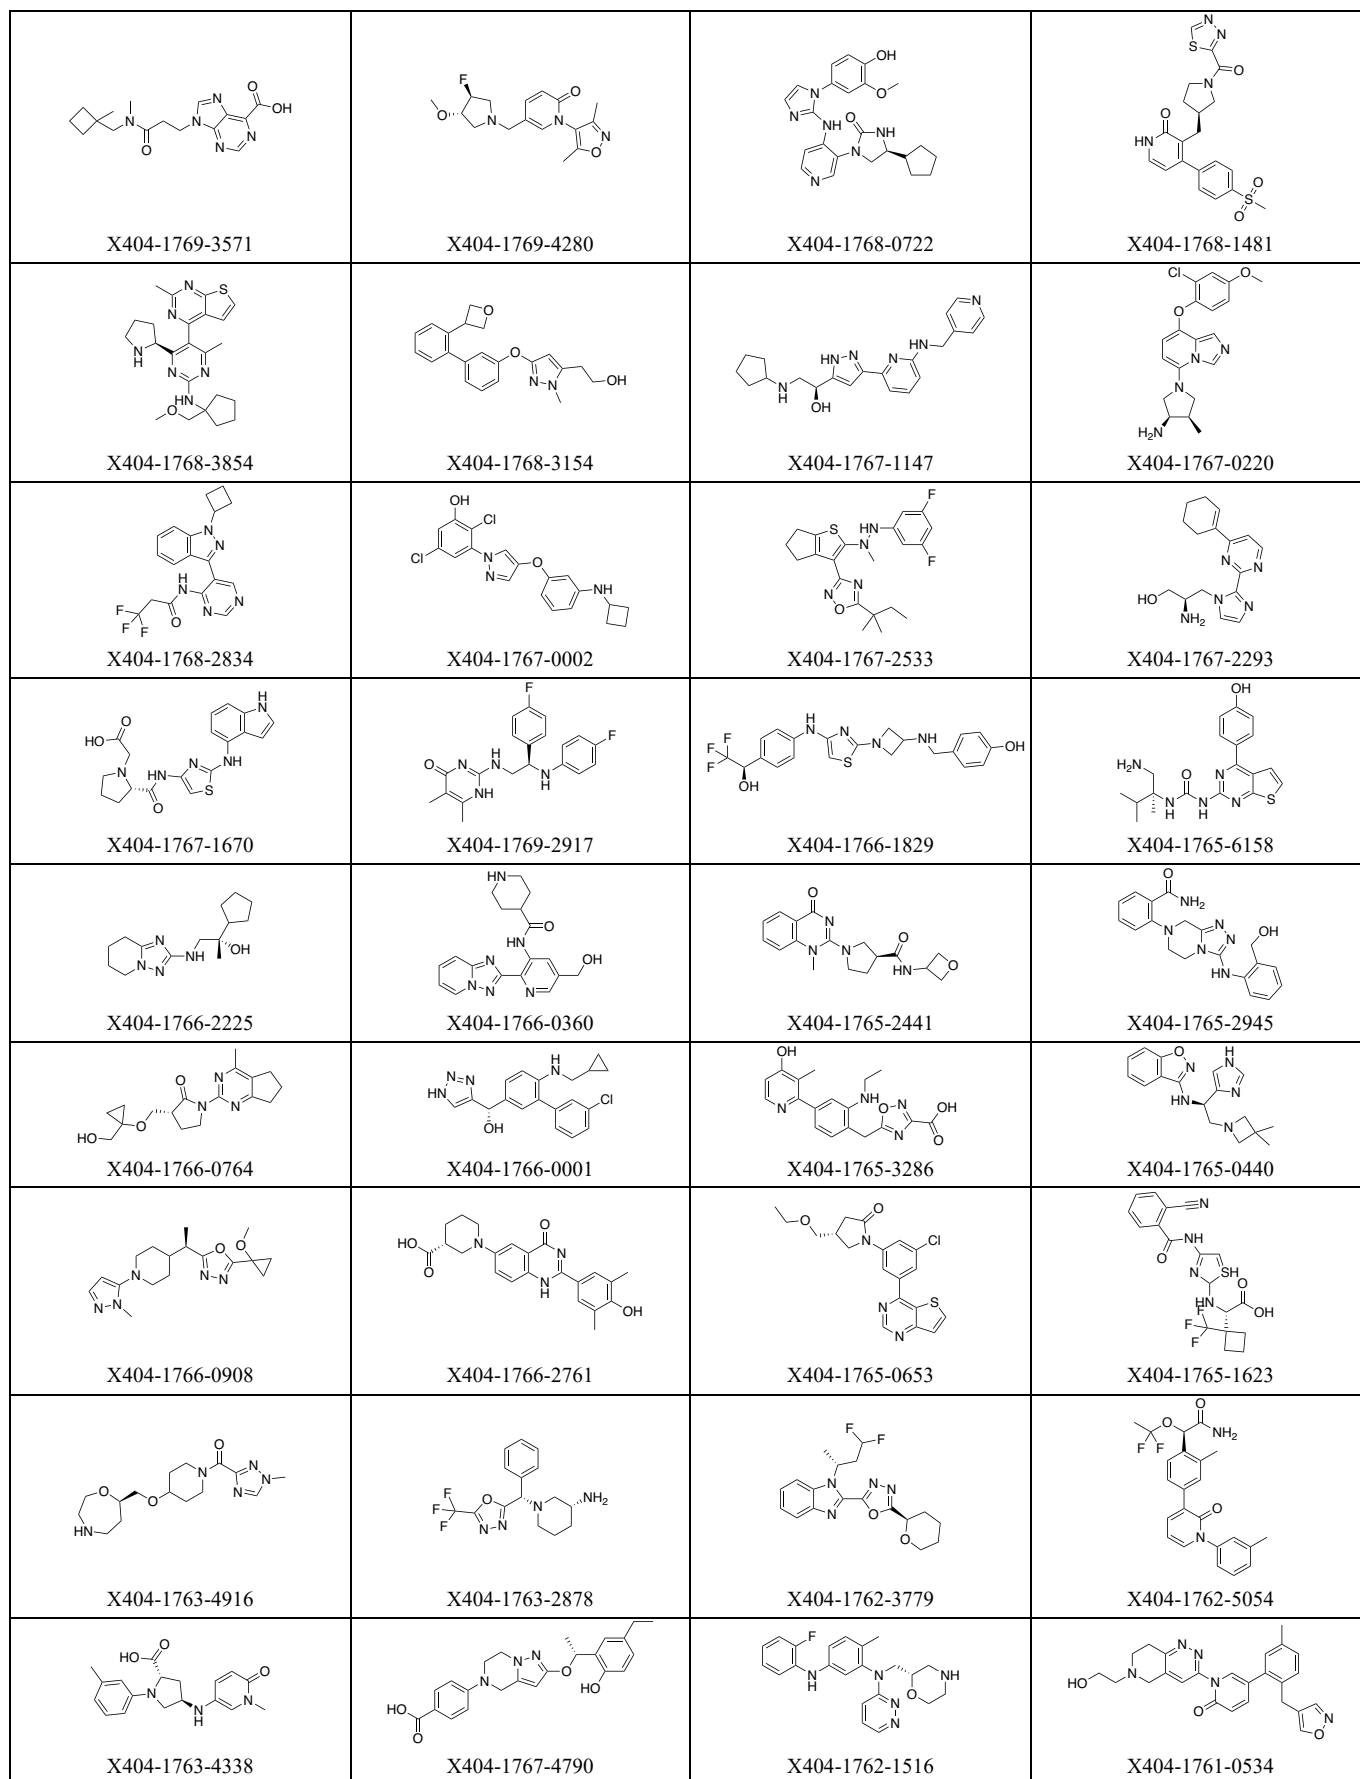   |
| 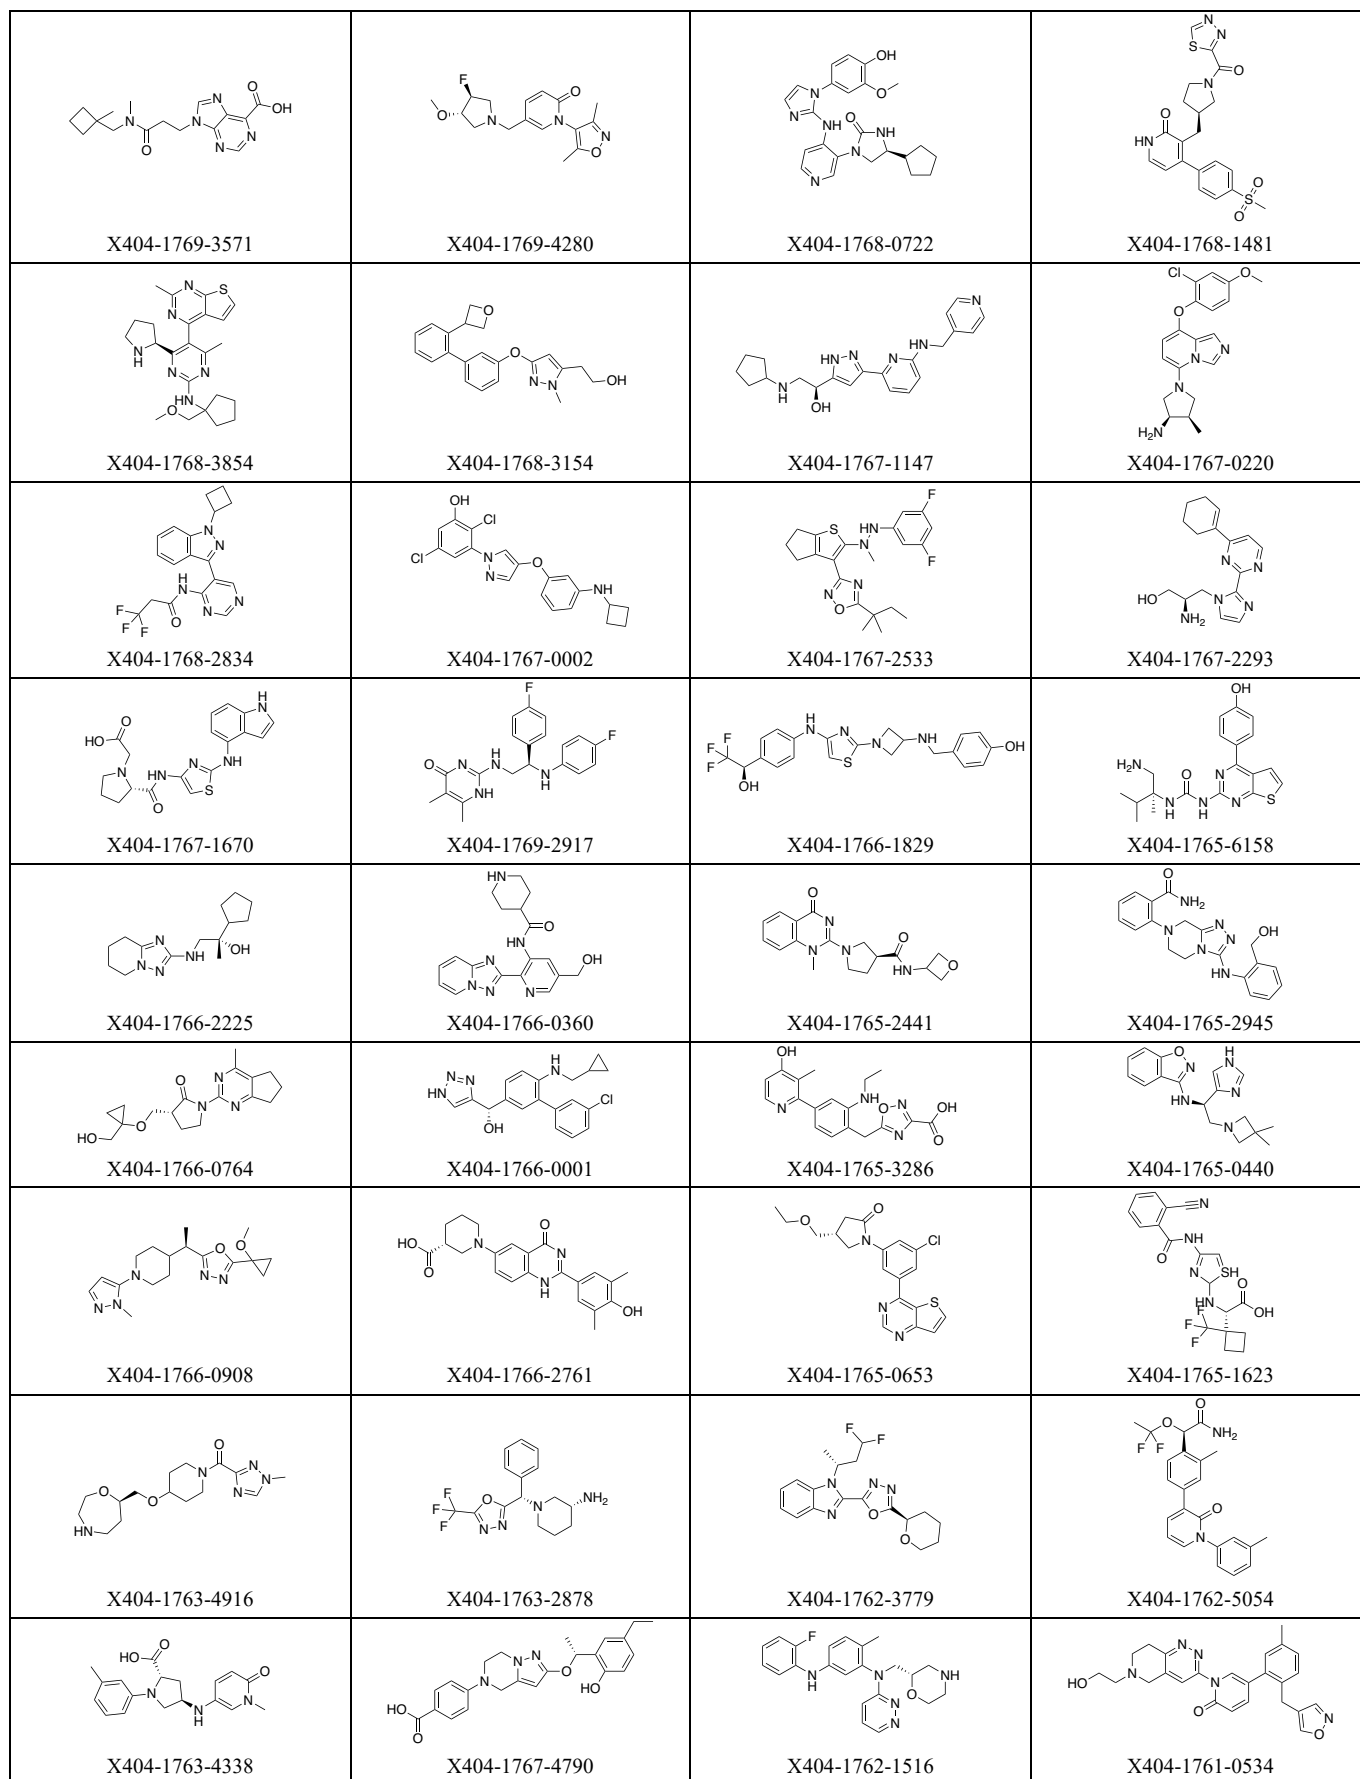 | 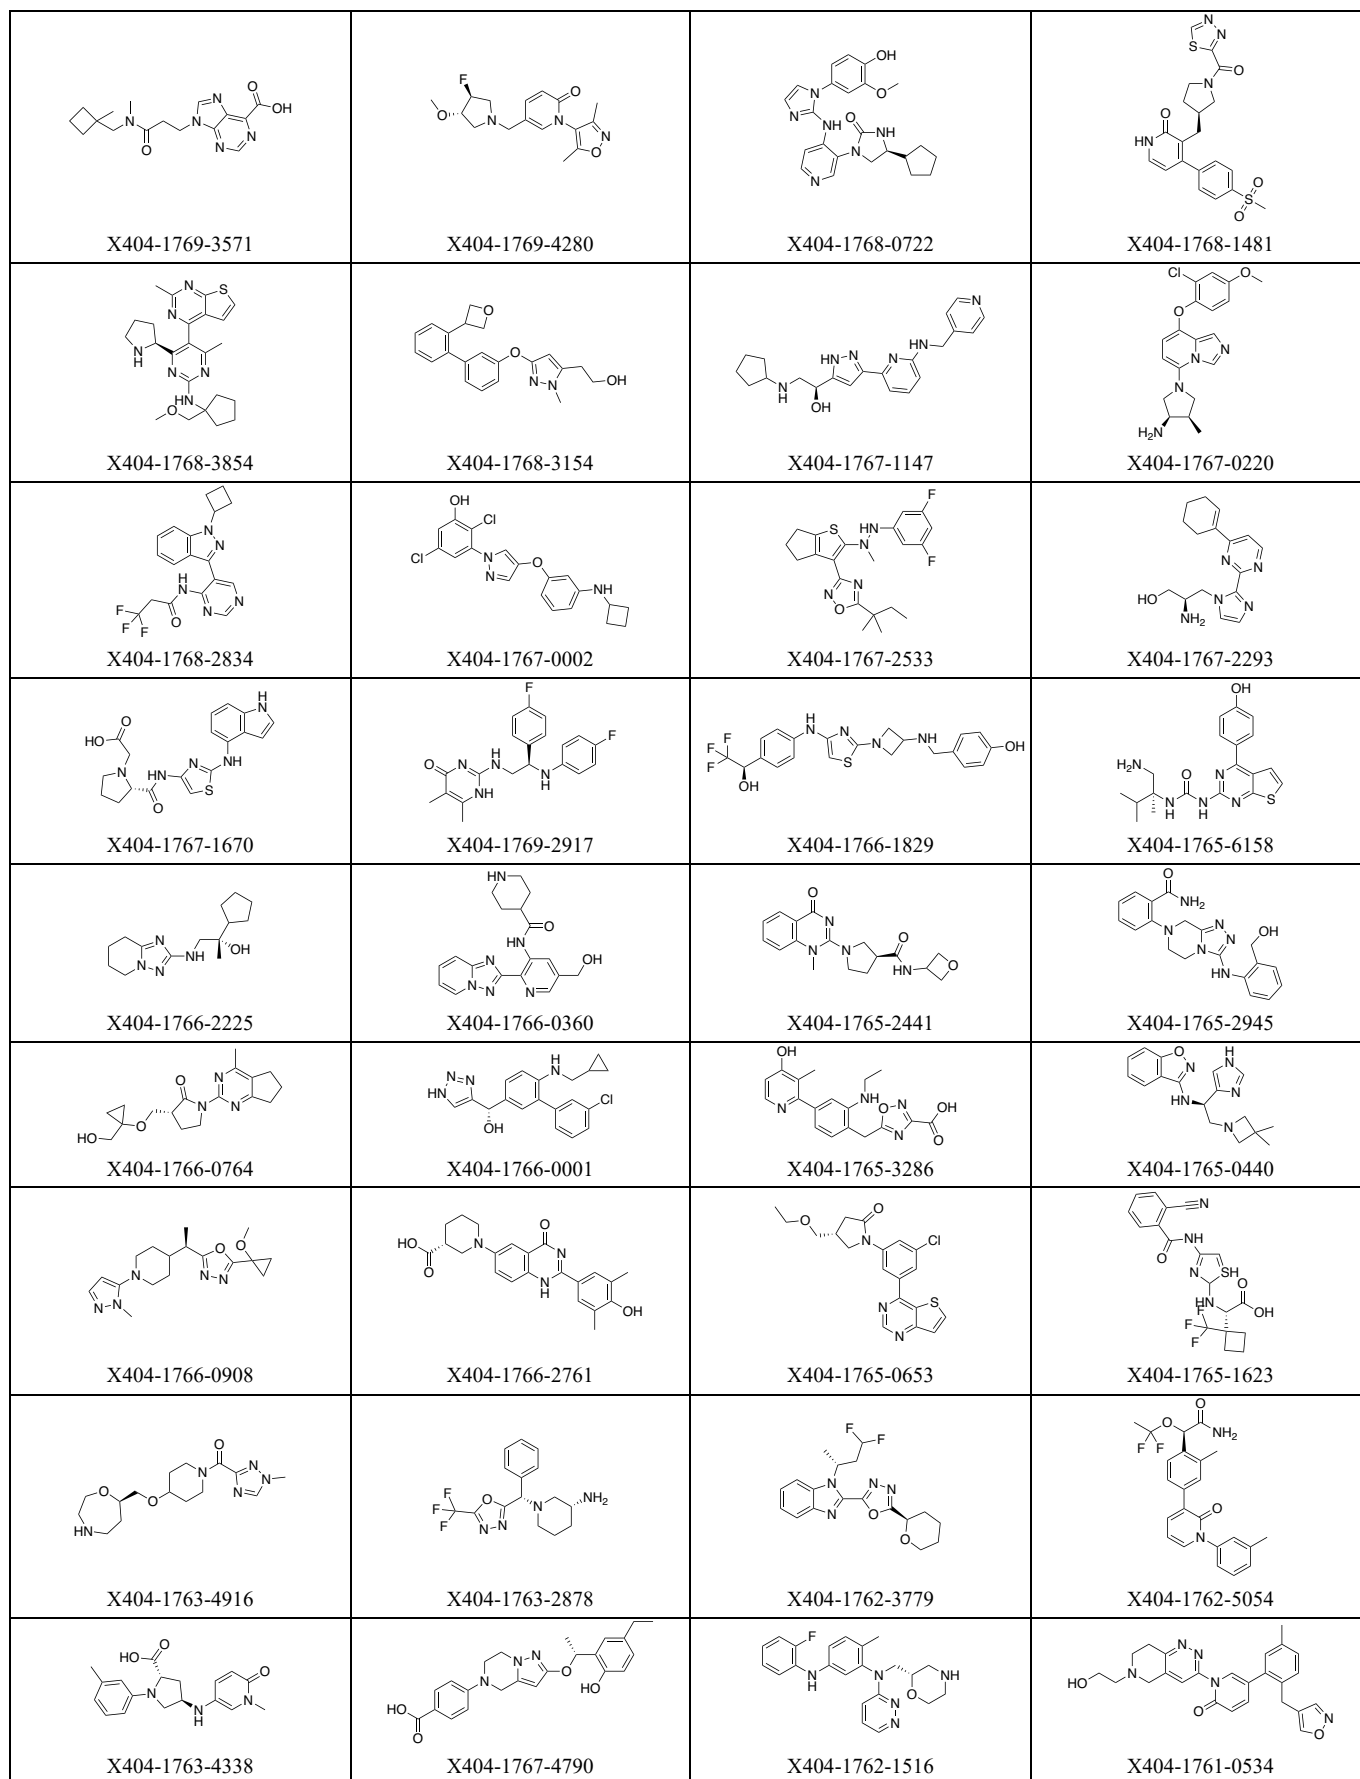  | 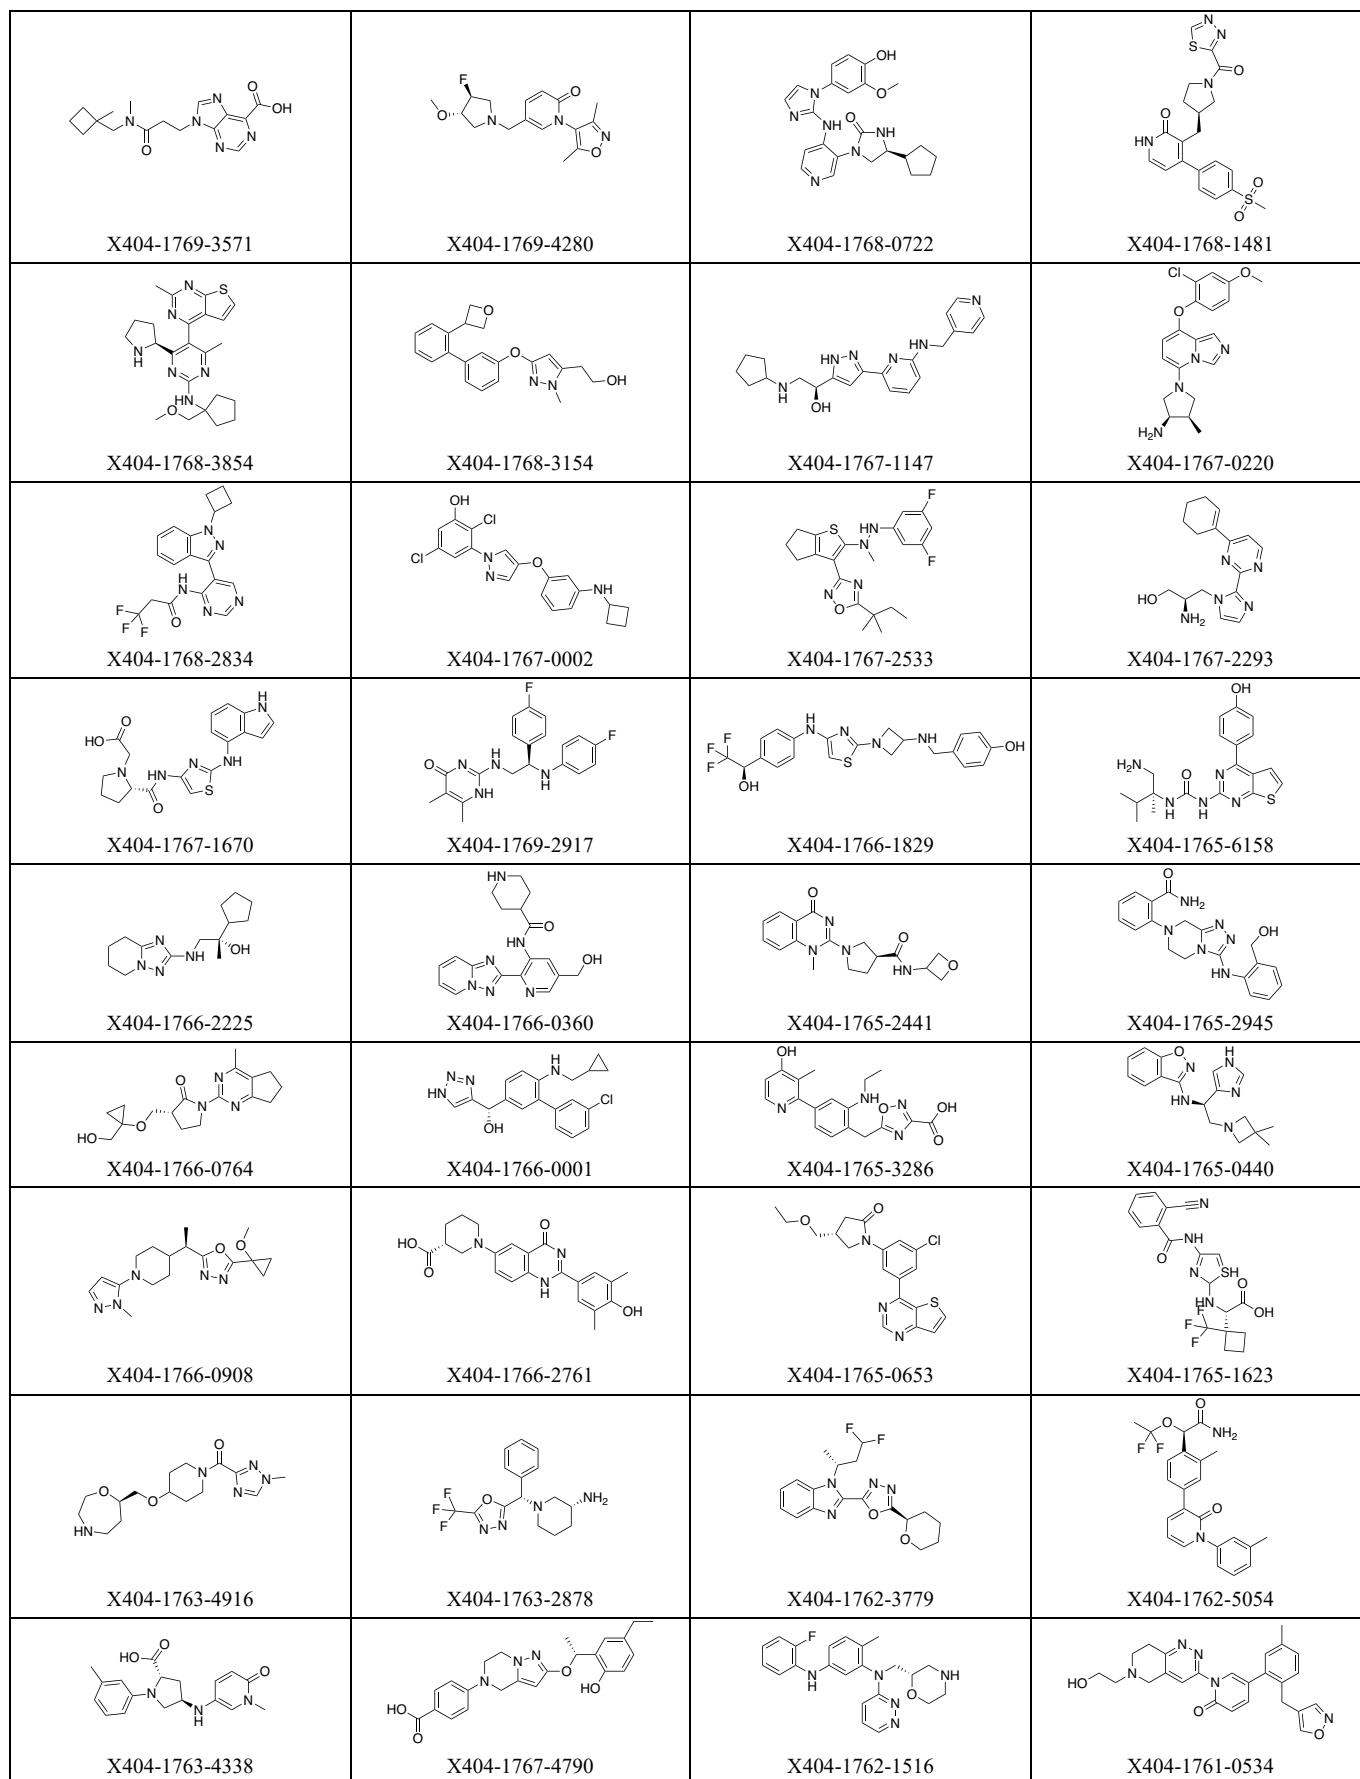 | 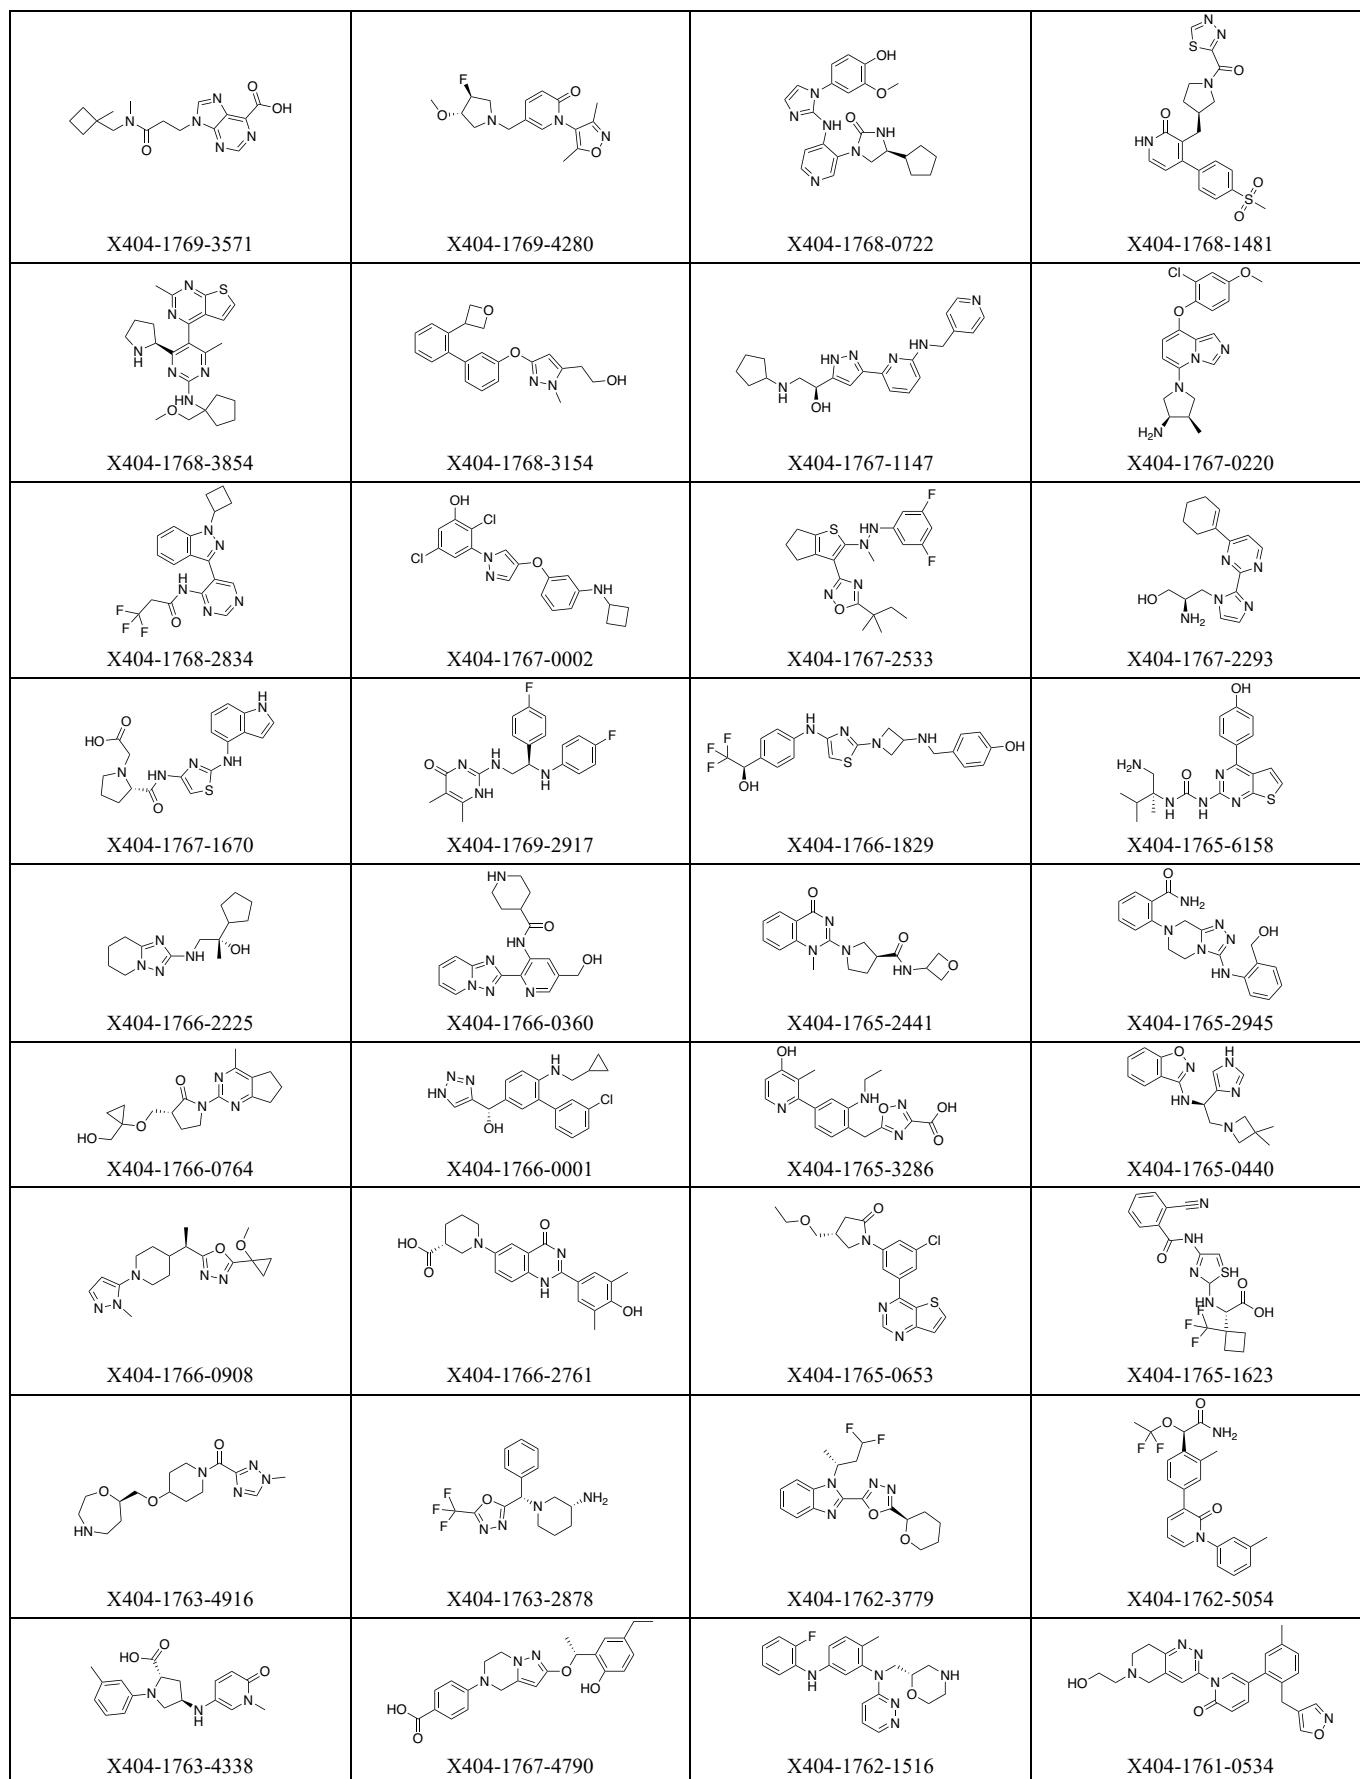  |
| 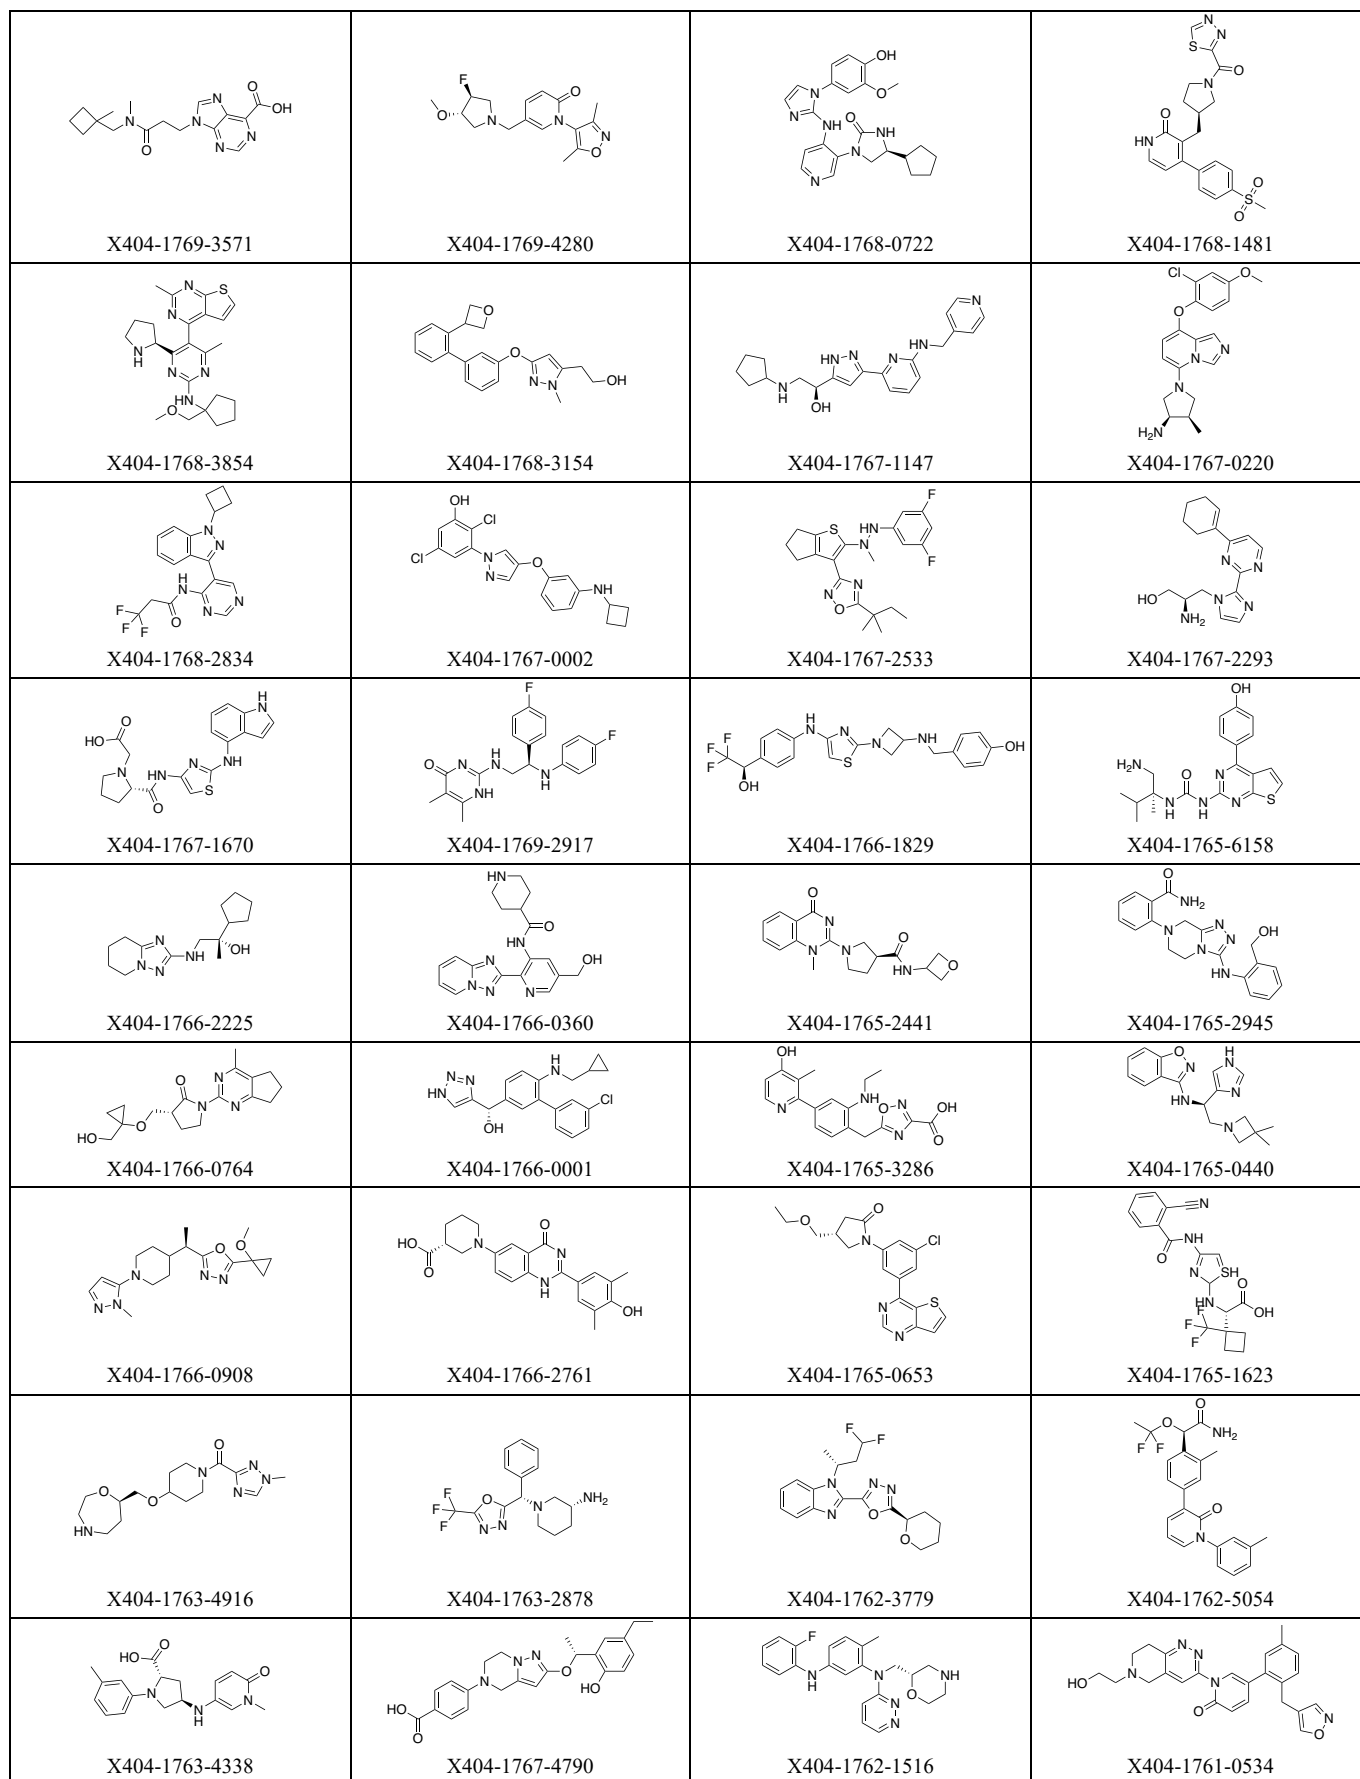 | 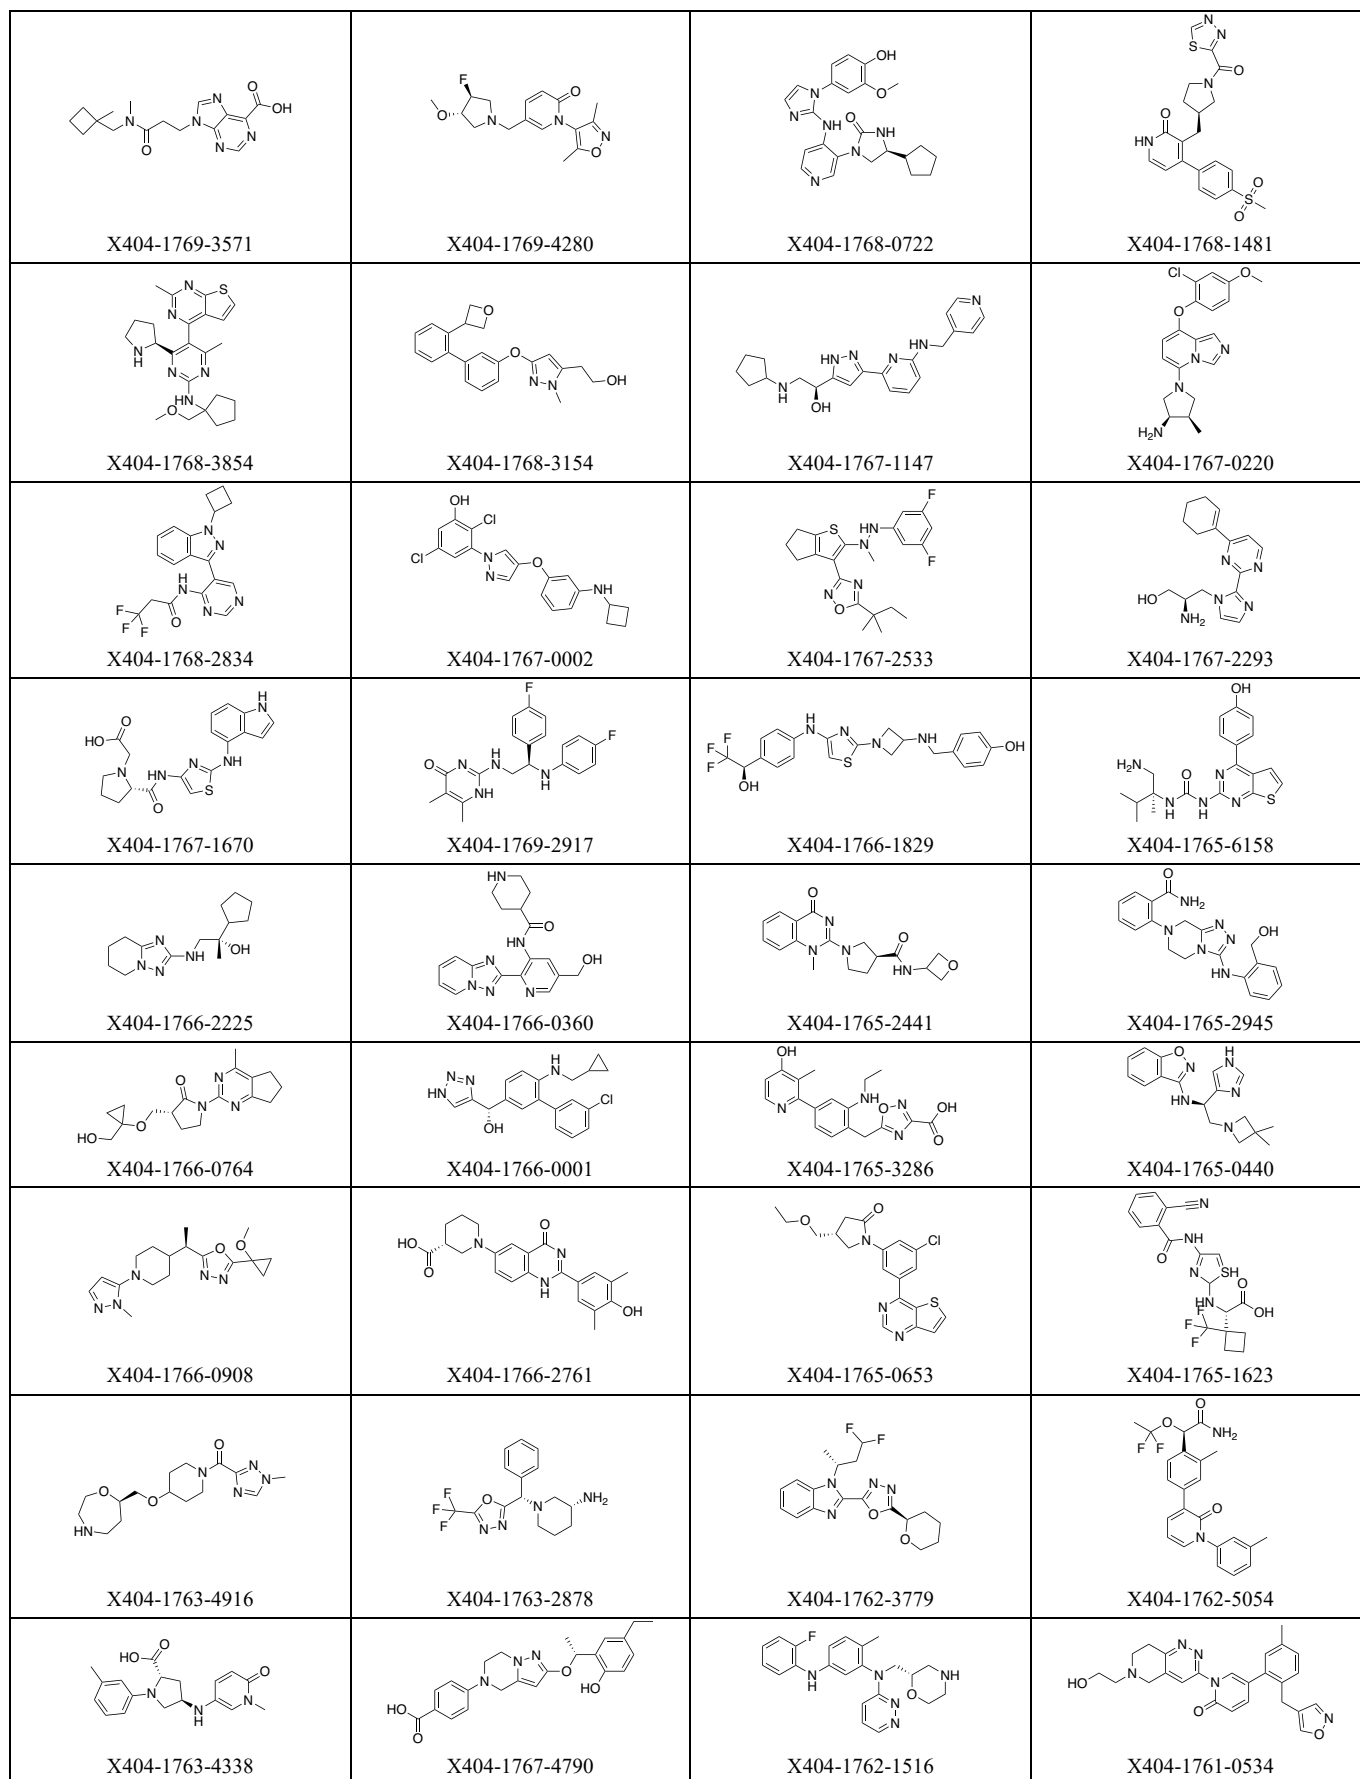 | 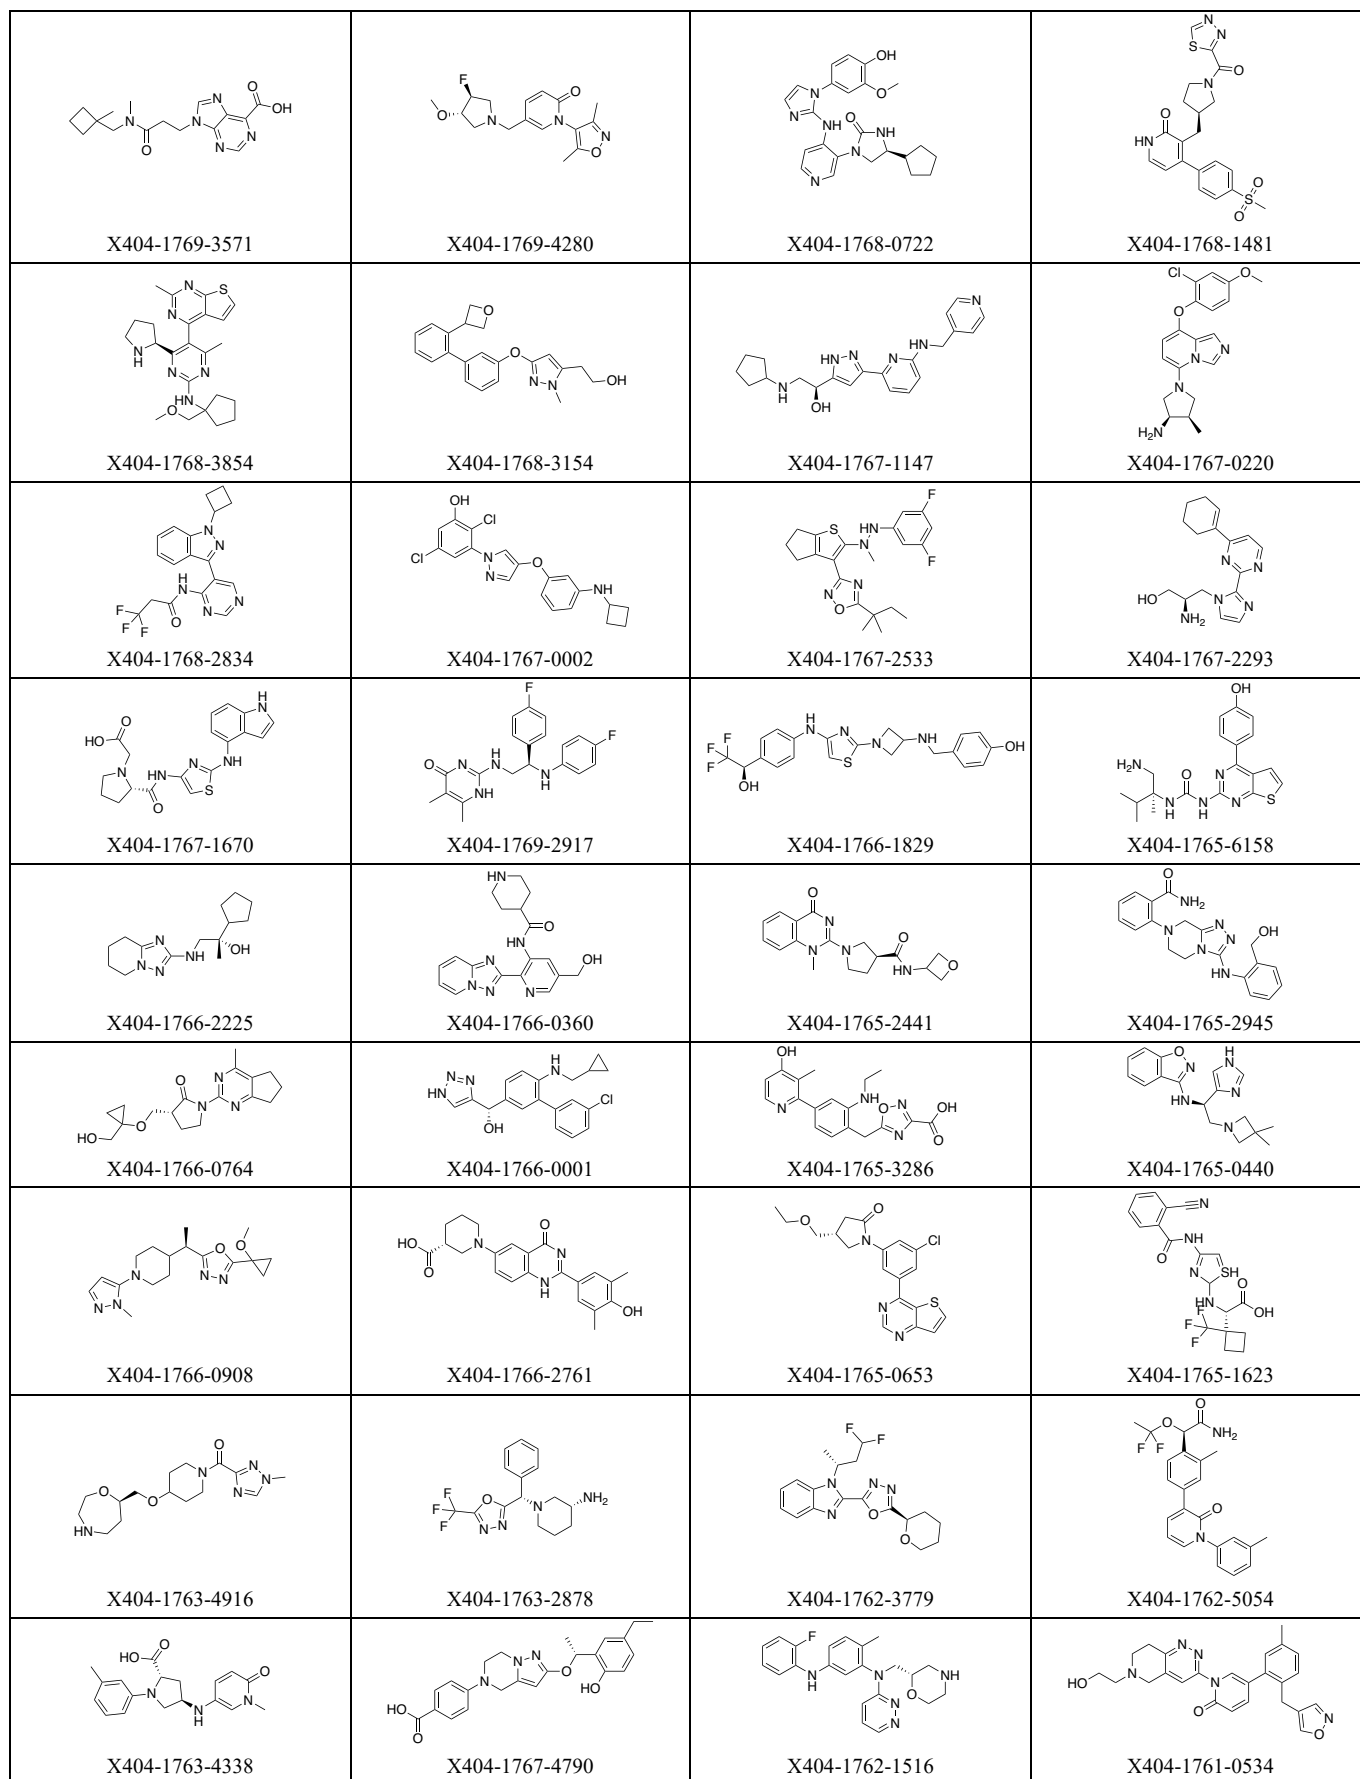 | 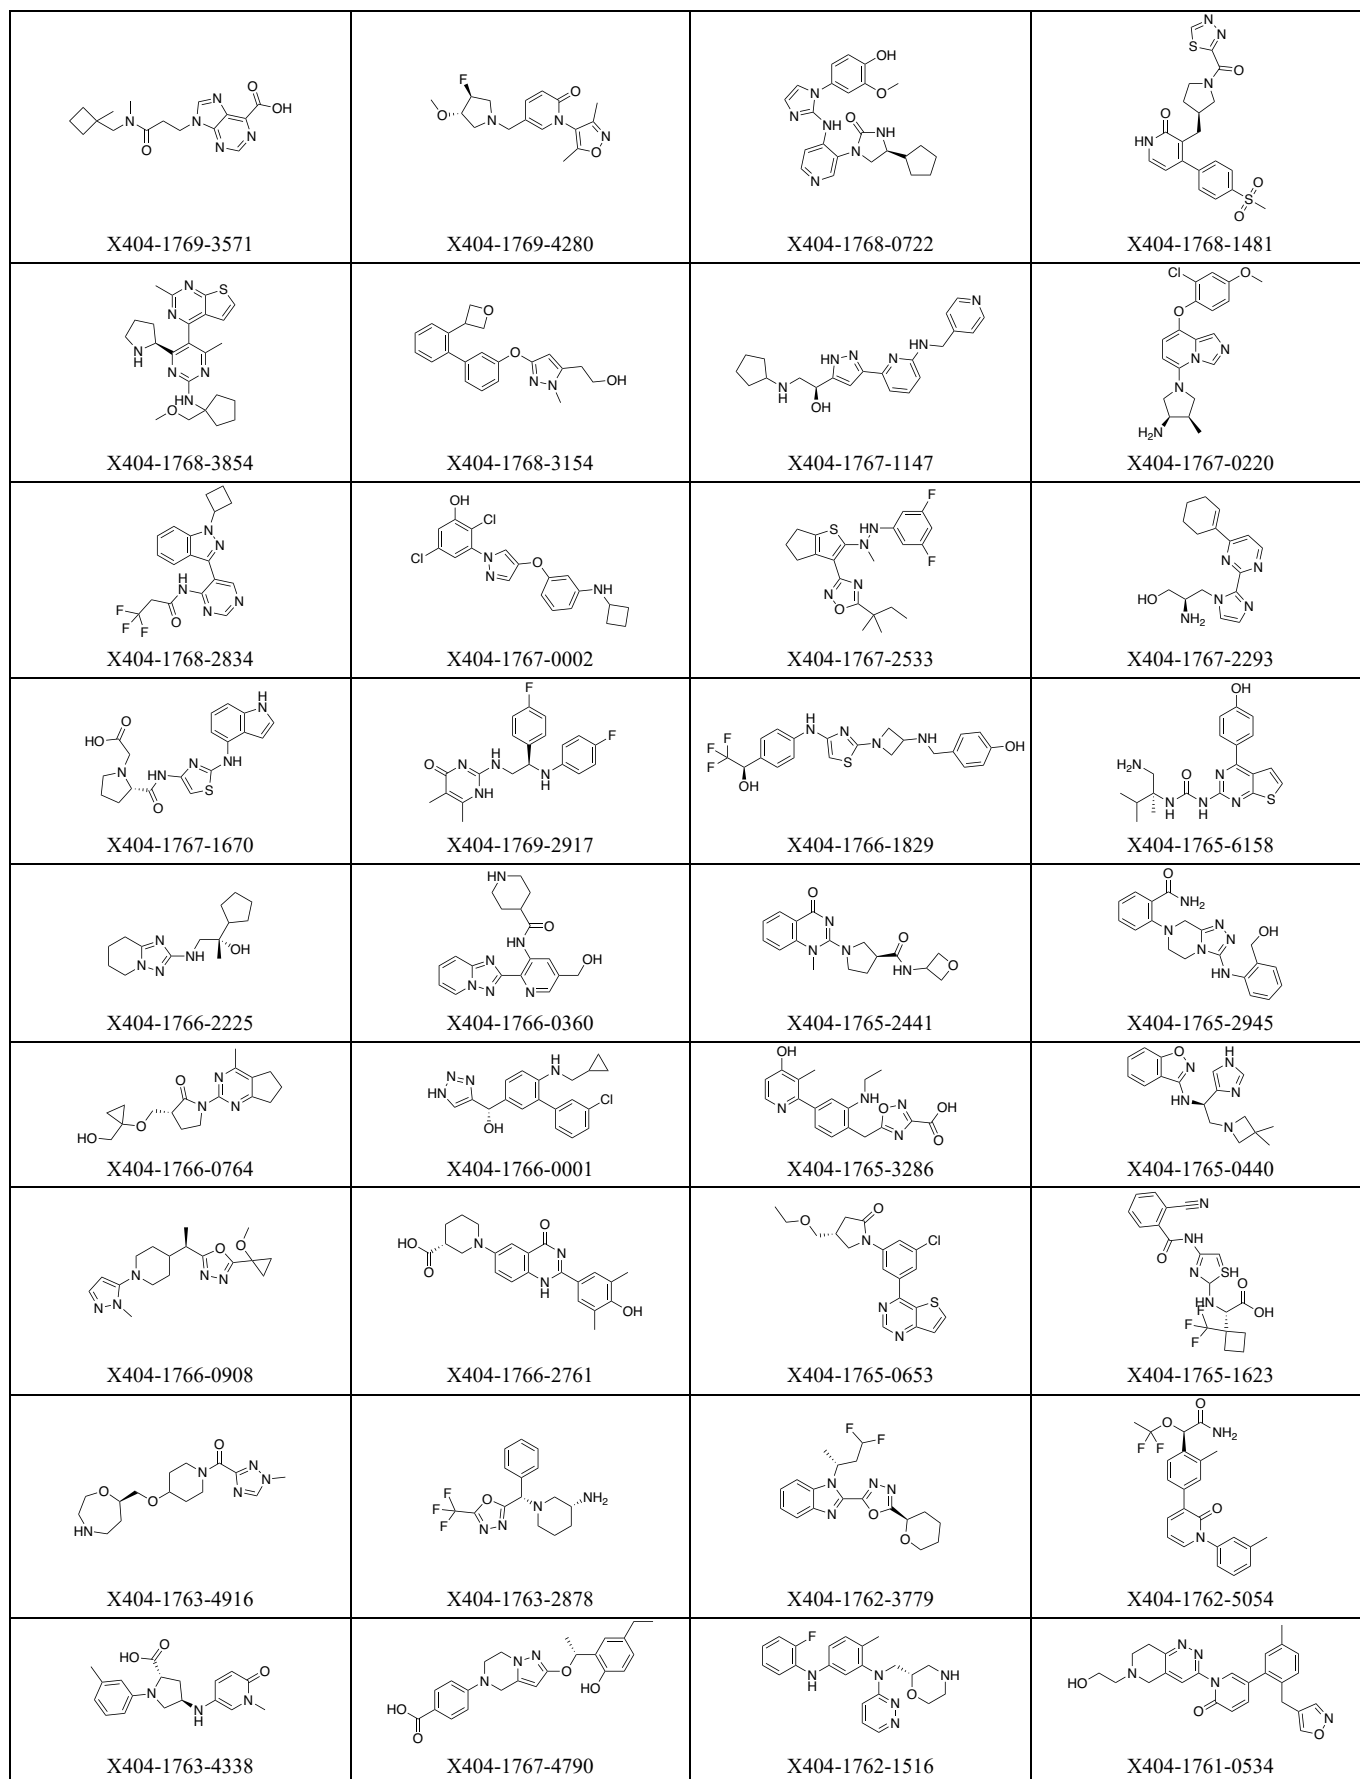 |
| 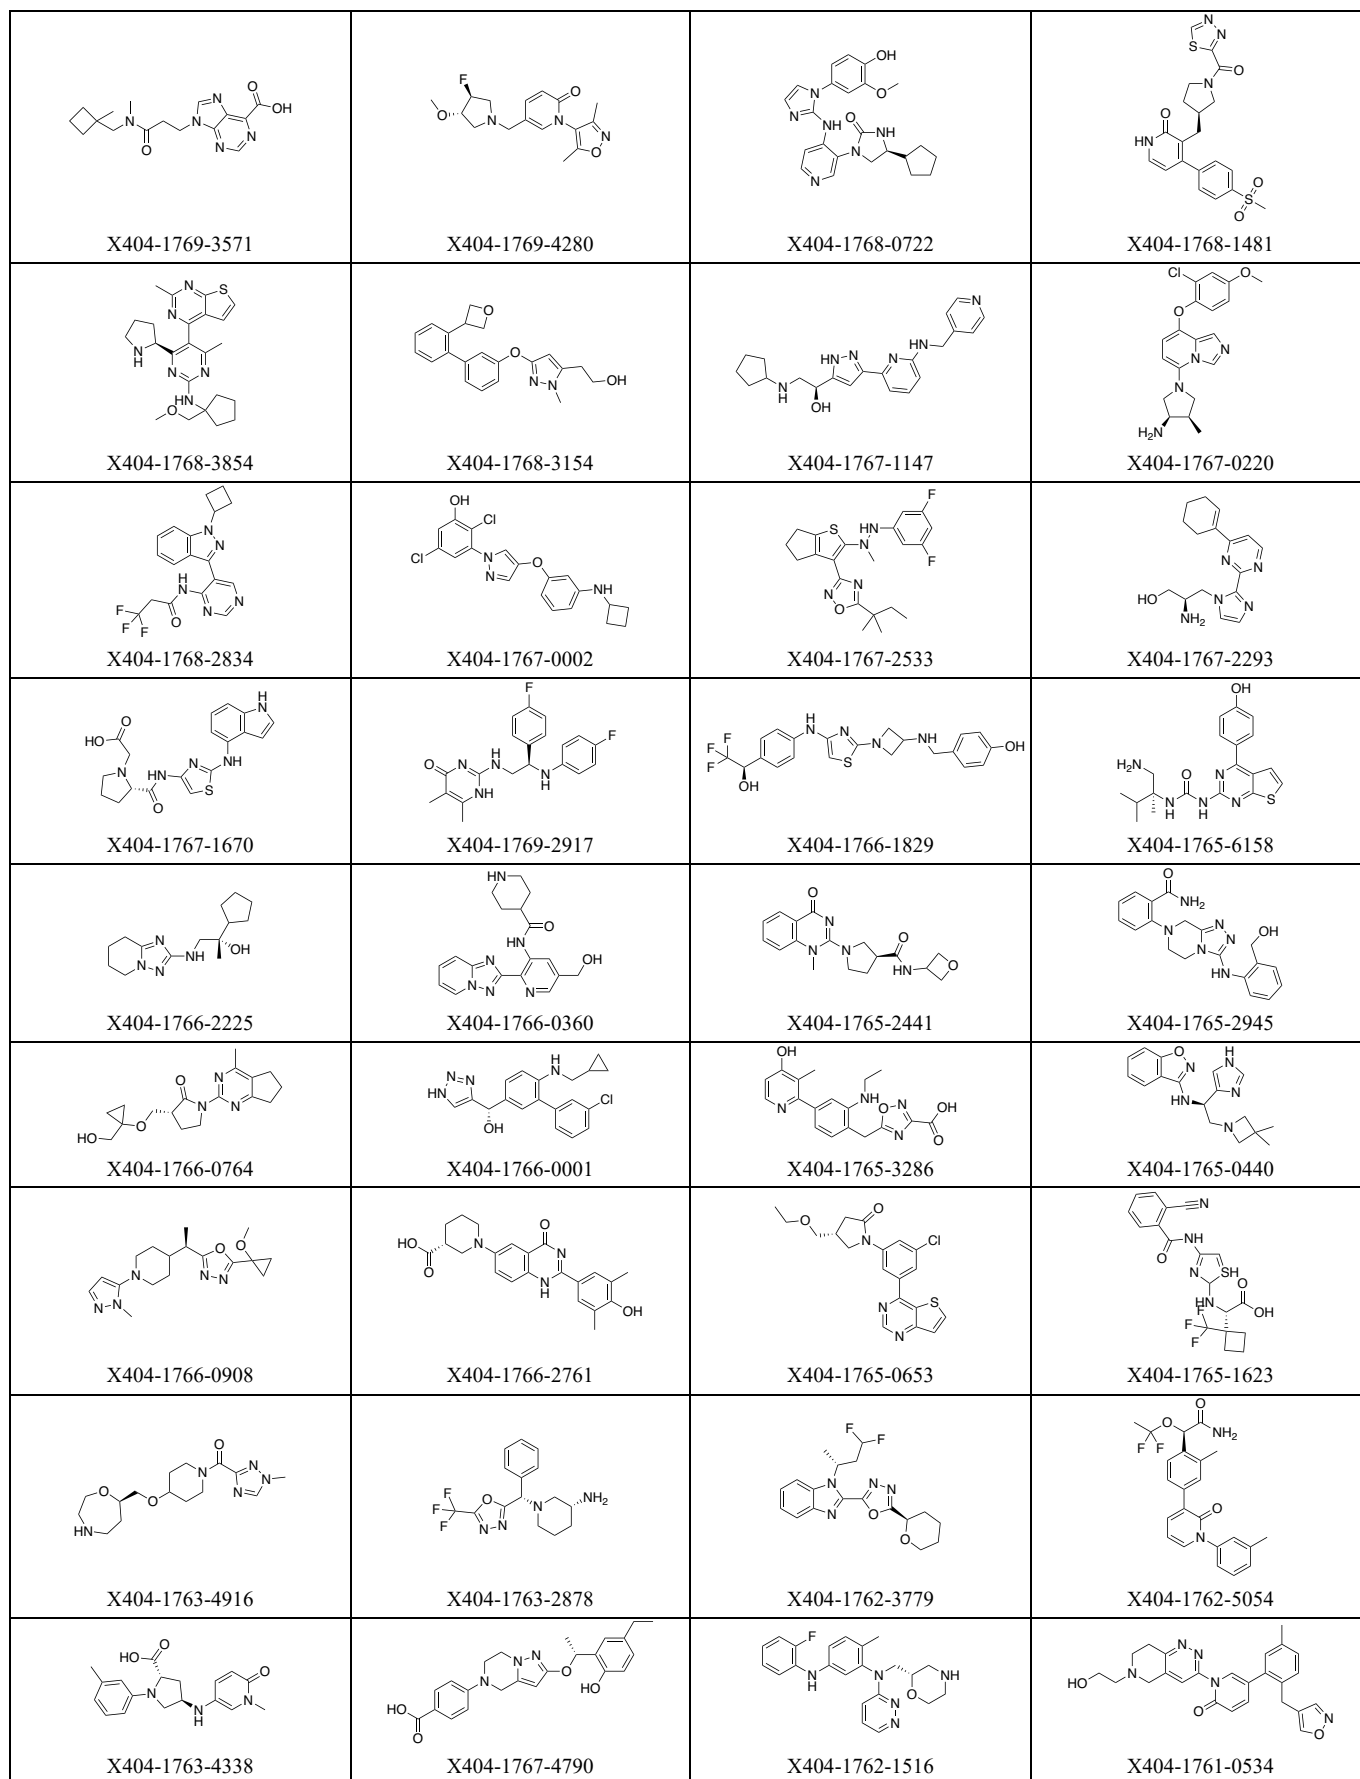 | 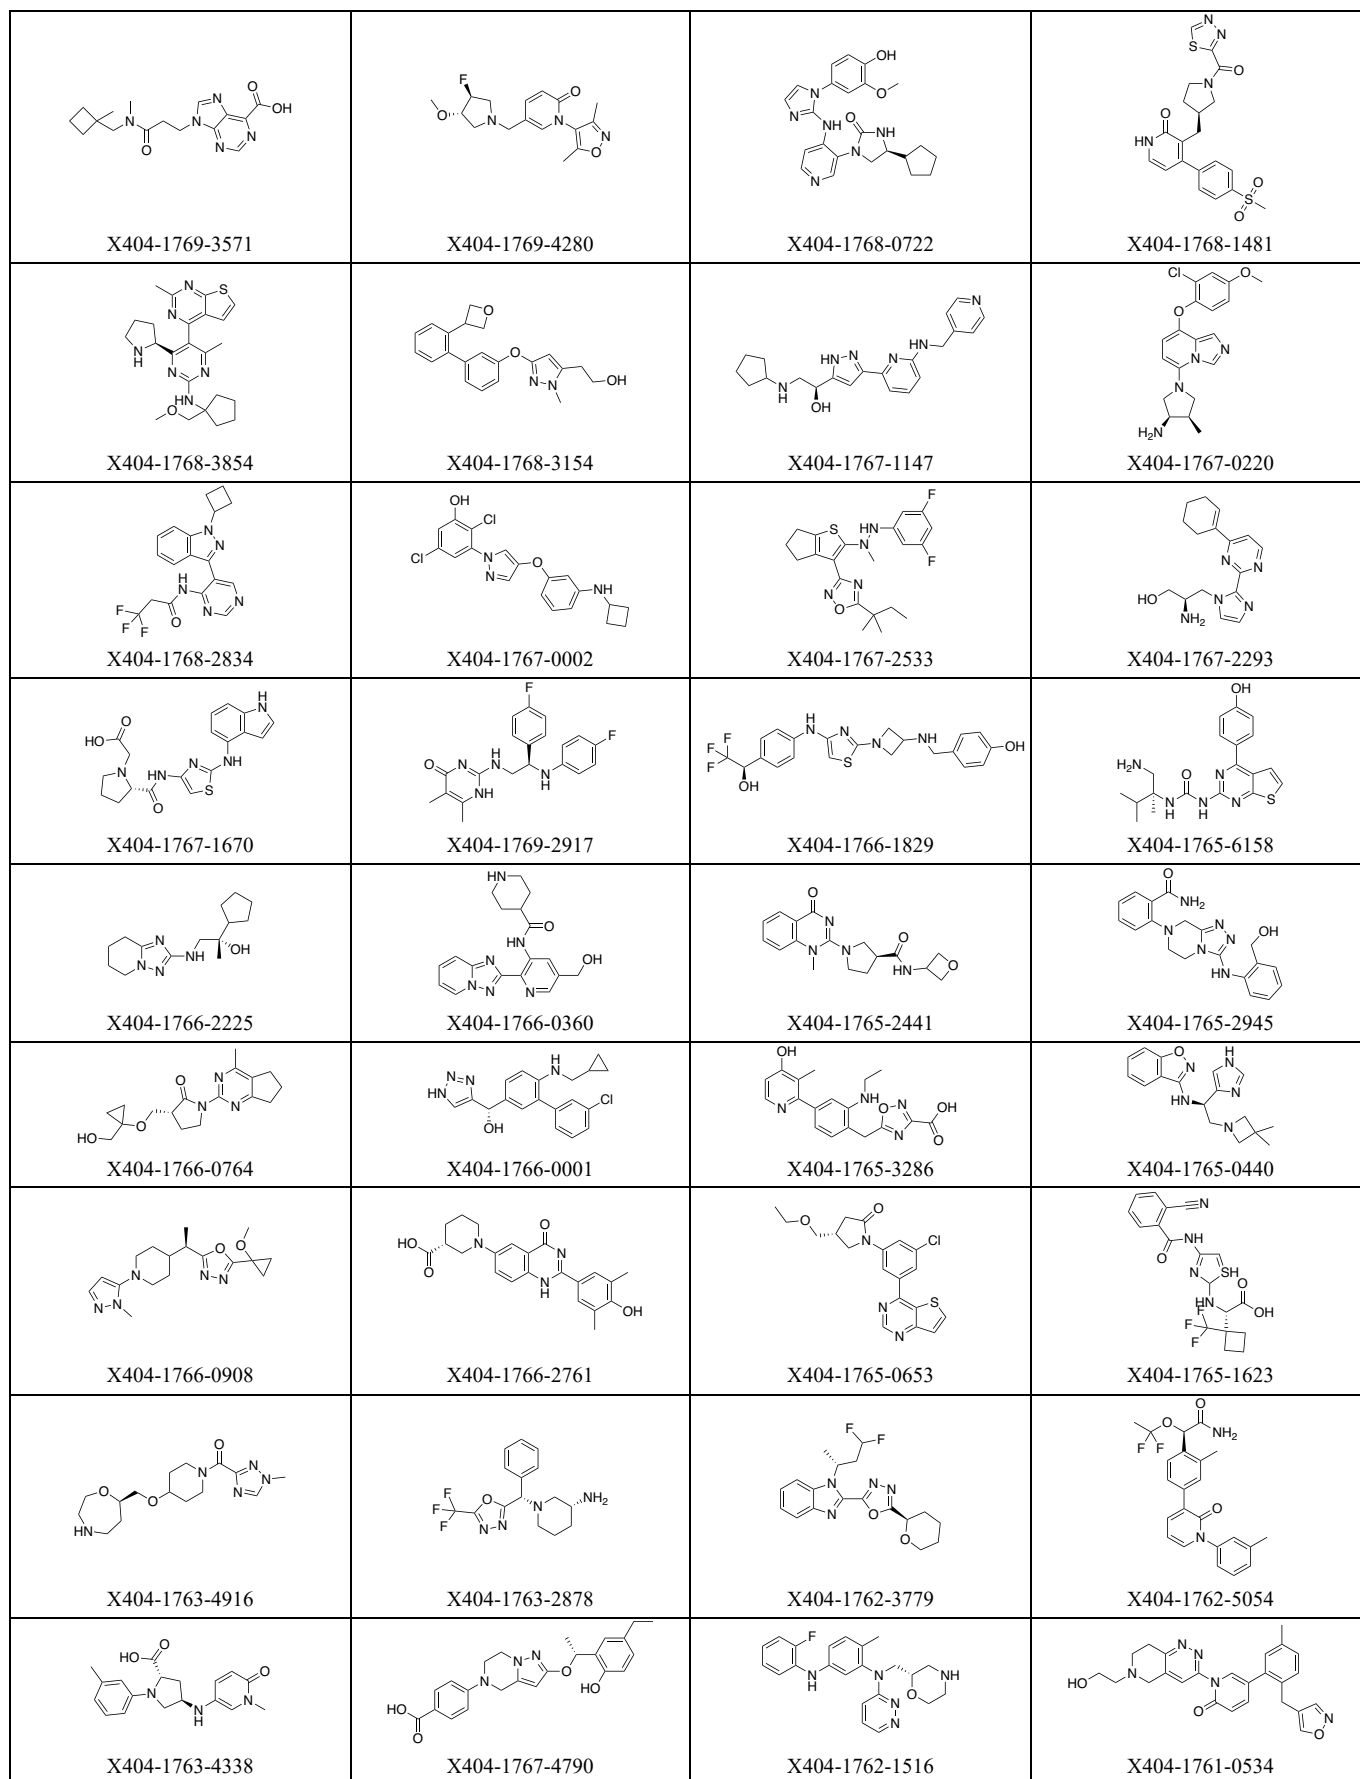 | 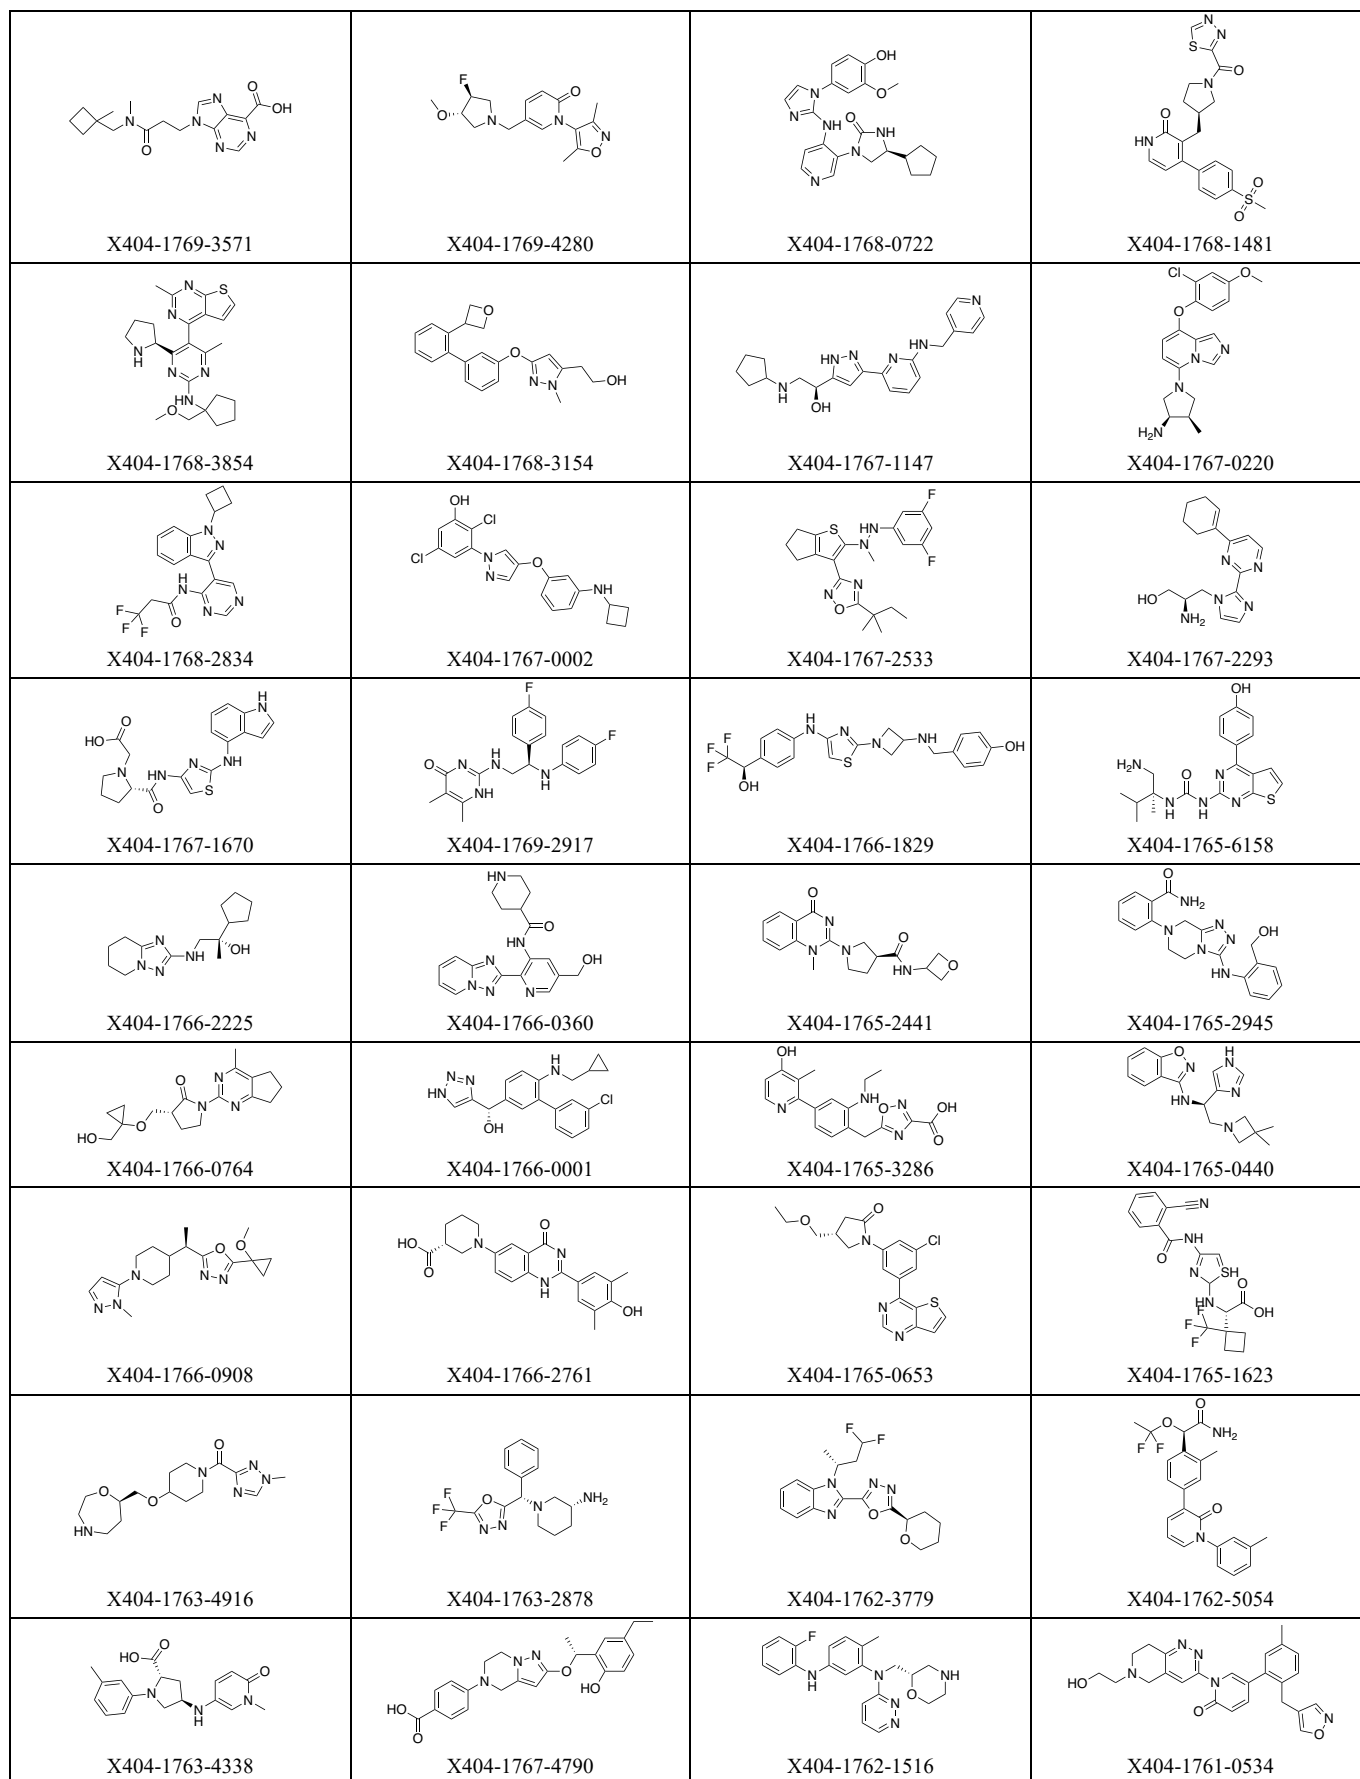 | 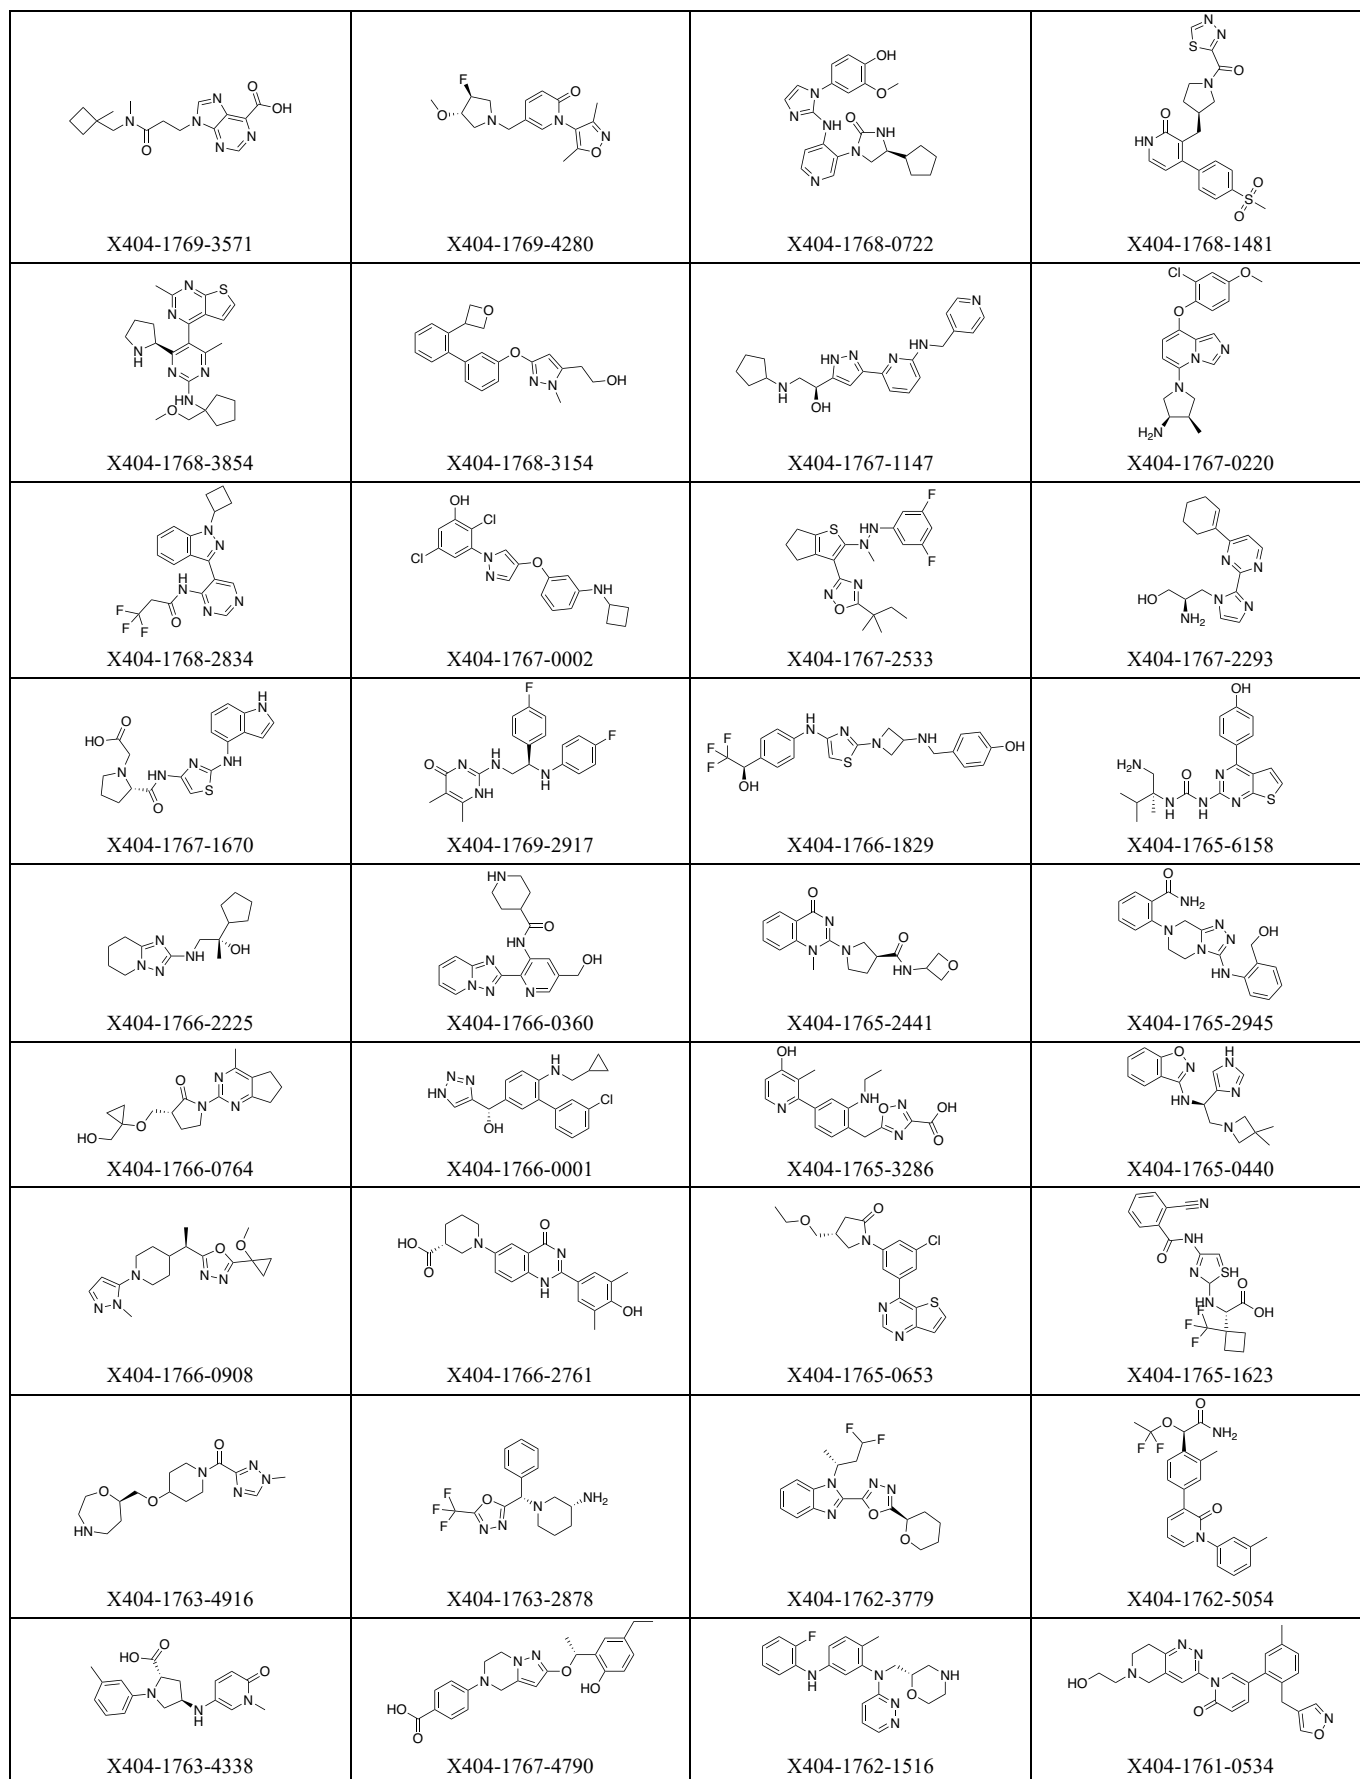 |
| 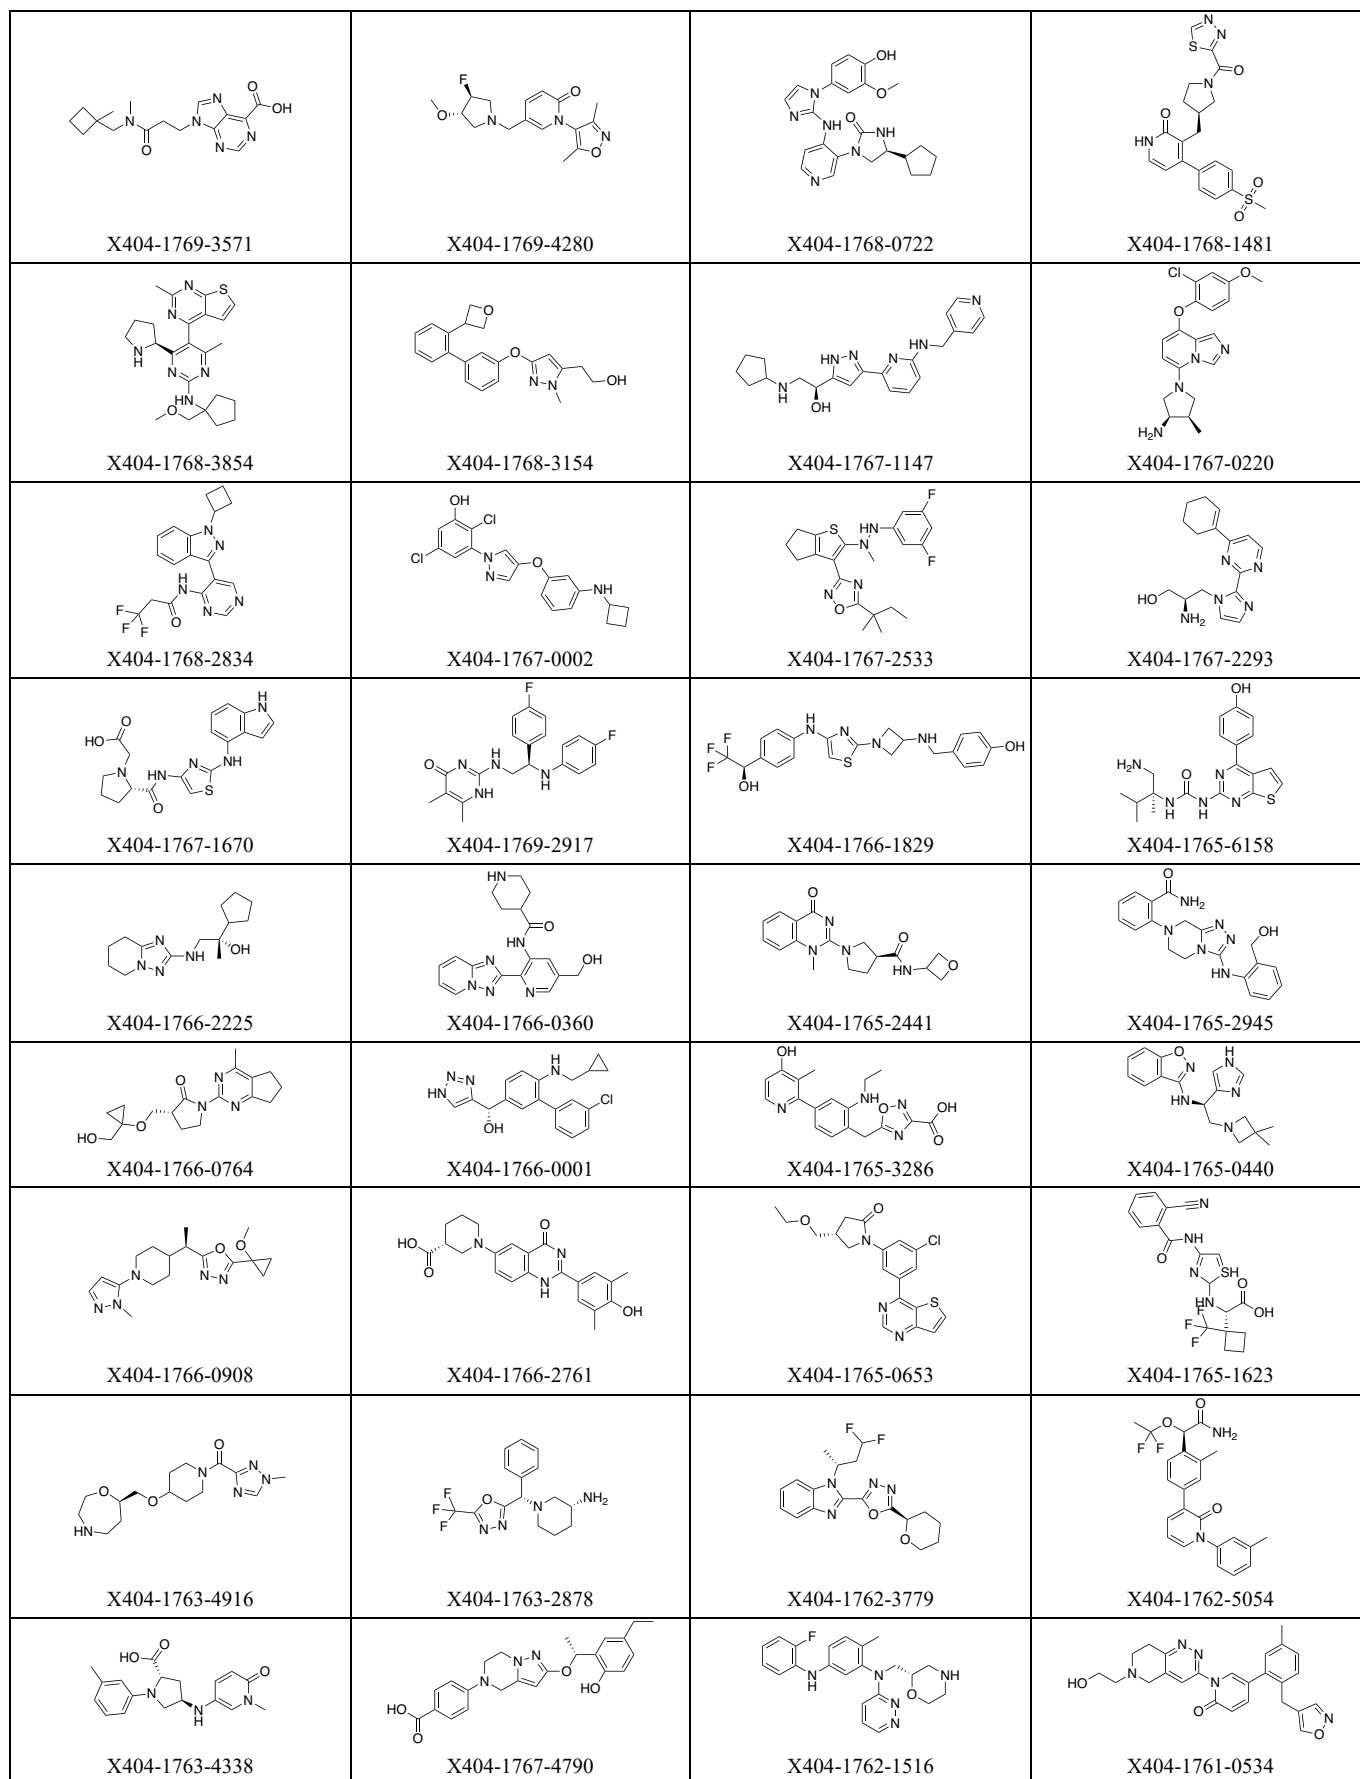 | 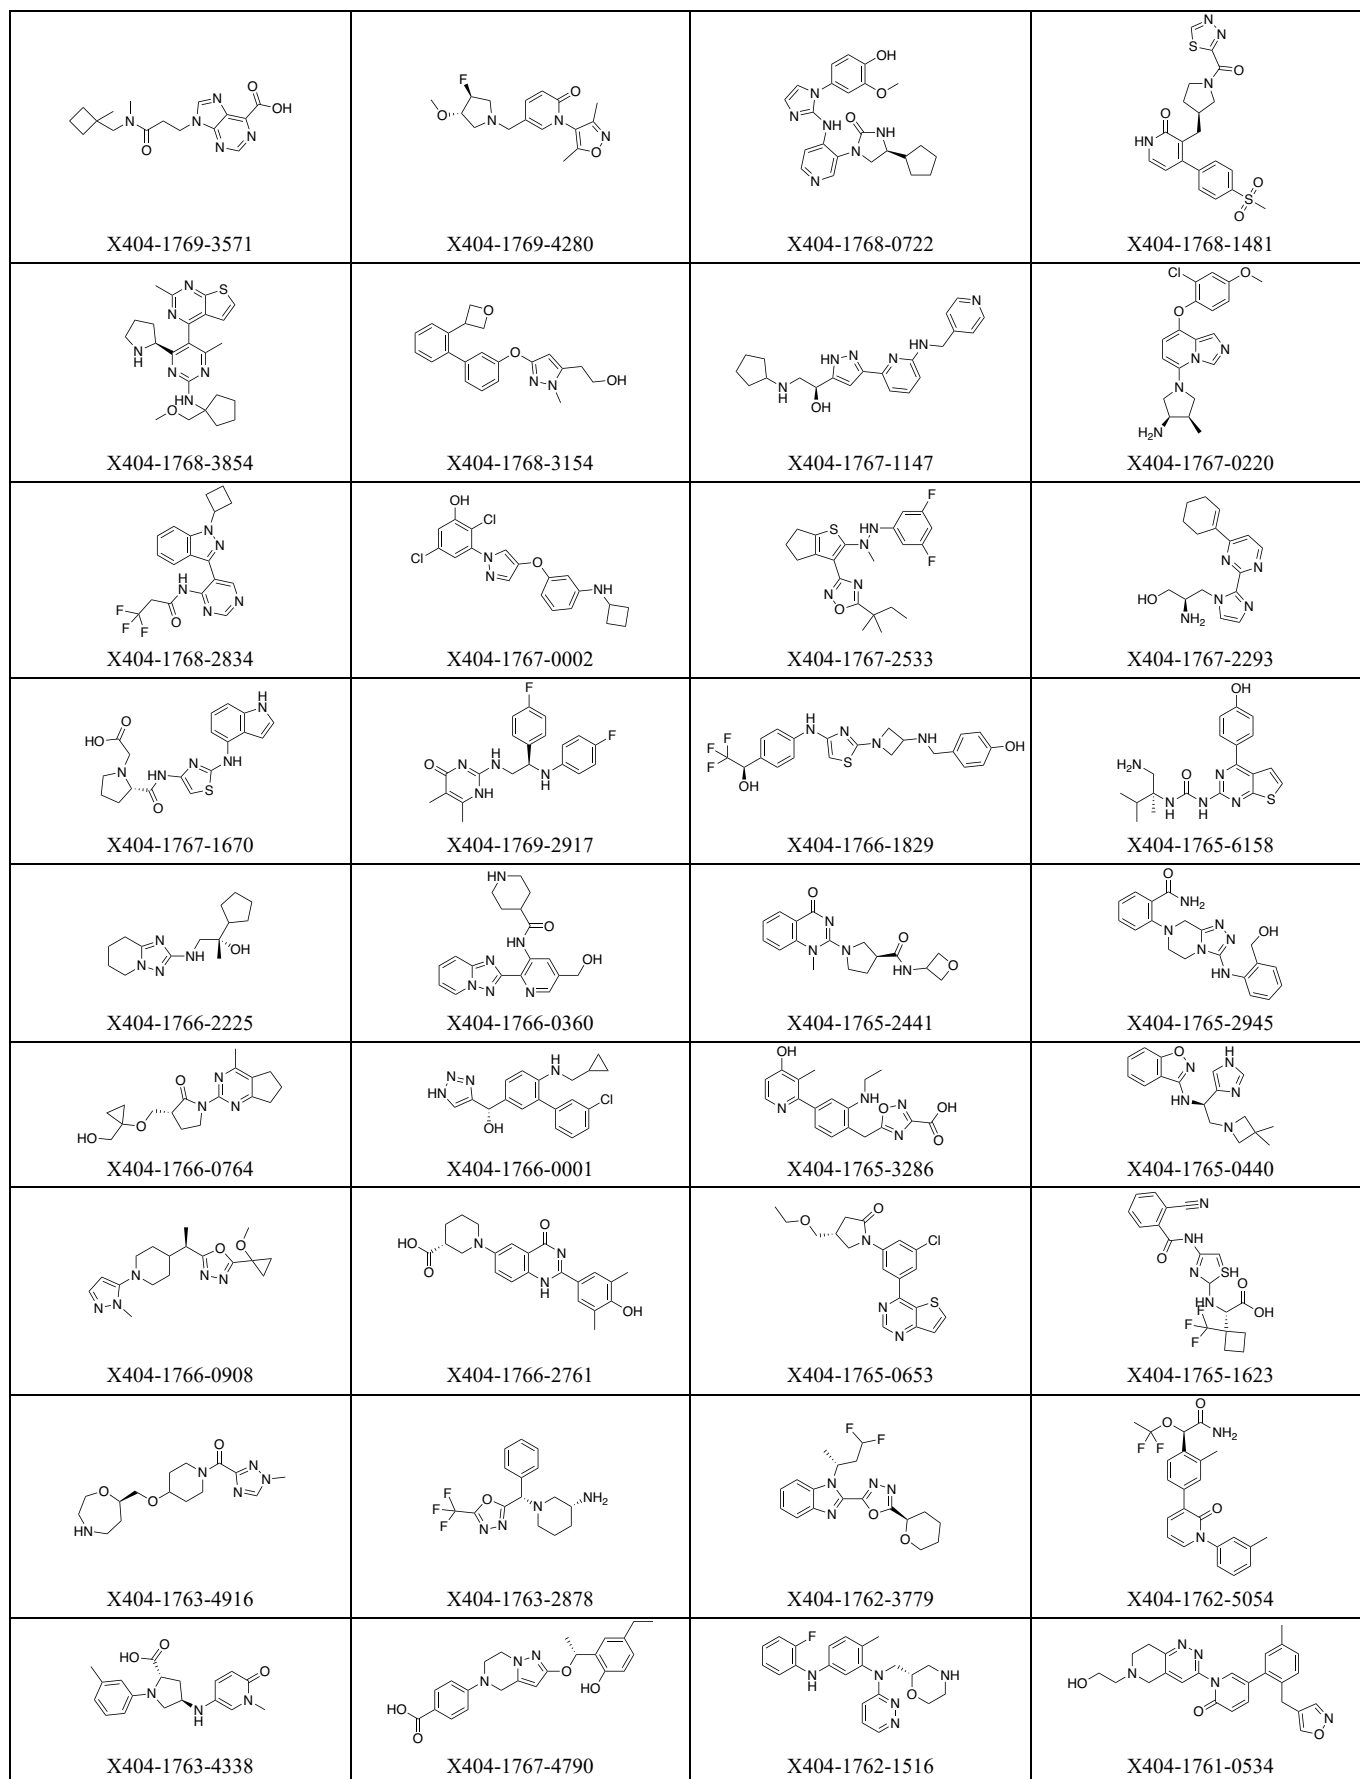 | 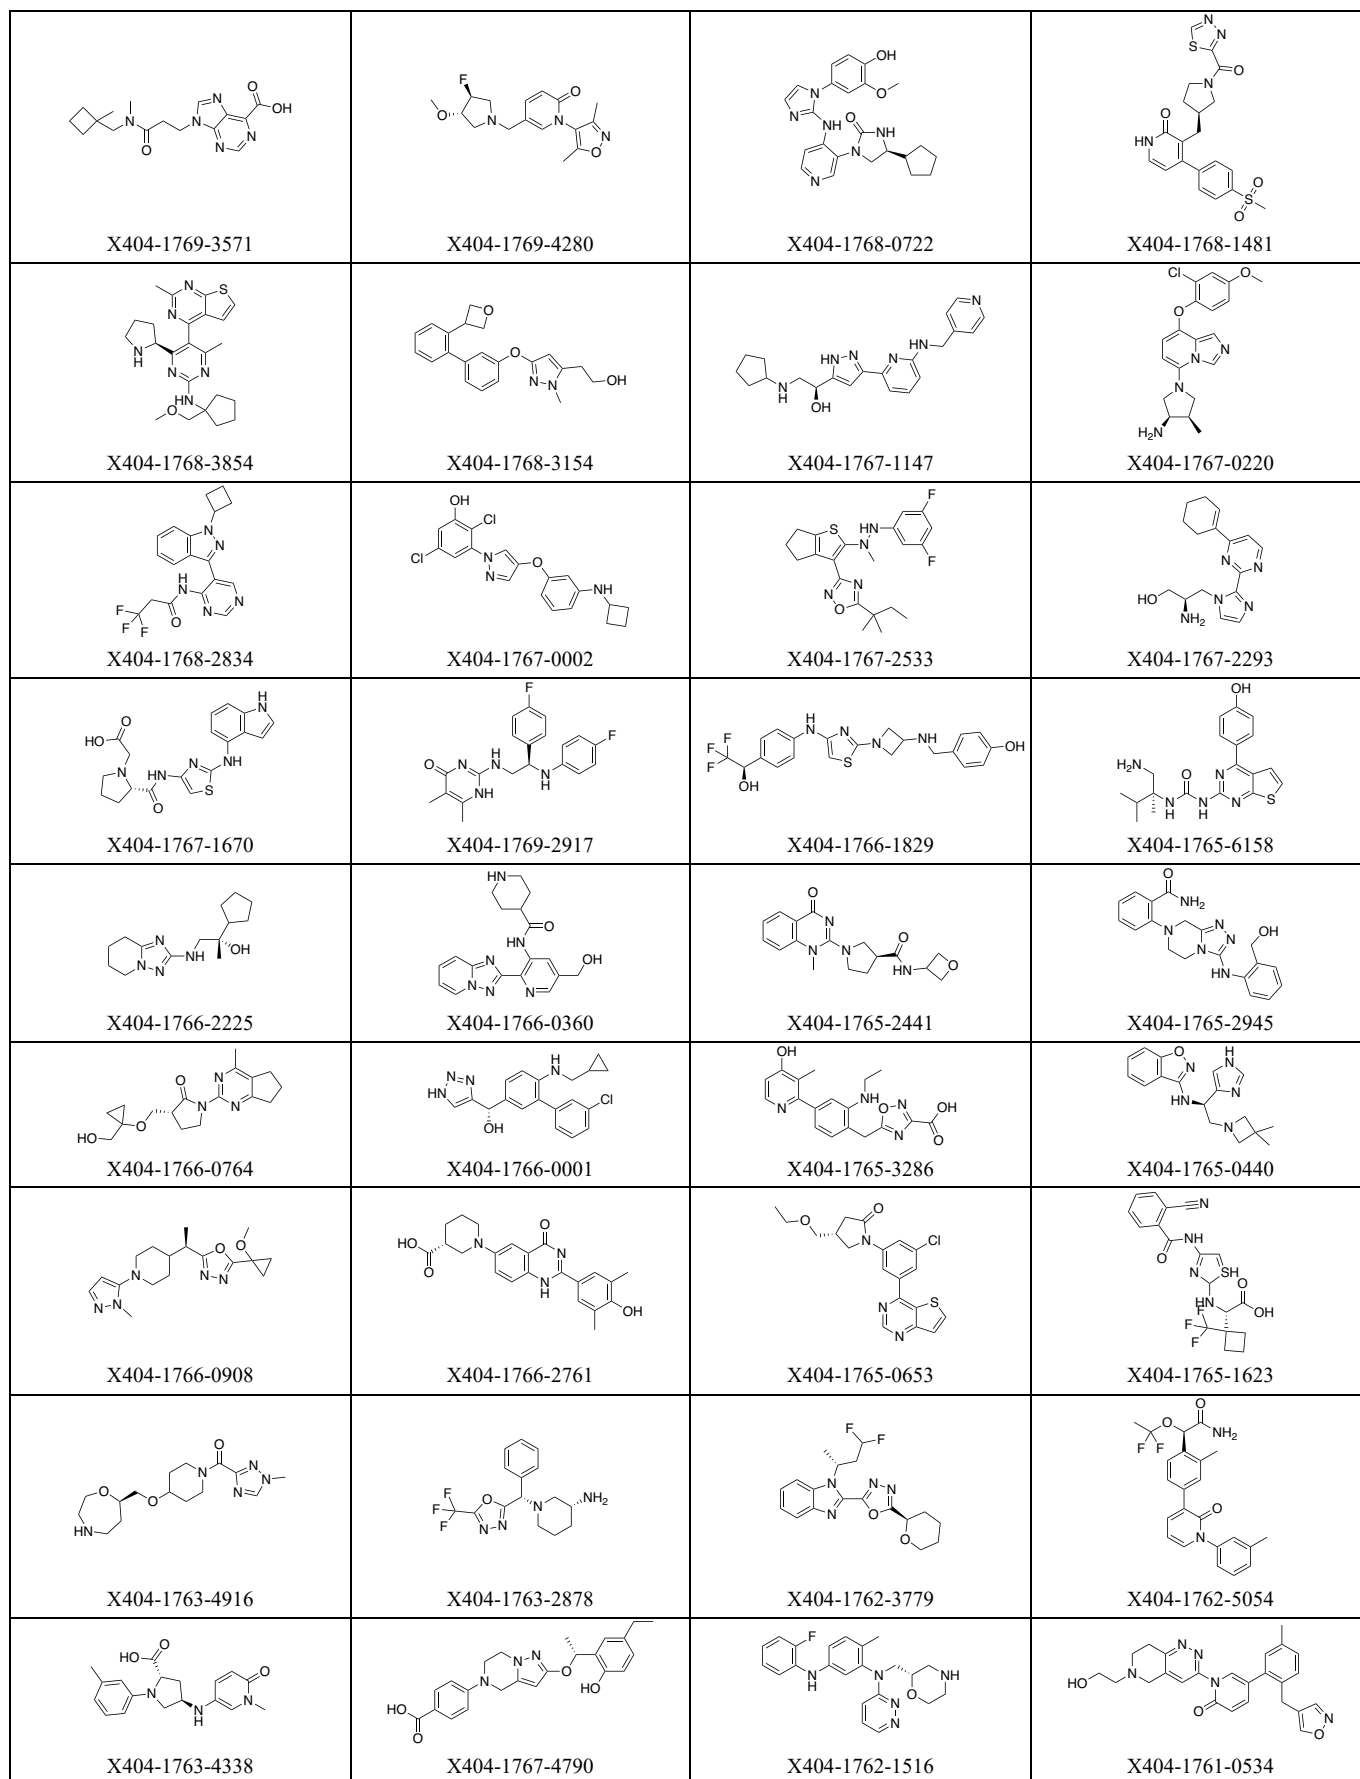 | 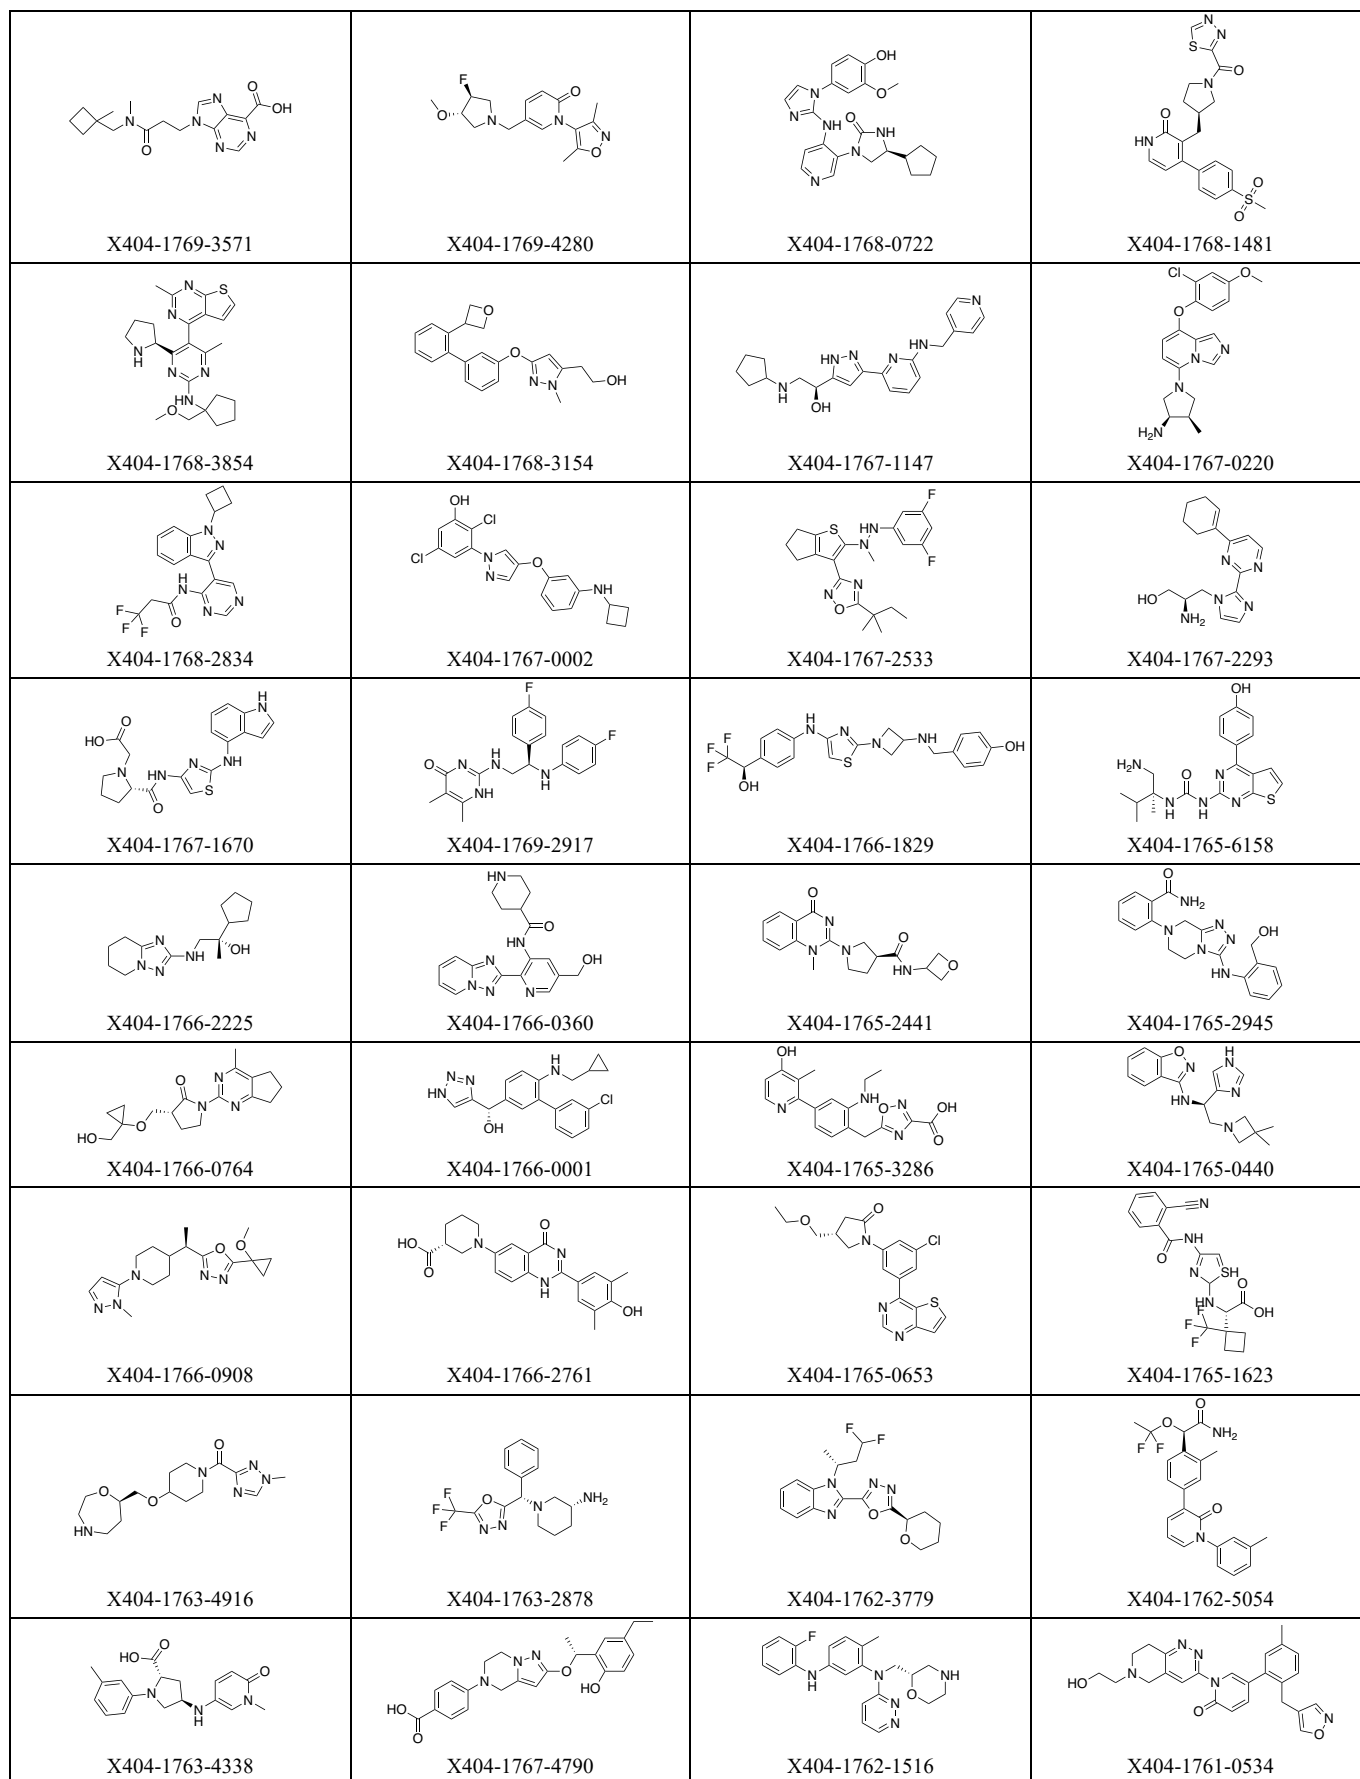 |
| 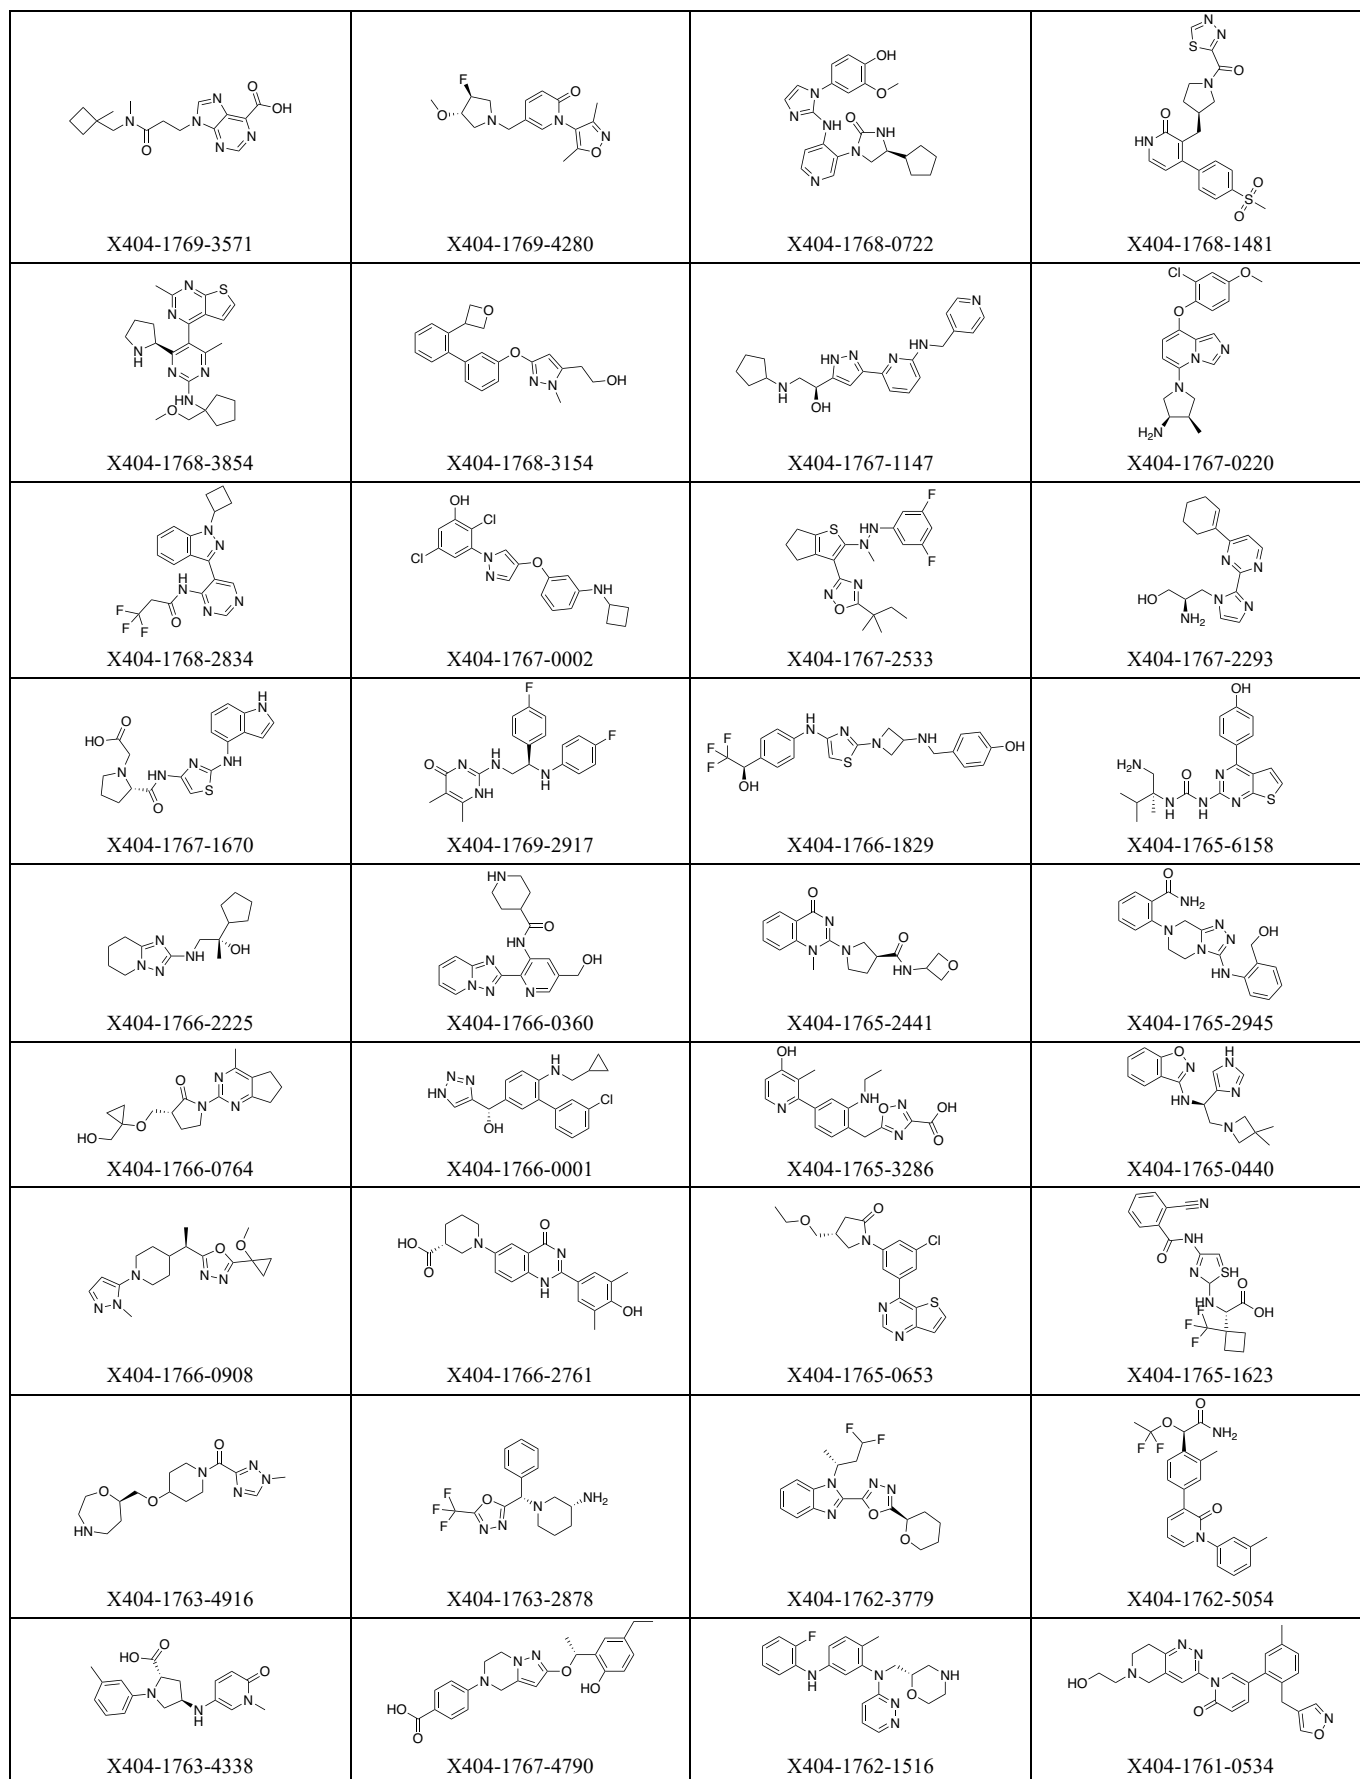 | 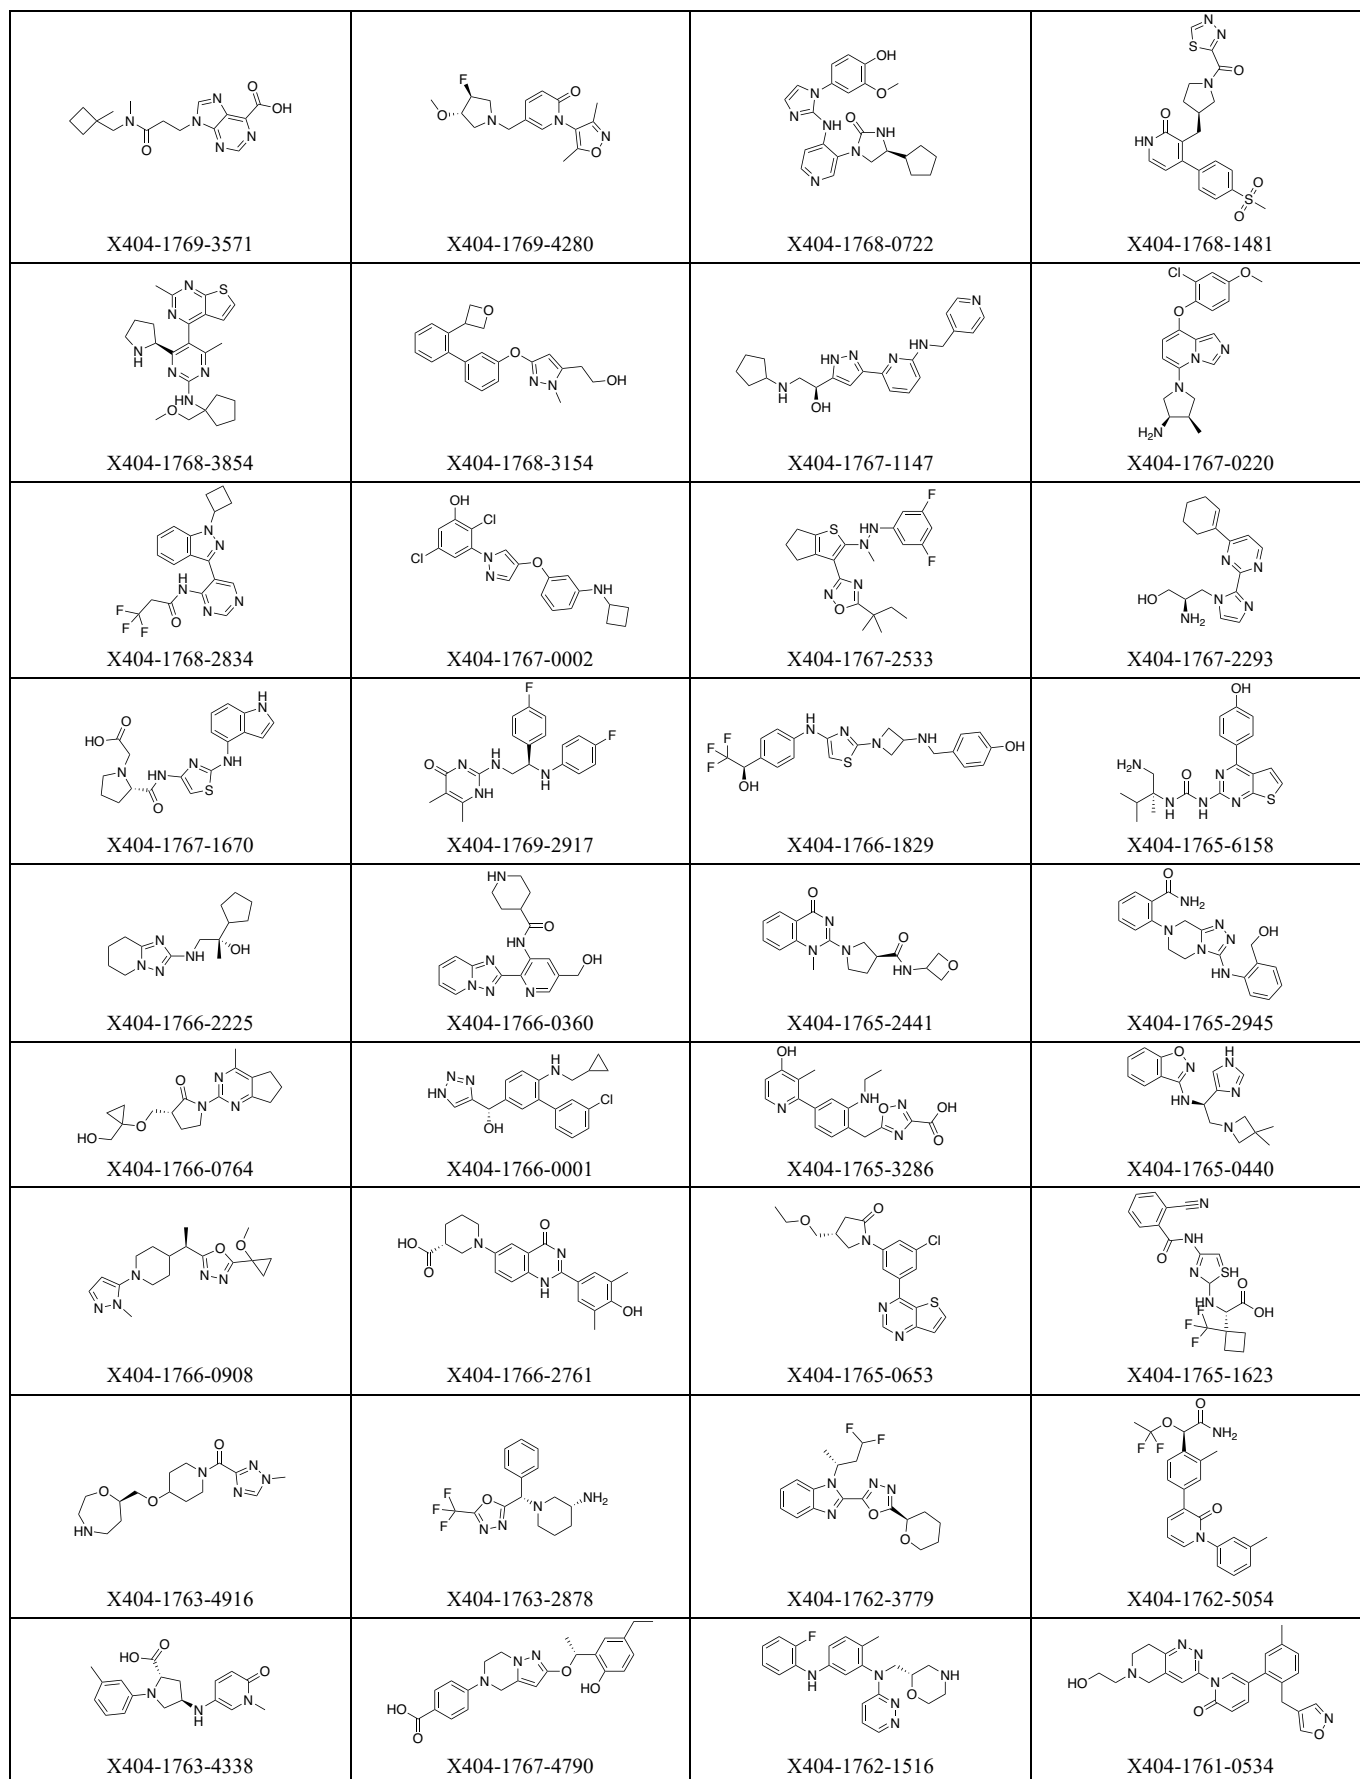 | 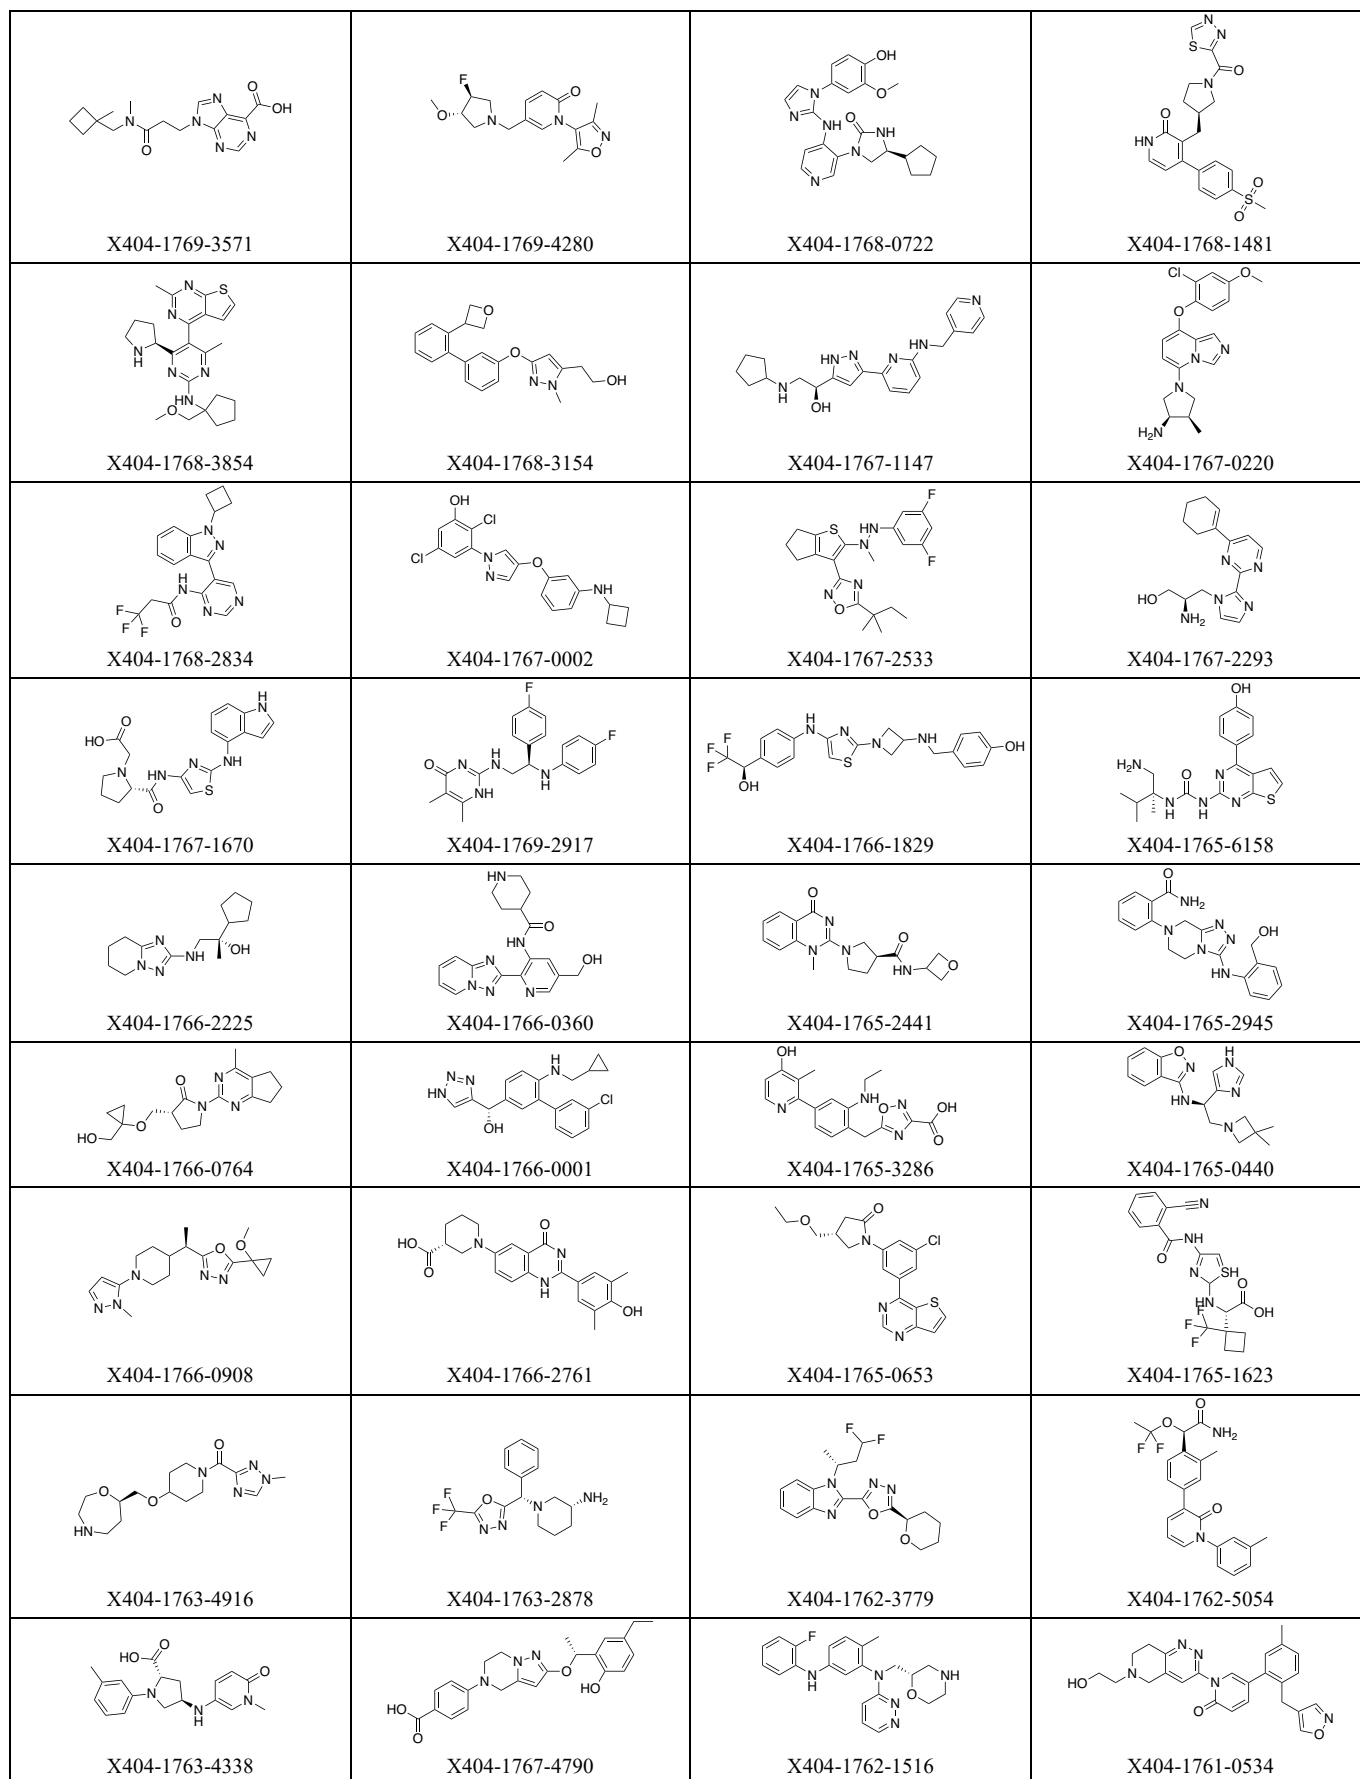 | 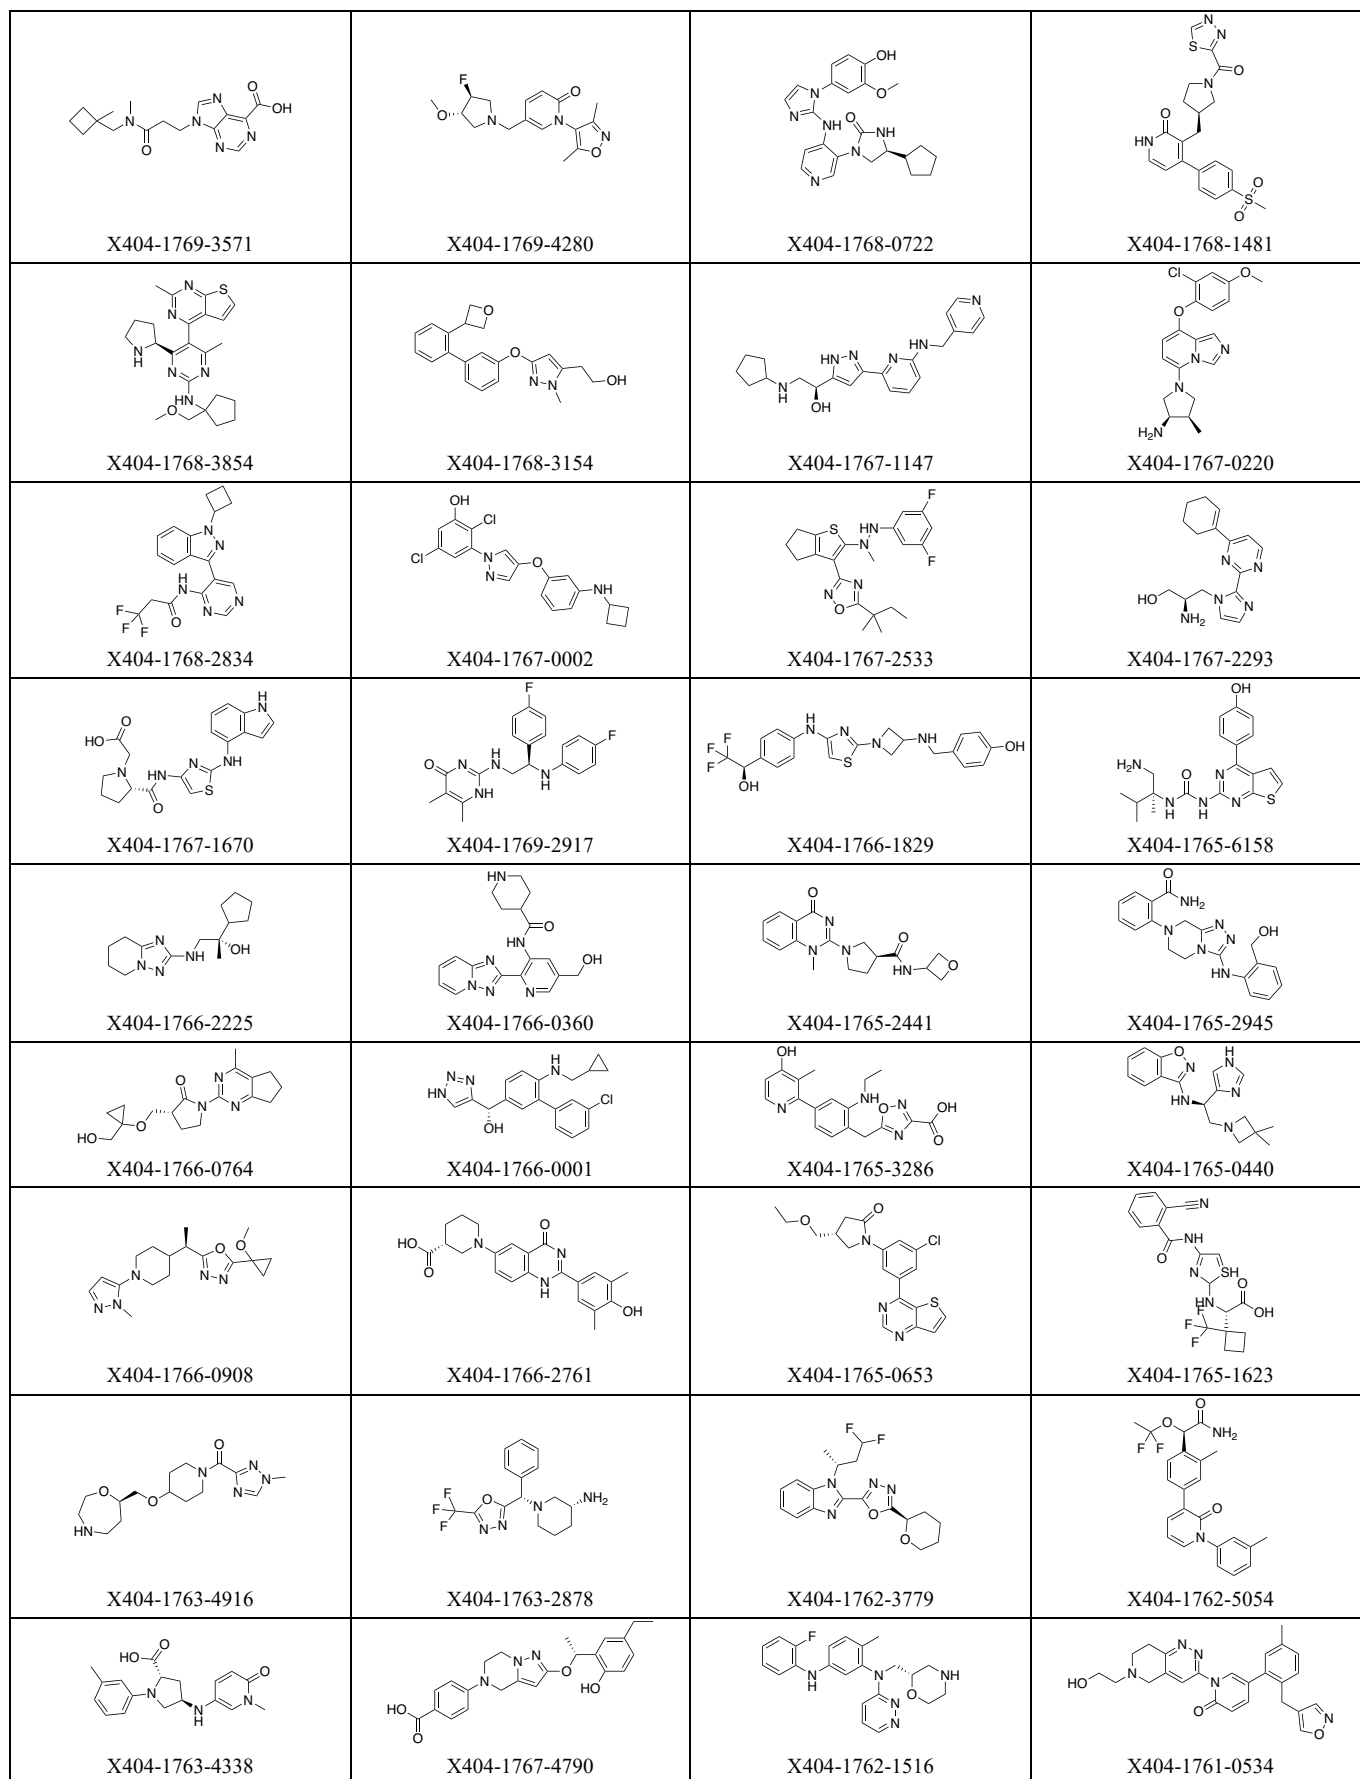 |

|                                                                                     |                                                                                     |                                                                                      |                                                                                       |
|-------------------------------------------------------------------------------------|-------------------------------------------------------------------------------------|--------------------------------------------------------------------------------------|---------------------------------------------------------------------------------------|
| 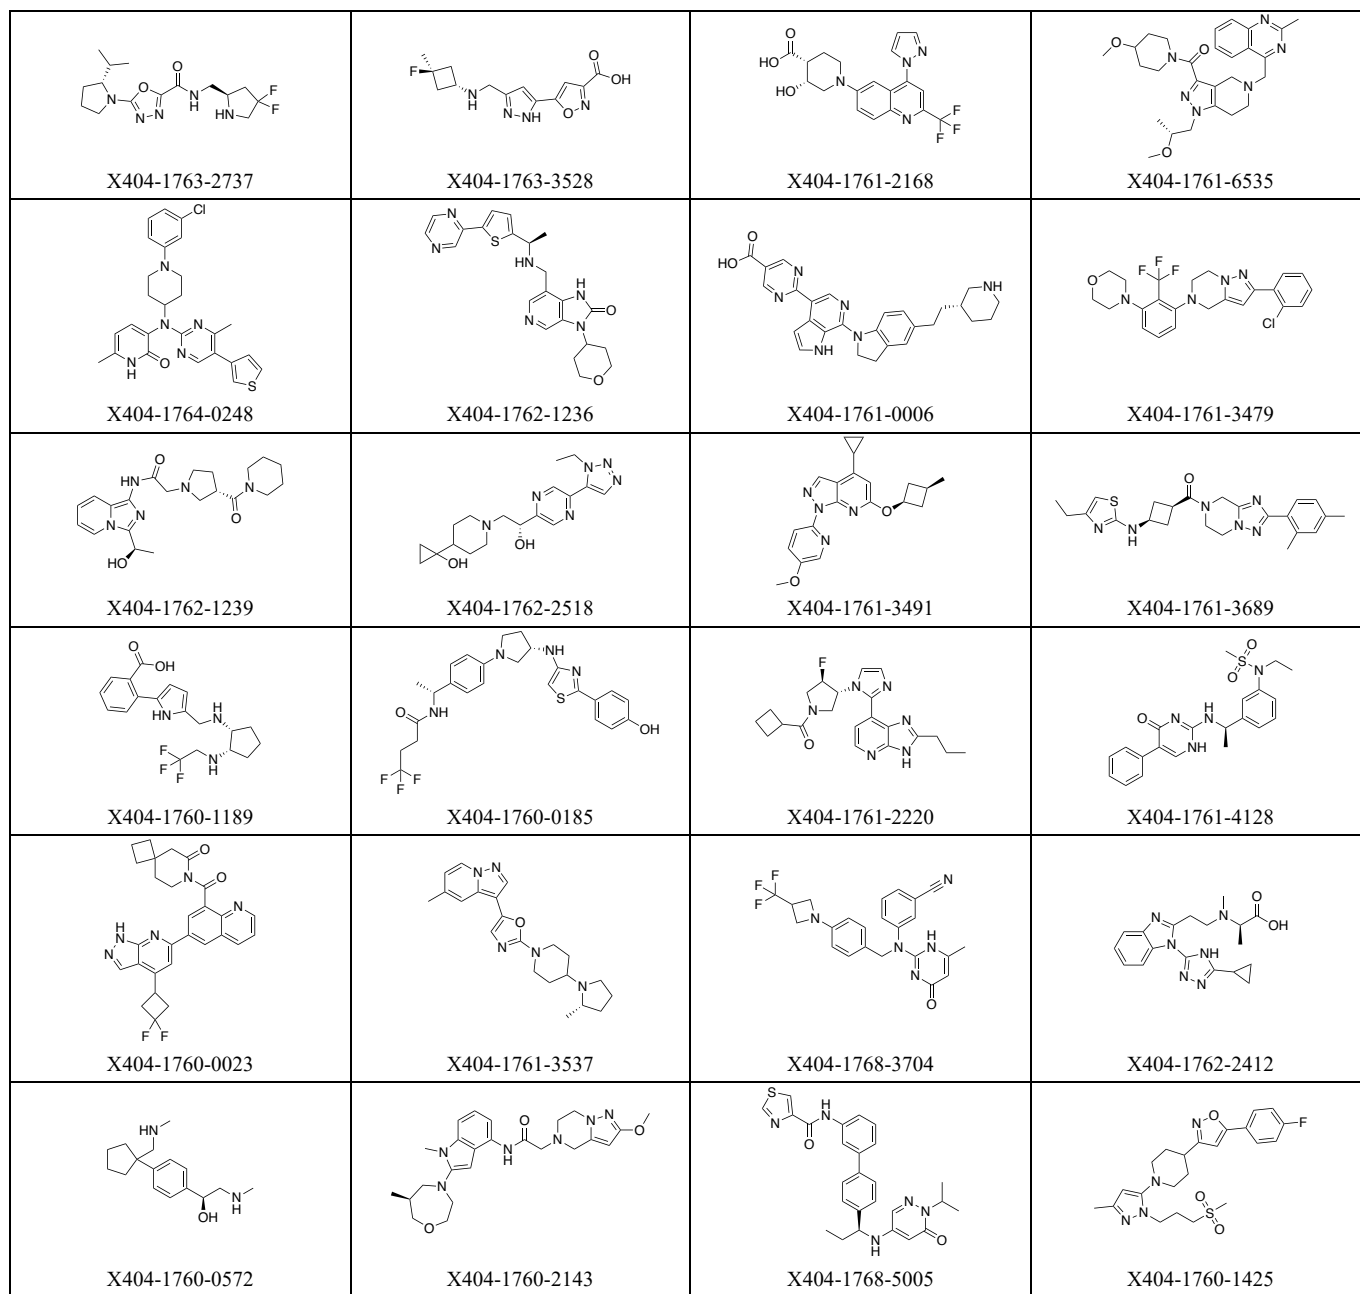   | 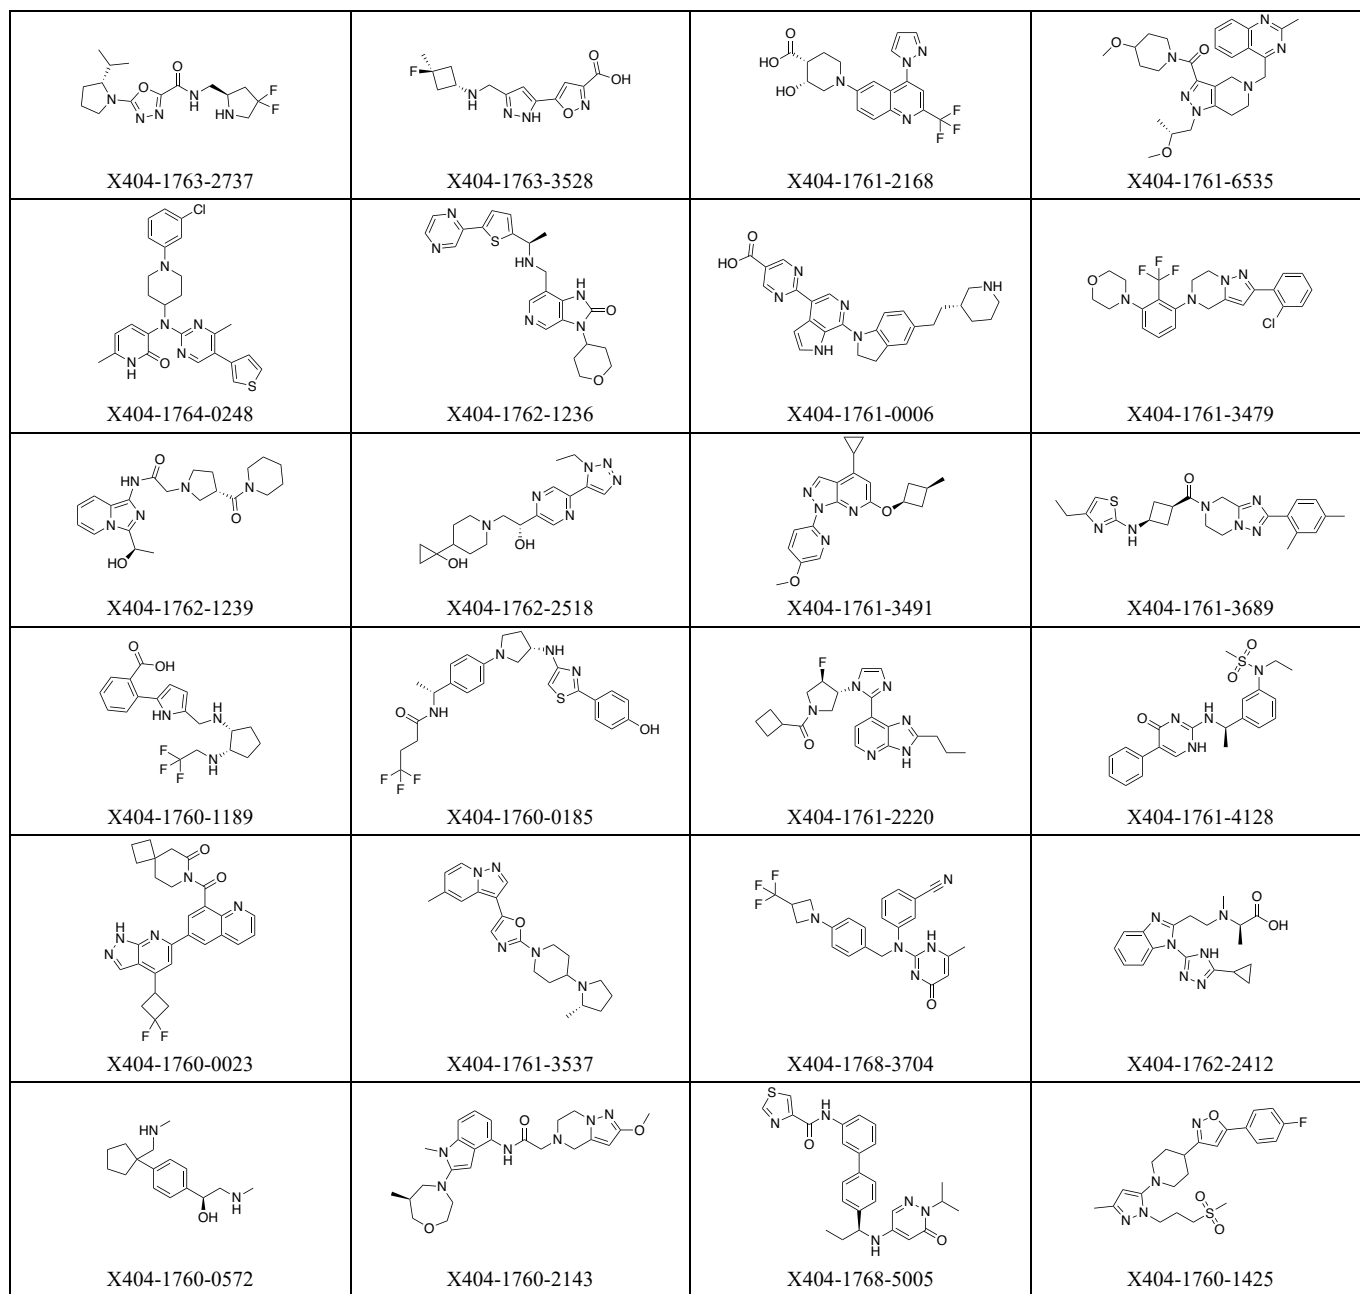   | 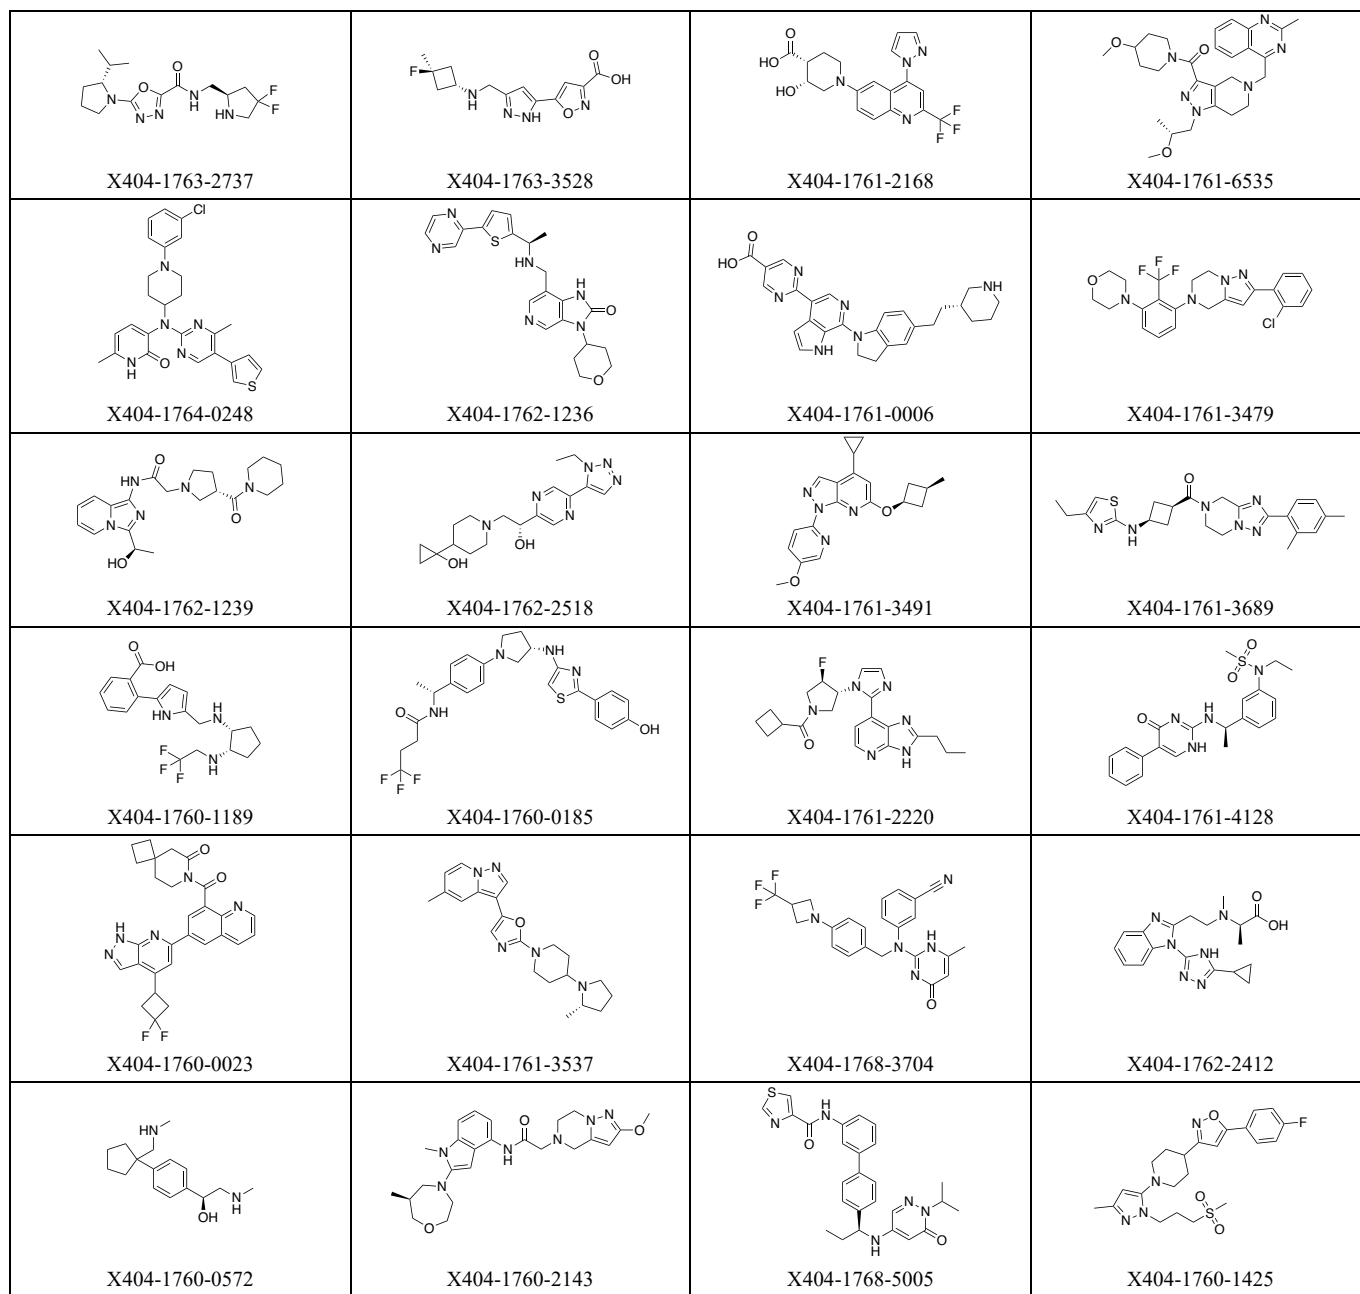   | 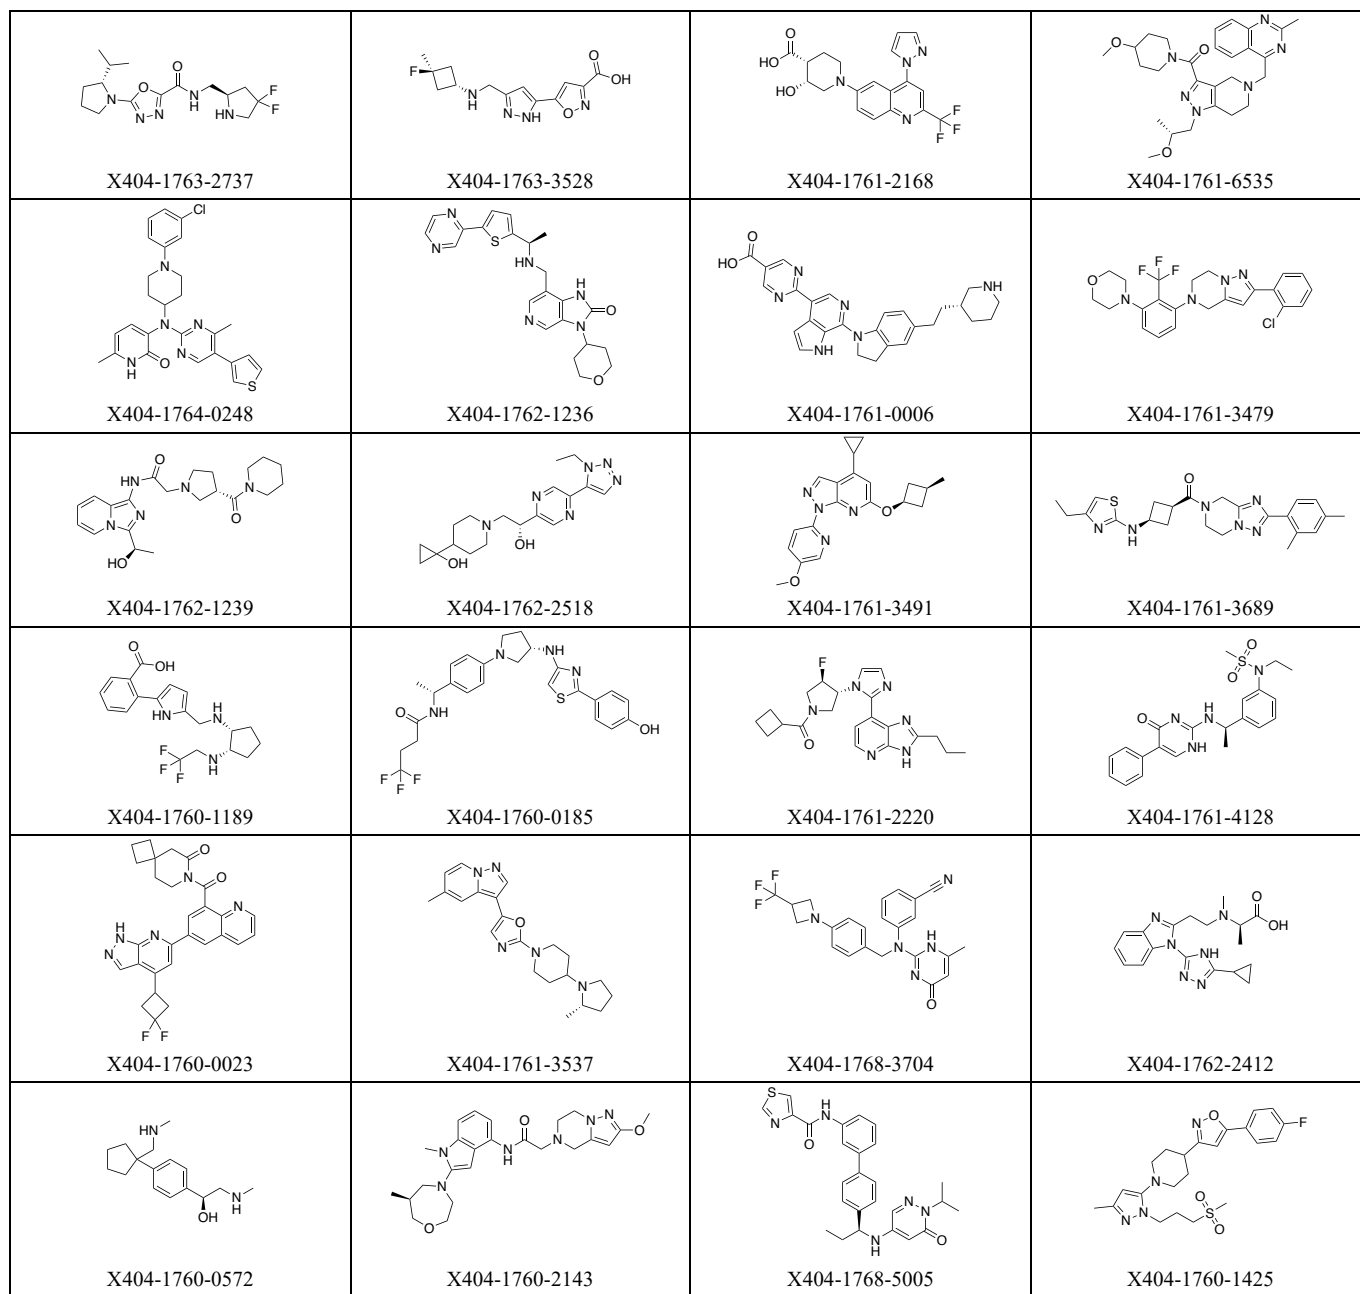   |
| <b>X404-1763-2737</b>                                                               | <b>X404-1763-3528</b>                                                               | <b>X404-1761-2168</b>                                                                | <b>X404-1761-6535</b>                                                                 |
| 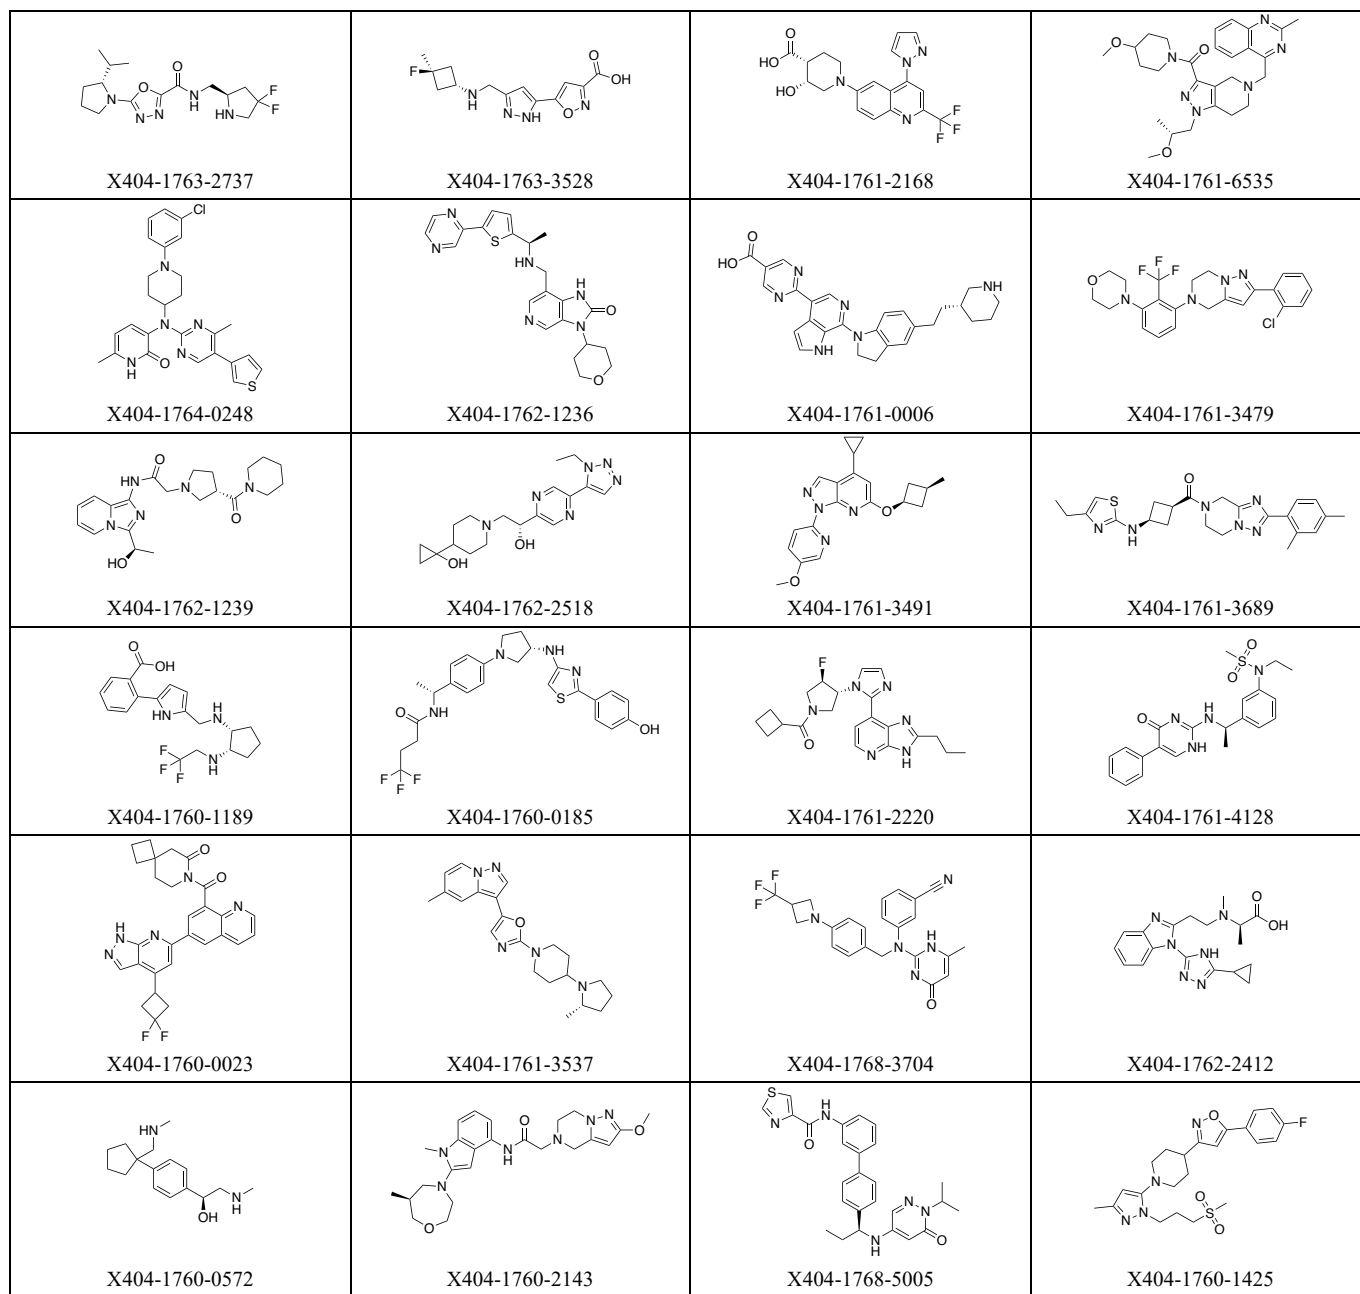   | 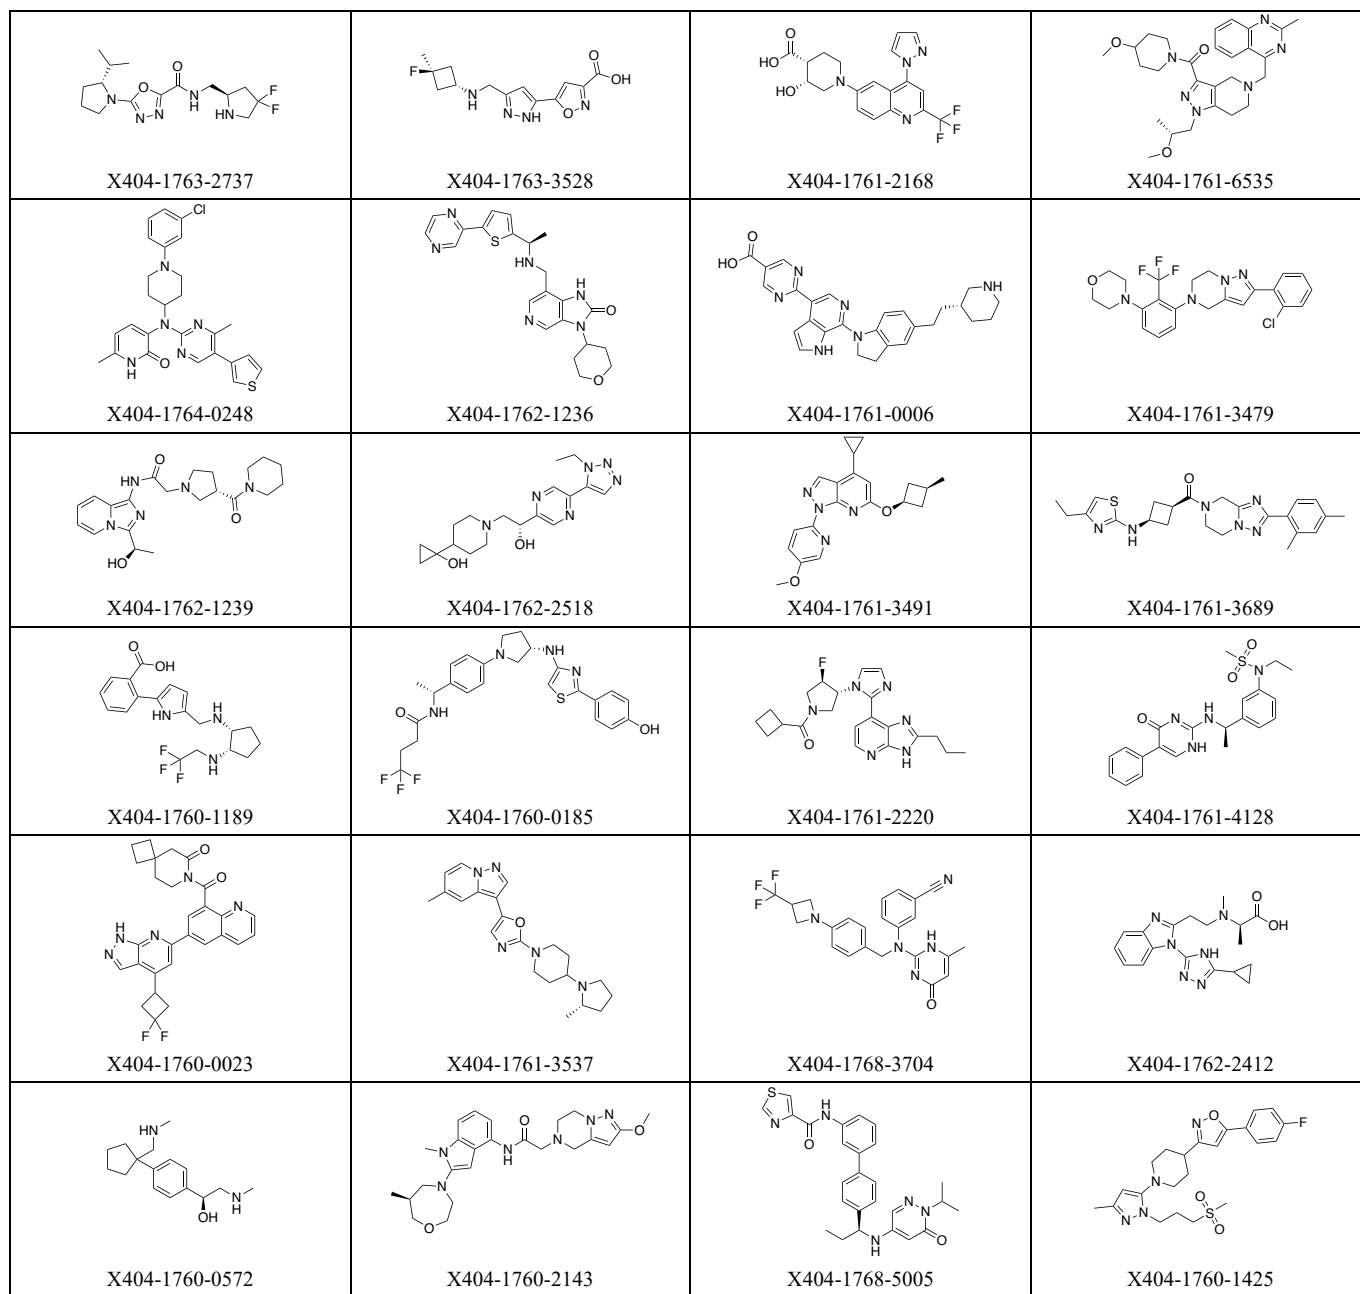   | 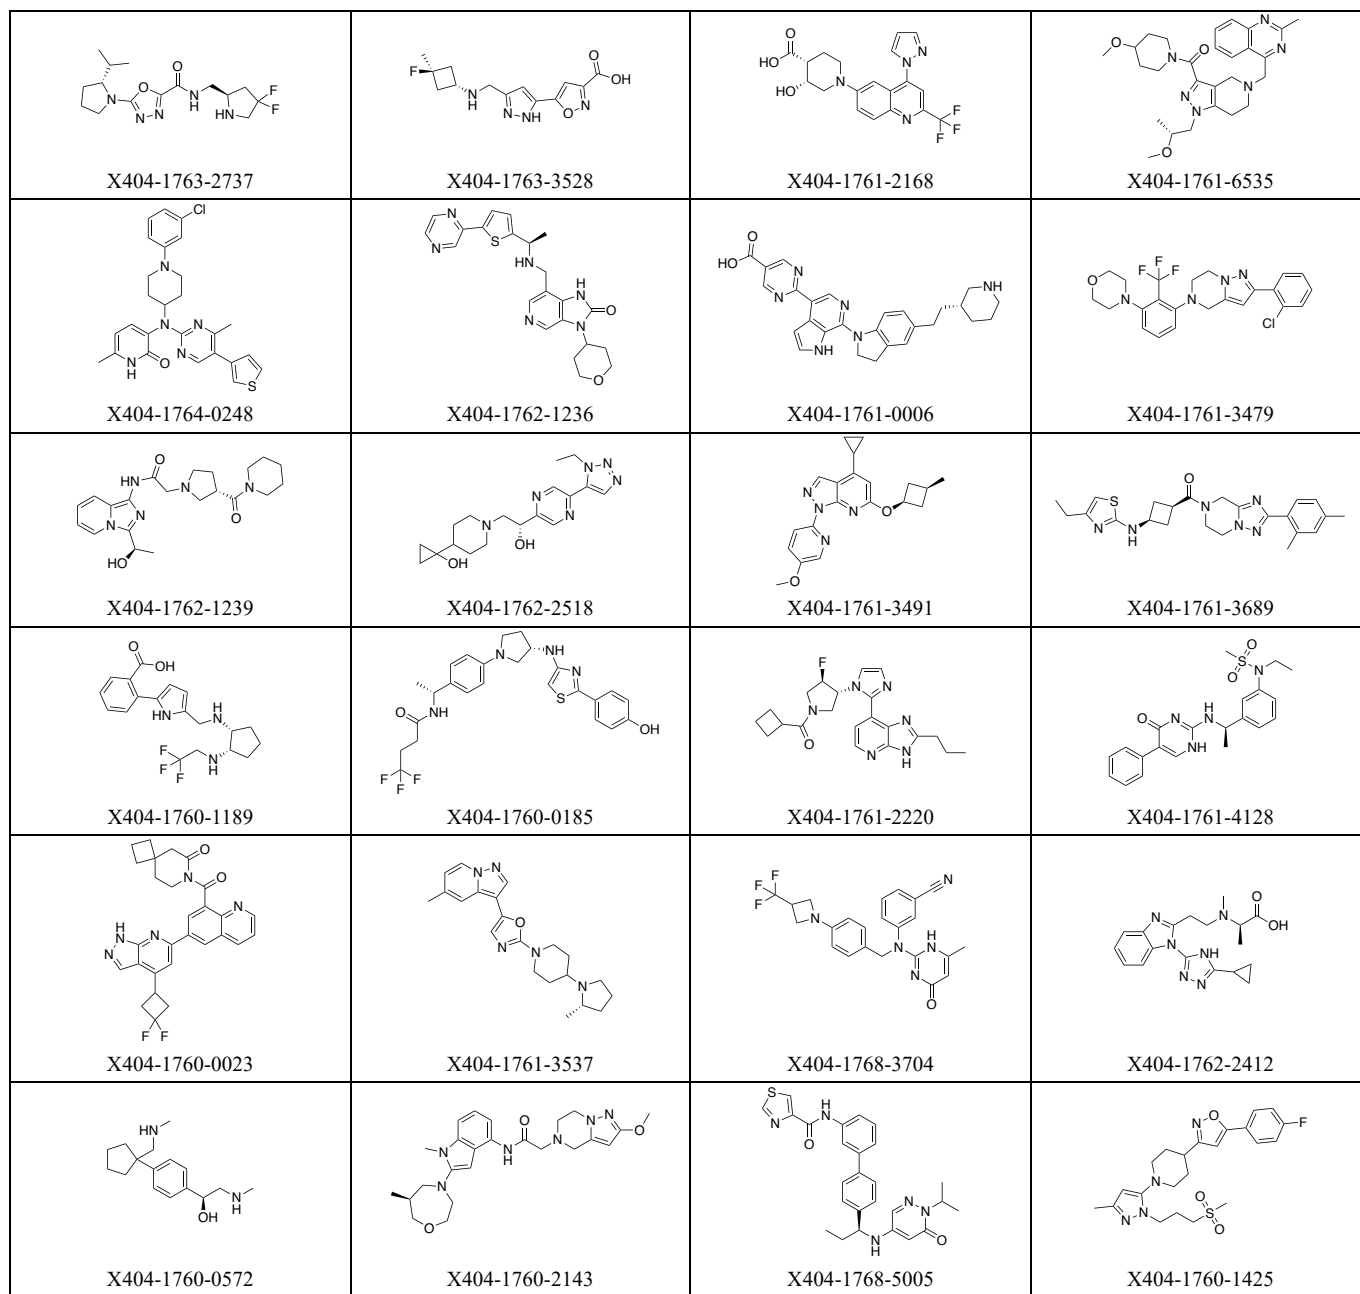   | 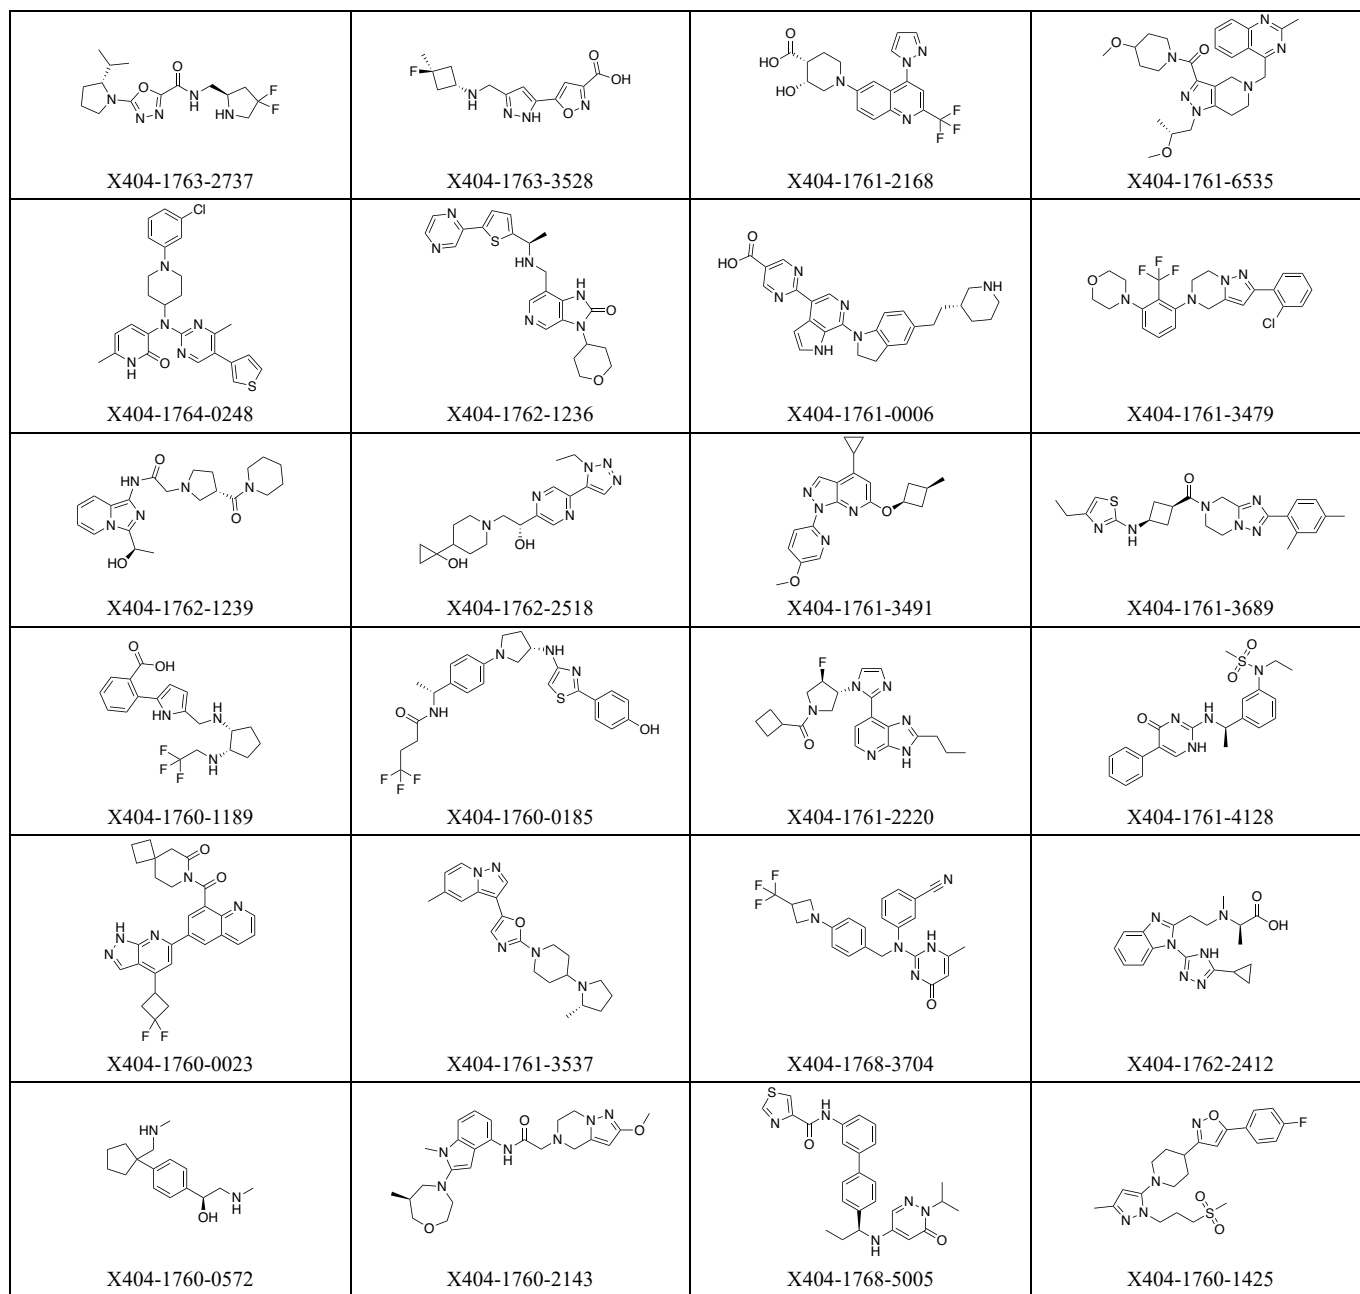   |
| <b>X404-1764-0248</b>                                                               | <b>X404-1762-1236</b>                                                               | <b>X404-1761-0006</b>                                                                | <b>X404-1761-3479</b>                                                                 |
| 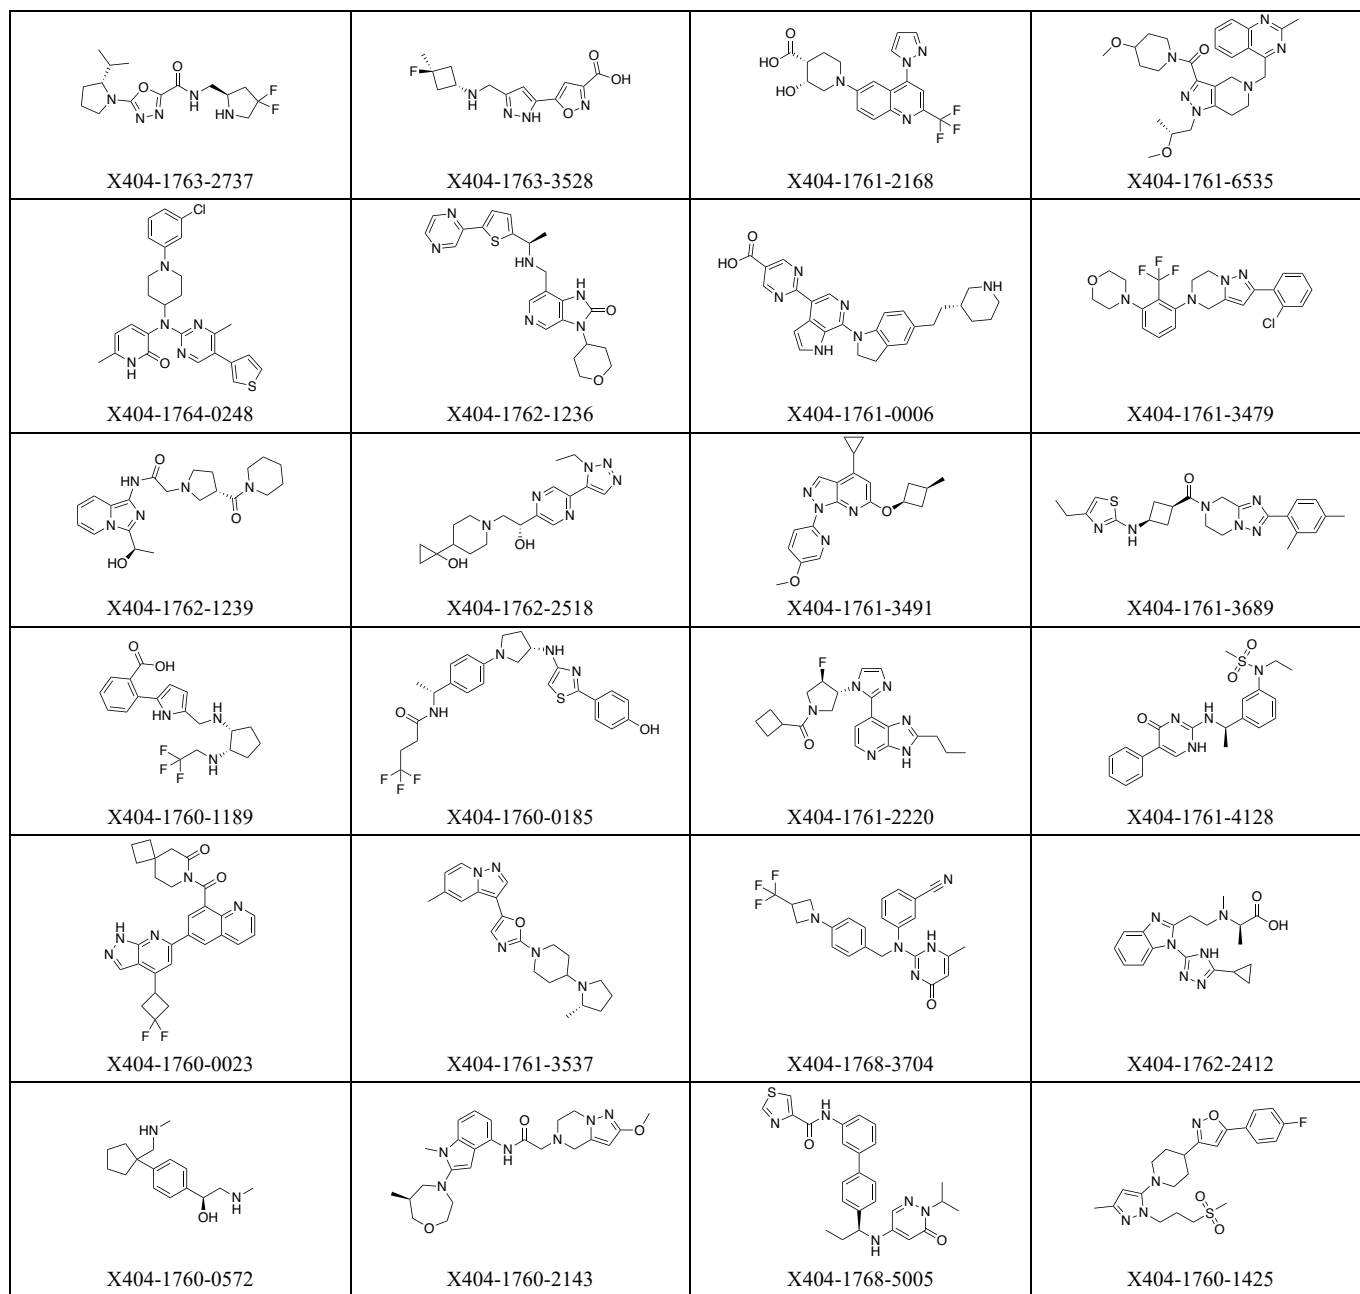   | 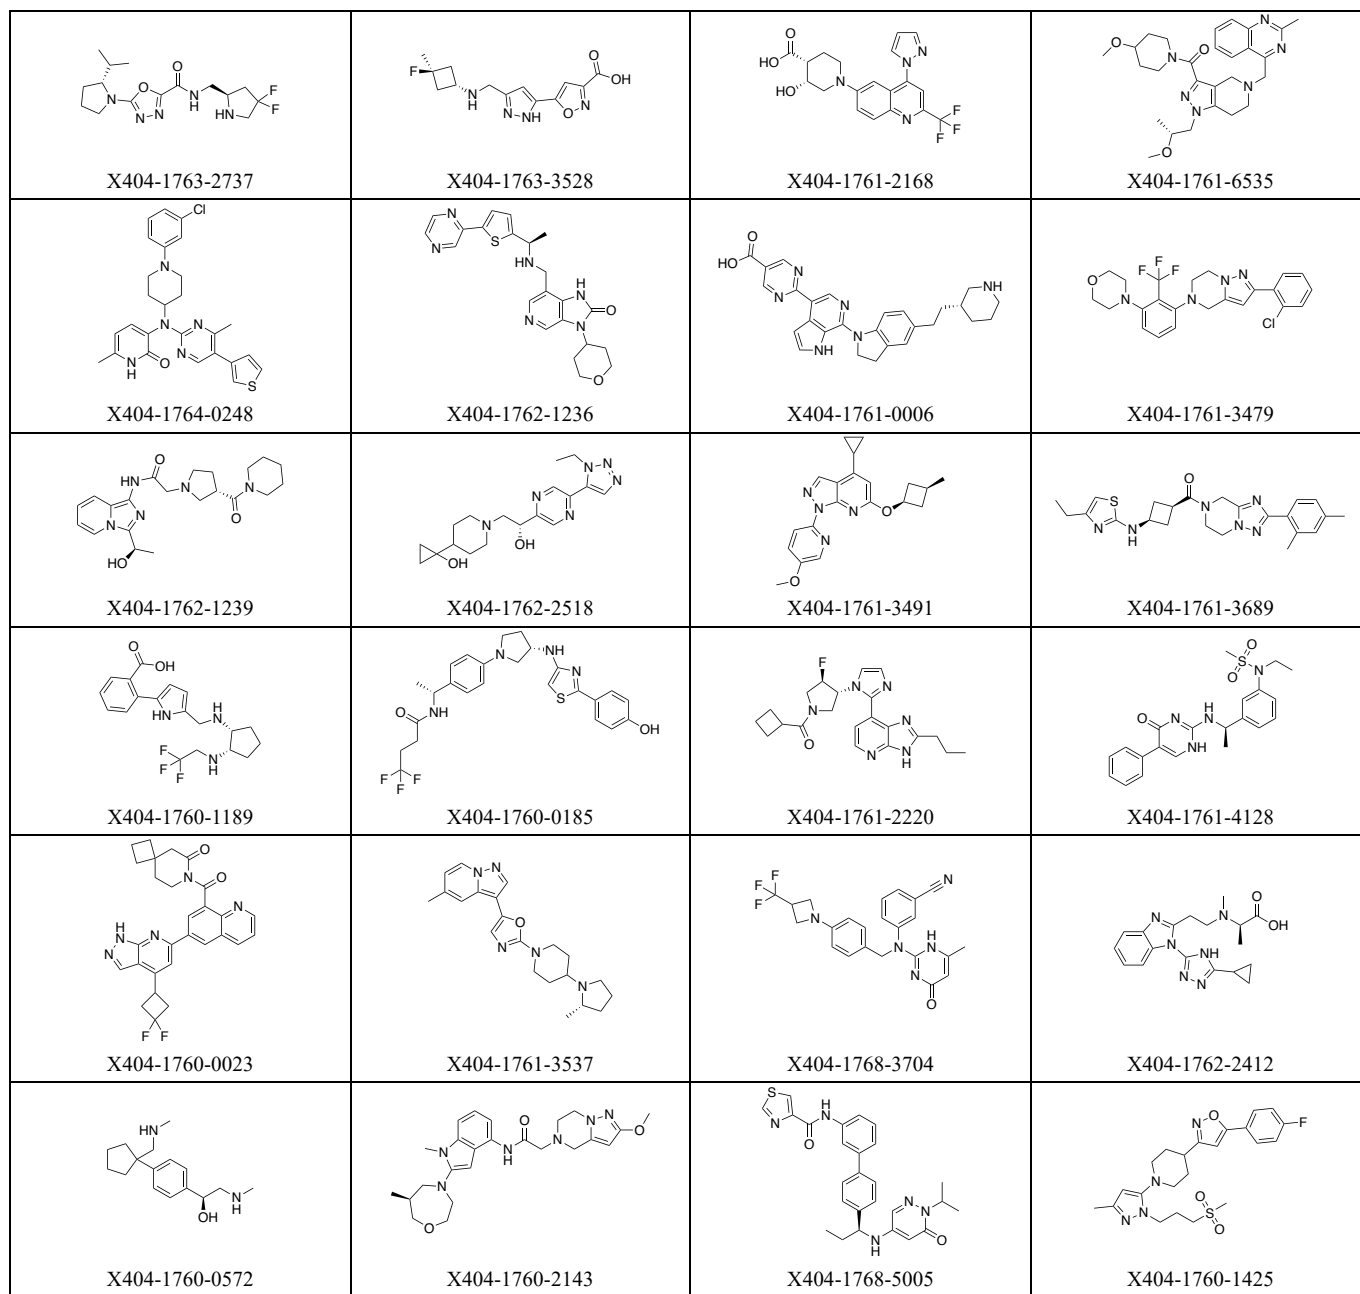   | 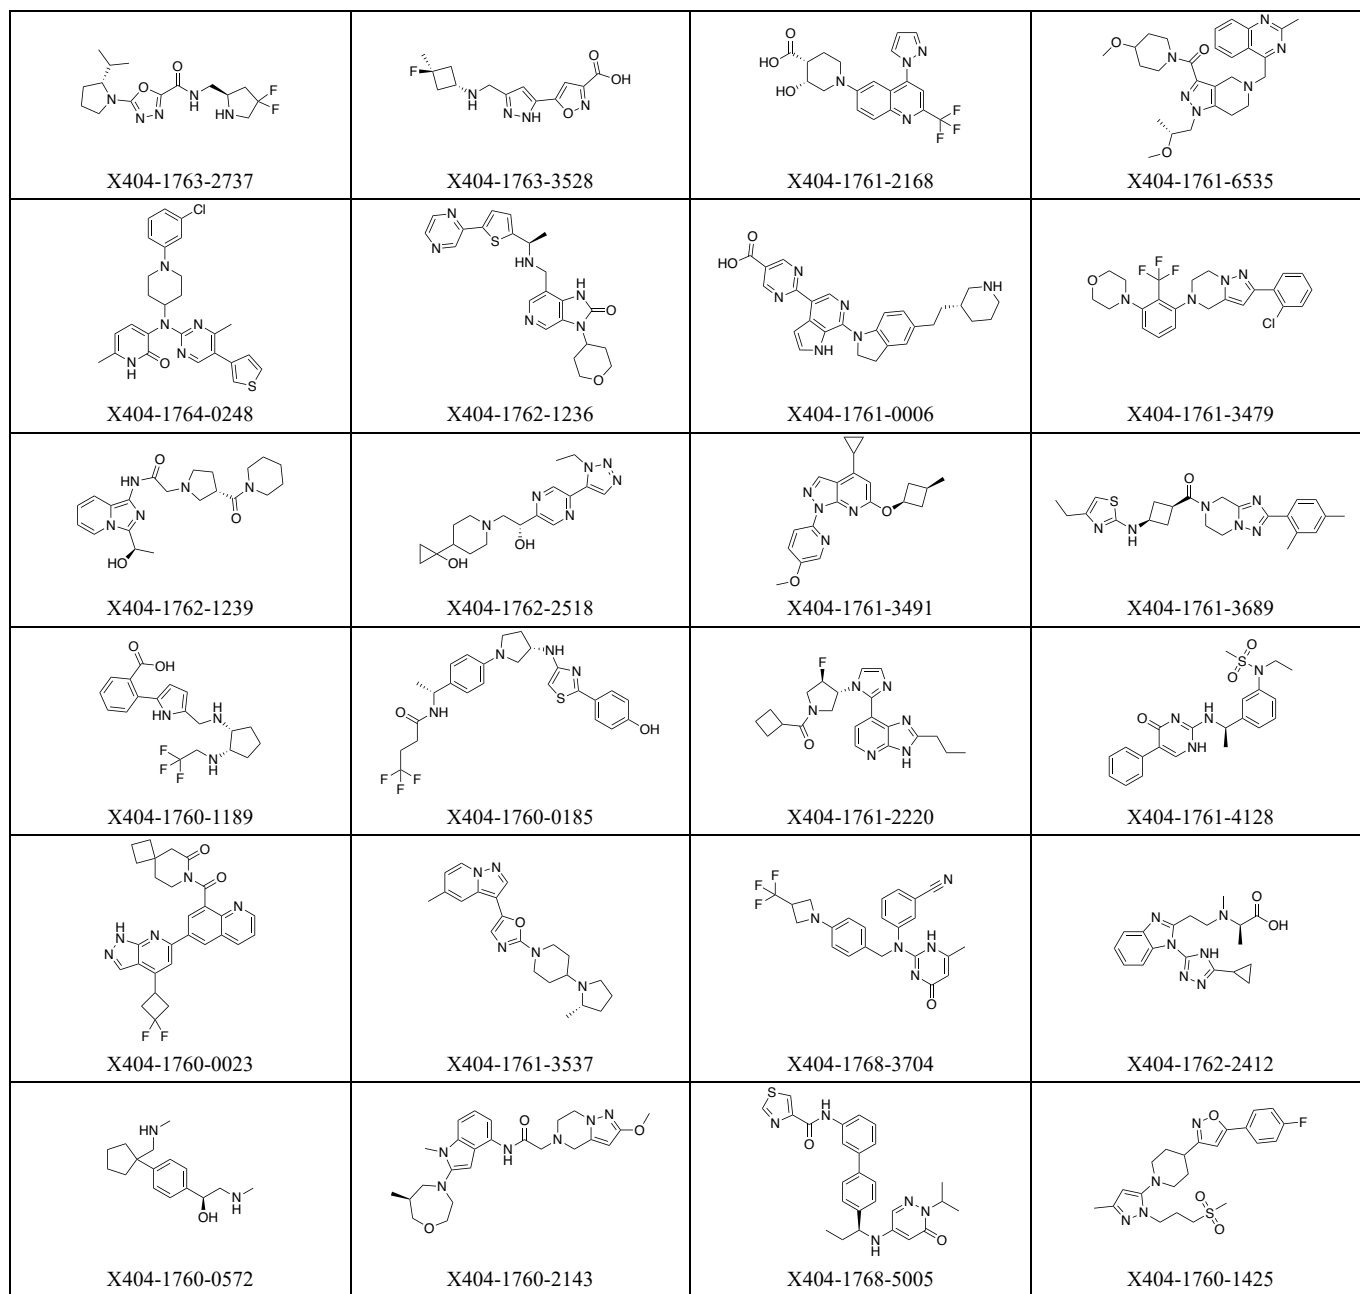   | 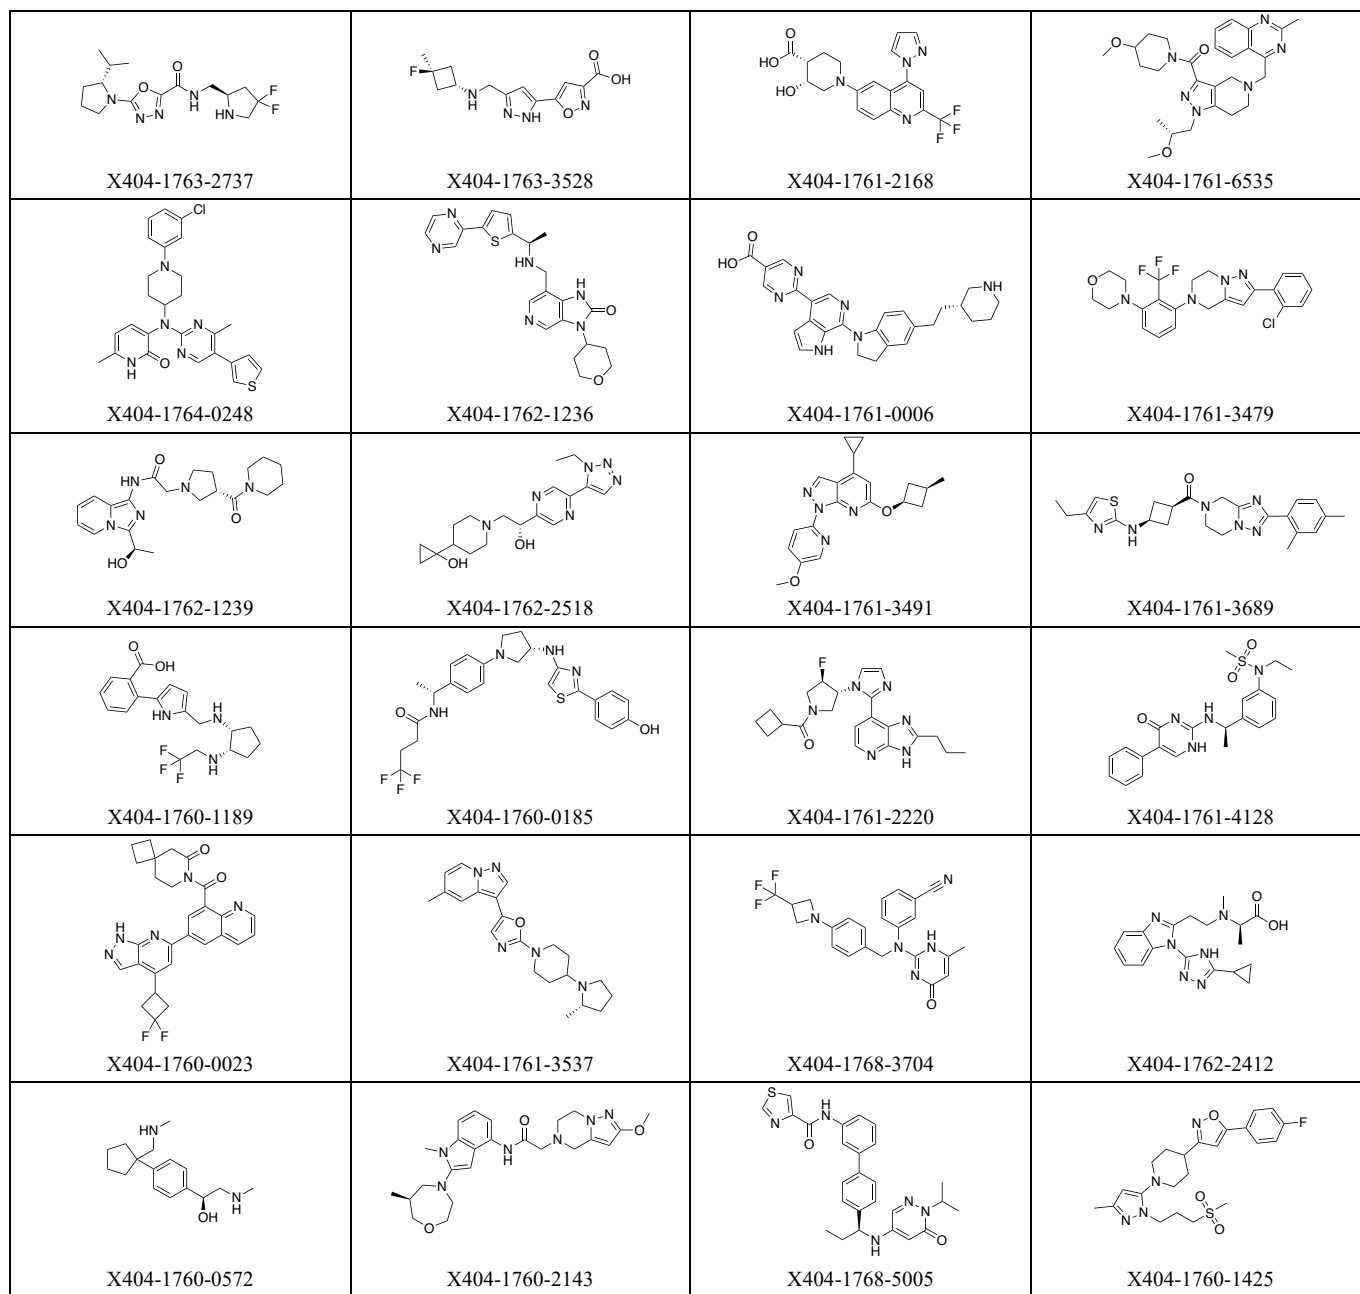   |
| <b>X404-1762-1239</b>                                                               | <b>X404-1762-2518</b>                                                               | <b>X404-1761-3491</b>                                                                | <b>X404-1761-3689</b>                                                                 |
| 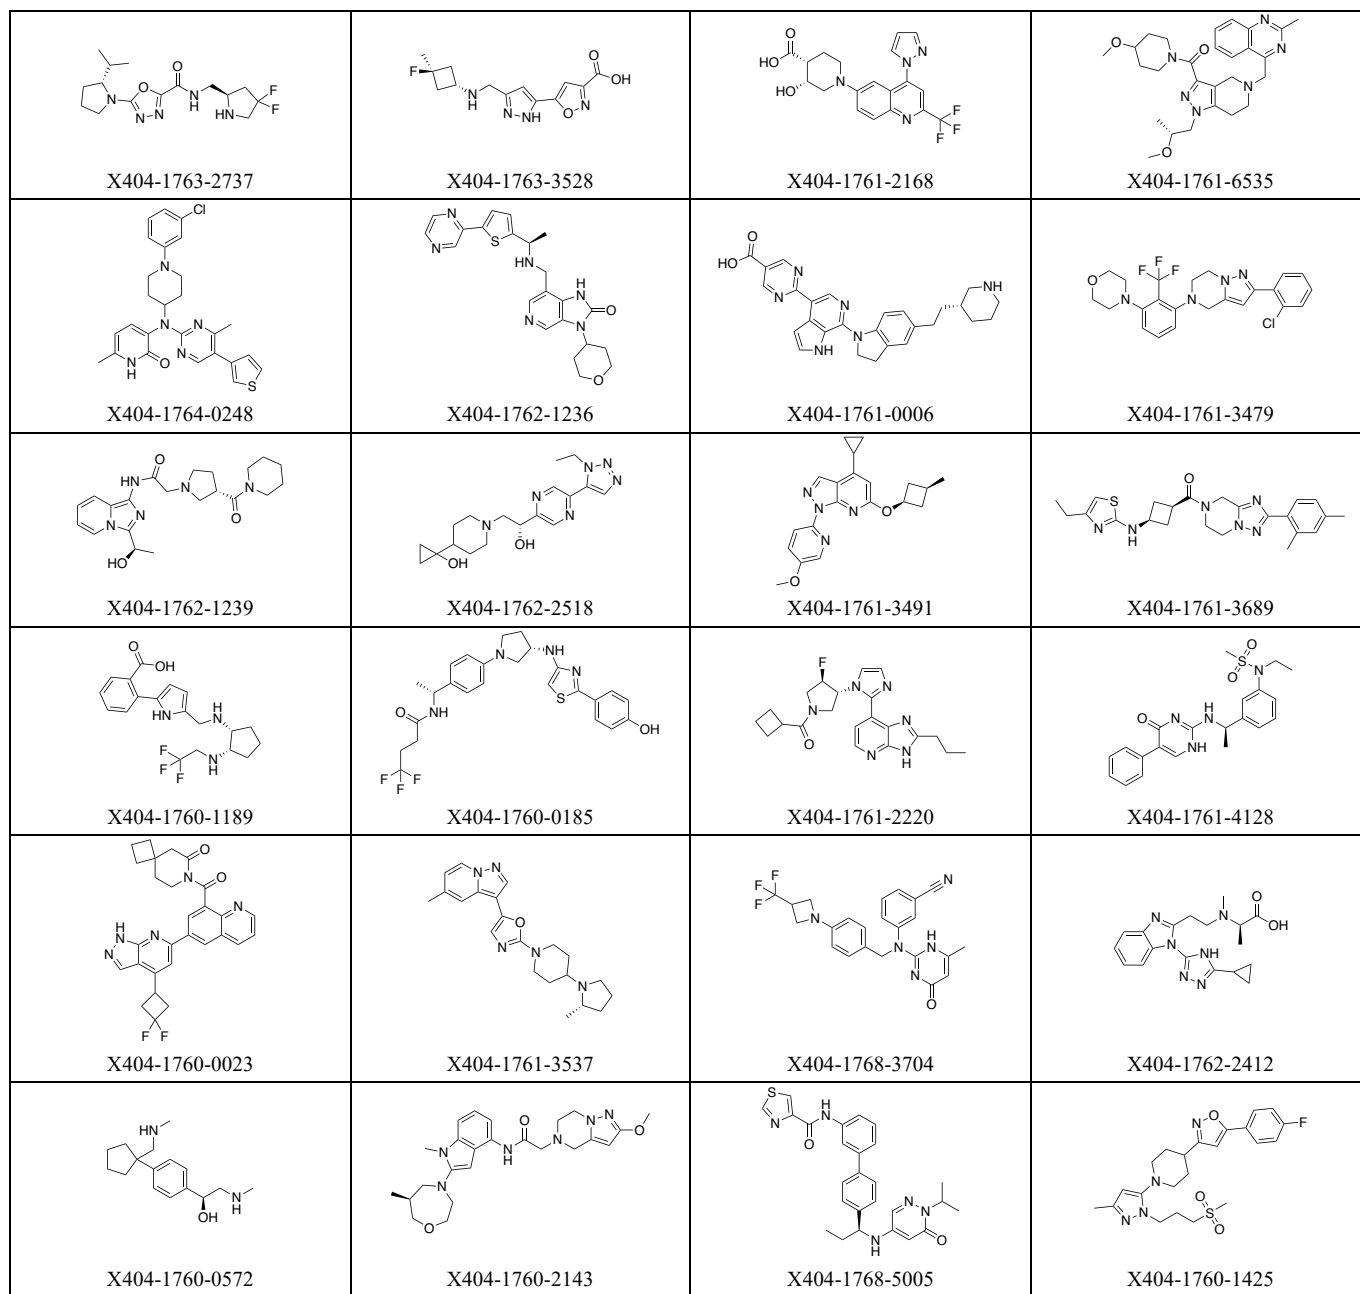   | 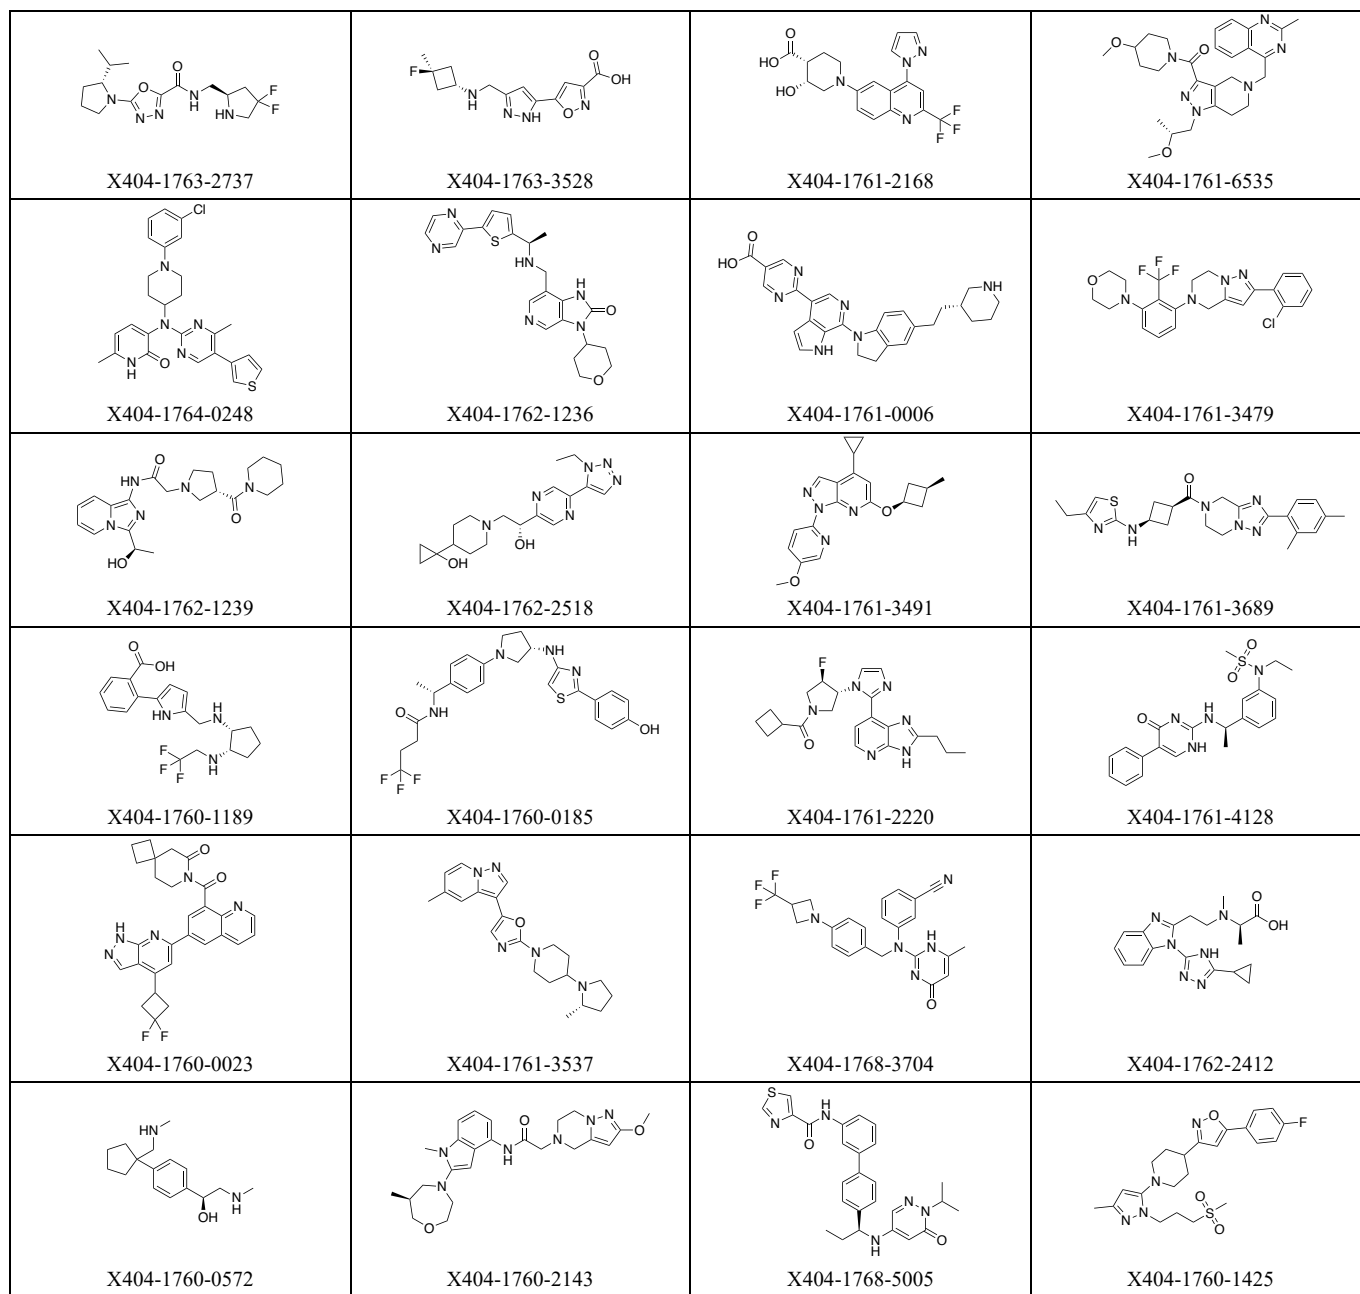   | 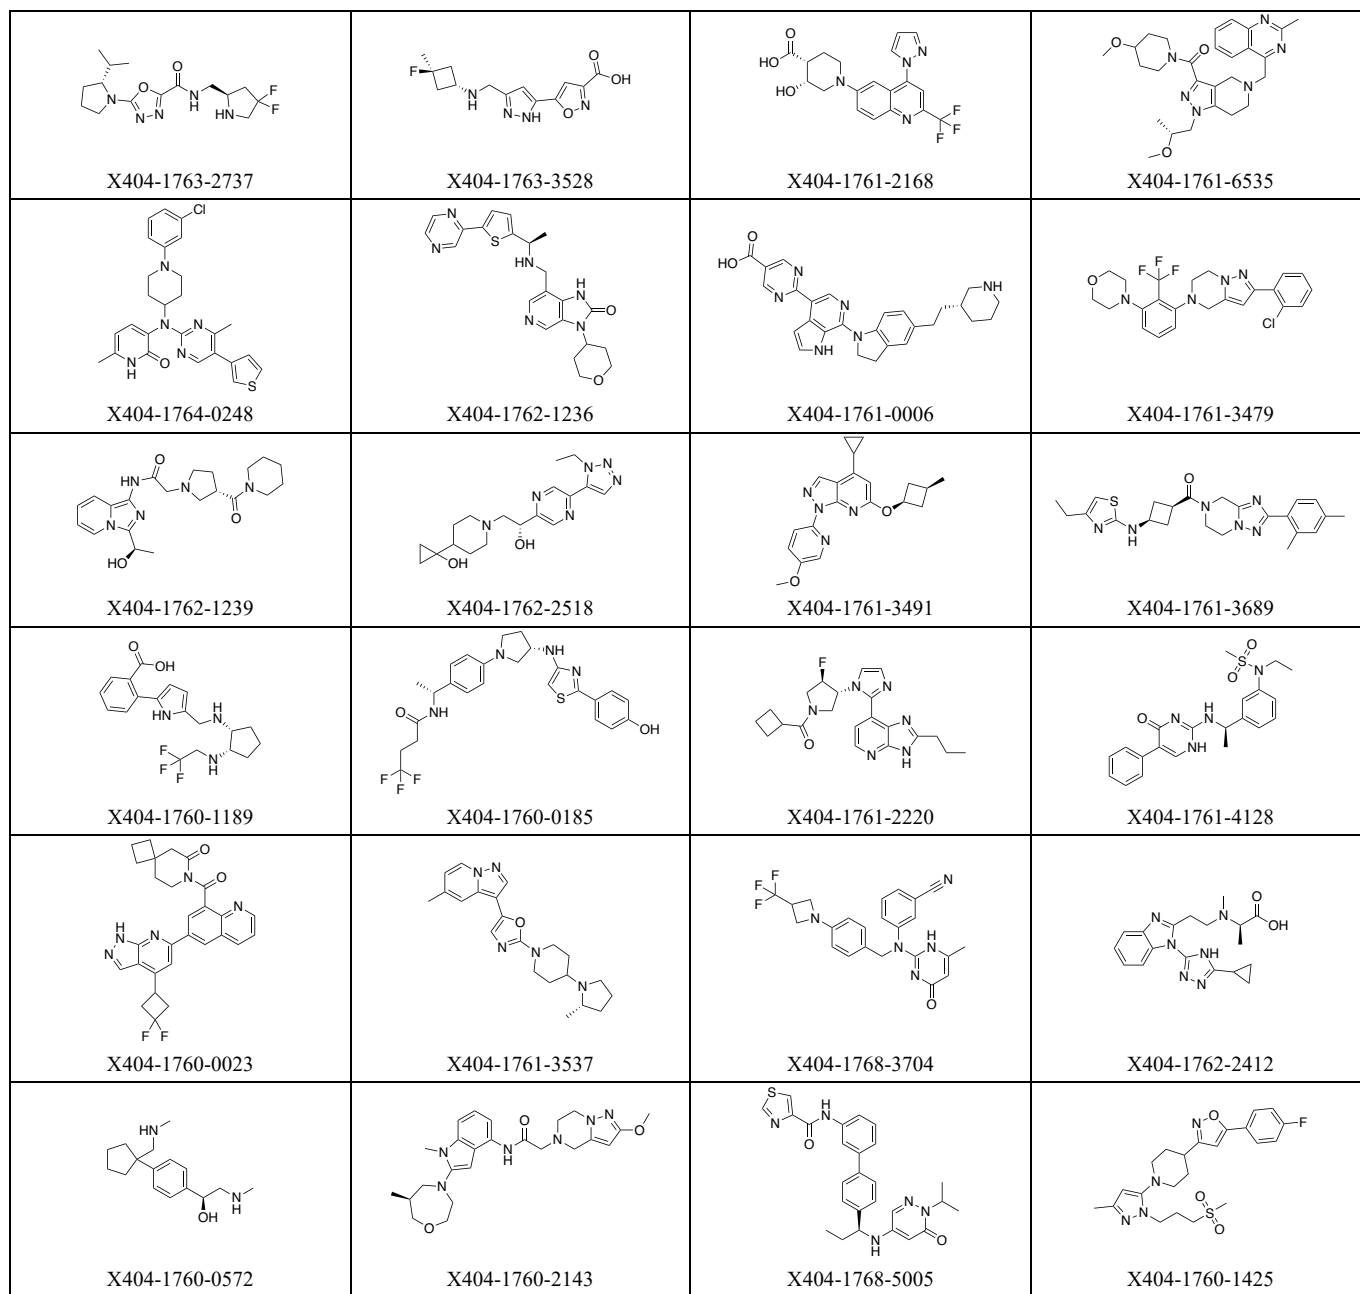   | 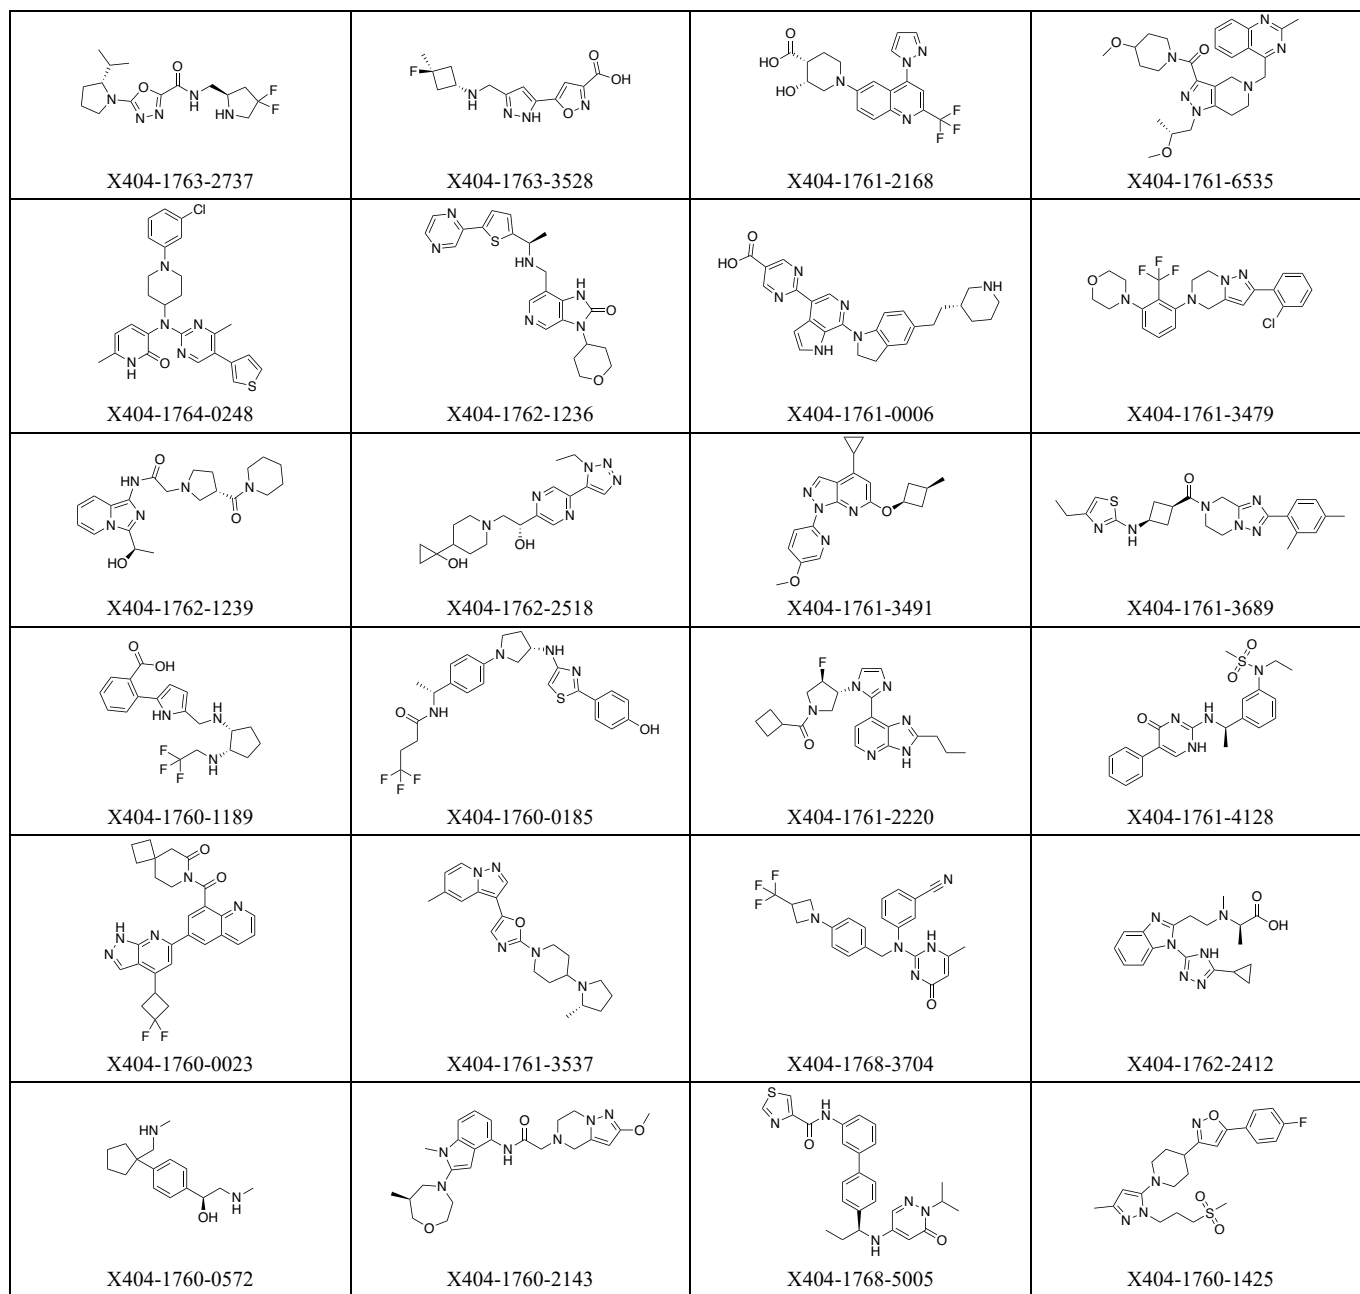   |
| <b>X404-1760-1189</b>                                                               | <b>X404-1760-0185</b>                                                               | <b>X404-1761-2220</b>                                                                | <b>X404-1761-4128</b>                                                                 |
| 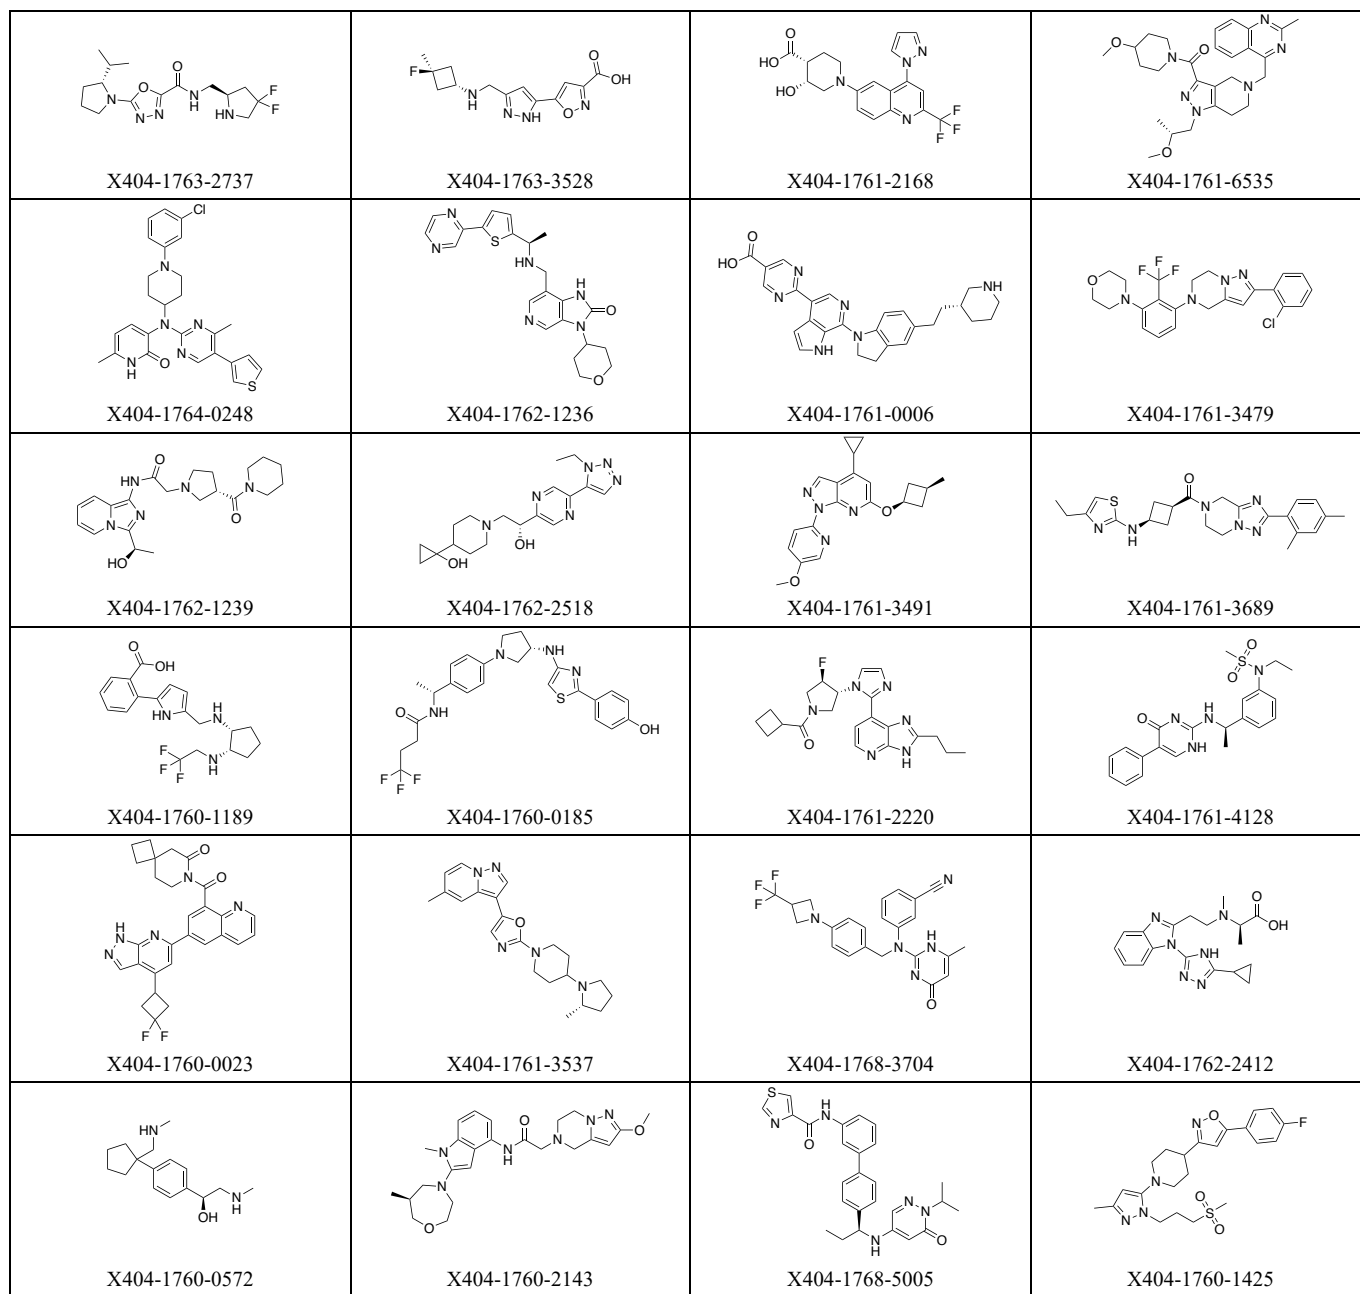  | 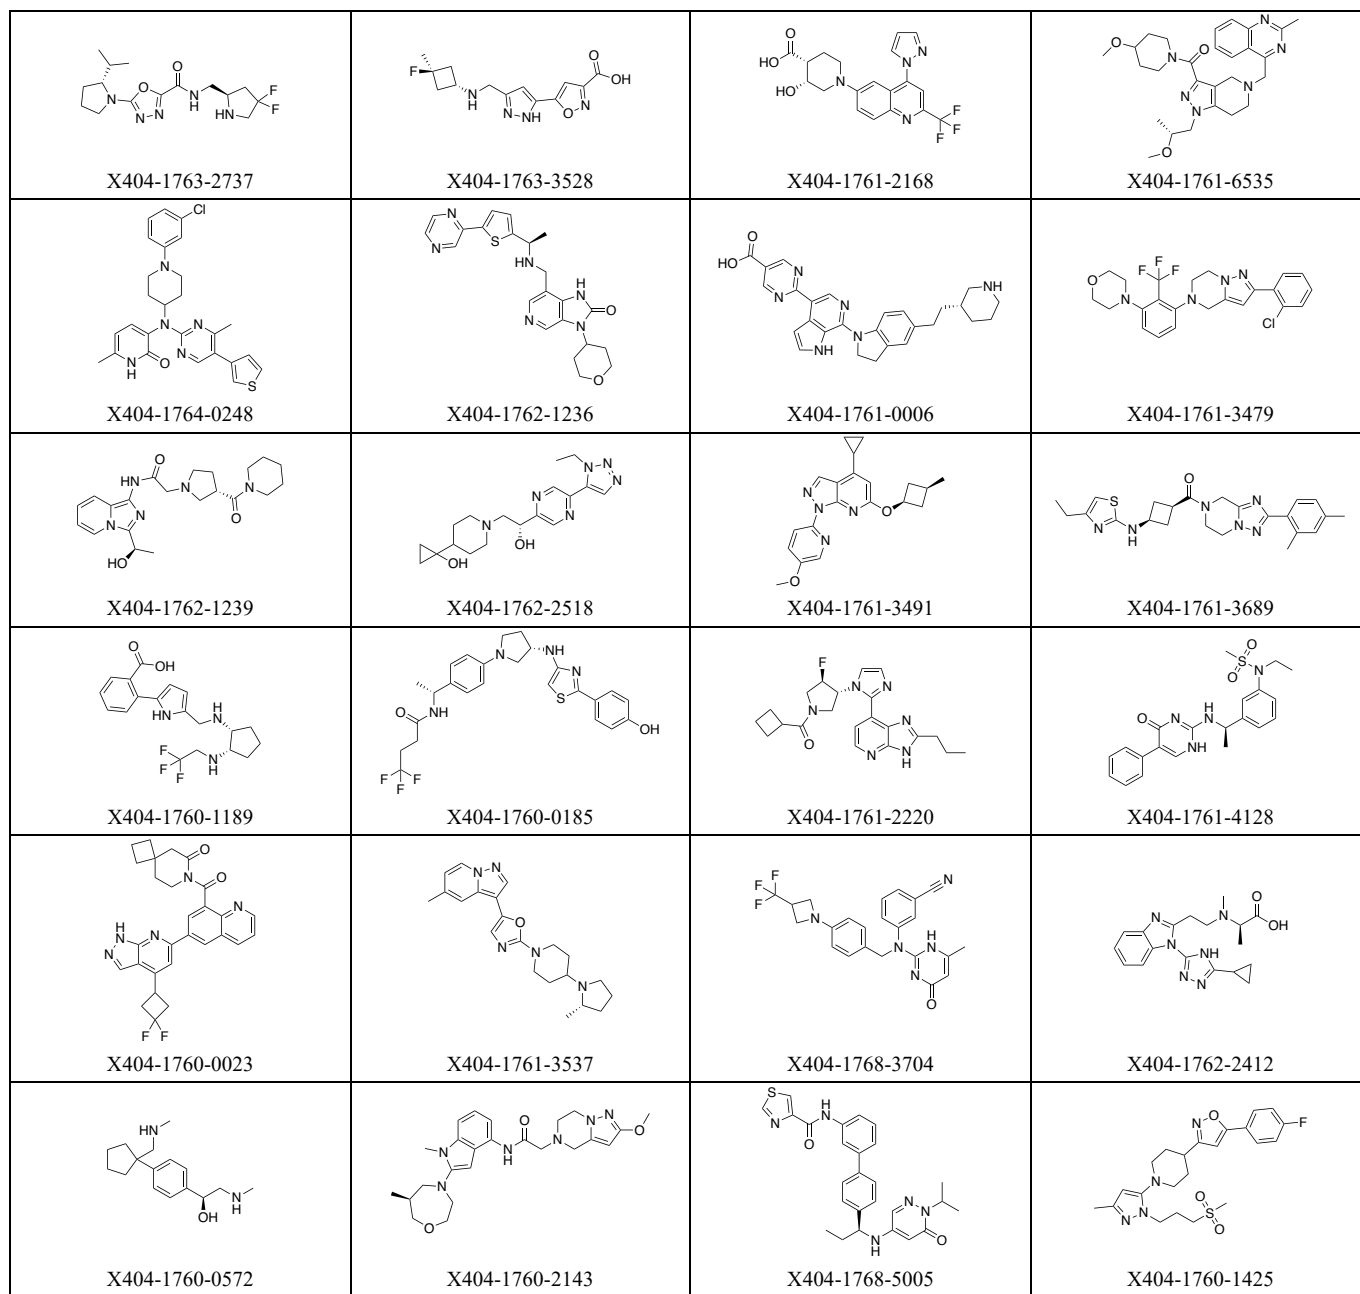  | 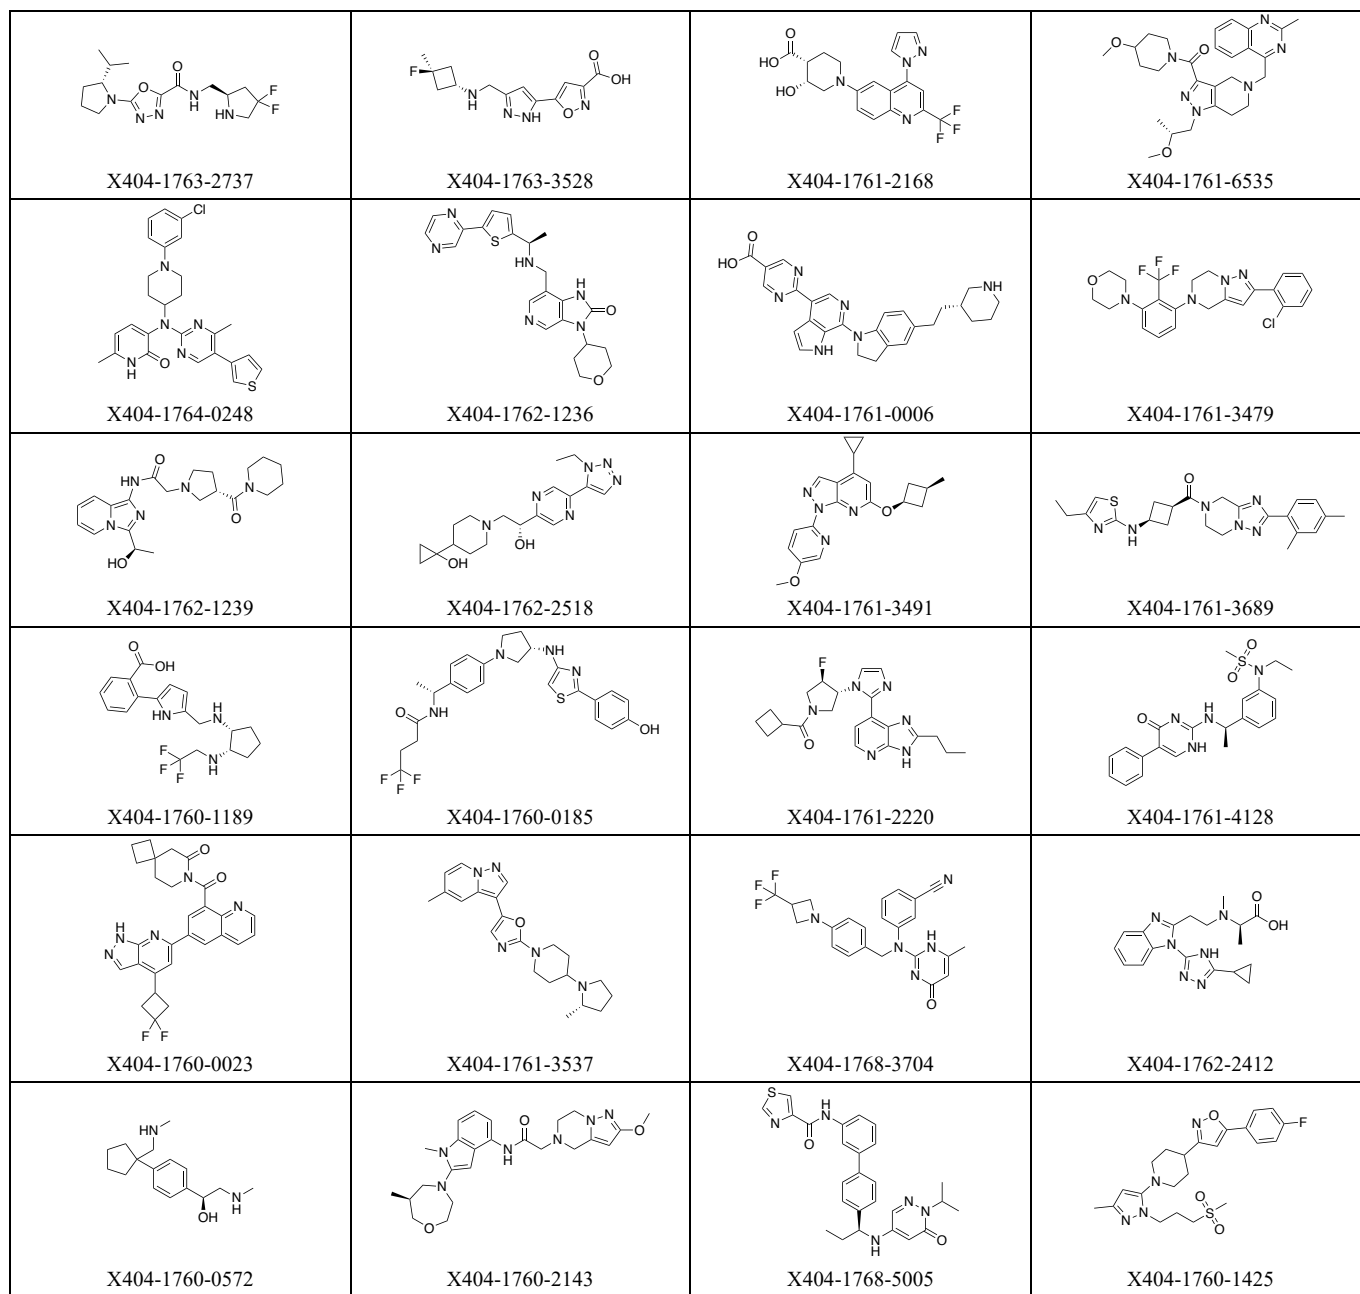  | 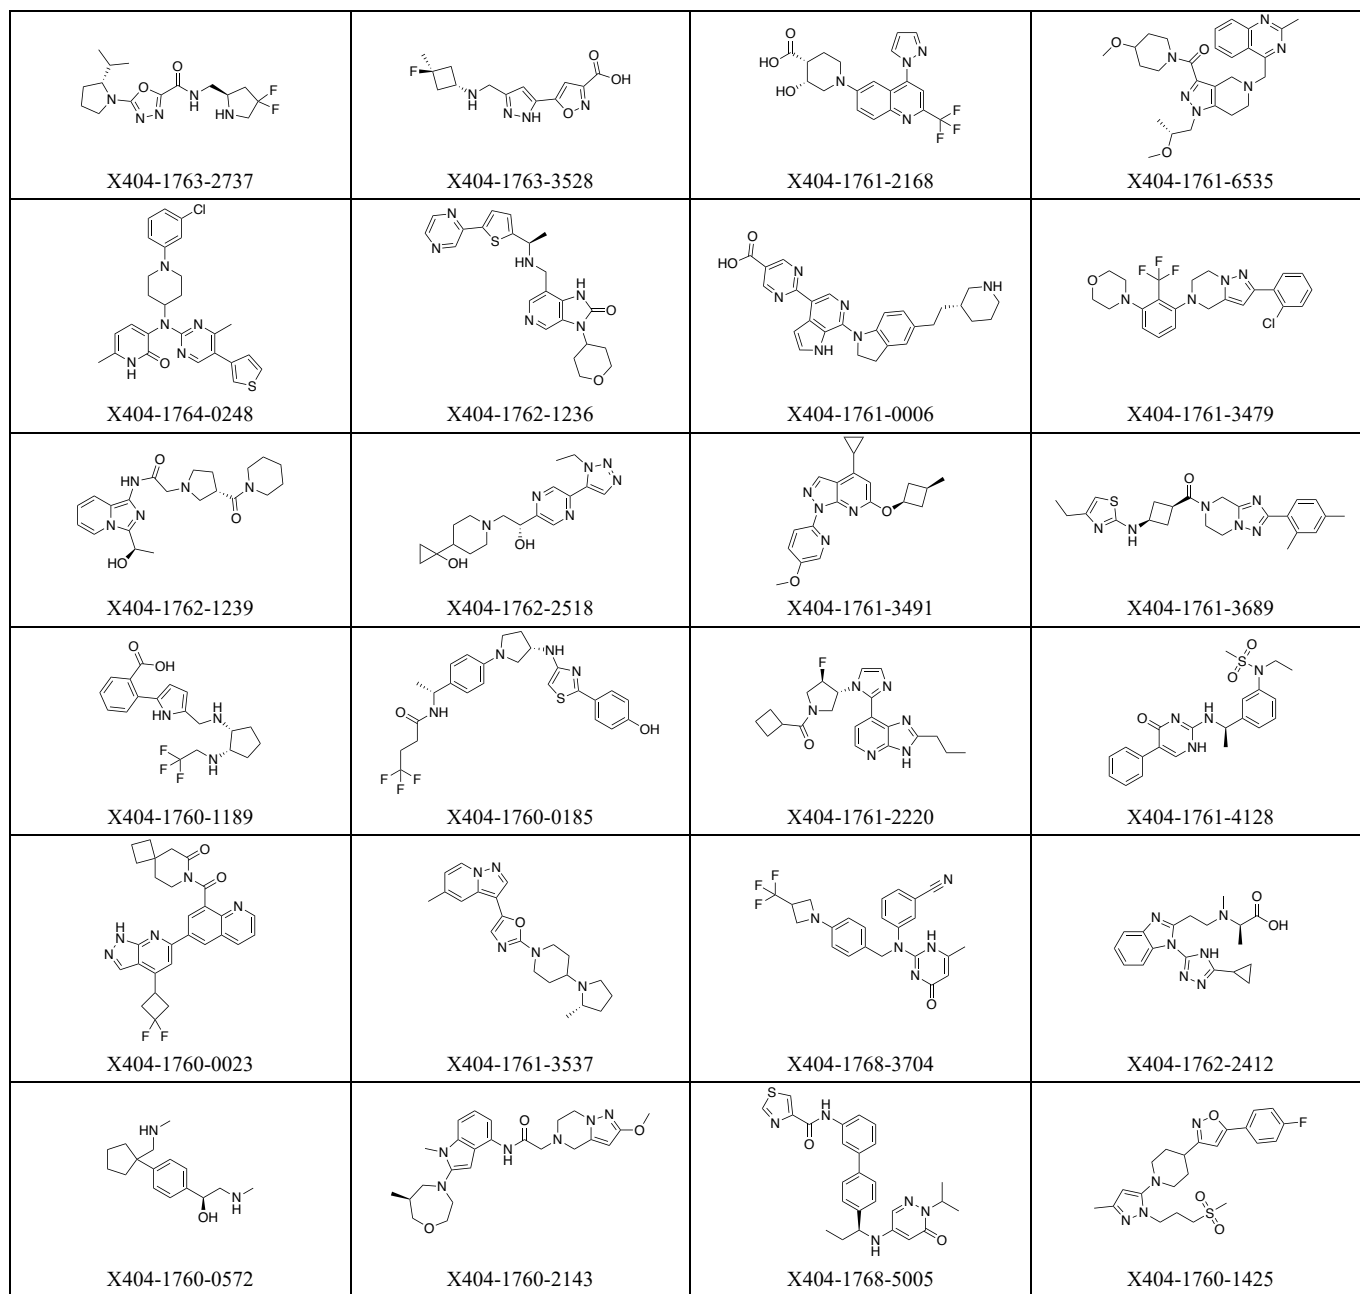 |
| <b>X404-1760-0023</b>                                                               | <b>X404-1761-3537</b>                                                               | <b>X404-1768-3704</b>                                                                | <b>X404-1762-2412</b>                                                                 |
| 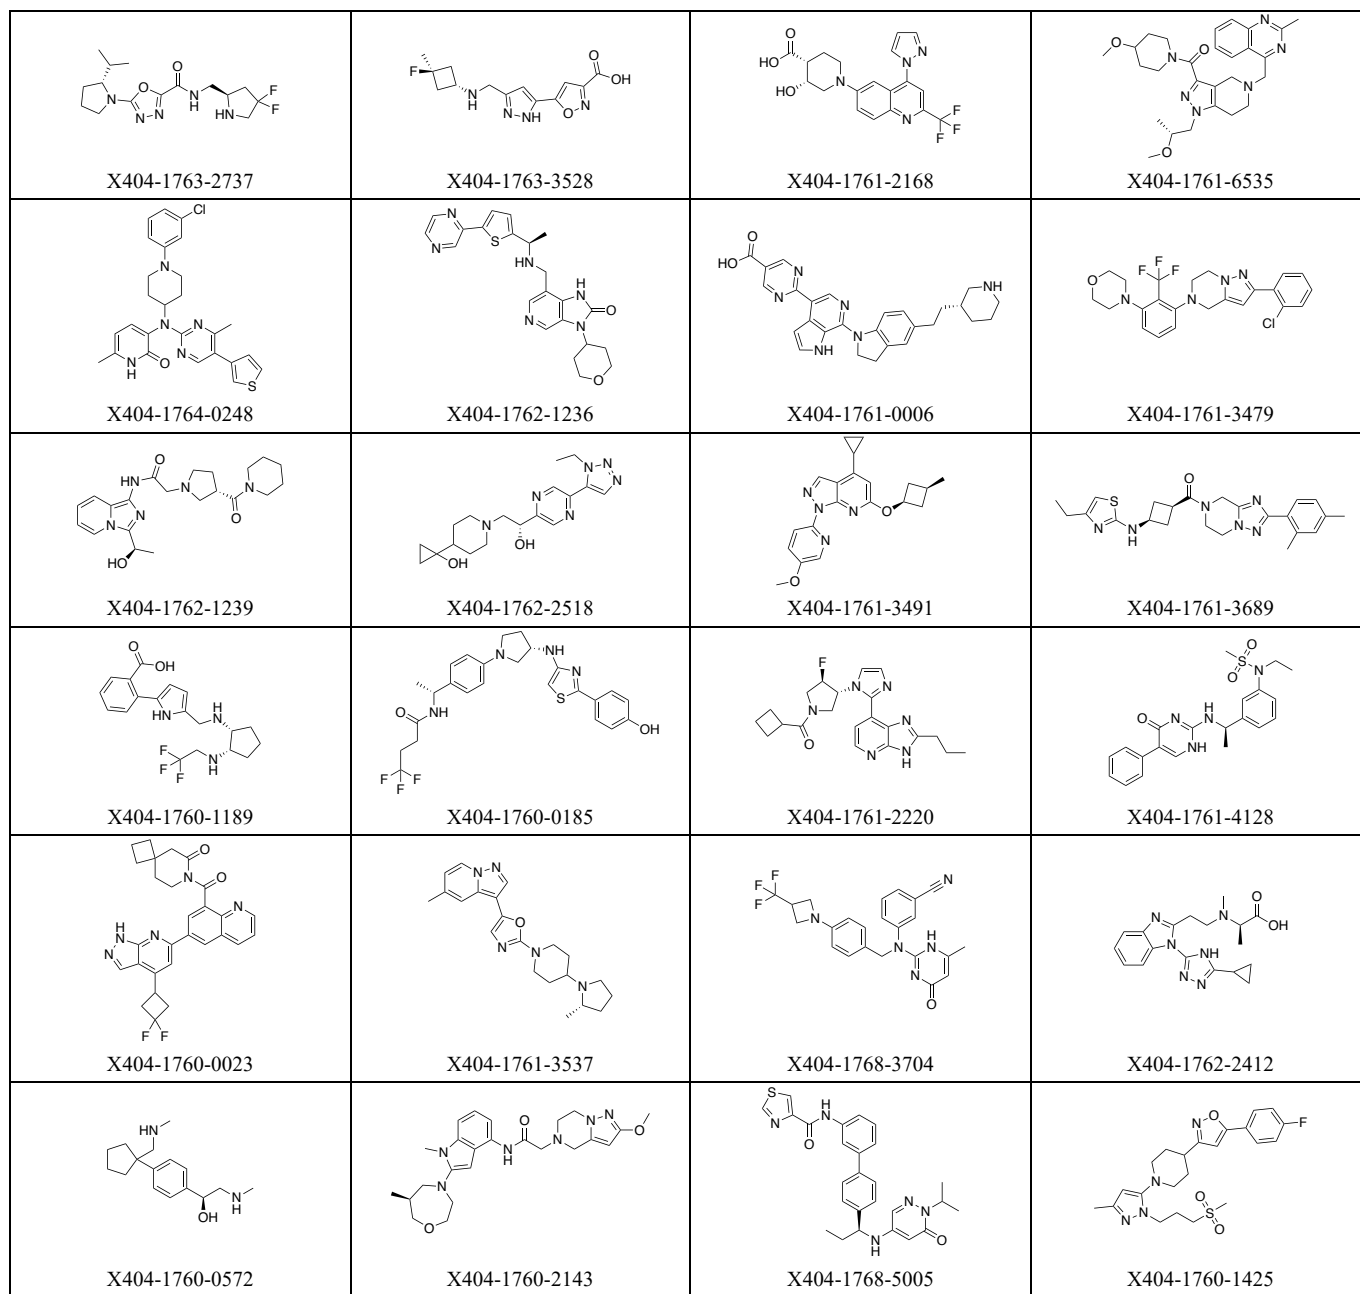 | 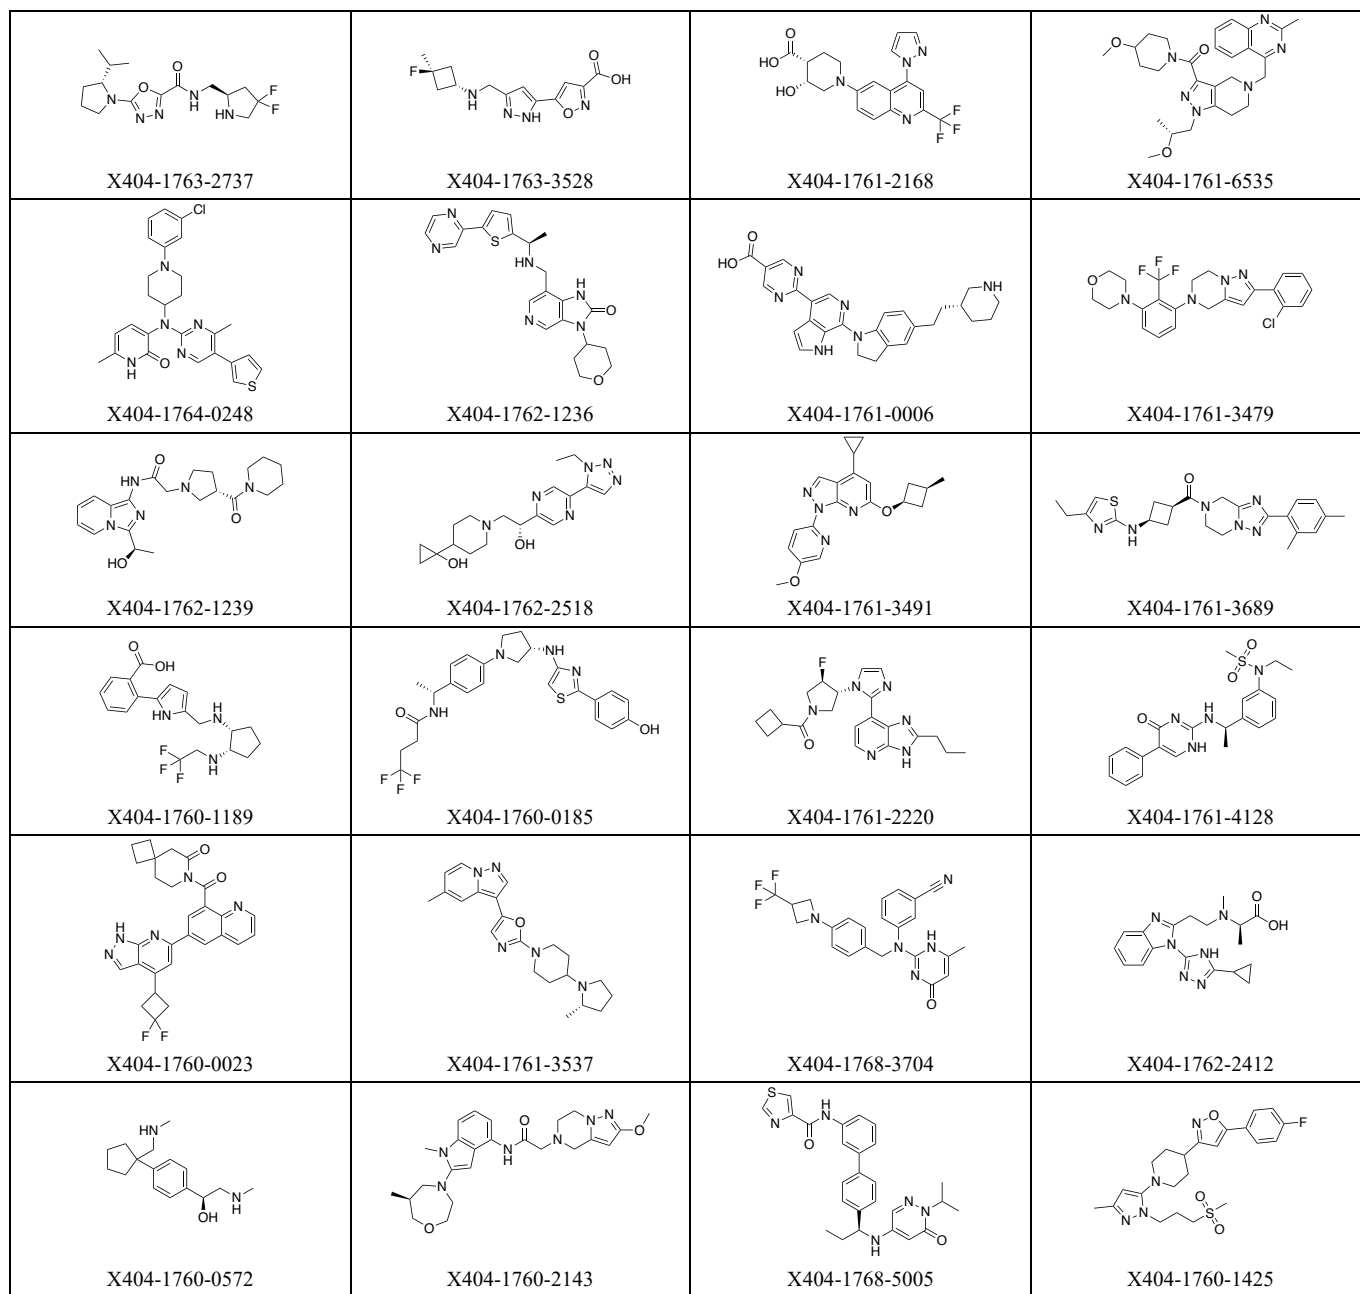 | 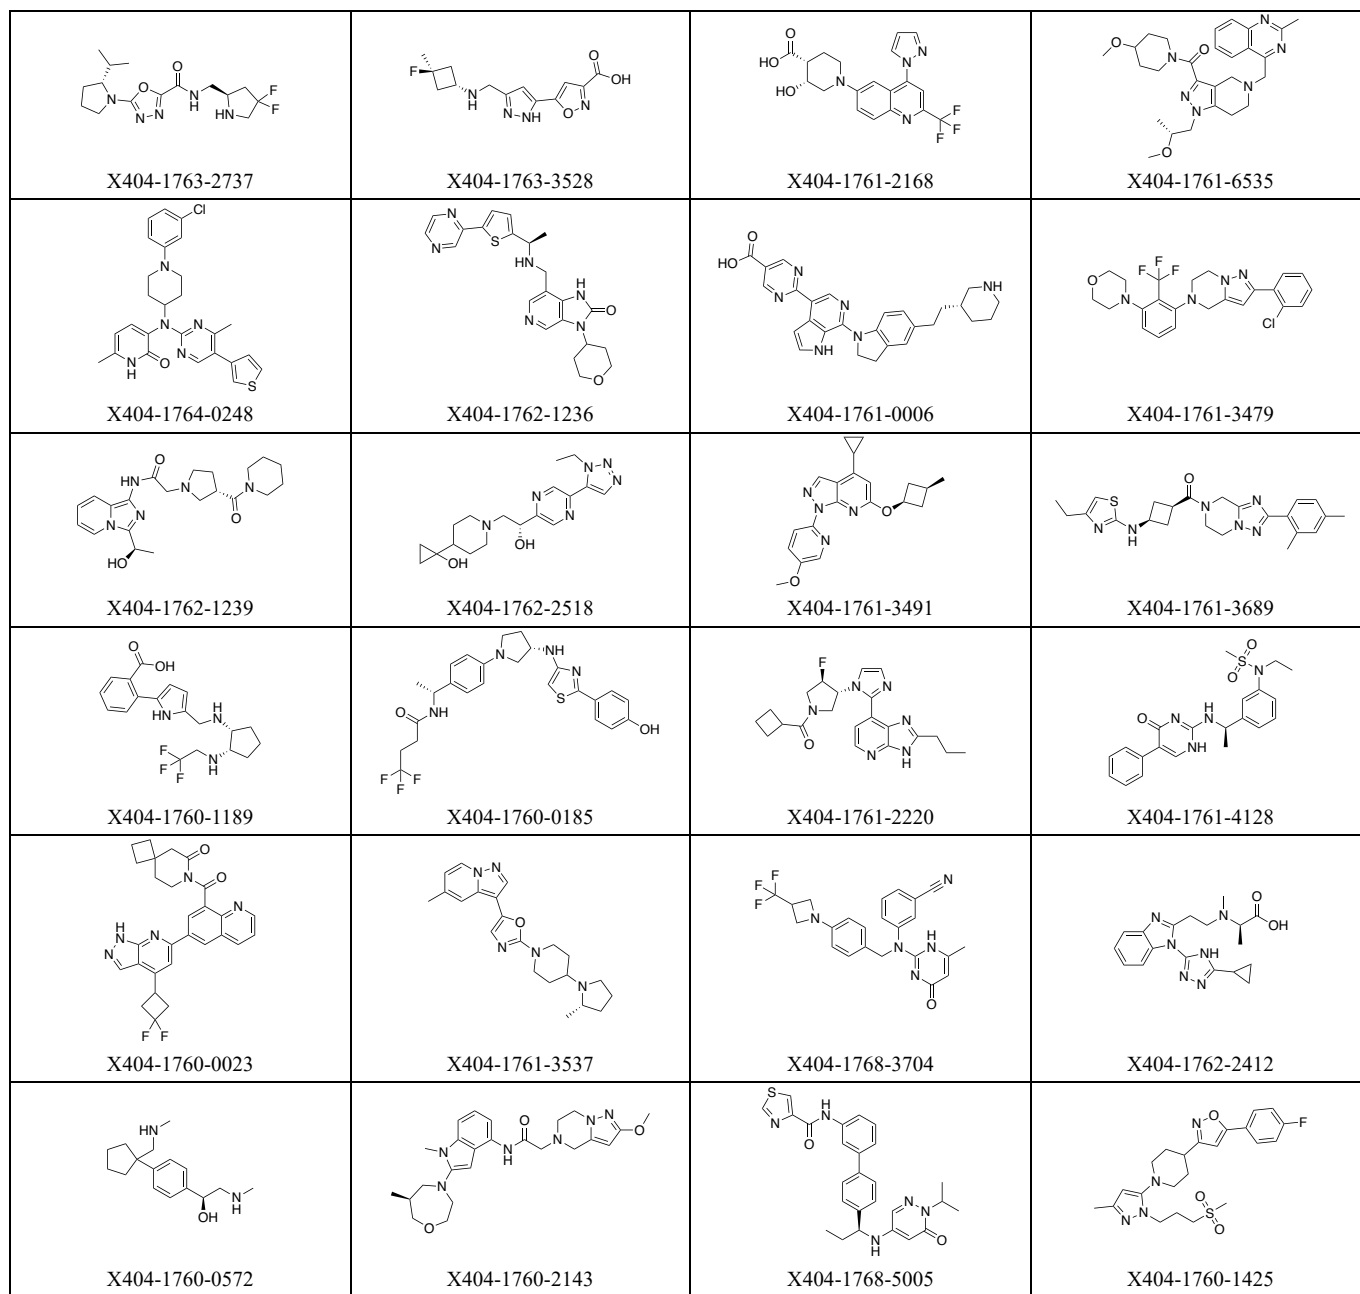 | 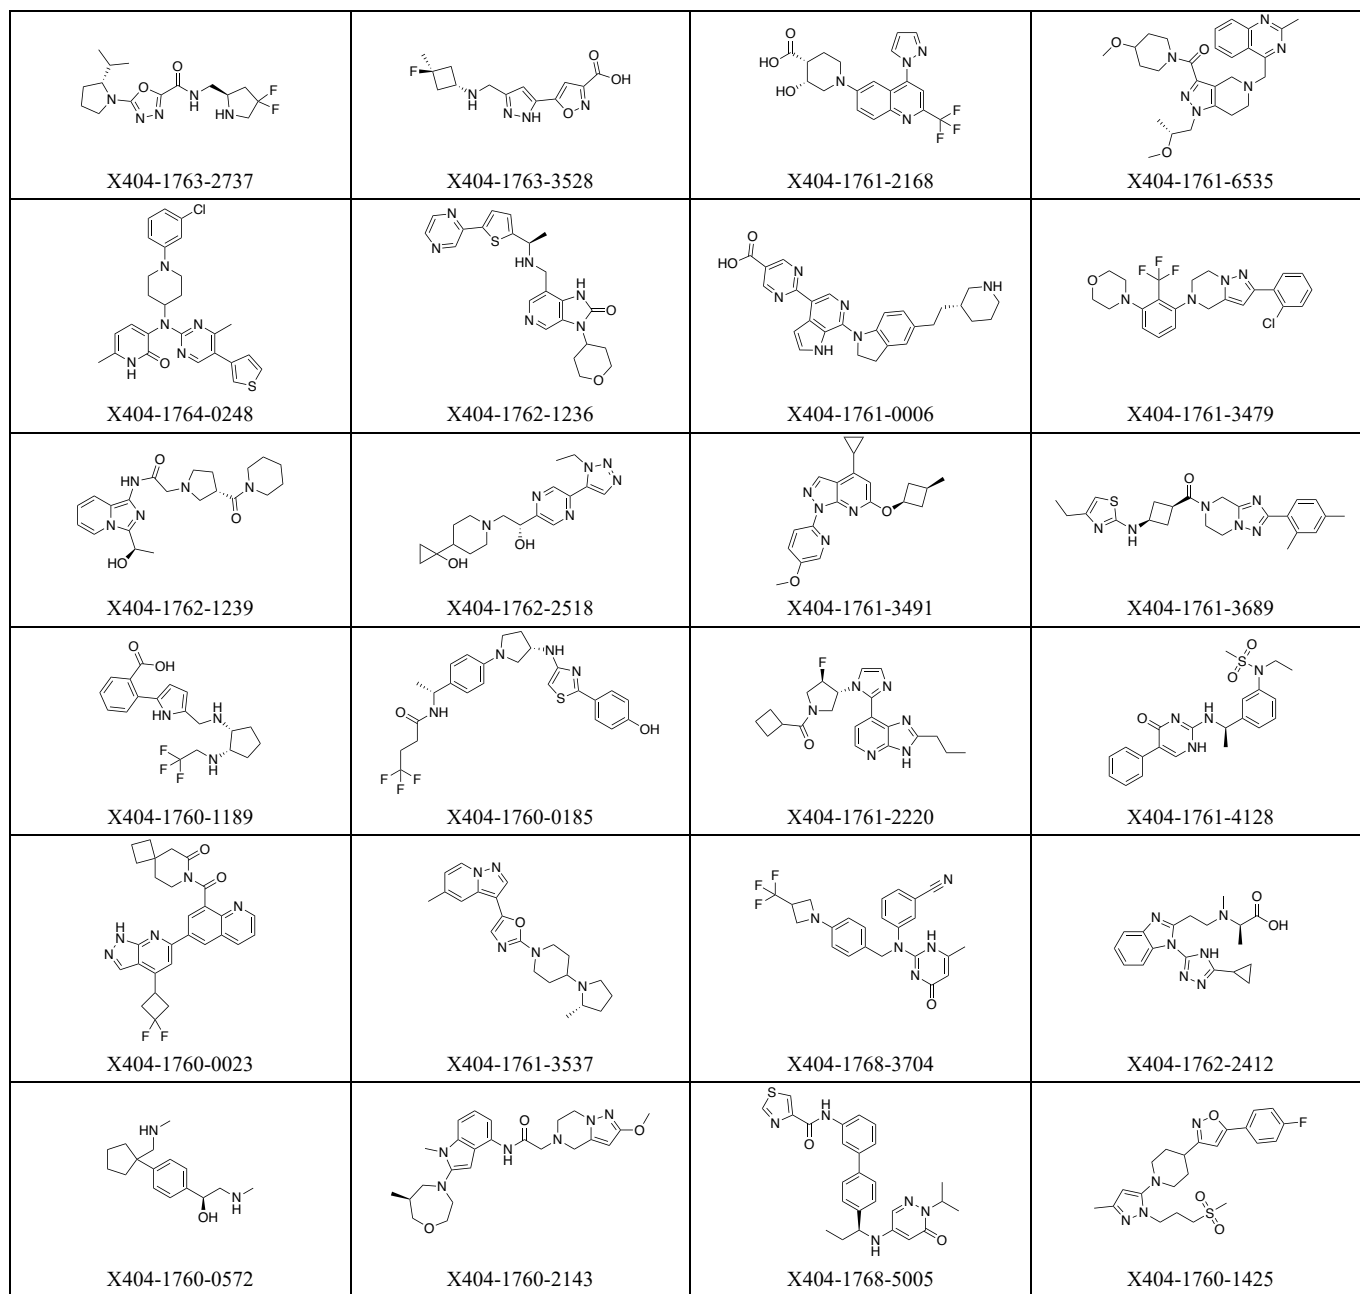 |
| <b>X404-1760-0572</b>                                                               | <b>X404-1760-2143</b>                                                               | <b>X404-1768-5005</b>                                                                | <b>X404-1760-1425</b>                                                                 |
