# Supplementary material for: When Single Answer Is Not Enough: Rethinking Single-Step Retrosynthesis Benchmarks for LLMs
Source: arXiv:2602.03554 source file (2026-05-29)
Supplement: Supplementary file 3 [file reaction_examples.pdf]

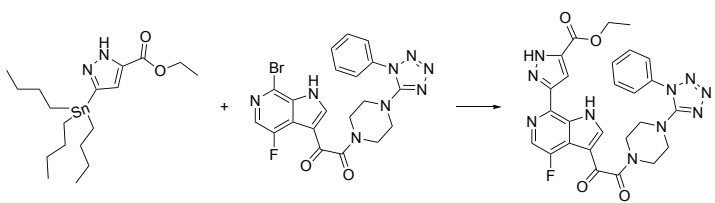

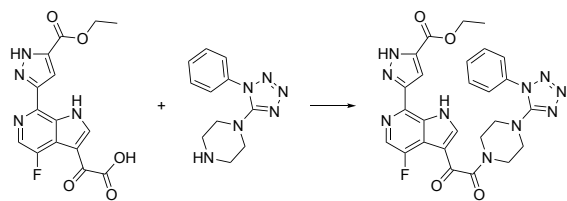

max LC = 2

Synthetic precedent found in US20040110785A1

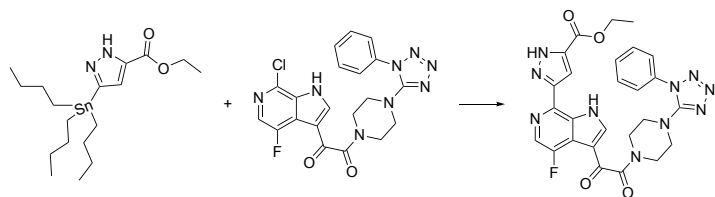

max LC = 2

Synthetic precedent found in US20070249570A1

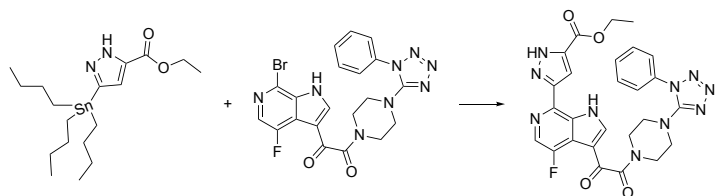

max LC = 5

Synthetic precedent found in US20070249570A1

**Ground truth**

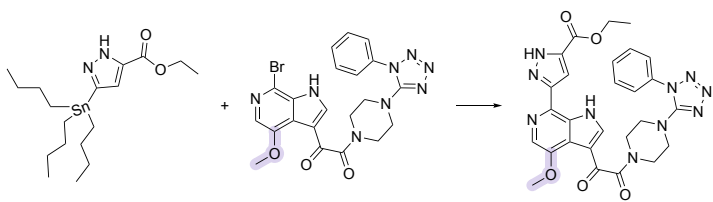

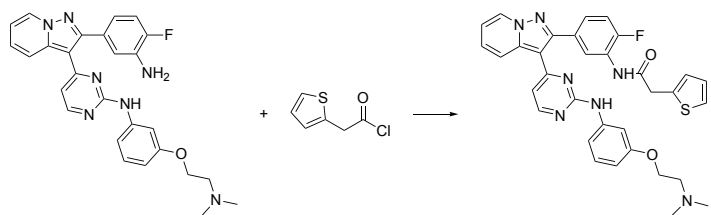

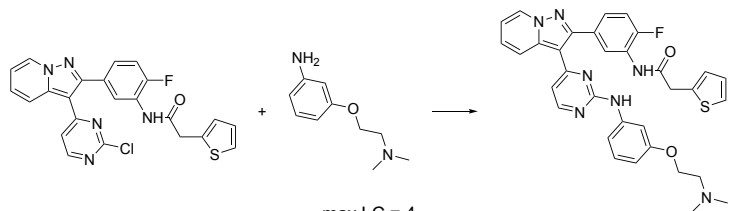

max LC = 4  
*Synthetic precedent found in US20110098296A1*

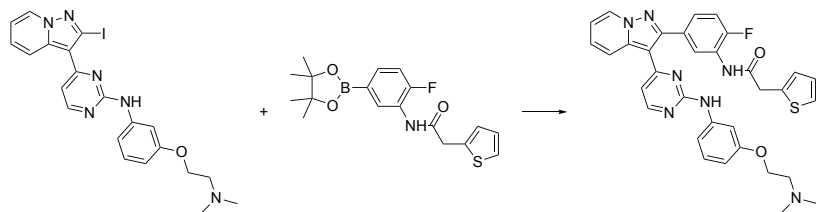

max LC = 1  
*Synthetic precedent found in US20040192767A1*

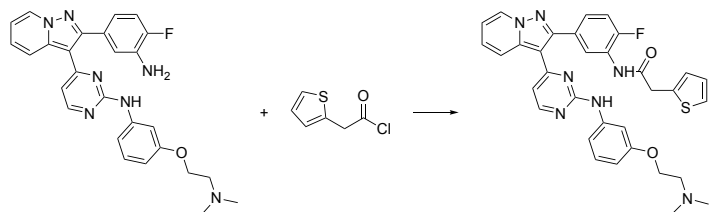

max LC = 5  
*Synthetic precedent found in US20090149456A1*  
**Ground truth**
