# Supplementary material for: When Single Answer Is Not Enough: Rethinking Single-Step Retrosynthesis Benchmarks for LLMs
Source: arXiv:2602.03554 source file (2026-05-29)
Supplement: Supplementary file 4 [file scoring_examples.pdf]

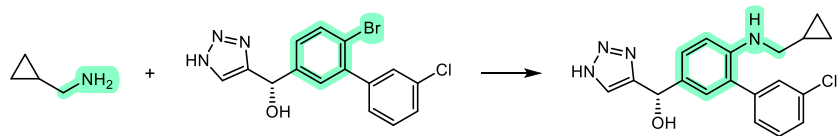

ChemCensor Score = 2

RC SMARTS:

[N&H2:7]-[C:8].Br-[c:6]1:[c:5]:[c:4]:[c:3]:[c:20]:[c:12]:1>>[c:3]1:[c:4]:[c:5]:[c:6](-[N&H1:7]-[C:8]):[c:12]:[c:20]:1

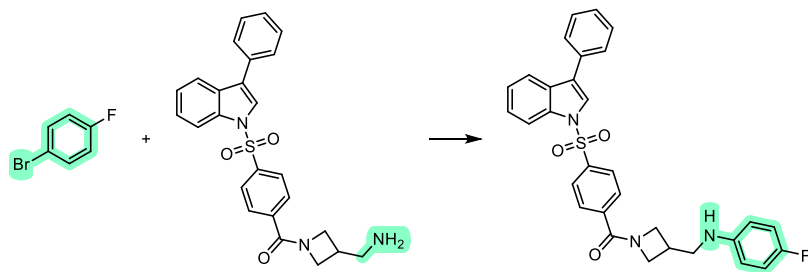

Synthetic precedent with the same RC. The document ID: US20070088018A1

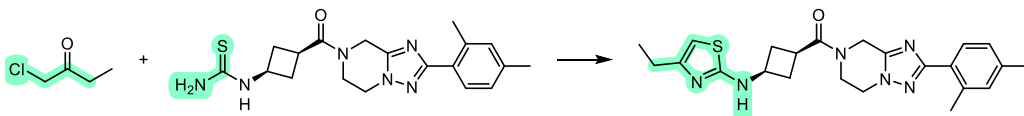

ChemCensor Score = 4

RC SMARTS:

O=[C:3](-[C:2])-[C&H2:4]-Cl.[S:5]=[C:6]-[N&H2:31]>>[C:2]-[c:3]1:[c&H1:4]:[s:5]:[c:6](-[N:7]):[n:31]:1.

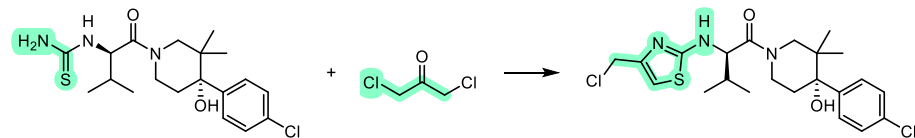

Synthetic precedent with the same RC. The document ID: US20070208056A1

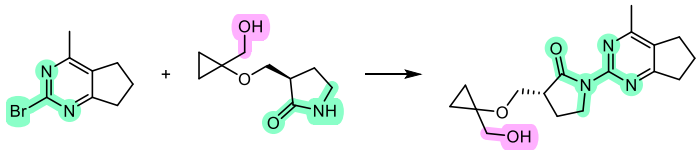

ChemCensor Score = 0

RC SMARTS:

Br-[c:4](-[n:3]):[n:18].[N&H1:5](-[C:6])-[C:16]=[O:17]>>[n:3]:[c:4](-[N:5](-[C:6])-[C:16]=[O:17]):[n:18]

No synthetic precedents with the following FGs: **Primary alcohol**

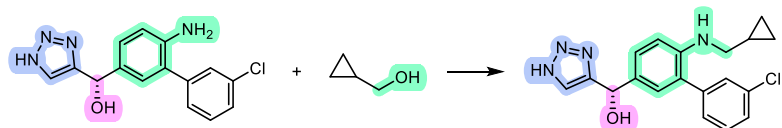

ChemCensor Score = 0

RC SMARTS:

[c:3]1:[c:4]:[c:5]:[c:6](-[N&H2:7]):[c:12]:[c:20]:1.O-[C&H2:8]-[C:9]>>[c:3]1:[c:4]:[c:5]:[c:6](-[N&H1:7]-[C&H2:8]-[C:9]):[c:12]:[c:20]:1

No synthetic precedents with the following FGs: **Secondary alcohol**, **Azole**

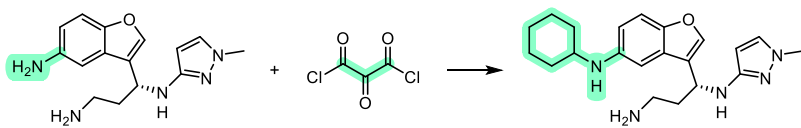

ChemCensor Score = 0

RC SMARTS:

[c:17]-[N&H2:18].O=[C:19](-Cl)-[C:23](=O)-[C:22](=O)-Cl>>[c:17]-[N&H1:18]-[C&H1:19]1-[C&H2:20]-[C&H2:21]-[C&H2:22]-[C&H2:23]-[C&H2:24]-1

No synthetic precedents with this RC
