# Supplementary material for: When Single Answer Is Not Enough: Rethinking Single-Step Retrosynthesis Benchmarks for LLMs
Source: arXiv:2602.03554 source file (2026-05-29)
Supplement: Supplementary file 5 [file ether0_table.tex]

\begin{tabular}{@{}l|c|cccc|c|cccc@{}}
\toprule
\multirow{2}{*}{\textbf{Model}} &
\multicolumn{5}{c|}{\textbf{URSA-expert-2026}} &
\multicolumn{5}{c}{\textbf{USPTO-50K-test}} \\
\cline{2-6}\cline{7-11}
& \multirow{2}{*}{\textbf{Unique}} & \multirow{2}{*}{\textbf{Max}} & \multicolumn{3}{c|}{\textbf{Av. PT-Top-K CC}}
& \multirow{2}{*}{\textbf{Unique}} & \multirow{2}{*}{\textbf{Max}} & \multicolumn{3}{c}{\textbf{Av. PT-Top-K CC}} \\
&  &  & \textbf{@3} & \textbf{@5} & \textbf{@10}
&  &  & \textbf{@3} & \textbf{@5} & \textbf{@10} \\
\midrule
ether0, original prompts                     & 20\% & 1.01 & 0.55 & 0.35 & 0.17 & 19\% & 2.08 & 1.07 & 0.67 & 0.34 \\
ether0, revised prompts                   & 24\% & 1.25 & 0.73 & 0.47 & 0.24 & 25\% & 2.17 & 1.24 & 0.79 & 0.40 \\
\bottomrule
\end{tabular}
