# Supplementary material for: When Single Answer Is Not Enough: Rethinking Single-Step Retrosynthesis Benchmarks for LLMs
Source: arXiv:2602.03554 source file (2026-05-29)
Supplement: Supplementary file 6 [file FG_errors.tex]

\section{FG–related error profiles}
\label{app:FG_errors}

\begin{figure*}[t]
  \centering

  \begin{minipage}{\textwidth}
    \centering
    \includegraphics[width=0.45\textwidth]{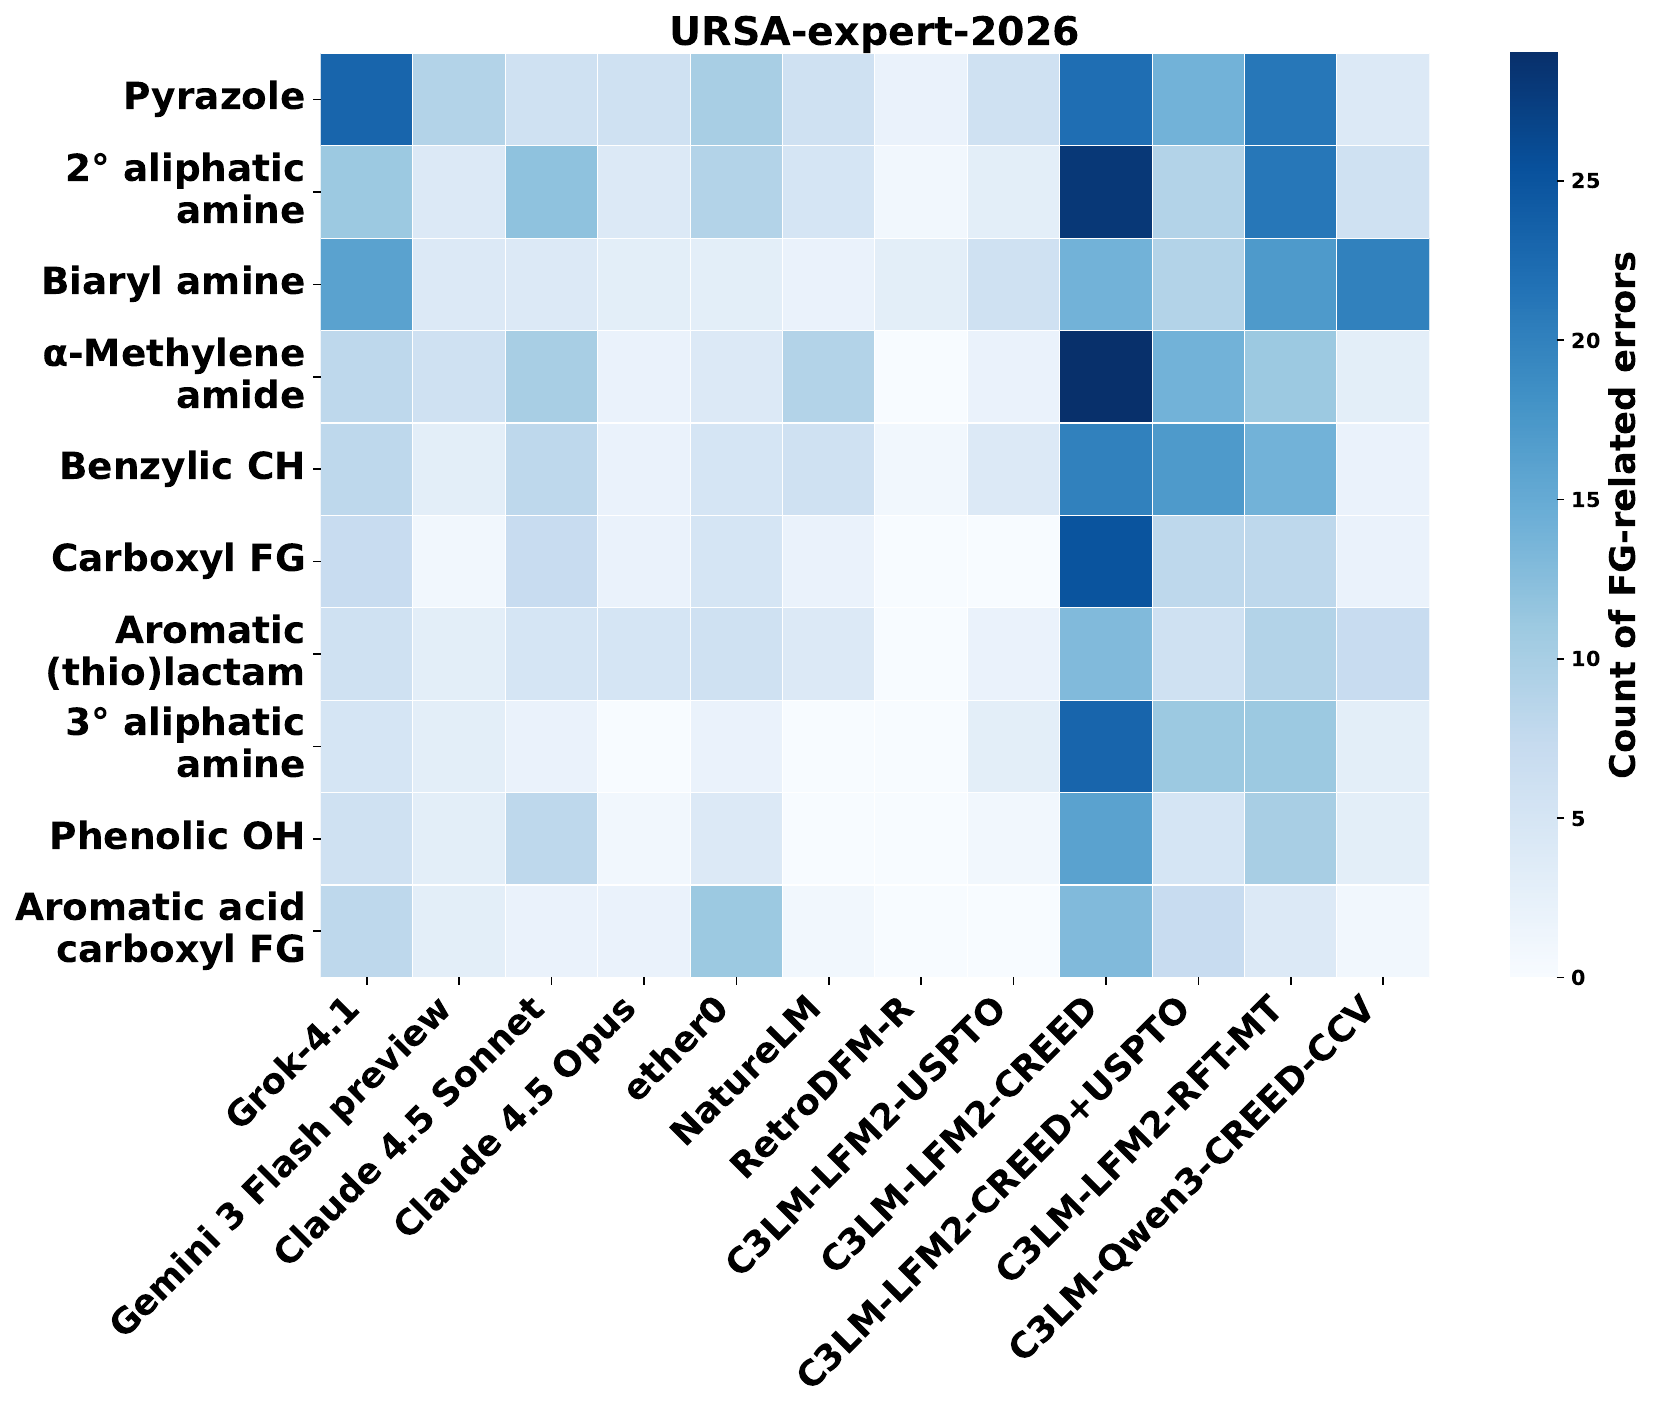}\hspace{1.3cm}
    \includegraphics[width=0.45\textwidth]{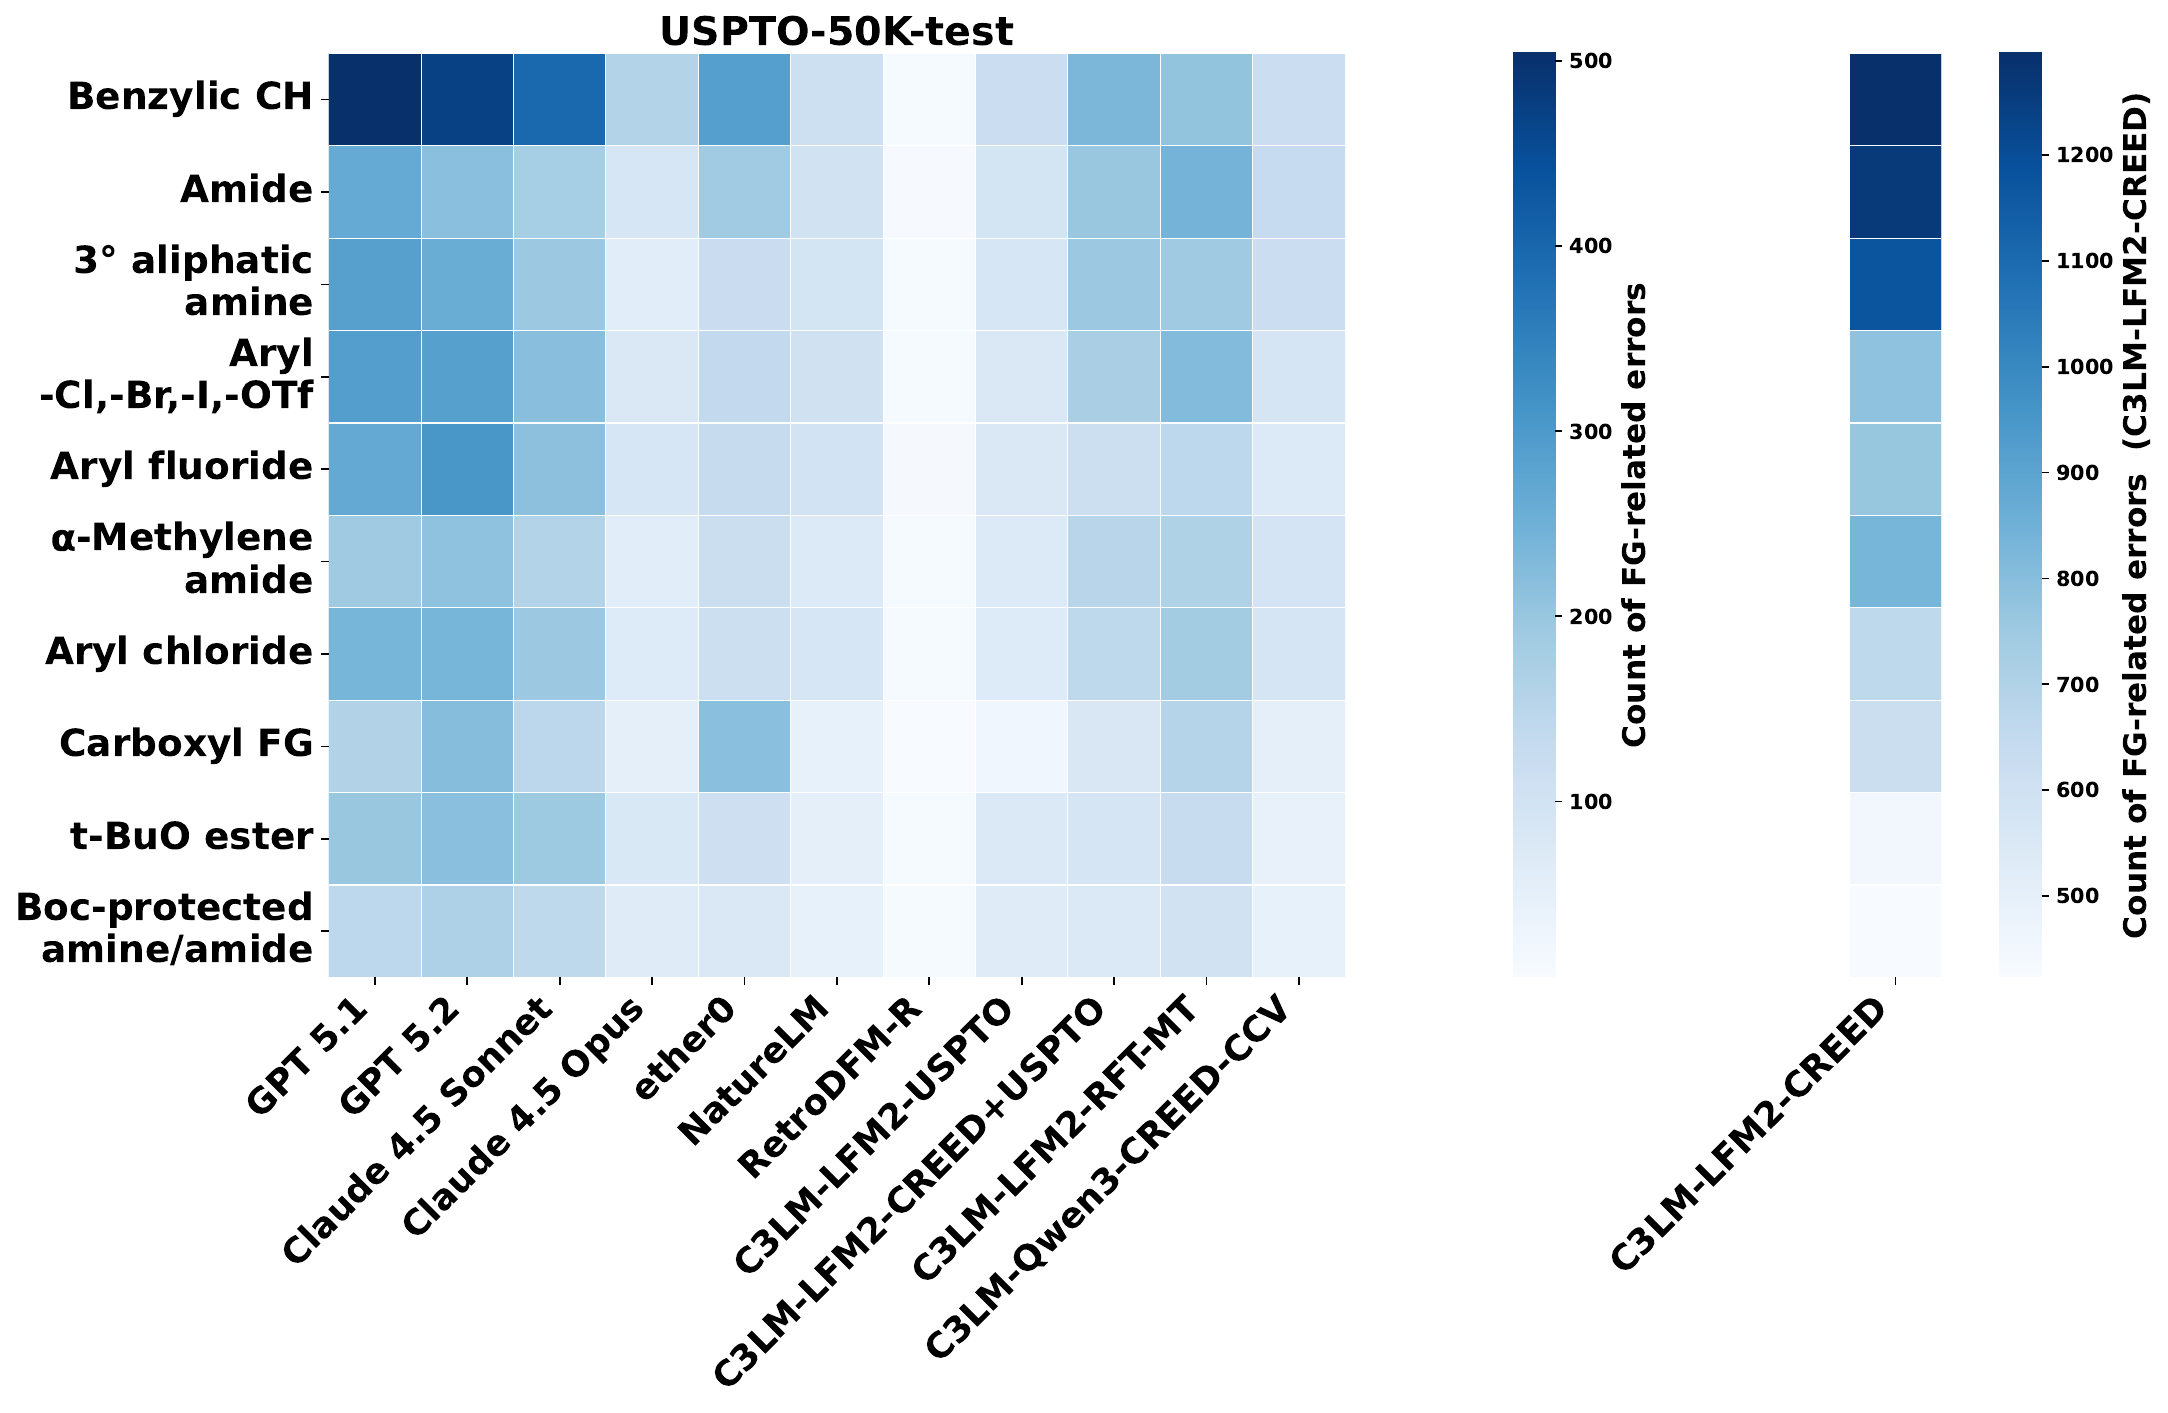}
  \end{minipage}
  \caption{The comparison of FG–related error profiles across models and benchmarking sets. Heat maps show the count of ChemCensor FG incompatibility errors for each model across the Top-10 models by means of \textbf{Av.~PT-Top-10 CC} (see \autoref{tab:chemcensor_benchmark_results}), darker cells indicate a higher error number.}
  \label{fig:fg_heatmap_by_model_full}
\end{figure*}
